# Supplementary material for: Drug Selection via Joint Push and Learning to Rank
Source: arXiv:1801.07691 ancillary file (2018-05-18)
Supplement: Supplementary file 1 [file supp.pdf]

# Drug Selection via Joint Push and Learning to Rank (Supplementary Materials)

Yicheng He*, Junfeng Liu*, and Xia Ning‡

## S1 Alternating Optimization for pLETORg

**Algorithm S1** Alternating Optimization for pLETORg

**Require:** cell lines $\{\mathcal{C}\}$ with drug sensitivities, cell line similarity matrix $W \in \mathbb{R}^{m\times m}$
**Require:** latent dimension $l$, weighting parameter $\alpha$, regularization parameters $\beta$ and $\gamma$
**Ensure:** $\alpha \in [0,1]$, $\beta \geq 0$, $\gamma \geq 0$

$U \leftarrow$ a random $l \times m$ matrix
$V \leftarrow$ a random $l \times n$ matrix
**while** not converged **do**
  fix $V$ and solve for $U$ using gradient descent (Equation S1,S2 in Section S2) in supplementary materials
  fix $U$ and solve for $V$ using gradient descent (Equation S3,S4 in Section S2) in supplementary materials
**end while**
**return** $U$ and $V$

## S2 Gradient Decent and Update Rules

$$\mathbf{u}_p^{(t+1)} \leftarrow \mathbf{u}_p^{(t)} - \eta\nabla_{\mathbf{u}_p}\mathcal{L}(U^{(t)}, V^{(t)}) \tag{S1}$$

$$\begin{aligned}\nabla_{\mathbf{u}_p}\mathcal{L} = &\frac{(1-\alpha)}{n_p^+ n_p^-}\sum_{d_i\in\mathcal{C}_p^-}\left\{\tilde{H}_p(d_j^-)\sum_{d_j\in\mathcal{C}_p^+}\frac{\mathbf{v}_i-\mathbf{v}_j}{1+\exp(\mathbf{u}_p^\mathsf{T}(\mathbf{v}_j-\mathbf{v}_i))}\right\}\\ &+\frac{\alpha}{|\{f_p(d_i^+) > f_p(d_j^+)\}|}\sum_{f_p(d_i^+)>f_p(d_j^+)}\left\{\frac{\mathbf{v}_j-\mathbf{v}_i}{1+\exp(\mathbf{u}_p^\mathsf{T}(\mathbf{v}_i-\mathbf{v}_j))}\right\}\\ &+\frac{\alpha}{|\{f_p(d_i^-) > f_p(d_j^-)\}|}\sum_{f_p(d_i^-)>f_p(d_j^-)}\left\{\frac{\mathbf{v}_j-\mathbf{v}_i}{1+\exp(\mathbf{u}_p^\mathsf{T}(\mathbf{v}_i-\mathbf{v}_j))}\right\}\\ &+\frac{\beta}{m}\mathbf{u}_p+\frac{\gamma}{m^2}\sum_{q=1}^{m}w_{pq}(\mathbf{u}_p-\mathbf{u}_q)\end{aligned} \tag{S2}$$

$$\mathbf{v}_i^{(t+1)} \leftarrow \mathbf{v}_i^{(t)} - \eta\nabla_{\mathbf{v}_i}\mathcal{L}(U^{(t+1)}, V^{(t)}) \tag{S3}$$

$$\begin{aligned}\nabla_{\mathbf{v}_i}\mathcal{L} = &\sum_{\mathcal{C}_p\in\Gamma_i^-}\frac{(1-\alpha)}{n_p^+ n_p^-}\sum_{d_j\in\mathcal{C}_p^-}\left\{\tilde{H}_p(d_j^-)\sum_{d_k\in\mathcal{C}_p^+}\frac{\mathbf{u}_p}{1+\exp(\mathbf{u}_p^\mathsf{T}(\mathbf{v}_k-\mathbf{v}_j))}\right\}\\ &-\sum_{\mathcal{C}_p\in\Gamma_i^+}\frac{(1-\alpha)}{n_p^+ n_p^-}\sum_{d_j\in\mathcal{C}_p^-}\left\{\tilde{H}_p(d_j^-)\sum_{d_k\in\mathcal{C}_p^+}\frac{\mathbf{u}_p}{1+\exp(\mathbf{u}_p^\mathsf{T}(\mathbf{v}_k-\mathbf{v}_j))}\right\}\\ &+\sum_{p=1}^{m}\frac{\alpha}{|\{f_p(d_j^+) > f_p(d_k^+)\}|}\left\{\sum_{f_p(d_j^+)>f_p(d_i^+)}\frac{\mathbf{u}_p}{1+\exp(\mathbf{u}_p^\mathsf{T}(\mathbf{v}_j-\mathbf{v}_i))}\right\}\\ &-\sum_{p=1}^{m}\frac{\alpha}{|\{f_p(d_j^+) > f_p(d_k^+)\}|}\left\{\sum_{f_p(d_i^+)>f_p(d_k^+)}\frac{\mathbf{u}_p}{1+\exp(\mathbf{u}_p^\mathsf{T}(\mathbf{v}_i-\mathbf{v}_k))}\right\}\\ &+\sum_{p=1}^{m}\frac{\alpha}{|\{f_p(d_j^-) > f_p(d_k^-)\}|}\left\{\sum_{f_p(d_j^-)>f_p(d_i^-)}\frac{\mathbf{u}_p}{1+\exp(\mathbf{u}_p^\mathsf{T}(\mathbf{v}_j-\mathbf{v}_i))}\right\}\\ &-\sum_{p=1}^{m}\frac{\alpha}{|\{f_p(d_j^-) > f_p(d_k^-)\}|}\left\{\sum_{f_p(d_i^-)>f_p(d_k^-)}\frac{\mathbf{u}_p}{1+\exp(\mathbf{u}_p^\mathsf{T}(\mathbf{v}_i-\mathbf{v}_k))}\right\}\\ &+\frac{\beta}{n}\mathbf{v}_i\end{aligned} \tag{S4}$$

where $\eta$ is the learning rate, where $\Gamma_i^-$ is the set of cell lines for which drug $d_i$ is insensitive, $\Gamma_i^+$ is the set of cell lines for which $d_i$ is sensitive.


- *Y. He* and J. Liu* have equal contribution to this work and are co-first authors.*
- *Y. He, J. Liu and X. Ning are with the Department of Computer and Information Science, Indiana University - Purdue University Indianapolis.*
- *X. Ning is with the Center for Computational Biology and Bioinformatics, Indiana University School of Medicine.*
  *Address: 410 West 10th St., HITS 5011, Indianapolis, IN 46202, USA*
  *‡E-mail: xning@iupui.edu*

## S3 Gene Selection Scheme

Fig. S1 demonstrates the regression method for gene selection as described in Section 4.4 in the main manuscript.

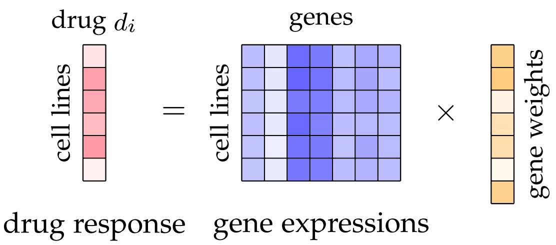


**Fig. S1:** Regression for gene selection

## S4 Cell Line Similarity Comparison

Fig. S2 shows the gene expression similarities of all such cell lines and their latent vector similarities.

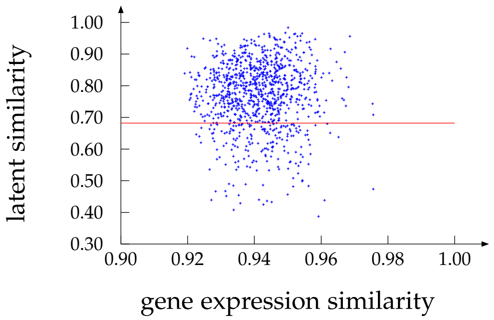


**Fig. S2:** Cell Line Similarity Comparison

## S5 Data Split Protocol for Testing New Cell Lines

To split cell lines into training and testing set for testing new cell lines as in Fig. 4, we apply the following data split protocol. We first define a candidate set of cell lines, denoted as $\mathcal{S}$. We also define that two cell lines are sufficiently similar if their similarity in gene expressions is above a threshold $t$. We construct a training set of cell lines, denoted as $\mathcal{S}_{tr}$, and a testing set of cell lines, denoted as $\mathcal{S}_{ts}$, as follows:

1) initialize $\mathcal{S}_{tr}$ and $\mathcal{S}_{ts}$ as empty, $\mathcal{S}$ as the set of all available cell lines, and $t$ as the 90 percentile of all pair-wise cell line similarities in $\mathcal{S}$;
2) sort the cell lines in $\mathcal{S}$ based on the number of their sufficiently similar cell lines in $\mathcal{S}$ in decreasing order;
3) find the cell line that has the maximum number of sufficiently similar cell lines in $\mathcal{S}$, denoted as $\mathcal{C}^0_{sim}$, and the cell line that is most similar to $\mathcal{C}^0_{sim}$ in $\mathcal{S}$, denoted as $\mathcal{C}^1_{sim}$;
4) $\mathcal{S}_{tr} = \mathcal{S}_{tr} \cup \{\mathcal{C}^1_{sim}\}$, $\mathcal{S}_{ts} = \mathcal{S}_{ts} \cup \{\mathcal{C}^0_{sim}\}$, $\mathcal{S} = \mathcal{S} - \{\mathcal{C}^0_{sim}, \mathcal{C}^1_{sim}\}$;
5) update $t$ as the 90 percentile of all pair-wise similarities in the current $\mathcal{S}$;
6) repeat 2 to 5 until $\mathcal{S}_{ts}$ is sufficiently large;
7) $\mathcal{S}_{tr} = \mathcal{S}_{tr} \cup \mathcal{S}$.

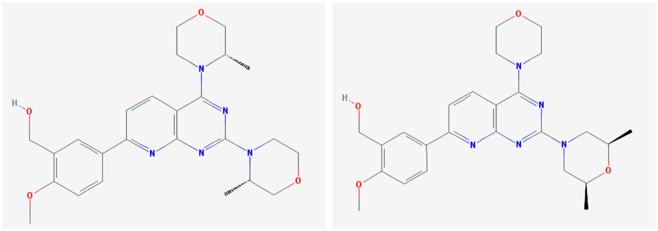

(a) BRD-K69932463[1] (b) BRD-K67566344[2]

**Fig. S3:** Drug structures: BRD-K69932463 vs BRD-K67566344

## S6 Drug Latent Vectors as New Drug Features

Both Fig. 7 and Fig. 8 show that higher/lower Tanimoto coefficients, and thus, higher/lower similarities in drug structures, do not necessarily indicate similar/different drug rankings or sensitivities (i.e., no row-block patterns in Fig. 7 or Fig. 8). For example, drug BRD-K69932463 (Fig. 3(a)) and drug BRD-K67566344 (Fig. 3(b)) are very similar in their intrinsic structures (i.e., $\texttt{TAN}_{\text{AF}}$ of these two drugs is above 99 percentile among all drug pairs), and they do share similar sensitivities in several cell lines, for example, in cell line HS888T (organ: bone, disease: osteosarcoma) and HS940T (organ: skin, disease: malignant melanoma), both of the drugs are sensitive. However, on many other cell lines, their sensitivity profiles are very different. For example, BRD-K69932463 is sensitive in cell line NCIH226 (organ: lung, disease: squamous cell carcinoma), HCC1500 (organ: breast, disease: ductal carcinoma) and OV56 (organ: ovary, disease: carcinoma), in which BRD-K67566344 is insensitive. Among 791 cell lines that have response values on both BRD-K69932463 and BRD-K67566344, the two drugs have different sensitivity labels on 456 cell lines. Please note that the above observation does not contradict to the well accepted conclusion that similar drugs (in terms of their intrinsic structures) have similar effectiveness (measured independently of any other drugs; e.g., in $\text{IC}_{50}$), as drugs of similar effectiveness in different cell lines may be ranked differently.

The difference among drugs of high intrinsic structure similarities is well captured by the drug latent vectors: $\texttt{COS}_{\text{L}}$ between the latent vectors of drug BRD-K69932463 and drug BRD-K67566344 is below 17 percentile among all drug pairs. This indicates that drug intrinsic structures are not discriminating enough in accurately predicting drug rankings in cell lines, whereas drug latent vectors derived from drug prioritization tasks are more informative in better differentiating drug sensitivities in cell lines. In fact, BRD-K69932463 (with active compound AZD8055) is used to treat diseases such as gliomas and liver cancer[1]. BRD-K67566344 is only know to be an inhibitor of MTOR kinase[2], and may have some potential to treat diseases such as cancers. As a matter of fact, $\Delta$r% is strongly negatively correlated to $\texttt{COS}_{\text{L}}$ with a correlation coefficient $-0.558$, that is, on average, if two drugs are ranked very differently, their latent vectors are more different. However, the correlation between $\Delta$r% and $\texttt{TAN}_{\text{AF}}$ is nearly 0 (correlation coefficient $-0.056$). This

1. https://pubchem.ncbi.nlm.nih.gov/compound/25262965
2. https://pubchem.ncbi.nlm.nih.gov/compound/16736978

indicates the advance of using ranking-specific drug latent vectors that are derived from drug ranking tasks as new drug features, compared to the ranking-independent drug structures, in predicting drug rankings and sensitivities.

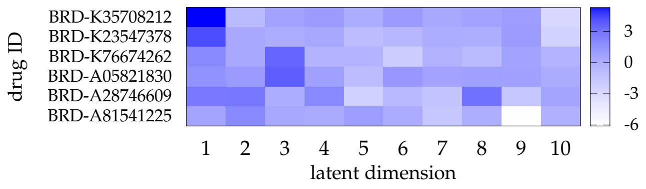


(a) Sensitive Drugs

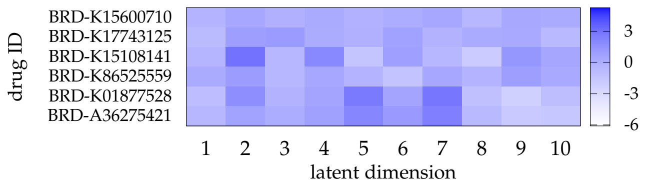


(b) Insensitive Drugs

**Fig. S4:** BL70 – Haematopoietic and Lymphoid Tissue ($\theta$=2)

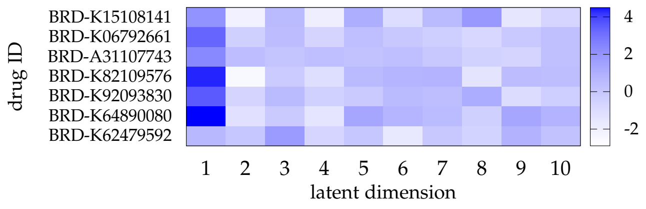


(a) Sensitive Drugs

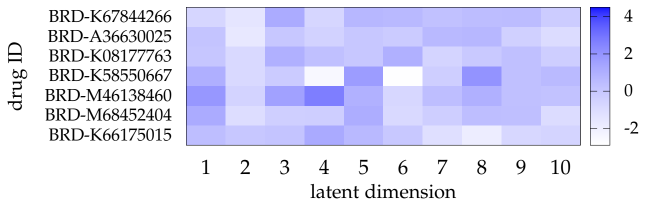


(b) Insensitive Drugs

**Fig. S5:** CAL51 – Breast ($\theta$=5)

## S7 Interpretability of Drug Latent Vectors

The drug latent vectors learned from pLETORg inherently suffer from the lack of interpretability. It is not easy to understand/explain what each of the latent dimensions represents or whether they correlate to any mechanisms of actions. This is because the latent vectors are learned only with respect to the goal of optimizing the drug ranking structures, without any potential MOA (if ever known) or causal features (if ever known) explicitly modeled. Even though, we try to visualize the latent vectors and decipher whether the latent dimensions encode useful information. Such information would provide insights to further development, quantification and selection of potential drugs.

Fig. S4 and Fig. S5 present two examples of learned drug latent vectors for cell line BL70 – haematopoietic and lymphoid tissue and CAL51 – breast, respectively. The sensitive/insensitive drugs are sorted based on their sensitivity values in decreasing order. These two figures show that the latent dimensions of drug latent vectors do represent signals that differentiate sensitive and insensitive drugs. For example, in cell line BL70 in Fig. S4, the 1st drug latent dimension corresponds to signals that are very strong in sensitive drugs (stronger in more sensitive drugs), but very weak in insensitive drugs; the 5th and 7th drug latent dimensions represent signals that are very weak in sensitive drugs, but very strong in insensitive drugs (stronger in more insensitive drugs). Similarly, in cell line CAL51 in Fig. S5, the 1st drug latent dimension corresponds to signals that are strong in sensitive drugs (stronger in less sensitive drugs), but weak in insensitive drugs (weaker in less insensitive drugs). Further wet-lab experiments could help correlate such drug latent dimensions with specific drug properties. Therefore, the latent vectors could help uncover hidden fact that a certain drug may actually exhibit certain properties, and thus inform potential drug repositioning [1] practice.

## S8 Additional References

Pairwise learning-to-rank methods [2]; Listwise learning-to-rank methods [3]; Multi-task learning [4]; Multiple kernel learning [5]; Tanimoto coefficients [6]; Concordance index [7];

## References

[1] T. I. Oprea and J. Mestres, "Drug repurposing: Far beyond new targets for old drugs," *The AAPS Journal*, vol. 14, no. 4, pp. 759–763, Dec 2012.

[2] C. J. Burges, R. Ragno, and Q. V. Le, "Learning to rank with nonsmooth cost functions," in *Advances in Neural Information Processing Systems 19*, P. B. Schölkopf, J. C. Platt, and T. Hoffman, Eds. MIT Press, 2007, pp. 193–200.

[3] G. Lebanon and J. D. Lafferty, "Cranking: Combining rankings using conditional probability models on permutations," in *Proceedings of the Nineteenth International Conference on Machine Learning*, ser. ICML '02. San Francisco, CA, USA: Morgan Kaufmann Publishers Inc., 2002, pp. 363–370.

[4] R. Caruana, "Multitask learning," *Machine Learning*, vol. 28, no. 1, pp. 41–75, Jul 1997.

[5] T. Hofmann, B. Sch olkopf, and A. J. Smola, "Kernel methods in machine learning," *Ann. Statist.*, vol. 36, no. 3, pp. 1171–1220, 06 2008.

[6] P. Willett, J. M. Barnard, and G. M. Downs, "Chemical similarity searching," *Journal of Chemical Information and Computer Sciences*, vol. 38, no. 6, pp. 983–996, 1998.

[7] F. E. Harrell, K. L. Lee, and D. B. Mark, "Multivariable prognostic models: issues in developing models, evaluating assumptions and adequacy, and measuring and reducing errors," *Statistics in medicine*, vol. 15, no. 4, pp. 361–387, 1996.

## S9 List of Selected Genes

**TABLE S1:** List of Selected Genes

| Gene Encodings | | | | | |
|---|---|---|---|---|---|
| ABCB1 | ABCC3 | ABLIM3 | ACADM | ACN9 | ACSL3 |
| ACTB | ACTG1 | ACTN4 | ACTR10 | ADAR | ADI1 |
| ADM | ADORA2B | ADSL | AGPAT9 | AGR2 | AHCY |
| AHR | AHSA1 | AIDA | AIFM2 | AIM1 | AKR1B1 |
| AKR1B10 | AKR1C1 | AKR1C2 | AKR1C3 | ALDH1A1 | ALDH1A3 |
| ALDH2 | ALDH3A1 | ALDH3A2 | ALDH9A1 | ALDOA | ALG8 |
| ALYREF | AMIGO2 | AMOTL2 | ANKMY2 | ANLN | ANP32B |
| ANP32E | ANXA2 | ANXA2P2 | ANXA3 | ANXA4 | ANXA5 |
| ANXA7 | AP1S2 | AP2M1 | AP2S1 | AP3S1 | APEX1 |
| APOA1BP | APOBEC3B | APOD | ARCN1 | ARF4 | ARHGAP15 |
| ARHGAP18 | ARHGAP29 | ARHGEF6 | ARL6IP1 | ARL6IP5 | ARMCX6 |
| ARNT2 | ARPC1A | ARPC1B | ARPC2 | ARPC3 | ARRDC4 |
| ASAP2 | ASRGL1 | ASS1 | ASUN | ATF4 | ATIC |
| ATOX1 | ATP1B1 | ATP5B | ATP5C1 | ATP5I | ATP5J |
| ATP5L | ATP6 | ATP6AP1 | ATP6V0B | ATP6V0C | ATP6V0D1 |
| ATP6V0E2 | ATP6V1E1 | ATP6V1F | AUP1 | AVPI1 | AXL |
| AZGP1 | B2M | BACE2 | BAG3 | BAMBI | BANF1 |
| BCAP31 | BCAR3 | BCAT1 | BCL11A | BDNF | BEX2 |
| BICC1 | BIRC2 | BLCAP | BLOC1S2 | BLVRB | BMI1 |
| BMP4 | BNIP3 | BOLA3 | BST2 | BUD31 | BZW1 |
| BZW2 | C10ORF116 | C11ORF10 | C12ORF23 | C12ORF57 | C12ORF75 |
| C14ORF119 | C14ORF166 | C14ORF2 | C15ORF48 | C16ORF54 | C16ORF80 |
| C17ORF58 | C19ORF10 | C19ORF33 | C19ORF53 | C1QBP | C1ORF51 |
| C20ORF24 | C20ORF30 | C2ORF28 | C4ORF19 | C5ORF43 | C9ORF3 |
| CA12 | CAMLG | CAP1 | CAP2 | CAPG | CAPNS1 |
| CAV1 | CAV2 | CBX1 | CCDC72 | CCDC99 | CCL2 |
| CCNB1 | CCND1 | CCNG1 | CCT2 | CCT3 | CCT6A |
| CCT7 | CD151 | CD164 | CD24 | CD55 | CD59 |
| CD63 | CD81 | CD99 | CDC123 | CDC20 | CDC42EP3 |
| CDCA7L | CDH1 | CDIPT | CDK2AP1 | CDK4 | CDKN1B |
| CDKN2C | CDKN3 | CEACAM6 | CEBPB | CENPW | CEP170 |
| CERS2 | CETN2 | CFL1 | CFL2 | CHCHD1 | CHCHD10 |
| CHCHD2 | CHCHD8 | CHMP2A | CHMP4C | CHMP5 | CHN1 |
| CIB1 | CIRH1A | CISD1 | CKB | CKS1B | CKS2 |
| CLDN3 | CLGN | CLIC1 | CLIC3 | CLIP4 | CMC2 |
| CNIH | CNN3 | CNRIP1 | COL4A2 | COL5A2 | COL6A3 |
| COMMD3 | COMMD8 | COPB2 | COPS5 | CORO1A | COTL1 |
| COX1 | COX2 | COX6B1 | COX6C | COX7A2 | COX7A2L |
| COX7C | COX8A | CPE | CREG1 | CRIM1 | CRIP1 |
| CRIP2 | CRNDE | CRYAB | CRYZ | CS | CSDE1 |
| CSNK2B | CSTA | CTBP2 | CTGF | CTNNAL1 | CTSA |
| CTSD | CTSH | CTSL1 | CTSL2 | CUTA | CWC15 |
| CXXC5 | CYB5R3 | CYC1 | CYFIP1 | CYP1B1 | CYP51A1 |
| CYR61 | CYSTM1 | DAB2 | DAD1 | DAP | DAP3 |
| DARS | DBI | DCTN3 | DCTPP1 | DDC | DDOST |
| DDR1 | DDX1 | DDX21 | DDX39A | DDX47 | DEGS1 |
| DEK | DENND5A | DEPDC7 | DFNA5 | DHCR24 | DHX15 |
| DKK1 | DNAJA1 | DNAJB11 | DNMT1 | DPM1 | DPP4 |
| DPY30 | DPYSL2 | DRG1 | DSG2 | DSP | DUSP23 |
| DUSP4 | DUSP5 | DUSP6 | DUT | DYNC1I2 | DYNLL1 |
| DYNLT1 | DYNLT3 | EBPL | ECHS1 | ECI2 | ECM1 |
| EDF1 | EEF1A1 | EEF1A2 | EEF1B2 | EEF1G | EEF2 |
| EID1 | EIF2A | EIF3D | EIF3E | EIF3G | EIF3H |
| EIF3I | EIF4A1 | EIF4A3 | EIF4H | EIF6 | ELOVL7 |
| EMB | EMP2 | EMP3 | ENC1 | ENO2 | EPCAM |
| EPDR1 | EPHA2 | EPHX1 | EPRS | EPS8 | ERH |

Continued on next page

TABLE S1 – continued from previous page

| Gene Encodings | | | | | |
|---|---|---|---|---|---|
| ERP29 | ERRFI1 | ESRP1 | ETFA | ETFB | ETHE1 |
| EVI2A | F3 | FABP5 | FAM101B | FAM108C1 | FAM114A1 |
| FAM127A | FAM171A1 | FAM176A | FAM210B | FAM216A | FAM83D |
| FAM96A | FAM96B | FAS | FAT1 | FAU | FBL |
| FBN1 | FERMT2 | FGF13 | FGF2 | FGFBP1 | FHL2 |
| FIS1 | FKBP9 | FN1 | FNBP1L | FOS | FOSL1 |
| FOXQ1 | FRMD6 | FTH1 | FTH1P5 | FTL | FUCA2 |
| FXYD3 | FXYD5 | G6PD | GABARAP | GABARAPL2 | GALNT11 |
| GANAB | GAPDH | GARS | GAS2L3 | GBAS | GBE1 |
| GBP3 | GCH1 | GDI2 | GEM | GGCT | GGH |
| GHITM | GHR | GJA1 | GLA | GLIPR1 | GLIS3 |
| GLO1 | GLRX2 | GLRX5 | GLUD1 | GMFG | GMNN |
| GNA15 | GNB1 | GNG11 | GNG12 | GNG5 | GNPAT |
| GOLPH3 | GORASP2 | GOT2 | GPI | GPM6B | GPR137B |
| GPR56 | GPR87 | GPRC5A | GPX1 | GPX2 | GPX3 |
| GPX4 | GPX8 | GRAMD3 | GSTA4 | GSTO1 | GSTO2 |
| GSTP1 | GTF3C6 | GULP1 | GYG1 | GYPC | H1F0 |
| H2AFV | H2AFZ | H3F3B | HADHB | HAT1 | HBXIP |
| HCLS1 | HDAC1 | HDGF | HEATR5A | HEBP1 | HEBP2 |
| HERPUD1 | HEXB | HEY1 | HIAT1 | HIF1A | HIGD2A |
| HINT1 | HIST1H2BK | HIST1H4C | HLA-A | HLA-B | HLA-C |
| HLA-DRA | HLTF | HMGB1 | HMGN1 | HMGN2 | HMGN3 |
| HMGN4 | HMOX1 | HN1 | HNRNPA1 | HNRNPK | HOXB2 |
| HOXC6 | HPCAL1 | HSBP1 | HSD17B10 | HSP90AA1 | HSP90AB1 |
| HSP90B1 | HSPA1A | HSPA5 | HSPA8 | HSPB1 | HSPE1 |
| HSPH1 | HTRA1 | IAH1 | IARS | IARS2 | ID1 |
| ID2 | ID3 | IER2 | IER3 | IFI16 | IFI27 |
| IFI6 | IFITM2 | IFITM3 | IGFBP2 | IGFBP3 | IGFBP4 |
| IGFBP5 | IGFBP6 | IKBIP | IL13RA1 | IL1B | IL32 |
| IL7R | ILF2 | IMP4 | IMPA1 | IMPA2 | IPO7 |
| IQGAP1 | IRF2BPL | IRS2 | IRX3 | ISCU | ITGA3 |
| ITGAE | ITGAV | ITM2B | JTB | KARS | KDELR2 |
| KDELR3 | KHDRBS3 | KIAA0101 | KIAA1191 | KIAA1598 | KIF21B |
| KLF5 | KPNA2 | KRT10 | KRT17 | KRT18 | KRT19 |
| KRT5 | KRT6A | KRT80 | KTN1 | LAMB1 | LAMC1 |
| LAMP2 | LAMTOR1 | LAP3 | LAPTM4A | LAPTM4B | LAPTM5 |
| LASP1 | LBR | LDHA | LDHB | LDOC1 | LEPRE1 |
| LGALS1 | LGALS3 | LGALS3BP | LGMN | LINC00493 | LOC100129361 |
| LOC100288911 | LOC100289026 | LOC100505937 | LOC100506377 | LOC100507246 | LOC344887 |
| LOX | LRP11 | LSM1 | LSM7 | LTA4H | LURAP1L |
| LXN | LYN | LYPLA1 | MAD2L1 | MAGEA12 | MAGEA3 |
| MAGEA6 | MAGED1 | MAGEH1 | MAL2 | MALAT1 | MALL |
| MANF | MANSC1 | MAP1B | MAP1LC3B | MAPK6 | MAPRE1 |
| MARCKS | MATN2 | MEA1 | MET | METTL23 | METTL7B |
| MFSD1 | MGAT4B | MGLL | MGST1 | MGST2 | MIEN1 |
| MIF | MIR22HG | MLF2 | MLH1 | MLLT11 | MLPH |
| MMADHC | MOK | MORC4 | MORF4L1 | MRFAP1 | MRPL13 |
| MRPL14 | MRPL15 | MRPL17 | MRPL18 | MRPL21 | MRPL3 |
| MRPL32 | MRPL33 | MRPL36 | MRPL49 | MRPL51 | MRPS21 |
| MRPS23 | MRPS24 | MRPS30 | MRPS33 | MRPS6 | MSMO1 |
| MSN | MT1E | MT1P2 | MT1X | MT2A | MTCH1 |
| MTHFD1 | MTHFD2 | MTUS1 | MVP | MX1 | MYH10 |
| MYL12B | MYL9 | MYO5C | MYO6 | MYOF | MZT2A |
| NAA20 | NACA | NACAP1 | NAE1 | NAMPT | NAP1L1 |
| NARS | NCEH1 | NCOA4 | ND2 | NDRG1 | NDUFA1 |
| NDUFA12 | NDUFA13 | NDUFA3 | NDUFA4 | NDUFA8 | NDUFA9 |
| NDUFAB1 | NDUFB11 | NDUFB3 | NDUFB5 | NDUFB9 | NDUFS3 |
| NDUFS6 | NDUFV2 | NEDD8 | NEK7 | NETO2 | NEXN |

Continued on next page

TABLE S1 – continued from previous page

| Gene Encodings | | | | | |
|---|---|---|---|---|---|
| NFKBIA | NGFRAP1 | NGRN | NHP2 | NIPA2 | NME1 |
| NNMT | NOL11 | NONO | NOP10 | NOP58 | NPC2 |
| NPDC1 | NPM1 | NPTN | NQO1 | NR3C1 | NSA2 |
| NT5E | NTN4 | NUAK1 | NUDT19 | NUP37 | NUPR1 |
| NUSAP1 | OAT | OAZ1 | OCIAD2 | ODC1 | ODZ2 |
| ORC6 | ORMDL2 | OST4 | OSTC | OXA1L | P2RY8 |
| P4HB | PABPC3 | PABPC4 | PAM | PAPSS1 | PAPSS2 |
| PARK7 | PBK | PBX1 | PCBD1 | PCBP1 | PCMT1 |
| PCNA | PDCD10 | PDHB | PDIA6 | PDLIM1 | PDP1 |
| PDZD11 | PDZK1 | PEA15 | PEBP1 | PEG10 | PFDN2 |
| PFDN5 | PFKP | PFN1 | PFN2 | PGAM1 | PGM1 |
| PGRMC1 | PHB2 | PHLDA1 | PIGP | PIR | PITPNB |
| PKD1P1 | PKIG | PKM2 | PLA2G16 | PLAT | PLAU |
| PLCB4 | PLEKHA1 | PLEKHH1 | PLIN3 | PLK2 | PLOD2 |
| PLOD3 | PLP1 | PLP2 | PLS1 | PLS3 | PMEPA1 |
| PMP22 | POLE3 | POLR2G | POLR2J | POPDC3 | PPA1 |
| PPAP2B | PPAP2C | PPIB | PPIC | PPIL1 | PPP1CA |
| PPP1CB | PPP1CC | PPP1R18 | PPP3CA | PPT1 | PRC1 |
| PRDX1 | PRDX4 | PRDX5 | PRDX6 | PRELID1 | PRICKLE2 |
| PRKCDBP | PRNP | PROCR | PRPS1 | PRR11 | PRR13 |
| PRSS23 | PSAP | PSMA1 | PSMA2 | PSMA4 | PSMA6 |
| PSMA7 | PSMB3 | PSMB4 | PSMB5 | PSMB6 | PSMB8 |
| PSMB9 | PSMC1 | PSMC3 | PSMC4 | PSMC5 | PSMC6 |
| PSMD10 | PSMD14 | PSMD2 | PSMD8 | PSME1 | PSME2 |
| PSMG1 | PSMG2 | PTDSS1 | PTGES3 | PTGFRN | PTGR1 |
| PTMA | PTP4A2 | PTPLAD1 | PTS | PTTG1 | PTTG1IP |
| PXDN | PYGL | QARS | QPCT | RAB10 | RAB13 |
| RAB31 | RAB38 | RAB8A | RABAC1 | RAC1 | RAC2 |
| RACGAP1 | RAD21 | RAI14 | RAN | RAP1B | RARRES3 |
| RARS | RBBP7 | RBM24 | RBX1 | RCN2 | RCSD1 |
| RDBP | REEP5 | RFC4 | RHPN2 | RNASEK | RND3 |
| RNF128 | RNF135 | ROMO1 | RPA3 | RPF2 | RPL11 |
| RPL12 | RPL13A | RPL14 | RPL17 | RPL19 | RPL21 |
| RPL22 | RPL22L1 | RPL23A | RPL24 | RPL26 | RPL26L1 |
| RPL27 | RPL28 | RPL29 | RPL3 | RPL30 | RPL31 |
| RPL32 | RPL34 | RPL35 | RPL36 | RPL36A | RPL36AL |
| RPL38 | RPL39 | RPL4 | RPL41 | RPL5 | RPL6 |
| RPL7A | RPL7L1 | RPL8 | RPL9 | RPLP0 | RPLP1 |
| RPN1 | RPN2 | RPS10 | RPS11 | RPS13 | RPS14P3 |
| RPS16 | RPS17 | RPS18 | RPS2 | RPS20 | RPS21 |
| RPS23 | RPS24 | RPS25 | RPS26 | RPS29 | RPS3 |
| RPS3A | RPS4X | RPS5 | RPS6 | RPS7 | RPSA |
| RRAGD | RRAS | RRAS2 | RRM1 | RRM2 | RSL24D1 |
| RTN4 | S100A10 | S100A11 | S100A16 | S100A2 | S100P |
| SACS | SARNP | SAT1 | SCD | SCG5 | SCP2 |
| SCRN1 | SDC1 | SDC2 | SDC4 | SDCBP | SDHA |
| SEC11A | SEC11C | SEC13 | SEC31A | SEC61G | SELK |
| SELM | SELS | SEMA3C | SEP15 | SEPHS2 | SEPT10 |
| SEPW1 | SERF2 | SERINC5 | SERPINE1 | SET | SF3B1 |
| SF3B5 | SFN | SGCE | SGK1 | SGK223 | SH2B3 |
| SH3BGRL | SH3BGRL3 | SH3KBP1 | SHCBP1 | SHFM1 | SHISA5 |
| SKP1 | SLBP | SLC16A4 | SLC22A18 | SLC25A3 | SLC25A5 |
| SLC25A6 | SLC2A10 | SLC38A2 | SLC3A2 | SLC7A11 | SLC7A5 |
| SLC9A3R1 | SLFN11 | SLIRP | SMAGP | SNAI2 | SNHG5 |
| SNHG6 | SNHG8 | SNRPA | SNRPB | SNRPD2 | SNRPD3 |
| SNRPF | SNRPG | SNX10 | SNX3 | SNX7 | SOD1 |
| SOWAHC | SOX9 | SPARC | SPCS1 | SPINK1 | SPINT2 |
| SPOCK1 | SPP1 | SQRDL | SRGN | SRP14 | SRP19 |

Continued on next page

TABLE S1 – continued from previous page

| Gene Encodings | | | | | |
|---|---|---|---|---|---|
| SRP68 | SRP9 | SRPX | SRSF2 | SRSF9 | SRXN1 |
| SSB | SSR2 | SSR4 | ST13 | ST6GALNAC2 | STARD7 |
| STAU1 | STEAP1 | STUB1 | STXBP1 | SUMO2 | SUMO3 |
| SURF4 | SVIP | SYNC | SYPL1 | SYT13 | SYTL2 |
| TAF7 | TAF9 | TAGLN2 | TALDO1 | TATDN1 | TAX1BP1 |
| TAX1BP3 | TBCA | TBCB | TCEAL3 | TCEAL4 | TCF4 |
| TCP1 | TCTEX1D2 | TDP2 | TEAD1 | TFF3 | TFPI |
| TGFB1I1 | TGFBI | TH1L | TIMMDC1 | TIMP1 | TIMP2 |
| TIMP3 | TJP1 | TK1 | TM4SF1 | TM4SF18 | TM9SF2 |
| TMBIM4 | TMBIM6 | TMED2 | TMEM123 | TMEM126A | TMEM139 |
| TMEM147 | TMEM14A | TMEM14B | TMEM14C | TMEM158 | TMEM167A |
| TMEM200A | TMEM47 | TMEM85 | TMEM93 | TMEM97 | TMSB10 |
| TMX2 | TNFRSF11B | TNFRSF12A | TNFRSF21 | TOB1 | TOMM20 |
| TOMM5 | TOP1 | TOP2B | TPD52L1 | TPM1 | TPT1 |
| TPX2 | TRAM1 | TRIM16 | TRIM59 | TRIP13 | TRMT112 |
| TSG101 | TSHZ1 | TSPAN13 | TSPAN4 | TSPAN6 | TSPAN8 |
| TSPO | TSPYL5 | TSTD1 | TUBA1A | TUBA1B | TUBA1C |
| TUBB | TUBB2A | TUBB3 | TUBB4B | TUBB6 | TUFT1 |
| TUSC1 | TXN | TXNDC12 | TXNIP | TYRP1 | UAP1 |
| UBA2 | UBA52 | UBB | UBC | UBE2C | UBE2E2 |
| UBE2E3 | UBE2S | UBE2V2 | UBL3 | UBL5 | UCHL1 |
| UCHL3 | UCP2 | UFC1 | UFD1L | UGCG | UGDH |
| UPP1 | UQCRC1 | UQCRFS1 | UQCRH | UQCRQ | USMG5 |
| USP1 | UXT | VAMP3 | VAMP7 | VAMP8 | VBP1 |
| VCAN | VDAC2 | VIM | VKORC1 | WBP5 | WDR82 |
| WDR83OS | WIPI1 | WNT5A | WRB | WWC3 | WWTR1 |
| XPOT | YAP1 | YPEL5 | YWHAB | YWHAE | YWHAG |
| YWHAQ | YWHAZ | ZC3H11A | ZCRB1 | ZEB1 | ZMPSTE24 |
| ZNF721 | ZNFX1-AS1 | ZWINT | | | |

# S10 Performance on Ranking New Drugs

**TABLE S2:** BMTMKL Performance on New Drugs ($\theta$ = 2)

| $\alpha_b$ | $\beta_b$ | usim | $\sigma$ | AP@5 | AH@5 | AP@10 | AH@10 | sCI | CI |
|---|---|---|---|---|---|---|---|---|---|
| 1 | 1 | RBF | 10.0 | 0.740 | 1.702 | 0.710 | 2.071 | 0.646 | 0.812 |
| 1e-10 | 1e-10 | RBF | 10.0 | 0.739 | 1.701 | 0.710 | 2.070 | 0.644 | 0.812 |
| 1e-10 | 1e10 | RBF | 10.0 | 0.740 | 1.702 | 0.711 | 2.072 | 0.646 | 0.812 |
| 1 | 1 | COS | - | 0.728 | 1.659 | 0.700 | 2.034 | 0.641 | 0.808 |
| 1e-10 | 1e-10 | COS | - | 0.727 | 1.657 | 0.696 | 2.030 | 0.636 | 0.807 |
| 1e-10 | 1e10 | COS | - | 0.729 | 1.662 | 0.698 | 2.041 | 0.641 | 0.808 |

The columns corresponding to "$\alpha_b$", "$\beta_b$", "usim", and "$\sigma$" have the two hyperparameters, cell line similarity function, and parameter for RBF cell line similarity, respectively, for BMTMKL.

**TABLE S3:** BMTMKL Performance on New Drugs ($\theta$ = 5)

| $\alpha_b$ | $\beta_b$ | usim | $\sigma$ | AP@5 | AH@5 | AP@10 | AH@10 | sCI | CI |
|---|---|---|---|---|---|---|---|---|---|
| 1 | 1 | RBF | 10.0 | 0.827 | 2.735 | 0.772 | 3.760 | 0.653 | 0.812 |
| 1e-10 | 1e-10 | RBF | 10.0 | 0.826 | 2.734 | 0.771 | 3.757 | 0.652 | 0.811 |
| 1e-10 | 1e10 | RBF | 10.0 | 0.828 | 2.736 | 0.772 | 3.761 | 0.652 | 0.812 |
| 1 | 1 | COS | - | 0.815 | 2.650 | 0.757 | 3.690 | 0.648 | 0.808 |
| 1e-10 | 1e-10 | COS | - | 0.817 | 2.647 | 0.759 | 3.670 | 0.646 | 0.807 |
| 1e-10 | 1e10 | COS | - | 0.815 | 2.661 | 0.758 | 3.693 | 0.649 | 0.808 |

The columns corresponding to "$\alpha_b$", "$\beta_b$", "usim", and "$\sigma$" have the two hyperparameters, cell line similarity function, and parameter for RBF cell line similarity, respectively, for BMTMKL.

**TABLE S4:** KRL Performance on New Drugs ($\theta$ = 2)

| $k$ | $\lambda$ | usim | $\sigma$ | AP@5 | AH@5 | AP@10 | AH@10 | sCI | CI |
|---|---|---|---|---|---|---|---|---|---|
| 10 | 0.000001 | LIN | - | 0.609 | 1.489 | 0.588 | 1.994 | 0.656 | 0.739 |
| 10 | 0.000001 | RBF | 0.0001 | 0.735 | 1.730 | 0.708 | 2.101 | 0.662 | 0.736 |
| 10 | 0.000001 | RBF | 0.001 | 0.753 | 1.784 | 0.725 | 2.137 | 0.673 | 0.702 |
| 10 | 0.000001 | RBF | 0.01 | 0.661 | 1.570 | 0.644 | 1.862 | 0.639 | 0.580 |
| 10 | 0.00001 | LIN | - | 0.668 | 1.620 | 0.642 | 2.065 | 0.683 | 0.745 |
| 10 | 0.00001 | RBF | 0.0001 | 0.735 | 1.730 | 0.708 | 2.101 | 0.662 | 0.736 |
| 10 | 0.00001 | RBF | 0.001 | 0.753 | 1.784 | 0.725 | 2.137 | 0.673 | 0.702 |
| 10 | 0.00001 | RBF | 0.01 | 0.635 | 1.477 | 0.620 | 1.728 | 0.631 | 0.574 |
| 10 | 0.0001 | LIN | - | 0.697 | 1.681 | 0.675 | 2.072 | 0.681 | 0.736 |
| 10 | 0.0001 | RBF | 0.0001 | 0.735 | 1.730 | 0.708 | 2.101 | 0.662 | 0.736 |
| 10 | 0.0001 | RBF | 0.001 | 0.753 | 1.784 | 0.725 | 2.137 | 0.673 | 0.702 |
| 10 | 0.0001 | RBF | 0.01 | 0.588 | 1.319 | 0.578 | 1.529 | 0.619 | 0.567 |
| 10 | 0.001 | LIN | - | 0.692 | 1.698 | 0.672 | 2.082 | 0.675 | 0.719 |
| 10 | 0.001 | RBF | 0.0001 | 0.735 | 1.730 | 0.708 | 2.101 | 0.662 | 0.736 |
| 10 | 0.001 | RBF | 0.001 | 0.753 | 1.784 | 0.725 | 2.137 | 0.673 | 0.702 |
| 10 | 0.001 | RBF | 0.01 | 0.513 | 1.113 | 0.509 | 1.284 | 0.607 | 0.557 |
| 10 | 0.01 | LIN | - | 0.701 | 1.718 | 0.680 | 2.089 | 0.672 | 0.697 |
| 10 | 0.01 | RBF | 0.0001 | 0.735 | 1.730 | 0.708 | 2.101 | 0.662 | 0.736 |
| 10 | 0.01 | RBF | 0.001 | 0.753 | 1.784 | 0.725 | 2.137 | 0.673 | 0.702 |
| 10 | 0.01 | RBF | 0.01 | 0.408 | 0.859 | 0.408 | 1.001 | 0.585 | 0.548 |
| 10 | 0.1 | LIN | - | 0.732 | 1.724 | 0.705 | 2.094 | 0.664 | 0.720 |
| 10 | 0.1 | RBF | 0.0001 | 0.735 | 1.730 | 0.708 | 2.101 | 0.662 | 0.736 |
| 10 | 0.1 | RBF | 0.001 | 0.753 | 1.784 | 0.725 | 2.137 | 0.673 | 0.702 |
| 10 | 0.1 | RBF | 0.01 | 0.310 | 0.629 | 0.314 | 0.753 | 0.560 | 0.541 |
| 10 | 0.2 | LIN | - | 0.731 | 1.722 | 0.705 | 2.092 | 0.663 | 0.720 |
| 10 | 0.2 | RBF | 0.0001 | 0.735 | 1.730 | 0.708 | 2.101 | 0.662 | 0.736 |
| 10 | 0.2 | RBF | 0.001 | 0.753 | 1.784 | 0.725 | 2.137 | 0.673 | 0.702 |
| 10 | 0.2 | RBF | 0.01 | 0.278 | 0.559 | 0.282 | 0.685 | 0.552 | 0.539 |
| 10 | 0.4 | LIN | - | 0.731 | 1.722 | 0.705 | 2.092 | 0.663 | 0.720 |
| 10 | 0.4 | RBF | 0.0001 | 0.735 | 1.730 | 0.708 | 2.101 | 0.662 | 0.736 |
| 10 | 0.4 | RBF | 0.001 | 0.753 | 1.784 | 0.725 | 2.137 | 0.673 | 0.702 |
| 10 | 0.4 | RBF | 0.01 | 0.244 | 0.493 | 0.250 | 0.617 | 0.542 | 0.537 |
| 10 | 0.6 | LIN | - | 0.731 | 1.722 | 0.705 | 2.092 | 0.663 | 0.720 |
| 10 | 0.6 | RBF | 0.0001 | 0.735 | 1.730 | 0.708 | 2.101 | 0.662 | 0.736 |
| 10 | 0.6 | RBF | 0.001 | 0.753 | 1.784 | 0.725 | 2.137 | 0.673 | 0.702 |
| 10 | 0.6 | RBF | 0.01 | 0.224 | 0.463 | 0.231 | 0.586 | 0.542 | 0.536 |
| 10 | 0.8 | LIN | - | 0.731 | 1.722 | 0.705 | 2.092 | 0.663 | 0.720 |
| 10 | 0.8 | RBF | 0.0001 | 0.735 | 1.730 | 0.708 | 2.101 | 0.662 | 0.736 |
| 10 | 0.8 | RBF | 0.001 | 0.753 | 1.784 | 0.725 | 2.137 | 0.673 | 0.702 |
| 10 | 0.8 | RBF | 0.01 | 0.214 | 0.441 | 0.221 | 0.567 | 0.540 | 0.536 |
| 10 | 1.0 | LIN | - | 0.731 | 1.722 | 0.705 | 2.092 | 0.663 | 0.720 |
| 10 | 1.0 | RBF | 0.0001 | 0.735 | 1.730 | 0.708 | 2.101 | 0.662 | 0.736 |
| 10 | 1.0 | RBF | 0.001 | 0.753 | 1.784 | 0.725 | 2.137 | 0.673 | 0.702 |
| 10 | 1.0 | RBF | 0.01 | 0.205 | 0.425 | 0.213 | 0.549 | 0.537 | 0.536 |
| 10 | 10 | LIN | - | 0.732 | 1.722 | 0.705 | 2.096 | 0.662 | 0.734 |
| 10 | 10 | RBF | 0.0001 | 0.735 | 1.730 | 0.708 | 2.101 | 0.662 | 0.736 |
| 10 | 10 | RBF | 0.001 | 0.753 | 1.784 | 0.725 | 2.137 | 0.673 | 0.702 |
| 10 | 10 | RBF | 0.01 | 0.146 | 0.318 | 0.156 | 0.452 | 0.521 | 0.533 |
| 10 | 50 | LIN | - | 0.733 | 1.723 | 0.705 | 2.095 | 0.662 | 0.737 |
| 10 | 50 | RBF | 0.0001 | 0.735 | 1.730 | 0.708 | 2.101 | 0.662 | 0.736 |
| 10 | 50 | RBF | 0.001 | 0.753 | 1.784 | 0.725 | 2.137 | 0.673 | 0.702 |
| 10 | 50 | RBF | 0.01 | 0.127 | 0.286 | 0.138 | 0.420 | 0.516 | 0.532 |
| 10 | 100 | LIN | - | 0.733 | 1.723 | 0.705 | 2.095 | 0.662 | 0.737 |
| 10 | 100 | RBF | 0.0001 | 0.735 | 1.730 | 0.708 | 2.101 | 0.662 | 0.736 |
| 10 | 100 | RBF | 0.001 | 0.753 | 1.783 | 0.725 | 2.137 | 0.673 | 0.702 |
| 10 | 100 | RBF | 0.01 | 0.121 | 0.277 | 0.132 | 0.411 | 0.514 | 0.532 |

The columns corresponding to "$k$", "$\lambda$", "usim", and "$\sigma$" have the two hyperparameters, cell line similarity function, and parameter for RBF cell line similarity, respectively, for KRL.

**TABLE S5:** KRL Performance on New Drugs ($\theta$ = 5)

| $k$ | $\lambda$ | usim | $\sigma$ | AP@5 | AH@5 | AP@10 | AH@10 | sCI | CI |
|---|---|---|---|---|---|---|---|---|---|
| 10 | 0.000001 | LIN | - | 0.665 | 2.088 | 0.615 | 3.214 | 0.657 | 0.722 |
| 10 | 0.000001 | RBF | 0.0001 | 0.805 | 2.627 | 0.746 | 3.733 | 0.675 | 0.760 |
| 10 | 0.000001 | RBF | 0.001 | 0.817 | 2.715 | 0.761 | 3.798 | 0.676 | 0.762 |
| 10 | 0.000001 | RBF | 0.01 | 0.735 | 2.321 | 0.684 | 3.256 | 0.635 | 0.637 |
| 10 | 0.00001 | LIN | - | 0.769 | 2.440 | 0.708 | 3.528 | 0.683 | 0.739 |
| 10 | 0.00001 | RBF | 0.0001 | 0.796 | 2.547 | 0.736 | 3.560 | 0.660 | 0.768 |
| 10 | 0.00001 | RBF | 0.001 | 0.817 | 2.715 | 0.761 | 3.798 | 0.676 | 0.762 |
| 10 | 0.00001 | RBF | 0.01 | 0.713 | 2.224 | 0.666 | 3.078 | 0.625 | 0.624 |
| 10 | 0.0001 | LIN | - | 0.789 | 2.580 | 0.730 | 3.690 | 0.689 | 0.756 |
| 10 | 0.0001 | RBF | 0.0001 | 0.796 | 2.547 | 0.736 | 3.560 | 0.660 | 0.768 |
| 10 | 0.0001 | RBF | 0.001 | 0.817 | 2.715 | 0.761 | 3.798 | 0.676 | 0.762 |
| 10 | 0.0001 | RBF | 0.01 | 0.674 | 2.046 | 0.633 | 2.804 | 0.608 | 0.606 |
| 10 | 0.001 | LIN | - | 0.785 | 2.521 | 0.722 | 3.618 | 0.676 | 0.714 |
| 10 | 0.001 | RBF | 0.0001 | 0.796 | 2.547 | 0.736 | 3.560 | 0.660 | 0.768 |
| 10 | 0.001 | RBF | 0.001 | 0.817 | 2.715 | 0.761 | 3.798 | 0.676 | 0.762 |
| 10 | 0.001 | RBF | 0.01 | 0.608 | 1.781 | 0.577 | 2.382 | 0.589 | 0.585 |
| 10 | 0.01 | LIN | - | 0.792 | 2.570 | 0.731 | 3.668 | 0.679 | 0.716 |
| 10 | 0.01 | RBF | 0.0001 | 0.796 | 2.547 | 0.736 | 3.560 | 0.660 | 0.768 |
| 10 | 0.01 | RBF | 0.001 | 0.817 | 2.715 | 0.761 | 3.798 | 0.676 | 0.762 |
| 10 | 0.01 | RBF | 0.01 | 0.512 | 1.436 | 0.494 | 1.905 | 0.566 | 0.565 |
| 10 | 0.1 | LIN | - | 0.799 | 2.556 | 0.736 | 3.663 | 0.676 | 0.662 |
| 10 | 0.1 | RBF | 0.0001 | 0.796 | 2.547 | 0.736 | 3.560 | 0.660 | 0.768 |
| 10 | 0.1 | RBF | 0.001 | 0.817 | 2.715 | 0.761 | 3.798 | 0.676 | 0.762 |
| 10 | 0.1 | RBF | 0.01 | 0.418 | 1.093 | 0.410 | 1.444 | 0.538 | 0.549 |
| 10 | 0.2 | LIN | - | 0.800 | 2.593 | 0.739 | 3.701 | 0.673 | 0.738 |
| 10 | 0.2 | RBF | 0.0001 | 0.796 | 2.547 | 0.736 | 3.560 | 0.660 | 0.768 |
| 10 | 0.2 | RBF | 0.001 | 0.817 | 2.715 | 0.761 | 3.798 | 0.676 | 0.762 |
| 10 | 0.2 | RBF | 0.01 | 0.386 | 0.987 | 0.380 | 1.317 | 0.531 | 0.545 |
| 10 | 0.4 | LIN | - | 0.797 | 2.556 | 0.735 | 3.619 | 0.663 | 0.743 |
| 10 | 0.4 | RBF | 0.0001 | 0.796 | 2.547 | 0.736 | 3.560 | 0.660 | 0.768 |
| 10 | 0.4 | RBF | 0.001 | 0.817 | 2.715 | 0.761 | 3.798 | 0.676 | 0.762 |
| 10 | 0.4 | RBF | 0.01 | 0.351 | 0.888 | 0.349 | 1.180 | 0.524 | 0.541 |
| 10 | 0.6 | LIN | - | 0.794 | 2.535 | 0.735 | 3.529 | 0.658 | 0.738 |
| 10 | 0.6 | RBF | 0.0001 | 0.796 | 2.547 | 0.736 | 3.560 | 0.660 | 0.768 |
| 10 | 0.6 | RBF | 0.001 | 0.817 | 2.715 | 0.761 | 3.798 | 0.676 | 0.762 |
| 10 | 0.6 | RBF | 0.01 | 0.332 | 0.834 | 0.332 | 1.120 | 0.520 | 0.539 |
| 10 | 0.8 | LIN | - | 0.794 | 2.535 | 0.735 | 3.529 | 0.658 | 0.738 |
| 10 | 0.8 | RBF | 0.0001 | 0.796 | 2.547 | 0.736 | 3.560 | 0.660 | 0.768 |
| 10 | 0.8 | RBF | 0.001 | 0.817 | 2.715 | 0.761 | 3.798 | 0.676 | 0.762 |
| 10 | 0.8 | RBF | 0.01 | 0.320 | 0.802 | 0.321 | 1.078 | 0.518 | 0.538 |
| 10 | 1.0 | LIN | - | 0.794 | 2.535 | 0.735 | 3.529 | 0.658 | 0.738 |
| 10 | 1.0 | RBF | 0.0001 | 0.796 | 2.547 | 0.736 | 3.560 | 0.660 | 0.768 |
| 10 | 1.0 | RBF | 0.001 | 0.817 | 2.715 | 0.761 | 3.798 | 0.676 | 0.762 |
| 10 | 1.0 | RBF | 0.01 | 0.310 | 0.773 | 0.311 | 1.052 | 0.517 | 0.537 |
| 10 | 10 | LIN | - | 0.794 | 2.535 | 0.735 | 3.529 | 0.658 | 0.738 |
| 10 | 10 | RBF | 0.0001 | 0.796 | 2.547 | 0.736 | 3.560 | 0.660 | 0.768 |
| 10 | 10 | RBF | 0.001 | 0.817 | 2.715 | 0.761 | 3.798 | 0.676 | 0.762 |
| 10 | 10 | RBF | 0.01 | 0.246 | 0.595 | 0.250 | 0.853 | 0.503 | 0.532 |
| 10 | 50 | LIN | - | 0.794 | 2.535 | 0.735 | 3.529 | 0.658 | 0.738 |
| 10 | 50 | RBF | 0.0001 | 0.796 | 2.547 | 0.736 | 3.560 | 0.660 | 0.768 |
| 10 | 50 | RBF | 0.001 | 0.817 | 2.715 | 0.761 | 3.798 | 0.676 | 0.762 |
| 10 | 50 | RBF | 0.01 | 0.223 | 0.538 | 0.231 | 0.788 | 0.497 | 0.530 |
| 10 | 100 | LIN | - | 0.794 | 2.535 | 0.735 | 3.529 | 0.658 | 0.738 |
| 10 | 100 | RBF | 0.0001 | 0.796 | 2.547 | 0.736 | 3.560 | 0.660 | 0.768 |
| 10 | 100 | RBF | 0.001 | 0.817 | 2.715 | 0.761 | 3.798 | 0.676 | 0.762 |
| 10 | 100 | RBF | 0.01 | 0.216 | 0.522 | 0.224 | 0.773 | 0.497 | 0.529 |

The columns corresponding to "$k$", "$\lambda$", "usim", and "$\sigma$" have the two hyperparameters, cell line similarity function, and parameter for RBF cell line similarity, respectively, for KRL.

**TABLE S6:** pLETORg Performance on New Drugs ($\theta$ = 2)

| $l$ | $\alpha$ | $\beta$ | $\gamma$ | usim | $\sigma$ | AP@5 | AH@5 | AP@10 | AH@10 | sCI | CI |
|---|---|---|---|---|---|---|---|---|---|---|---|
| 5 | 0.00 | 0.1 | 0.0 | COS | - | 0.771 | 1.802 | 0.744 | 2.131 | 0.653 | 0.769 |
| 5 | 0.00 | 0.1 | 0.0 | RBF | 10.0 | 0.771 | 1.802 | 0.744 | 2.131 | 0.653 | 0.769 |
| 5 | 0.00 | 0.1 | 1.0 | COS | - | 0.771 | 1.802 | 0.744 | 2.131 | 0.653 | 0.769 |
| 5 | 0.00 | 0.1 | 1.0 | RBF | 10.0 | 0.771 | 1.802 | 0.744 | 2.131 | 0.653 | 0.769 |
| 5 | 0.00 | 0.1 | 10.0 | COS | - | 0.771 | 1.802 | 0.744 | 2.132 | 0.653 | 0.769 |
| 5 | 0.00 | 0.1 | 10.0 | RBF | 10.0 | 0.771 | 1.802 | 0.744 | 2.132 | 0.653 | 0.769 |
| 5 | 0.00 | 0.1 | 100.0 | COS | - | 0.771 | 1.805 | 0.745 | 2.133 | 0.652 | 0.771 |
| 5 | 0.00 | 0.1 | 100.0 | RBF | 10.0 | 0.771 | 1.805 | 0.745 | 2.133 | 0.652 | 0.772 |
| 5 | 0.00 | 1.0 | 0.0 | COS | - | 0.771 | 1.805 | 0.744 | 2.132 | 0.652 | 0.772 |
| 5 | 0.00 | 1.0 | 0.0 | RBF | 10.0 | 0.771 | 1.805 | 0.744 | 2.132 | 0.652 | 0.772 |
| 5 | 0.00 | 1.0 | 1.0 | COS | - | 0.771 | 1.805 | 0.744 | 2.132 | 0.652 | 0.772 |
| 5 | 0.00 | 1.0 | 1.0 | RBF | 10.0 | 0.771 | 1.805 | 0.744 | 2.132 | 0.652 | 0.772 |
| 5 | 0.00 | 1.0 | 10.0 | COS | - | 0.771 | 1.805 | 0.744 | 2.133 | 0.652 | 0.772 |
| 5 | 0.00 | 1.0 | 10.0 | RBF | 10.0 | 0.771 | 1.805 | 0.744 | 2.133 | 0.652 | 0.772 |
| 5 | 0.00 | 1.0 | 100.0 | COS | - | 0.771 | 1.805 | 0.745 | 2.133 | 0.652 | 0.771 |
| 5 | 0.00 | 1.0 | 100.0 | RBF | 10.0 | 0.771 | 1.805 | 0.745 | 2.133 | 0.652 | 0.772 |
| 5 | 0.05 | 0.1 | 0.0 | COS | - | 0.772 | 1.808 | 0.745 | 2.133 | 0.653 | 0.774 |
| 5 | 0.05 | 0.1 | 0.0 | RBF | 10.0 | 0.772 | 1.808 | 0.745 | 2.133 | 0.653 | 0.774 |
| 5 | 0.05 | 0.1 | 1.0 | COS | - | 0.772 | 1.808 | 0.745 | 2.133 | 0.653 | 0.774 |
| 5 | 0.05 | 0.1 | 1.0 | RBF | 10.0 | 0.772 | 1.808 | 0.745 | 2.133 | 0.653 | 0.774 |
| 5 | 0.05 | 0.1 | 10.0 | COS | - | 0.772 | 1.808 | 0.745 | 2.133 | 0.653 | 0.774 |
| 5 | 0.05 | 0.1 | 10.0 | RBF | 10.0 | 0.772 | 1.808 | 0.745 | 2.133 | 0.653 | 0.774 |
| 5 | 0.05 | 0.1 | 100.0 | COS | - | 0.772 | 1.806 | 0.745 | 2.133 | 0.653 | 0.774 |
| 5 | 0.05 | 0.1 | 100.0 | RBF | 10.0 | 0.772 | 1.806 | 0.745 | 2.133 | 0.653 | 0.774 |
| 5 | 0.05 | 1.0 | 0.0 | COS | - | 0.772 | 1.808 | 0.745 | 2.133 | 0.653 | 0.774 |
| 5 | 0.05 | 1.0 | 0.0 | RBF | 10.0 | 0.772 | 1.808 | 0.745 | 2.133 | 0.653 | 0.774 |
| 5 | 0.05 | 1.0 | 1.0 | COS | - | 0.772 | 1.808 | 0.745 | 2.133 | 0.653 | 0.774 |
| 5 | 0.05 | 1.0 | 1.0 | RBF | 10.0 | 0.772 | 1.808 | 0.745 | 2.133 | 0.653 | 0.774 |
| 5 | 0.05 | 1.0 | 10.0 | COS | - | 0.772 | 1.808 | 0.745 | 2.133 | 0.653 | 0.774 |
| 5 | 0.05 | 1.0 | 10.0 | RBF | 10.0 | 0.772 | 1.808 | 0.745 | 2.133 | 0.653 | 0.774 |
| 5 | 0.05 | 1.0 | 100.0 | COS | - | 0.772 | 1.806 | 0.745 | 2.133 | 0.653 | 0.774 |
| 5 | 0.05 | 1.0 | 100.0 | RBF | 10.0 | 0.772 | 1.806 | 0.745 | 2.133 | 0.653 | 0.774 |
| 5 | 0.10 | 0.1 | 0.0 | COS | - | 0.773 | 1.810 | 0.745 | 2.135 | 0.653 | 0.776 |
| 5 | 0.10 | 0.1 | 0.0 | RBF | 10.0 | 0.773 | 1.810 | 0.745 | 2.135 | 0.653 | 0.776 |
| 5 | 0.10 | 0.1 | 1.0 | COS | - | 0.773 | 1.810 | 0.745 | 2.135 | 0.653 | 0.776 |
| 5 | 0.10 | 0.1 | 1.0 | RBF | 10.0 | 0.773 | 1.810 | 0.745 | 2.135 | 0.653 | 0.776 |
| 5 | 0.10 | 0.1 | 10.0 | COS | - | 0.772 | 1.809 | 0.745 | 2.135 | 0.653 | 0.776 |
| 5 | 0.10 | 0.1 | 10.0 | RBF | 10.0 | 0.772 | 1.809 | 0.745 | 2.135 | 0.653 | 0.776 |
| 5 | 0.10 | 0.1 | 100.0 | COS | - | 0.772 | 1.808 | 0.745 | 2.135 | 0.653 | 0.776 |
| 5 | 0.10 | 0.1 | 100.0 | RBF | 10.0 | 0.772 | 1.808 | 0.745 | 2.135 | 0.653 | 0.776 |
| 5 | 0.10 | 1.0 | 0.0 | COS | - | 0.773 | 1.810 | 0.745 | 2.135 | 0.653 | 0.776 |
| 5 | 0.10 | 1.0 | 0.0 | RBF | 10.0 | 0.773 | 1.810 | 0.745 | 2.135 | 0.653 | 0.776 |
| 5 | 0.10 | 1.0 | 1.0 | COS | - | 0.773 | 1.810 | 0.745 | 2.135 | 0.653 | 0.776 |
| 5 | 0.10 | 1.0 | 1.0 | RBF | 10.0 | 0.773 | 1.810 | 0.745 | 2.135 | 0.653 | 0.776 |
| 5 | 0.10 | 1.0 | 10.0 | COS | - | 0.772 | 1.809 | 0.745 | 2.135 | 0.653 | 0.776 |
| 5 | 0.10 | 1.0 | 10.0 | RBF | 10.0 | 0.772 | 1.809 | 0.745 | 2.135 | 0.653 | 0.776 |
| 5 | 0.10 | 1.0 | 100.0 | COS | - | 0.772 | 1.808 | 0.745 | 2.135 | 0.653 | 0.776 |
| 5 | 0.10 | 1.0 | 100.0 | RBF | 10.0 | 0.772 | 1.808 | 0.745 | 2.135 | 0.653 | 0.776 |
| 5 | 0.50 | 0.1 | 0.0 | COS | - | 0.773 | 1.814 | 0.745 | 2.141 | 0.652 | 0.792 |
| 5 | 0.50 | 0.1 | 0.0 | RBF | 10.0 | 0.773 | 1.814 | 0.745 | 2.141 | 0.652 | 0.792 |
| 5 | 0.50 | 0.1 | 1.0 | COS | - | 0.773 | 1.814 | 0.745 | 2.141 | 0.652 | 0.792 |
| 5 | 0.50 | 0.1 | 1.0 | RBF | 10.0 | 0.773 | 1.814 | 0.745 | 2.141 | 0.652 | 0.792 |
| 5 | 0.50 | 0.1 | 10.0 | COS | - | 0.773 | 1.815 | 0.745 | 2.141 | 0.652 | 0.792 |
| 5 | 0.50 | 0.1 | 10.0 | RBF | 10.0 | 0.773 | 1.815 | 0.745 | 2.141 | 0.652 | 0.792 |
| 5 | 0.50 | 0.1 | 100.0 | COS | - | 0.773 | 1.816 | 0.745 | 2.142 | 0.651 | 0.792 |
| 5 | 0.50 | 0.1 | 100.0 | RBF | 10.0 | 0.773 | 1.815 | 0.745 | 2.141 | 0.651 | 0.792 |
| 5 | 0.50 | 1.0 | 0.0 | COS | - | 0.773 | 1.814 | 0.745 | 2.141 | 0.652 | 0.792 |

Continued on next page

TABLE S6 – continued from previous page

| $l$ | $\alpha$ | $\beta$ | $\gamma$ | usim | $\sigma$ | AP@5 | AH@5 | AP@10 | AH@10 | sCI | CI |
|---|---|---|---|---|---|---|---|---|---|---|---|
| 5 | 0.50 | 1.0 | 0.0 | RBF | 10.0 | 0.773 | 1.814 | 0.745 | 2.141 | 0.652 | 0.792 |
| 5 | 0.50 | 1.0 | 1.0 | COS | - | 0.773 | 1.814 | 0.745 | 2.141 | 0.652 | 0.792 |
| 5 | 0.50 | 1.0 | 1.0 | RBF | 10.0 | 0.773 | 1.814 | 0.745 | 2.141 | 0.652 | 0.792 |
| 5 | 0.50 | 1.0 | 10.0 | COS | - | 0.773 | 1.815 | 0.745 | 2.141 | 0.652 | 0.792 |
| 5 | 0.50 | 1.0 | 10.0 | RBF | 10.0 | 0.773 | 1.815 | 0.745 | 2.141 | 0.652 | 0.792 |
| 5 | 0.50 | 1.0 | 100.0 | COS | - | 0.773 | 1.816 | 0.745 | 2.142 | 0.651 | 0.792 |
| 5 | 0.50 | 1.0 | 100.0 | RBF | 10.0 | 0.773 | 1.815 | 0.745 | 2.141 | 0.651 | 0.792 |
| 5 | 1.00 | 0.1 | 0.0 | COS | - | 0.531 | 1.129 | 0.514 | 1.392 | 0.587 | 0.639 |
| 5 | 1.00 | 0.1 | 0.0 | RBF | 10.0 | 0.531 | 1.129 | 0.514 | 1.392 | 0.587 | 0.639 |
| 5 | 1.00 | 0.1 | 1.0 | COS | - | 0.536 | 1.132 | 0.519 | 1.398 | 0.588 | 0.641 |
| 5 | 1.00 | 0.1 | 1.0 | RBF | 10.0 | 0.532 | 1.127 | 0.514 | 1.392 | 0.589 | 0.639 |
| 5 | 1.00 | 0.1 | 10.0 | COS | - | 0.546 | 1.155 | 0.528 | 1.415 | 0.591 | 0.648 |
| 5 | 1.00 | 0.1 | 10.0 | RBF | 10.0 | 0.544 | 1.154 | 0.527 | 1.414 | 0.591 | 0.648 |
| 5 | 1.00 | 0.1 | 100.0 | COS | - | 0.570 | 1.216 | 0.553 | 1.487 | 0.607 | 0.672 |
| 5 | 1.00 | 0.1 | 100.0 | RBF | 10.0 | 0.572 | 1.219 | 0.555 | 1.491 | 0.603 | 0.676 |
| 5 | 1.00 | 1.0 | 0.0 | COS | - | 0.538 | 1.137 | 0.521 | 1.397 | 0.587 | 0.640 |
| 5 | 1.00 | 1.0 | 0.0 | RBF | 10.0 | 0.538 | 1.137 | 0.521 | 1.397 | 0.587 | 0.640 |
| 5 | 1.00 | 1.0 | 1.0 | COS | - | 0.540 | 1.139 | 0.523 | 1.400 | 0.588 | 0.641 |
| 5 | 1.00 | 1.0 | 1.0 | RBF | 10.0 | 0.537 | 1.137 | 0.520 | 1.393 | 0.588 | 0.640 |
| 5 | 1.00 | 1.0 | 10.0 | COS | - | 0.548 | 1.165 | 0.530 | 1.421 | 0.591 | 0.650 |
| 5 | 1.00 | 1.0 | 10.0 | RBF | 10.0 | 0.545 | 1.160 | 0.527 | 1.414 | 0.591 | 0.647 |
| 5 | 1.00 | 1.0 | 100.0 | COS | - | 0.572 | 1.214 | 0.554 | 1.486 | 0.603 | 0.671 |
| 5 | 1.00 | 1.0 | 100.0 | RBF | 10.0 | 0.572 | 1.219 | 0.556 | 1.489 | 0.603 | 0.676 |
| 10 | 0.00 | 0.1 | 0.0 | COS | - | 0.780 | 1.851 | 0.755 | 2.157 | 0.631 | 0.786 |
| 10 | 0.00 | 0.1 | 0.0 | RBF | 10.0 | 0.780 | 1.851 | 0.755 | 2.157 | 0.631 | 0.786 |
| 10 | 0.00 | 0.1 | 1.0 | COS | - | 0.780 | 1.851 | 0.755 | 2.157 | 0.631 | 0.786 |
| 10 | 0.00 | 0.1 | 1.0 | RBF | 10.0 | 0.780 | 1.851 | 0.755 | 2.157 | 0.631 | 0.786 |
| 10 | 0.00 | 0.1 | 10.0 | COS | - | 0.780 | 1.851 | 0.755 | 2.157 | 0.632 | 0.786 |
| 10 | 0.00 | 0.1 | 10.0 | RBF | 10.0 | 0.780 | 1.850 | 0.755 | 2.157 | 0.632 | 0.786 |
| 10 | 0.00 | 0.1 | 100.0 | COS | - | 0.783 | 1.856 | 0.758 | 2.159 | 0.638 | 0.774 |
| 10 | 0.00 | 0.1 | 100.0 | RBF | 10.0 | 0.782 | 1.858 | 0.757 | 2.159 | 0.638 | 0.777 |
| 10 | 0.00 | 1.0 | 0.0 | COS | - | 0.779 | 1.849 | 0.754 | 2.157 | 0.631 | 0.790 |
| 10 | 0.00 | 1.0 | 0.0 | RBF | 10.0 | 0.779 | 1.849 | 0.754 | 2.157 | 0.631 | 0.790 |
| 10 | 0.00 | 1.0 | 1.0 | COS | - | 0.779 | 1.849 | 0.754 | 2.157 | 0.631 | 0.790 |
| 10 | 0.00 | 1.0 | 1.0 | RBF | 10.0 | 0.779 | 1.849 | 0.754 | 2.157 | 0.631 | 0.790 |
| 10 | 0.00 | 1.0 | 10.0 | COS | - | 0.779 | 1.849 | 0.754 | 2.157 | 0.631 | 0.790 |
| 10 | 0.00 | 1.0 | 10.0 | RBF | 10.0 | 0.779 | 1.849 | 0.754 | 2.157 | 0.631 | 0.790 |
| 10 | 0.00 | 1.0 | 100.0 | COS | - | 0.779 | 1.852 | 0.754 | 2.156 | 0.631 | 0.790 |
| 10 | 0.00 | 1.0 | 100.0 | RBF | 10.0 | 0.779 | 1.851 | 0.754 | 2.157 | 0.632 | 0.790 |
| 10 | 0.05 | 0.1 | 0.0 | COS | - | 0.778 | 1.850 | 0.754 | 2.156 | 0.630 | 0.792 |
| 10 | 0.05 | 0.1 | 0.0 | RBF | 10.0 | 0.778 | 1.850 | 0.754 | 2.156 | 0.630 | 0.792 |
| 10 | 0.05 | 0.1 | 1.0 | COS | - | 0.778 | 1.850 | 0.754 | 2.156 | 0.630 | 0.792 |
| 10 | 0.05 | 0.1 | 1.0 | RBF | 10.0 | 0.778 | 1.850 | 0.754 | 2.156 | 0.630 | 0.792 |
| 10 | 0.05 | 0.1 | 10.0 | COS | - | 0.778 | 1.849 | 0.754 | 2.156 | 0.630 | 0.792 |
| 10 | 0.05 | 0.1 | 10.0 | RBF | 10.0 | 0.778 | 1.849 | 0.754 | 2.156 | 0.630 | 0.792 |
| 10 | 0.05 | 0.1 | 100.0 | COS | - | 0.778 | 1.849 | 0.753 | 2.156 | 0.632 | 0.792 |
| 10 | 0.05 | 0.1 | 100.0 | RBF | 10.0 | 0.778 | 1.850 | 0.753 | 2.156 | 0.632 | 0.792 |
| 10 | 0.05 | 1.0 | 0.0 | COS | - | 0.778 | 1.850 | 0.754 | 2.156 | 0.630 | 0.792 |
| 10 | 0.05 | 1.0 | 0.0 | RBF | 10.0 | 0.778 | 1.850 | 0.754 | 2.156 | 0.630 | 0.792 |
| 10 | 0.05 | 1.0 | 1.0 | COS | - | 0.778 | 1.850 | 0.754 | 2.156 | 0.630 | 0.792 |
| 10 | 0.05 | 1.0 | 1.0 | RBF | 10.0 | 0.778 | 1.850 | 0.754 | 2.156 | 0.630 | 0.792 |
| 10 | 0.05 | 1.0 | 10.0 | COS | - | 0.778 | 1.849 | 0.754 | 2.156 | 0.630 | 0.792 |
| 10 | 0.05 | 1.0 | 10.0 | RBF | 10.0 | 0.778 | 1.849 | 0.754 | 2.156 | 0.630 | 0.792 |
| 10 | 0.05 | 1.0 | 100.0 | COS | - | 0.778 | 1.849 | 0.753 | 2.156 | 0.632 | 0.792 |
| 10 | 0.05 | 1.0 | 100.0 | RBF | 10.0 | 0.778 | 1.850 | 0.753 | 2.156 | 0.632 | 0.792 |
| 10 | 0.10 | 0.1 | 0.0 | COS | - | 0.777 | 1.845 | 0.753 | 2.155 | 0.629 | 0.794 |
| 10 | 0.10 | 0.1 | 0.0 | RBF | 10.0 | 0.777 | 1.845 | 0.753 | 2.155 | 0.629 | 0.794 |
| 10 | 0.10 | 0.1 | 1.0 | COS | - | 0.777 | 1.845 | 0.753 | 2.155 | 0.629 | 0.794 |

Continued on next page

TABLE S6 – continued from previous page

| $l$ | $\alpha$ | $\beta$ | $\gamma$ | usim | $\sigma$ | AP@5 | AH@5 | AP@10 | AH@10 | sCI | CI |
|---|---|---|---|---|---|---|---|---|---|---|---|
| 10 | 0.10 | 0.1 | 1.0 | RBF | 10.0 | 0.777 | 1.845 | 0.753 | 2.155 | 0.629 | 0.794 |
| 10 | 0.10 | 0.1 | 10.0 | COS | - | 0.777 | 1.845 | 0.753 | 2.155 | 0.629 | 0.794 |
| 10 | 0.10 | 0.1 | 10.0 | RBF | 10.0 | 0.777 | 1.845 | 0.753 | 2.155 | 0.629 | 0.794 |
| 10 | 0.10 | 0.1 | 100.0 | COS | - | 0.777 | 1.849 | 0.753 | 2.155 | 0.629 | 0.794 |
| 10 | 0.10 | 0.1 | 100.0 | RBF | 10.0 | 0.777 | 1.848 | 0.753 | 2.155 | 0.629 | 0.794 |
| 10 | 0.10 | 1.0 | 0.0 | COS | - | 0.777 | 1.845 | 0.753 | 2.155 | 0.629 | 0.794 |
| 10 | 0.10 | 1.0 | 0.0 | RBF | 10.0 | 0.777 | 1.845 | 0.753 | 2.155 | 0.629 | 0.794 |
| 10 | 0.10 | 1.0 | 1.0 | COS | - | 0.777 | 1.845 | 0.753 | 2.155 | 0.629 | 0.794 |
| 10 | 0.10 | 1.0 | 1.0 | RBF | 10.0 | 0.777 | 1.845 | 0.753 | 2.155 | 0.629 | 0.794 |
| 10 | 0.10 | 1.0 | 10.0 | COS | - | 0.777 | 1.845 | 0.753 | 2.155 | 0.629 | 0.794 |
| 10 | 0.10 | 1.0 | 10.0 | RBF | 10.0 | 0.777 | 1.845 | 0.753 | 2.155 | 0.629 | 0.794 |
| 10 | 0.10 | 1.0 | 100.0 | COS | - | 0.777 | 1.849 | 0.753 | 2.156 | 0.629 | 0.794 |
| 10 | 0.10 | 1.0 | 100.0 | RBF | 10.0 | 0.777 | 1.848 | 0.753 | 2.155 | 0.629 | 0.794 |
| 10 | 0.50 | 0.1 | 0.0 | COS | - | 0.757 | 1.787 | 0.735 | 2.091 | 0.648 | 0.703 |
| 10 | 0.50 | 0.1 | 0.0 | RBF | 10.0 | 0.757 | 1.787 | 0.735 | 2.091 | 0.648 | 0.703 |
| 10 | 0.50 | 0.1 | 1.0 | COS | - | 0.757 | 1.786 | 0.735 | 2.091 | 0.648 | 0.703 |
| 10 | 0.50 | 0.1 | 1.0 | RBF | 10.0 | 0.757 | 1.786 | 0.735 | 2.091 | 0.648 | 0.703 |
| 10 | 0.50 | 0.1 | 10.0 | COS | - | 0.757 | 1.786 | 0.736 | 2.091 | 0.648 | 0.703 |
| 10 | 0.50 | 0.1 | 10.0 | RBF | 10.0 | 0.757 | 1.786 | 0.735 | 2.091 | 0.648 | 0.703 |
| 10 | 0.50 | 0.1 | 100.0 | COS | - | 0.758 | 1.785 | 0.737 | 2.088 | 0.656 | 0.703 |
| 10 | 0.50 | 0.1 | 100.0 | RBF | 10.0 | 0.758 | 1.786 | 0.737 | 2.090 | 0.656 | 0.703 |
| 10 | 0.50 | 1.0 | 0.0 | COS | - | 0.772 | 1.832 | 0.747 | 2.138 | 0.654 | 0.735 |
| 10 | 0.50 | 1.0 | 0.0 | RBF | 10.0 | 0.772 | 1.832 | 0.747 | 2.138 | 0.654 | 0.735 |
| 10 | 0.50 | 1.0 | 1.0 | COS | - | 0.772 | 1.832 | 0.747 | 2.139 | 0.654 | 0.736 |
| 10 | 0.50 | 1.0 | 1.0 | RBF | 10.0 | 0.772 | 1.832 | 0.747 | 2.139 | 0.654 | 0.736 |
| 10 | 0.50 | 1.0 | 10.0 | COS | - | 0.773 | 1.835 | 0.747 | 2.140 | 0.654 | 0.737 |
| 10 | 0.50 | 1.0 | 10.0 | RBF | 10.0 | 0.772 | 1.834 | 0.747 | 2.140 | 0.654 | 0.737 |
| 10 | 0.50 | 1.0 | 100.0 | COS | - | 0.774 | 1.834 | 0.749 | 2.140 | 0.657 | 0.736 |
| 10 | 0.50 | 1.0 | 100.0 | RBF | 10.0 | 0.773 | 1.834 | 0.749 | 2.140 | 0.655 | 0.737 |
| 10 | 1.00 | 0.1 | 0.0 | COS | - | 0.578 | 1.207 | 0.559 | 1.478 | 0.592 | 0.644 |
| 10 | 1.00 | 0.1 | 0.0 | RBF | 10.0 | 0.578 | 1.207 | 0.559 | 1.478 | 0.592 | 0.644 |
| 10 | 1.00 | 0.1 | 1.0 | COS | - | 0.580 | 1.215 | 0.562 | 1.484 | 0.594 | 0.646 |
| 10 | 1.00 | 0.1 | 1.0 | RBF | 10.0 | 0.580 | 1.214 | 0.562 | 1.482 | 0.594 | 0.645 |
| 10 | 1.00 | 0.1 | 10.0 | COS | - | 0.589 | 1.260 | 0.569 | 1.534 | 0.605 | 0.656 |
| 10 | 1.00 | 0.1 | 10.0 | RBF | 10.0 | 0.588 | 1.253 | 0.568 | 1.529 | 0.605 | 0.655 |
| 10 | 1.00 | 0.1 | 100.0 | COS | - | 0.612 | 1.341 | 0.593 | 1.647 | 0.618 | 0.696 |
| 10 | 1.00 | 0.1 | 100.0 | RBF | 10.0 | 0.608 | 1.335 | 0.591 | 1.636 | 0.620 | 0.695 |
| 10 | 1.00 | 1.0 | 0.0 | COS | - | 0.577 | 1.206 | 0.559 | 1.471 | 0.592 | 0.640 |
| 10 | 1.00 | 1.0 | 0.0 | RBF | 10.0 | 0.577 | 1.206 | 0.559 | 1.471 | 0.592 | 0.640 |
| 10 | 1.00 | 1.0 | 1.0 | COS | - | 0.581 | 1.215 | 0.562 | 1.483 | 0.594 | 0.645 |
| 10 | 1.00 | 1.0 | 1.0 | RBF | 10.0 | 0.581 | 1.214 | 0.562 | 1.482 | 0.594 | 0.645 |
| 10 | 1.00 | 1.0 | 10.0 | COS | - | 0.586 | 1.246 | 0.567 | 1.522 | 0.605 | 0.651 |
| 10 | 1.00 | 1.0 | 10.0 | RBF | 10.0 | 0.585 | 1.246 | 0.566 | 1.519 | 0.604 | 0.650 |
| 10 | 1.00 | 1.0 | 100.0 | COS | - | 0.611 | 1.334 | 0.592 | 1.645 | 0.620 | 0.695 |
| 10 | 1.00 | 1.0 | 100.0 | RBF | 10.0 | 0.609 | 1.335 | 0.592 | 1.631 | 0.622 | 0.692 |
| 15 | 0.00 | 0.1 | 0.0 | COS | - | 0.763 | 1.837 | 0.736 | 2.162 | 0.613 | 0.786 |
| 15 | 0.00 | 0.1 | 0.0 | RBF | 10.0 | 0.763 | 1.837 | 0.736 | 2.162 | 0.613 | 0.786 |
| 15 | 0.00 | 0.1 | 1.0 | COS | - | 0.763 | 1.837 | 0.736 | 2.162 | 0.613 | 0.786 |
| 15 | 0.00 | 0.1 | 1.0 | RBF | 10.0 | 0.763 | 1.837 | 0.736 | 2.162 | 0.613 | 0.786 |
| 15 | 0.00 | 0.1 | 10.0 | COS | - | 0.759 | 1.831 | 0.733 | 2.161 | 0.610 | 0.788 |
| 15 | 0.00 | 0.1 | 10.0 | RBF | 10.0 | 0.759 | 1.831 | 0.733 | 2.160 | 0.610 | 0.788 |
| 15 | 0.00 | 0.1 | 100.0 | COS | - | 0.779 | 1.858 | 0.753 | 2.169 | 0.643 | 0.768 |
| 15 | 0.00 | 0.1 | 100.0 | RBF | 10.0 | 0.777 | 1.858 | 0.751 | 2.171 | 0.632 | 0.774 |
| 15 | 0.00 | 1.0 | 0.0 | COS | - | 0.747 | 1.798 | 0.719 | 2.148 | 0.590 | 0.796 |
| 15 | 0.00 | 1.0 | 0.0 | RBF | 10.0 | 0.747 | 1.798 | 0.719 | 2.148 | 0.590 | 0.796 |
| 15 | 0.00 | 1.0 | 1.0 | COS | - | 0.747 | 1.798 | 0.719 | 2.148 | 0.590 | 0.796 |
| 15 | 0.00 | 1.0 | 1.0 | RBF | 10.0 | 0.747 | 1.798 | 0.719 | 2.148 | 0.590 | 0.796 |
| 15 | 0.00 | 1.0 | 10.0 | COS | - | 0.746 | 1.795 | 0.717 | 2.147 | 0.588 | 0.796 |

Continued on next page

TABLE S6 – continued from previous page

| $l$ | $\alpha$ | $\beta$ | $\gamma$ | usim | $\sigma$ | AP@5 | AH@5 | AP@10 | AH@10 | sCI | CI |
|---|---|---|---|---|---|---|---|---|---|---|---|
| 15 | 0.00 | 1.0 | 10.0 | RBF | 10.0 | 0.746 | 1.794 | 0.717 | 2.147 | 0.588 | 0.796 |
| 15 | 0.00 | 1.0 | 100.0 | COS | - | 0.754 | 1.817 | 0.726 | 2.158 | 0.598 | 0.793 |
| 15 | 0.00 | 1.0 | 100.0 | RBF | 10.0 | 0.749 | 1.800 | 0.720 | 2.152 | 0.592 | 0.796 |
| 15 | 0.05 | 0.1 | 0.0 | COS | - | 0.738 | 1.779 | 0.710 | 2.138 | 0.585 | 0.798 |
| 15 | 0.05 | 0.1 | 0.0 | RBF | 10.0 | 0.738 | 1.779 | 0.710 | 2.138 | 0.585 | 0.798 |
| 15 | 0.05 | 0.1 | 1.0 | COS | - | 0.739 | 1.779 | 0.710 | 2.138 | 0.585 | 0.798 |
| 15 | 0.05 | 0.1 | 1.0 | RBF | 10.0 | 0.739 | 1.779 | 0.710 | 2.138 | 0.585 | 0.798 |
| 15 | 0.05 | 0.1 | 10.0 | COS | - | 0.739 | 1.780 | 0.710 | 2.138 | 0.585 | 0.798 |
| 15 | 0.05 | 0.1 | 10.0 | RBF | 10.0 | 0.739 | 1.780 | 0.710 | 2.138 | 0.585 | 0.798 |
| 15 | 0.05 | 0.1 | 100.0 | COS | - | 0.742 | 1.788 | 0.713 | 2.143 | 0.588 | 0.798 |
| 15 | 0.05 | 0.1 | 100.0 | RBF | 10.0 | 0.740 | 1.784 | 0.711 | 2.140 | 0.586 | 0.798 |
| 15 | 0.05 | 1.0 | 0.0 | COS | - | 0.738 | 1.779 | 0.710 | 2.138 | 0.585 | 0.798 |
| 15 | 0.05 | 1.0 | 0.0 | RBF | 10.0 | 0.738 | 1.779 | 0.710 | 2.138 | 0.585 | 0.798 |
| 15 | 0.05 | 1.0 | 1.0 | COS | - | 0.739 | 1.779 | 0.710 | 2.138 | 0.585 | 0.798 |
| 15 | 0.05 | 1.0 | 1.0 | RBF | 10.0 | 0.739 | 1.779 | 0.710 | 2.138 | 0.585 | 0.798 |
| 15 | 0.05 | 1.0 | 10.0 | COS | - | 0.739 | 1.780 | 0.710 | 2.138 | 0.585 | 0.798 |
| 15 | 0.05 | 1.0 | 10.0 | RBF | 10.0 | 0.739 | 1.780 | 0.710 | 2.138 | 0.585 | 0.798 |
| 15 | 0.05 | 1.0 | 100.0 | COS | - | 0.740 | 1.784 | 0.712 | 2.141 | 0.587 | 0.798 |
| 15 | 0.05 | 1.0 | 100.0 | RBF | 10.0 | 0.740 | 1.784 | 0.711 | 2.140 | 0.586 | 0.798 |
| 15 | 0.10 | 0.1 | 0.0 | COS | - | 0.732 | 1.764 | 0.704 | 2.128 | 0.580 | 0.800 |
| 15 | 0.10 | 0.1 | 0.0 | RBF | 10.0 | 0.732 | 1.764 | 0.704 | 2.128 | 0.580 | 0.800 |
| 15 | 0.10 | 0.1 | 1.0 | COS | - | 0.732 | 1.764 | 0.704 | 2.129 | 0.580 | 0.800 |
| 15 | 0.10 | 0.1 | 1.0 | RBF | 10.0 | 0.732 | 1.764 | 0.704 | 2.129 | 0.580 | 0.800 |
| 15 | 0.10 | 0.1 | 10.0 | COS | - | 0.733 | 1.764 | 0.704 | 2.129 | 0.580 | 0.800 |
| 15 | 0.10 | 0.1 | 10.0 | RBF | 10.0 | 0.733 | 1.764 | 0.704 | 2.129 | 0.580 | 0.800 |
| 15 | 0.10 | 0.1 | 100.0 | COS | - | 0.735 | 1.773 | 0.706 | 2.132 | 0.582 | 0.800 |
| 15 | 0.10 | 0.1 | 100.0 | RBF | 10.0 | 0.734 | 1.770 | 0.705 | 2.131 | 0.581 | 0.800 |
| 15 | 0.10 | 1.0 | 0.0 | COS | - | 0.732 | 1.764 | 0.704 | 2.129 | 0.580 | 0.800 |
| 15 | 0.10 | 1.0 | 0.0 | RBF | 10.0 | 0.732 | 1.764 | 0.704 | 2.129 | 0.580 | 0.800 |
| 15 | 0.10 | 1.0 | 1.0 | COS | - | 0.732 | 1.764 | 0.704 | 2.129 | 0.580 | 0.800 |
| 15 | 0.10 | 1.0 | 1.0 | RBF | 10.0 | 0.732 | 1.764 | 0.704 | 2.129 | 0.580 | 0.800 |
| 15 | 0.10 | 1.0 | 10.0 | COS | - | 0.733 | 1.764 | 0.704 | 2.129 | 0.580 | 0.800 |
| 15 | 0.10 | 1.0 | 10.0 | RBF | 10.0 | 0.733 | 1.764 | 0.705 | 2.129 | 0.580 | 0.800 |
| 15 | 0.10 | 1.0 | 100.0 | COS | - | 0.735 | 1.773 | 0.707 | 2.132 | 0.582 | 0.800 |
| 15 | 0.10 | 1.0 | 100.0 | RBF | 10.0 | 0.734 | 1.771 | 0.705 | 2.131 | 0.582 | 0.800 |
| 15 | 0.50 | 0.1 | 0.0 | COS | - | 0.742 | 1.766 | 0.717 | 2.079 | 0.615 | 0.713 |
| 15 | 0.50 | 0.1 | 0.0 | RBF | 10.0 | 0.742 | 1.766 | 0.717 | 2.079 | 0.615 | 0.713 |
| 15 | 0.50 | 0.1 | 1.0 | COS | - | 0.742 | 1.766 | 0.718 | 2.079 | 0.615 | 0.713 |
| 15 | 0.50 | 0.1 | 1.0 | RBF | 10.0 | 0.742 | 1.766 | 0.718 | 2.079 | 0.615 | 0.713 |
| 15 | 0.50 | 0.1 | 10.0 | COS | - | 0.743 | 1.770 | 0.719 | 2.081 | 0.619 | 0.713 |
| 15 | 0.50 | 0.1 | 10.0 | RBF | 10.0 | 0.743 | 1.770 | 0.719 | 2.082 | 0.619 | 0.713 |
| 15 | 0.50 | 0.1 | 100.0 | COS | - | 0.751 | 1.786 | 0.727 | 2.094 | 0.632 | 0.712 |
| 15 | 0.50 | 0.1 | 100.0 | RBF | 10.0 | 0.750 | 1.786 | 0.726 | 2.093 | 0.628 | 0.712 |
| 15 | 0.50 | 1.0 | 0.0 | COS | - | 0.742 | 1.784 | 0.717 | 2.112 | 0.610 | 0.732 |
| 15 | 0.50 | 1.0 | 0.0 | RBF | 10.0 | 0.742 | 1.784 | 0.717 | 2.112 | 0.610 | 0.732 |
| 15 | 0.50 | 1.0 | 1.0 | COS | - | 0.742 | 1.786 | 0.717 | 2.112 | 0.611 | 0.733 |
| 15 | 0.50 | 1.0 | 1.0 | RBF | 10.0 | 0.742 | 1.786 | 0.717 | 2.112 | 0.611 | 0.733 |
| 15 | 0.50 | 1.0 | 10.0 | COS | - | 0.742 | 1.790 | 0.718 | 2.118 | 0.611 | 0.736 |
| 15 | 0.50 | 1.0 | 10.0 | RBF | 10.0 | 0.742 | 1.790 | 0.718 | 2.117 | 0.611 | 0.735 |
| 15 | 0.50 | 1.0 | 100.0 | COS | - | 0.750 | 1.809 | 0.726 | 2.129 | 0.622 | 0.735 |
| 15 | 0.50 | 1.0 | 100.0 | RBF | 10.0 | 0.749 | 1.807 | 0.725 | 2.128 | 0.620 | 0.736 |
| 15 | 1.00 | 0.1 | 0.0 | COS | - | 0.587 | 1.251 | 0.569 | 1.520 | 0.600 | 0.676 |
| 15 | 1.00 | 0.1 | 0.0 | RBF | 10.0 | 0.587 | 1.251 | 0.569 | 1.520 | 0.600 | 0.676 |
| 15 | 1.00 | 0.1 | 1.0 | COS | - | 0.589 | 1.261 | 0.571 | 1.538 | 0.602 | 0.679 |
| 15 | 1.00 | 0.1 | 1.0 | RBF | 10.0 | 0.589 | 1.260 | 0.571 | 1.536 | 0.602 | 0.679 |
| 15 | 1.00 | 0.1 | 10.0 | COS | - | 0.612 | 1.333 | 0.594 | 1.633 | 0.624 | 0.696 |
| 15 | 1.00 | 0.1 | 10.0 | RBF | 10.0 | 0.610 | 1.323 | 0.591 | 1.623 | 0.624 | 0.695 |
| 15 | 1.00 | 0.1 | 100.0 | COS | - | 0.631 | 1.417 | 0.611 | 1.774 | 0.639 | 0.736 |

Continued on next page

TABLE S6 – continued from previous page

| $l$ | $\alpha$ | $\beta$ | $\gamma$ | usim | $\sigma$ | AP@5 | AH@5 | AP@10 | AH@10 | sCI | CI |
|---|---|---|---|---|---|---|---|---|---|---|---|
| 15 | 1.00 | 0.1 | 100.0 | RBF | 10.0 | 0.629 | 1.418 | 0.610 | 1.760 | 0.639 | 0.730 |
| 15 | 1.00 | 1.0 | 0.0 | COS | - | 0.586 | 1.252 | 0.568 | 1.518 | 0.601 | 0.673 |
| 15 | 1.00 | 1.0 | 0.0 | RBF | 10.0 | 0.586 | 1.252 | 0.568 | 1.518 | 0.601 | 0.673 |
| 15 | 1.00 | 1.0 | 1.0 | COS | - | 0.590 | 1.261 | 0.571 | 1.537 | 0.602 | 0.679 |
| 15 | 1.00 | 1.0 | 1.0 | RBF | 10.0 | 0.590 | 1.260 | 0.571 | 1.534 | 0.602 | 0.678 |
| 15 | 1.00 | 1.0 | 10.0 | COS | - | 0.609 | 1.322 | 0.591 | 1.616 | 0.624 | 0.688 |
| 15 | 1.00 | 1.0 | 10.0 | RBF | 10.0 | 0.606 | 1.311 | 0.589 | 1.607 | 0.622 | 0.686 |
| 15 | 1.00 | 1.0 | 100.0 | COS | - | 0.630 | 1.419 | 0.609 | 1.765 | 0.641 | 0.731 |
| 15 | 1.00 | 1.0 | 100.0 | RBF | 10.0 | 0.633 | 1.413 | 0.612 | 1.757 | 0.639 | 0.733 |
| 30 | 0.00 | 0.1 | 0.0 | COS | - | 0.665 | 1.631 | 0.639 | 2.051 | 0.591 | 0.783 |
| 30 | 0.00 | 0.1 | 0.0 | RBF | 10.0 | 0.665 | 1.631 | 0.639 | 2.051 | 0.591 | 0.783 |
| 30 | 0.00 | 0.1 | 1.0 | COS | - | 0.663 | 1.625 | 0.637 | 2.049 | 0.590 | 0.784 |
| 30 | 0.00 | 0.1 | 1.0 | RBF | 10.0 | 0.663 | 1.625 | 0.637 | 2.049 | 0.590 | 0.784 |
| 30 | 0.00 | 0.1 | 10.0 | COS | - | 0.640 | 1.580 | 0.615 | 2.027 | 0.577 | 0.788 |
| 30 | 0.00 | 0.1 | 10.0 | RBF | 10.0 | 0.641 | 1.582 | 0.616 | 2.029 | 0.578 | 0.788 |
| 30 | 0.00 | 0.1 | 100.0 | COS | - | 0.763 | 1.767 | 0.733 | 2.100 | 0.657 | 0.725 |
| 30 | 0.00 | 0.1 | 100.0 | RBF | 10.0 | 0.755 | 1.784 | 0.727 | 2.127 | 0.649 | 0.744 |
| 30 | 0.00 | 1.0 | 0.0 | COS | - | 0.552 | 1.359 | 0.528 | 1.873 | 0.523 | 0.802 |
| 30 | 0.00 | 1.0 | 0.0 | RBF | 10.0 | 0.552 | 1.359 | 0.528 | 1.873 | 0.523 | 0.802 |
| 30 | 0.00 | 1.0 | 1.0 | COS | - | 0.548 | 1.345 | 0.524 | 1.863 | 0.520 | 0.803 |
| 30 | 0.00 | 1.0 | 1.0 | RBF | 10.0 | 0.548 | 1.345 | 0.524 | 1.863 | 0.520 | 0.803 |
| 30 | 0.00 | 1.0 | 10.0 | COS | - | 0.546 | 1.342 | 0.523 | 1.861 | 0.519 | 0.803 |
| 30 | 0.00 | 1.0 | 10.0 | RBF | 10.0 | 0.546 | 1.342 | 0.522 | 1.861 | 0.519 | 0.803 |
| 30 | 0.00 | 1.0 | 100.0 | COS | - | 0.706 | 1.708 | 0.677 | 2.101 | 0.609 | 0.775 |
| 30 | 0.00 | 1.0 | 100.0 | RBF | 10.0 | 0.651 | 1.605 | 0.626 | 2.046 | 0.585 | 0.788 |
| 30 | 0.05 | 0.1 | 0.0 | COS | - | 0.531 | 1.299 | 0.509 | 1.820 | 0.509 | 0.804 |
| 30 | 0.05 | 0.1 | 0.0 | RBF | 10.0 | 0.531 | 1.299 | 0.509 | 1.820 | 0.509 | 0.804 |
| 30 | 0.05 | 0.1 | 1.0 | COS | - | 0.531 | 1.299 | 0.509 | 1.821 | 0.509 | 0.804 |
| 30 | 0.05 | 0.1 | 1.0 | RBF | 10.0 | 0.531 | 1.299 | 0.509 | 1.821 | 0.509 | 0.804 |
| 30 | 0.05 | 0.1 | 10.0 | COS | - | 0.531 | 1.300 | 0.509 | 1.823 | 0.509 | 0.804 |
| 30 | 0.05 | 0.1 | 10.0 | RBF | 10.0 | 0.531 | 1.300 | 0.509 | 1.823 | 0.509 | 0.804 |
| 30 | 0.05 | 0.1 | 100.0 | COS | - | 0.691 | 1.690 | 0.664 | 2.089 | 0.606 | 0.777 |
| 30 | 0.05 | 0.1 | 100.0 | RBF | 10.0 | 0.628 | 1.558 | 0.603 | 2.015 | 0.569 | 0.791 |
| 30 | 0.05 | 1.0 | 0.0 | COS | - | 0.531 | 1.299 | 0.509 | 1.820 | 0.509 | 0.804 |
| 30 | 0.05 | 1.0 | 0.0 | RBF | 10.0 | 0.531 | 1.299 | 0.509 | 1.820 | 0.509 | 0.804 |
| 30 | 0.05 | 1.0 | 1.0 | COS | - | 0.531 | 1.299 | 0.509 | 1.821 | 0.509 | 0.804 |
| 30 | 0.05 | 1.0 | 1.0 | RBF | 10.0 | 0.531 | 1.299 | 0.509 | 1.821 | 0.509 | 0.804 |
| 30 | 0.05 | 1.0 | 10.0 | COS | - | 0.531 | 1.300 | 0.509 | 1.823 | 0.509 | 0.804 |
| 30 | 0.05 | 1.0 | 10.0 | RBF | 10.0 | 0.531 | 1.300 | 0.509 | 1.823 | 0.509 | 0.804 |
| 30 | 0.05 | 1.0 | 100.0 | COS | - | 0.600 | 1.504 | 0.577 | 1.980 | 0.551 | 0.795 |
| 30 | 0.05 | 1.0 | 100.0 | RBF | 10.0 | 0.546 | 1.343 | 0.523 | 1.858 | 0.517 | 0.803 |
| 30 | 0.10 | 0.1 | 0.0 | COS | - | 0.522 | 1.273 | 0.501 | 1.789 | 0.501 | 0.804 |
| 30 | 0.10 | 0.1 | 0.0 | RBF | 10.0 | 0.522 | 1.273 | 0.501 | 1.789 | 0.501 | 0.804 |
| 30 | 0.10 | 0.1 | 1.0 | COS | - | 0.522 | 1.273 | 0.501 | 1.789 | 0.501 | 0.804 |
| 30 | 0.10 | 0.1 | 1.0 | RBF | 10.0 | 0.522 | 1.273 | 0.501 | 1.789 | 0.501 | 0.804 |
| 30 | 0.10 | 0.1 | 10.0 | COS | - | 0.521 | 1.269 | 0.501 | 1.784 | 0.501 | 0.804 |
| 30 | 0.10 | 0.1 | 10.0 | RBF | 10.0 | 0.521 | 1.268 | 0.501 | 1.783 | 0.501 | 0.804 |
| 30 | 0.10 | 0.1 | 100.0 | COS | - | 0.642 | 1.591 | 0.616 | 2.037 | 0.578 | 0.786 |
| 30 | 0.10 | 0.1 | 100.0 | RBF | 10.0 | 0.560 | 1.378 | 0.537 | 1.891 | 0.527 | 0.800 |
| 30 | 0.10 | 1.0 | 0.0 | COS | - | 0.521 | 1.268 | 0.500 | 1.782 | 0.500 | 0.804 |
| 30 | 0.10 | 1.0 | 0.0 | RBF | 10.0 | 0.521 | 1.268 | 0.500 | 1.782 | 0.500 | 0.804 |
| 30 | 0.10 | 1.0 | 1.0 | COS | - | 0.521 | 1.268 | 0.500 | 1.782 | 0.500 | 0.804 |
| 30 | 0.10 | 1.0 | 1.0 | RBF | 10.0 | 0.521 | 1.268 | 0.500 | 1.782 | 0.500 | 0.804 |
| 30 | 0.10 | 1.0 | 10.0 | COS | - | 0.521 | 1.269 | 0.501 | 1.784 | 0.501 | 0.804 |
| 30 | 0.10 | 1.0 | 10.0 | RBF | 10.0 | 0.521 | 1.268 | 0.501 | 1.783 | 0.501 | 0.804 |
| 30 | 0.10 | 1.0 | 100.0 | COS | - | 0.561 | 1.380 | 0.538 | 1.895 | 0.527 | 0.800 |
| 30 | 0.10 | 1.0 | 100.0 | RBF | 10.0 | 0.527 | 1.290 | 0.505 | 1.809 | 0.505 | 0.805 |
| 30 | 0.50 | 0.1 | 0.0 | COS | - | 0.648 | 1.567 | 0.622 | 1.970 | 0.586 | 0.726 |

Continued on next page

TABLE S6 – continued from previous page

| $l$ | $\alpha$ | $\beta$ | $\gamma$ | usim | $\sigma$ | AP@5 | AH@5 | AP@10 | AH@10 | sCI | CI |
|---|---|---|---|---|---|---|---|---|---|---|---|
| 30 | 0.50 | 0.1 | 0.0 | RBF | 10.0 | 0.648 | 1.567 | 0.622 | 1.970 | 0.586 | 0.726 |
| 30 | 0.50 | 0.1 | 1.0 | COS | - | 0.648 | 1.568 | 0.622 | 1.970 | 0.586 | 0.726 |
| 30 | 0.50 | 0.1 | 1.0 | RBF | 10.0 | 0.648 | 1.568 | 0.622 | 1.970 | 0.586 | 0.726 |
| 30 | 0.50 | 0.1 | 10.0 | COS | - | 0.652 | 1.582 | 0.626 | 1.980 | 0.589 | 0.726 |
| 30 | 0.50 | 0.1 | 10.0 | RBF | 10.0 | 0.651 | 1.578 | 0.625 | 1.979 | 0.589 | 0.726 |
| 30 | 0.50 | 0.1 | 100.0 | COS | - | 0.685 | 1.666 | 0.660 | 2.042 | 0.611 | 0.726 |
| 30 | 0.50 | 0.1 | 100.0 | RBF | 10.0 | 0.681 | 1.660 | 0.655 | 2.036 | 0.609 | 0.726 |
| 30 | 0.50 | 1.0 | 0.0 | COS | - | 0.628 | 1.529 | 0.604 | 1.956 | 0.573 | 0.739 |
| 30 | 0.50 | 1.0 | 0.0 | RBF | 10.0 | 0.628 | 1.529 | 0.604 | 1.956 | 0.573 | 0.739 |
| 30 | 0.50 | 1.0 | 1.0 | COS | - | 0.627 | 1.529 | 0.603 | 1.958 | 0.572 | 0.739 |
| 30 | 0.50 | 1.0 | 1.0 | RBF | 10.0 | 0.627 | 1.529 | 0.603 | 1.958 | 0.572 | 0.739 |
| 30 | 0.50 | 1.0 | 10.0 | COS | - | 0.624 | 1.524 | 0.599 | 1.961 | 0.569 | 0.743 |
| 30 | 0.50 | 1.0 | 10.0 | RBF | 10.0 | 0.623 | 1.523 | 0.598 | 1.959 | 0.568 | 0.743 |
| 30 | 0.50 | 1.0 | 100.0 | COS | - | 0.659 | 1.618 | 0.633 | 2.033 | 0.599 | 0.740 |
| 30 | 0.50 | 1.0 | 100.0 | RBF | 10.0 | 0.647 | 1.589 | 0.622 | 2.020 | 0.589 | 0.744 |
| 30 | 1.00 | 0.1 | 0.0 | COS | - | 0.525 | 1.139 | 0.511 | 1.451 | 0.594 | 0.706 |
| 30 | 1.00 | 0.1 | 0.0 | RBF | 10.0 | 0.525 | 1.139 | 0.511 | 1.451 | 0.594 | 0.706 |
| 30 | 1.00 | 0.1 | 1.0 | COS | - | 0.538 | 1.173 | 0.522 | 1.484 | 0.598 | 0.712 |
| 30 | 1.00 | 0.1 | 1.0 | RBF | 10.0 | 0.537 | 1.170 | 0.521 | 1.482 | 0.598 | 0.711 |
| 30 | 1.00 | 0.1 | 10.0 | COS | - | 0.629 | 1.403 | 0.607 | 1.735 | 0.641 | 0.736 |
| 30 | 1.00 | 0.1 | 10.0 | RBF | 10.0 | 0.621 | 1.384 | 0.599 | 1.706 | 0.639 | 0.734 |
| 30 | 1.00 | 0.1 | 100.0 | COS | - | 0.672 | 1.561 | 0.647 | 1.903 | 0.664 | 0.760 |
| 30 | 1.00 | 0.1 | 100.0 | RBF | 10.0 | 0.676 | 1.560 | 0.651 | 1.897 | 0.668 | 0.759 |
| 30 | 1.00 | 1.0 | 0.0 | COS | - | 0.528 | 1.142 | 0.513 | 1.448 | 0.595 | 0.704 |
| 30 | 1.00 | 1.0 | 0.0 | RBF | 10.0 | 0.528 | 1.142 | 0.513 | 1.448 | 0.595 | 0.704 |
| 30 | 1.00 | 1.0 | 1.0 | COS | - | 0.537 | 1.168 | 0.522 | 1.478 | 0.599 | 0.711 |
| 30 | 1.00 | 1.0 | 1.0 | RBF | 10.0 | 0.536 | 1.163 | 0.520 | 1.474 | 0.599 | 0.711 |
| 30 | 1.00 | 1.0 | 10.0 | COS | - | 0.627 | 1.396 | 0.605 | 1.722 | 0.640 | 0.726 |
| 30 | 1.00 | 1.0 | 10.0 | RBF | 10.0 | 0.620 | 1.373 | 0.598 | 1.687 | 0.639 | 0.724 |
| 30 | 1.00 | 1.0 | 100.0 | COS | - | 0.675 | 1.562 | 0.651 | 1.893 | 0.666 | 0.758 |
| 30 | 1.00 | 1.0 | 100.0 | RBF | 10.0 | 0.676 | 1.562 | 0.652 | 1.890 | 0.665 | 0.758 |
| 50 | 0.00 | 0.1 | 0.0 | COS | - | 0.666 | 1.566 | 0.634 | 1.990 | 0.628 | 0.770 |
| 50 | 0.00 | 0.1 | 0.0 | RBF | 10.0 | 0.666 | 1.566 | 0.634 | 1.990 | 0.628 | 0.770 |
| 50 | 0.00 | 0.1 | 1.0 | COS | - | 0.643 | 1.511 | 0.611 | 1.962 | 0.621 | 0.775 |
| 50 | 0.00 | 0.1 | 1.0 | RBF | 10.0 | 0.643 | 1.511 | 0.611 | 1.962 | 0.621 | 0.775 |
| 50 | 0.00 | 0.1 | 10.0 | COS | - | 0.589 | 1.424 | 0.561 | 1.893 | 0.601 | 0.783 |
| 50 | 0.00 | 0.1 | 10.0 | RBF | 10.0 | 0.599 | 1.437 | 0.570 | 1.904 | 0.602 | 0.782 |
| 50 | 0.00 | 0.1 | 100.0 | COS | - | 0.746 | 1.634 | 0.713 | 1.973 | 0.658 | 0.698 |
| 50 | 0.00 | 0.1 | 100.0 | RBF | 10.0 | 0.749 | 1.686 | 0.717 | 2.036 | 0.660 | 0.714 |
| 50 | 0.00 | 1.0 | 0.0 | COS | - | 0.473 | 1.161 | 0.460 | 1.687 | 0.557 | 0.794 |
| 50 | 0.00 | 1.0 | 0.0 | RBF | 10.0 | 0.473 | 1.161 | 0.460 | 1.687 | 0.557 | 0.794 |
| 50 | 0.00 | 1.0 | 1.0 | COS | - | 0.473 | 1.162 | 0.460 | 1.688 | 0.557 | 0.794 |
| 50 | 0.00 | 1.0 | 1.0 | RBF | 10.0 | 0.473 | 1.162 | 0.460 | 1.688 | 0.557 | 0.794 |
| 50 | 0.00 | 1.0 | 10.0 | COS | - | 0.435 | 1.052 | 0.426 | 1.596 | 0.535 | 0.797 |
| 50 | 0.00 | 1.0 | 10.0 | RBF | 10.0 | 0.438 | 1.057 | 0.428 | 1.604 | 0.535 | 0.796 |
| 50 | 0.00 | 1.0 | 100.0 | COS | - | 0.740 | 1.717 | 0.709 | 2.088 | 0.654 | 0.745 |
| 50 | 0.00 | 1.0 | 100.0 | RBF | 10.0 | 0.710 | 1.651 | 0.676 | 2.053 | 0.644 | 0.763 |
| 50 | 0.05 | 0.1 | 0.0 | COS | - | 0.433 | 1.052 | 0.426 | 1.595 | 0.539 | 0.796 |
| 50 | 0.05 | 0.1 | 0.0 | RBF | 10.0 | 0.433 | 1.052 | 0.426 | 1.595 | 0.539 | 0.796 |
| 50 | 0.05 | 0.1 | 1.0 | COS | - | 0.434 | 1.053 | 0.426 | 1.596 | 0.539 | 0.796 |
| 50 | 0.05 | 0.1 | 1.0 | RBF | 10.0 | 0.434 | 1.053 | 0.426 | 1.595 | 0.539 | 0.796 |
| 50 | 0.05 | 0.1 | 10.0 | COS | - | 0.415 | 0.993 | 0.409 | 1.524 | 0.524 | 0.797 |
| 50 | 0.05 | 0.1 | 10.0 | RBF | 10.0 | 0.417 | 1.001 | 0.410 | 1.534 | 0.525 | 0.797 |
| 50 | 0.05 | 0.1 | 100.0 | COS | - | 0.753 | 1.713 | 0.722 | 2.061 | 0.666 | 0.715 |
| 50 | 0.05 | 0.1 | 100.0 | RBF | 10.0 | 0.729 | 1.711 | 0.698 | 2.088 | 0.658 | 0.747 |
| 50 | 0.05 | 1.0 | 0.0 | COS | - | 0.406 | 0.965 | 0.400 | 1.491 | 0.522 | 0.798 |
| 50 | 0.05 | 1.0 | 0.0 | RBF | 10.0 | 0.406 | 0.965 | 0.400 | 1.491 | 0.522 | 0.798 |
| 50 | 0.05 | 1.0 | 1.0 | COS | - | 0.406 | 0.965 | 0.400 | 1.491 | 0.522 | 0.798 |

Continued on next page

TABLE S6 – continued from previous page

| $l$ | $\alpha$ | $\beta$ | $\gamma$ | usim | $\sigma$ | AP@5 | AH@5 | AP@10 | AH@10 | sCI | CI |
|---|---|---|---|---|---|---|---|---|---|---|---|
| 50 | 0.05 | 1.0 | 1.0 | RBF | 10.0 | 0.406 | 0.965 | 0.400 | 1.491 | 0.522 | 0.798 |
| 50 | 0.05 | 1.0 | 10.0 | COS | - | 0.404 | 0.960 | 0.398 | 1.489 | 0.521 | 0.798 |
| 50 | 0.05 | 1.0 | 10.0 | RBF | 10.0 | 0.404 | 0.960 | 0.398 | 1.488 | 0.521 | 0.798 |
| 50 | 0.05 | 1.0 | 100.0 | COS | - | 0.706 | 1.655 | 0.673 | 2.065 | 0.645 | 0.760 |
| 50 | 0.05 | 1.0 | 100.0 | RBF | 10.0 | 0.617 | 1.476 | 0.588 | 1.938 | 0.615 | 0.781 |
| 50 | 0.10 | 0.1 | 0.0 | COS | - | 0.424 | 1.023 | 0.416 | 1.554 | 0.531 | 0.796 |
| 50 | 0.10 | 0.1 | 0.0 | RBF | 10.0 | 0.424 | 1.023 | 0.416 | 1.554 | 0.531 | 0.796 |
| 50 | 0.10 | 0.1 | 1.0 | COS | - | 0.423 | 1.018 | 0.415 | 1.548 | 0.531 | 0.796 |
| 50 | 0.10 | 0.1 | 1.0 | RBF | 10.0 | 0.423 | 1.018 | 0.415 | 1.548 | 0.531 | 0.796 |
| 50 | 0.10 | 0.1 | 10.0 | COS | - | 0.404 | 0.959 | 0.399 | 1.484 | 0.523 | 0.797 |
| 50 | 0.10 | 0.1 | 10.0 | RBF | 10.0 | 0.406 | 0.963 | 0.400 | 1.490 | 0.524 | 0.797 |
| 50 | 0.10 | 0.1 | 100.0 | COS | - | 0.757 | 1.720 | 0.727 | 2.059 | 0.673 | 0.707 |
| 50 | 0.10 | 0.1 | 100.0 | RBF | 10.0 | 0.746 | 1.724 | 0.716 | 2.080 | 0.668 | 0.727 |
| 50 | 0.10 | 1.0 | 0.0 | COS | - | 0.397 | 0.933 | 0.392 | 1.451 | 0.521 | 0.798 |
| 50 | 0.10 | 1.0 | 0.0 | RBF | 10.0 | 0.397 | 0.933 | 0.392 | 1.451 | 0.521 | 0.798 |
| 50 | 0.10 | 1.0 | 1.0 | COS | - | 0.397 | 0.933 | 0.392 | 1.451 | 0.521 | 0.798 |
| 50 | 0.10 | 1.0 | 1.0 | RBF | 10.0 | 0.397 | 0.933 | 0.392 | 1.451 | 0.521 | 0.798 |
| 50 | 0.10 | 1.0 | 10.0 | COS | - | 0.396 | 0.931 | 0.391 | 1.448 | 0.520 | 0.798 |
| 50 | 0.10 | 1.0 | 10.0 | RBF | 10.0 | 0.396 | 0.930 | 0.391 | 1.447 | 0.520 | 0.798 |
| 50 | 0.10 | 1.0 | 100.0 | COS | - | 0.700 | 1.664 | 0.670 | 2.069 | 0.649 | 0.757 |
| 50 | 0.10 | 1.0 | 100.0 | RBF | 10.0 | 0.601 | 1.458 | 0.573 | 1.931 | 0.608 | 0.781 |
| 50 | 0.50 | 0.1 | 0.0 | COS | - | 0.604 | 1.466 | 0.583 | 1.893 | 0.622 | 0.731 |
| 50 | 0.50 | 0.1 | 0.0 | RBF | 10.0 | 0.604 | 1.466 | 0.583 | 1.893 | 0.622 | 0.731 |
| 50 | 0.50 | 0.1 | 1.0 | COS | - | 0.605 | 1.468 | 0.583 | 1.894 | 0.622 | 0.731 |
| 50 | 0.50 | 0.1 | 1.0 | RBF | 10.0 | 0.604 | 1.467 | 0.583 | 1.894 | 0.622 | 0.731 |
| 50 | 0.50 | 0.1 | 10.0 | COS | - | 0.611 | 1.484 | 0.588 | 1.912 | 0.625 | 0.731 |
| 50 | 0.50 | 0.1 | 10.0 | RBF | 10.0 | 0.610 | 1.482 | 0.588 | 1.909 | 0.625 | 0.731 |
| 50 | 0.50 | 0.1 | 100.0 | COS | - | 0.665 | 1.611 | 0.642 | 2.014 | 0.646 | 0.734 |
| 50 | 0.50 | 0.1 | 100.0 | RBF | 10.0 | 0.658 | 1.596 | 0.634 | 2.005 | 0.643 | 0.734 |
| 50 | 0.50 | 1.0 | 0.0 | COS | - | 0.579 | 1.417 | 0.558 | 1.868 | 0.615 | 0.740 |
| 50 | 0.50 | 1.0 | 0.0 | RBF | 10.0 | 0.579 | 1.417 | 0.558 | 1.868 | 0.615 | 0.740 |
| 50 | 0.50 | 1.0 | 1.0 | COS | - | 0.577 | 1.411 | 0.556 | 1.865 | 0.615 | 0.741 |
| 50 | 0.50 | 1.0 | 1.0 | RBF | 10.0 | 0.578 | 1.414 | 0.558 | 1.868 | 0.615 | 0.740 |
| 50 | 0.50 | 1.0 | 10.0 | COS | - | 0.565 | 1.375 | 0.542 | 1.855 | 0.609 | 0.748 |
| 50 | 0.50 | 1.0 | 10.0 | RBF | 10.0 | 0.567 | 1.384 | 0.545 | 1.856 | 0.611 | 0.747 |
| 50 | 0.50 | 1.0 | 100.0 | COS | - | 0.649 | 1.589 | 0.625 | 2.000 | 0.642 | 0.740 |
| 50 | 0.50 | 1.0 | 100.0 | RBF | 10.0 | 0.622 | 1.524 | 0.597 | 1.968 | 0.630 | 0.746 |
| 50 | 1.00 | 0.1 | 0.0 | COS | - | 0.512 | 1.034 | 0.501 | 1.287 | 0.628 | 0.706 |
| 50 | 1.00 | 0.1 | 0.0 | RBF | 10.0 | 0.512 | 1.034 | 0.501 | 1.287 | 0.628 | 0.706 |
| 50 | 1.00 | 0.1 | 1.0 | COS | - | 0.530 | 1.071 | 0.516 | 1.331 | 0.631 | 0.715 |
| 50 | 1.00 | 0.1 | 1.0 | RBF | 10.0 | 0.528 | 1.066 | 0.514 | 1.326 | 0.631 | 0.714 |
| 50 | 1.00 | 0.1 | 10.0 | COS | - | 0.650 | 1.420 | 0.626 | 1.724 | 0.665 | 0.750 |
| 50 | 1.00 | 0.1 | 10.0 | RBF | 10.0 | 0.641 | 1.384 | 0.617 | 1.686 | 0.664 | 0.748 |
| 50 | 1.00 | 0.1 | 100.0 | COS | - | 0.687 | 1.612 | 0.664 | 1.941 | 0.679 | 0.770 |
| 50 | 1.00 | 0.1 | 100.0 | RBF | 10.0 | 0.689 | 1.609 | 0.664 | 1.940 | 0.679 | 0.772 |
| 50 | 1.00 | 1.0 | 0.0 | COS | - | 0.515 | 1.034 | 0.503 | 1.284 | 0.627 | 0.706 |
| 50 | 1.00 | 1.0 | 0.0 | RBF | 10.0 | 0.515 | 1.034 | 0.503 | 1.284 | 0.627 | 0.706 |
| 50 | 1.00 | 1.0 | 1.0 | COS | - | 0.527 | 1.063 | 0.514 | 1.322 | 0.632 | 0.713 |
| 50 | 1.00 | 1.0 | 1.0 | RBF | 10.0 | 0.525 | 1.059 | 0.512 | 1.319 | 0.631 | 0.713 |
| 50 | 1.00 | 1.0 | 10.0 | COS | - | 0.649 | 1.403 | 0.625 | 1.703 | 0.664 | 0.741 |
| 50 | 1.00 | 1.0 | 10.0 | RBF | 10.0 | 0.639 | 1.377 | 0.615 | 1.667 | 0.662 | 0.738 |
| 50 | 1.00 | 1.0 | 100.0 | COS | - | 0.686 | 1.606 | 0.663 | 1.938 | 0.680 | 0.770 |
| 50 | 1.00 | 1.0 | 100.0 | RBF | 10.0 | 0.688 | 1.603 | 0.663 | 1.932 | 0.680 | 0.769 |

The columns corresponding to "$l$", "$\alpha$", "$\beta$", "$\gamma$", "usim", and "$\sigma$" have the latent dimension, weighting factor, latent vector regularization parameter, cell line similarity regularization parameter, cell line similarity function, and parameter for rbf cell line similarity, respectively, for pLETORg.

**TABLE S7:** pLETORg Performance on New Drugs ($\theta$ = 5)

| $l$ | $\alpha$ | $\beta$ | $\gamma$ | usim | $\sigma$ | AP@5 | AH@5 | AP@10 | AH@10 | sCI | CI |
|---|---|---|---|---|---|---|---|---|---|---|---|
| 5 | 0.00 | 0.1 | 0.0 | COS | - | 0.842 | 2.858 | 0.789 | 3.897 | 0.665 | 0.769 |
| 5 | 0.00 | 0.1 | 0.0 | RBF | 10.0 | 0.842 | 2.858 | 0.789 | 3.897 | 0.665 | 0.769 |
| 5 | 0.00 | 0.1 | 1.0 | COS | - | 0.842 | 2.858 | 0.789 | 3.897 | 0.665 | 0.769 |
| 5 | 0.00 | 0.1 | 1.0 | RBF | 10.0 | 0.842 | 2.858 | 0.789 | 3.897 | 0.665 | 0.769 |
| 5 | 0.00 | 0.1 | 10.0 | COS | - | 0.842 | 2.858 | 0.789 | 3.897 | 0.665 | 0.769 |
| 5 | 0.00 | 0.1 | 10.0 | RBF | 10.0 | 0.842 | 2.858 | 0.789 | 3.897 | 0.665 | 0.769 |
| 5 | 0.00 | 0.1 | 100.0 | COS | - | 0.841 | 2.857 | 0.789 | 3.896 | 0.665 | 0.768 |
| 5 | 0.00 | 0.1 | 100.0 | RBF | 10.0 | 0.842 | 2.857 | 0.789 | 3.896 | 0.665 | 0.769 |
| 5 | 0.00 | 1.0 | 0.0 | COS | - | 0.842 | 2.858 | 0.789 | 3.897 | 0.665 | 0.769 |
| 5 | 0.00 | 1.0 | 0.0 | RBF | 10.0 | 0.842 | 2.858 | 0.789 | 3.897 | 0.665 | 0.769 |
| 5 | 0.00 | 1.0 | 1.0 | COS | - | 0.842 | 2.858 | 0.789 | 3.897 | 0.665 | 0.769 |
| 5 | 0.00 | 1.0 | 1.0 | RBF | 10.0 | 0.842 | 2.858 | 0.789 | 3.897 | 0.665 | 0.769 |
| 5 | 0.00 | 1.0 | 10.0 | COS | - | 0.842 | 2.858 | 0.789 | 3.897 | 0.665 | 0.769 |
| 5 | 0.00 | 1.0 | 10.0 | RBF | 10.0 | 0.842 | 2.858 | 0.789 | 3.897 | 0.665 | 0.769 |
| 5 | 0.00 | 1.0 | 100.0 | COS | - | 0.841 | 2.857 | 0.789 | 3.896 | 0.665 | 0.768 |
| 5 | 0.00 | 1.0 | 100.0 | RBF | 10.0 | 0.842 | 2.857 | 0.789 | 3.896 | 0.665 | 0.769 |
| 5 | 0.05 | 0.1 | 0.0 | COS | - | 0.843 | 2.863 | 0.789 | 3.900 | 0.665 | 0.771 |
| 5 | 0.05 | 0.1 | 0.0 | RBF | 10.0 | 0.843 | 2.863 | 0.789 | 3.900 | 0.665 | 0.771 |
| 5 | 0.05 | 0.1 | 1.0 | COS | - | 0.843 | 2.863 | 0.789 | 3.900 | 0.665 | 0.771 |
| 5 | 0.05 | 0.1 | 1.0 | RBF | 10.0 | 0.843 | 2.863 | 0.789 | 3.900 | 0.665 | 0.771 |
| 5 | 0.05 | 0.1 | 10.0 | COS | - | 0.843 | 2.861 | 0.789 | 3.900 | 0.665 | 0.771 |
| 5 | 0.05 | 0.1 | 10.0 | RBF | 10.0 | 0.843 | 2.862 | 0.789 | 3.900 | 0.665 | 0.771 |
| 5 | 0.05 | 0.1 | 100.0 | COS | - | 0.842 | 2.860 | 0.789 | 3.900 | 0.665 | 0.770 |
| 5 | 0.05 | 0.1 | 100.0 | RBF | 10.0 | 0.843 | 2.860 | 0.789 | 3.899 | 0.665 | 0.770 |
| 5 | 0.05 | 1.0 | 0.0 | COS | - | 0.843 | 2.863 | 0.789 | 3.900 | 0.665 | 0.771 |
| 5 | 0.05 | 1.0 | 0.0 | RBF | 10.0 | 0.843 | 2.863 | 0.789 | 3.900 | 0.665 | 0.771 |
| 5 | 0.05 | 1.0 | 1.0 | COS | - | 0.843 | 2.862 | 0.789 | 3.900 | 0.665 | 0.771 |
| 5 | 0.05 | 1.0 | 1.0 | RBF | 10.0 | 0.843 | 2.862 | 0.789 | 3.900 | 0.665 | 0.771 |
| 5 | 0.05 | 1.0 | 10.0 | COS | - | 0.843 | 2.861 | 0.789 | 3.900 | 0.665 | 0.771 |
| 5 | 0.05 | 1.0 | 10.0 | RBF | 10.0 | 0.843 | 2.861 | 0.789 | 3.900 | 0.665 | 0.771 |
| 5 | 0.05 | 1.0 | 100.0 | COS | - | 0.842 | 2.860 | 0.789 | 3.900 | 0.665 | 0.770 |
| 5 | 0.05 | 1.0 | 100.0 | RBF | 10.0 | 0.843 | 2.860 | 0.789 | 3.899 | 0.665 | 0.770 |
| 5 | 0.10 | 0.1 | 0.0 | COS | - | 0.843 | 2.867 | 0.790 | 3.901 | 0.665 | 0.773 |
| 5 | 0.10 | 0.1 | 0.0 | RBF | 10.0 | 0.843 | 2.867 | 0.790 | 3.901 | 0.665 | 0.773 |
| 5 | 0.10 | 0.1 | 1.0 | COS | - | 0.843 | 2.867 | 0.790 | 3.901 | 0.665 | 0.773 |
| 5 | 0.10 | 0.1 | 1.0 | RBF | 10.0 | 0.843 | 2.867 | 0.790 | 3.901 | 0.665 | 0.773 |
| 5 | 0.10 | 0.1 | 10.0 | COS | - | 0.843 | 2.867 | 0.790 | 3.901 | 0.665 | 0.773 |
| 5 | 0.10 | 0.1 | 10.0 | RBF | 10.0 | 0.843 | 2.867 | 0.790 | 3.901 | 0.665 | 0.773 |
| 5 | 0.10 | 0.1 | 100.0 | COS | - | 0.842 | 2.864 | 0.789 | 3.902 | 0.665 | 0.772 |
| 5 | 0.10 | 0.1 | 100.0 | RBF | 10.0 | 0.843 | 2.865 | 0.789 | 3.902 | 0.665 | 0.772 |
| 5 | 0.10 | 1.0 | 0.0 | COS | - | 0.843 | 2.867 | 0.790 | 3.901 | 0.665 | 0.773 |
| 5 | 0.10 | 1.0 | 0.0 | RBF | 10.0 | 0.843 | 2.867 | 0.790 | 3.901 | 0.665 | 0.773 |
| 5 | 0.10 | 1.0 | 1.0 | COS | - | 0.843 | 2.867 | 0.790 | 3.901 | 0.665 | 0.773 |
| 5 | 0.10 | 1.0 | 1.0 | RBF | 10.0 | 0.843 | 2.867 | 0.790 | 3.901 | 0.665 | 0.773 |
| 5 | 0.10 | 1.0 | 10.0 | COS | - | 0.843 | 2.867 | 0.790 | 3.901 | 0.665 | 0.773 |
| 5 | 0.10 | 1.0 | 10.0 | RBF | 10.0 | 0.843 | 2.867 | 0.790 | 3.901 | 0.665 | 0.773 |
| 5 | 0.10 | 1.0 | 100.0 | COS | - | 0.843 | 2.864 | 0.789 | 3.902 | 0.665 | 0.772 |
| 5 | 0.10 | 1.0 | 100.0 | RBF | 10.0 | 0.843 | 2.865 | 0.789 | 3.902 | 0.665 | 0.772 |
| 5 | 0.50 | 0.1 | 0.0 | COS | - | 0.845 | 2.880 | 0.792 | 3.923 | 0.668 | 0.789 |
| 5 | 0.50 | 0.1 | 0.0 | RBF | 10.0 | 0.845 | 2.880 | 0.792 | 3.923 | 0.668 | 0.789 |
| 5 | 0.50 | 0.1 | 1.0 | COS | - | 0.845 | 2.880 | 0.792 | 3.923 | 0.668 | 0.789 |
| 5 | 0.50 | 0.1 | 1.0 | RBF | 10.0 | 0.845 | 2.880 | 0.792 | 3.923 | 0.668 | 0.789 |
| 5 | 0.50 | 0.1 | 10.0 | COS | - | 0.845 | 2.880 | 0.792 | 3.923 | 0.668 | 0.789 |
| 5 | 0.50 | 0.1 | 10.0 | RBF | 10.0 | 0.845 | 2.880 | 0.792 | 3.923 | 0.668 | 0.789 |
| 5 | 0.50 | 0.1 | 100.0 | COS | - | 0.845 | 2.879 | 0.792 | 3.920 | 0.669 | 0.789 |
| 5 | 0.50 | 0.1 | 100.0 | RBF | 10.0 | 0.845 | 2.879 | 0.792 | 3.921 | 0.668 | 0.789 |
| 5 | 0.50 | 1.0 | 0.0 | COS | - | 0.845 | 2.880 | 0.792 | 3.923 | 0.668 | 0.789 |

Continued on next page

TABLE S7 – continued from previous page

| $l$ | $\alpha$ | $\beta$ | $\gamma$ | usim | $\sigma$ | AP@5 | AH@5 | AP@10 | AH@10 | sCI | CI |
|---|---|---|---|---|---|---|---|---|---|---|---|
| 5 | 0.50 | 1.0 | 0.0 | RBF | 10.0 | 0.845 | 2.880 | 0.792 | 3.923 | 0.668 | 0.789 |
| 5 | 0.50 | 1.0 | 1.0 | COS | - | 0.845 | 2.880 | 0.792 | 3.923 | 0.668 | 0.789 |
| 5 | 0.50 | 1.0 | 1.0 | RBF | 10.0 | 0.845 | 2.880 | 0.792 | 3.923 | 0.668 | 0.789 |
| 5 | 0.50 | 1.0 | 10.0 | COS | - | 0.845 | 2.880 | 0.792 | 3.923 | 0.669 | 0.789 |
| 5 | 0.50 | 1.0 | 10.0 | RBF | 10.0 | 0.845 | 2.880 | 0.792 | 3.923 | 0.668 | 0.789 |
| 5 | 0.50 | 1.0 | 100.0 | COS | - | 0.845 | 2.879 | 0.792 | 3.920 | 0.668 | 0.789 |
| 5 | 0.50 | 1.0 | 100.0 | RBF | 10.0 | 0.845 | 2.879 | 0.792 | 3.920 | 0.668 | 0.789 |
| 5 | 1.00 | 0.1 | 0.0 | COS | - | 0.689 | 2.080 | 0.638 | 2.981 | 0.668 | 0.696 |
| 5 | 1.00 | 0.1 | 0.0 | RBF | 10.0 | 0.689 | 2.080 | 0.638 | 2.981 | 0.668 | 0.696 |
| 5 | 1.00 | 0.1 | 1.0 | COS | - | 0.692 | 2.091 | 0.641 | 2.994 | 0.668 | 0.698 |
| 5 | 1.00 | 0.1 | 1.0 | RBF | 10.0 | 0.692 | 2.089 | 0.641 | 2.993 | 0.669 | 0.697 |
| 5 | 1.00 | 0.1 | 10.0 | COS | - | 0.703 | 2.129 | 0.651 | 3.029 | 0.669 | 0.704 |
| 5 | 1.00 | 0.1 | 10.0 | RBF | 10.0 | 0.702 | 2.127 | 0.651 | 3.025 | 0.669 | 0.703 |
| 5 | 1.00 | 0.1 | 100.0 | COS | - | 0.737 | 2.227 | 0.681 | 3.125 | 0.675 | 0.727 |
| 5 | 1.00 | 0.1 | 100.0 | RBF | 10.0 | 0.733 | 2.213 | 0.676 | 3.107 | 0.675 | 0.722 |
| 5 | 1.00 | 1.0 | 0.0 | COS | - | 0.693 | 2.091 | 0.642 | 2.985 | 0.668 | 0.695 |
| 5 | 1.00 | 1.0 | 0.0 | RBF | 10.0 | 0.693 | 2.091 | 0.642 | 2.985 | 0.668 | 0.695 |
| 5 | 1.00 | 1.0 | 1.0 | COS | - | 0.695 | 2.101 | 0.644 | 2.991 | 0.669 | 0.696 |
| 5 | 1.00 | 1.0 | 1.0 | RBF | 10.0 | 0.694 | 2.101 | 0.644 | 2.992 | 0.669 | 0.696 |
| 5 | 1.00 | 1.0 | 10.0 | COS | - | 0.705 | 2.134 | 0.654 | 3.026 | 0.669 | 0.702 |
| 5 | 1.00 | 1.0 | 10.0 | RBF | 10.0 | 0.704 | 2.133 | 0.652 | 3.026 | 0.669 | 0.702 |
| 5 | 1.00 | 1.0 | 100.0 | COS | - | 0.737 | 2.231 | 0.682 | 3.120 | 0.675 | 0.725 |
| 5 | 1.00 | 1.0 | 100.0 | RBF | 10.0 | 0.733 | 2.212 | 0.677 | 3.101 | 0.675 | 0.720 |
| 10 | 0.00 | 0.1 | 0.0 | COS | - | 0.854 | 2.954 | 0.804 | 3.978 | 0.659 | 0.786 |
| 10 | 0.00 | 0.1 | 0.0 | RBF | 10.0 | 0.854 | 2.954 | 0.804 | 3.978 | 0.659 | 0.786 |
| 10 | 0.00 | 0.1 | 1.0 | COS | - | 0.854 | 2.954 | 0.804 | 3.978 | 0.659 | 0.786 |
| 10 | 0.00 | 0.1 | 1.0 | RBF | 10.0 | 0.854 | 2.954 | 0.804 | 3.978 | 0.659 | 0.786 |
| 10 | 0.00 | 0.1 | 10.0 | COS | - | 0.854 | 2.954 | 0.804 | 3.977 | 0.659 | 0.786 |
| 10 | 0.00 | 0.1 | 10.0 | RBF | 10.0 | 0.854 | 2.954 | 0.804 | 3.977 | 0.659 | 0.786 |
| 10 | 0.00 | 0.1 | 100.0 | COS | - | 0.854 | 2.953 | 0.804 | 3.977 | 0.659 | 0.785 |
| 10 | 0.00 | 0.1 | 100.0 | RBF | 10.0 | 0.854 | 2.953 | 0.804 | 3.977 | 0.659 | 0.785 |
| 10 | 0.00 | 1.0 | 0.0 | COS | - | 0.854 | 2.954 | 0.804 | 3.978 | 0.659 | 0.786 |
| 10 | 0.00 | 1.0 | 0.0 | RBF | 10.0 | 0.854 | 2.954 | 0.804 | 3.978 | 0.659 | 0.786 |
| 10 | 0.00 | 1.0 | 1.0 | COS | - | 0.854 | 2.954 | 0.804 | 3.978 | 0.659 | 0.786 |
| 10 | 0.00 | 1.0 | 1.0 | RBF | 10.0 | 0.854 | 2.954 | 0.804 | 3.978 | 0.659 | 0.786 |
| 10 | 0.00 | 1.0 | 10.0 | COS | - | 0.854 | 2.954 | 0.805 | 3.977 | 0.659 | 0.786 |
| 10 | 0.00 | 1.0 | 10.0 | RBF | 10.0 | 0.854 | 2.954 | 0.804 | 3.977 | 0.659 | 0.786 |
| 10 | 0.00 | 1.0 | 100.0 | COS | - | 0.854 | 2.953 | 0.804 | 3.977 | 0.659 | 0.785 |
| 10 | 0.00 | 1.0 | 100.0 | RBF | 10.0 | 0.854 | 2.953 | 0.804 | 3.977 | 0.659 | 0.785 |
| 10 | 0.05 | 0.1 | 0.0 | COS | - | 0.853 | 2.958 | 0.804 | 3.983 | 0.660 | 0.787 |
| 10 | 0.05 | 0.1 | 0.0 | RBF | 10.0 | 0.853 | 2.958 | 0.804 | 3.983 | 0.660 | 0.787 |
| 10 | 0.05 | 0.1 | 1.0 | COS | - | 0.853 | 2.958 | 0.804 | 3.983 | 0.659 | 0.787 |
| 10 | 0.05 | 0.1 | 1.0 | RBF | 10.0 | 0.853 | 2.958 | 0.804 | 3.983 | 0.659 | 0.787 |
| 10 | 0.05 | 0.1 | 10.0 | COS | - | 0.853 | 2.958 | 0.804 | 3.982 | 0.660 | 0.787 |
| 10 | 0.05 | 0.1 | 10.0 | RBF | 10.0 | 0.853 | 2.958 | 0.804 | 3.983 | 0.660 | 0.787 |
| 10 | 0.05 | 0.1 | 100.0 | COS | - | 0.853 | 2.955 | 0.804 | 3.980 | 0.660 | 0.787 |
| 10 | 0.05 | 0.1 | 100.0 | RBF | 10.0 | 0.853 | 2.955 | 0.804 | 3.980 | 0.660 | 0.787 |
| 10 | 0.05 | 1.0 | 0.0 | COS | - | 0.853 | 2.958 | 0.804 | 3.983 | 0.659 | 0.787 |
| 10 | 0.05 | 1.0 | 0.0 | RBF | 10.0 | 0.853 | 2.958 | 0.804 | 3.983 | 0.659 | 0.787 |
| 10 | 0.05 | 1.0 | 1.0 | COS | - | 0.853 | 2.958 | 0.804 | 3.983 | 0.659 | 0.787 |
| 10 | 0.05 | 1.0 | 1.0 | RBF | 10.0 | 0.853 | 2.958 | 0.804 | 3.983 | 0.659 | 0.787 |
| 10 | 0.05 | 1.0 | 10.0 | COS | - | 0.853 | 2.958 | 0.804 | 3.982 | 0.660 | 0.787 |
| 10 | 0.05 | 1.0 | 10.0 | RBF | 10.0 | 0.853 | 2.958 | 0.804 | 3.983 | 0.660 | 0.787 |
| 10 | 0.05 | 1.0 | 100.0 | COS | - | 0.853 | 2.955 | 0.804 | 3.980 | 0.660 | 0.787 |
| 10 | 0.05 | 1.0 | 100.0 | RBF | 10.0 | 0.853 | 2.955 | 0.804 | 3.980 | 0.660 | 0.787 |
| 10 | 0.10 | 0.1 | 0.0 | COS | - | 0.854 | 2.960 | 0.805 | 3.981 | 0.661 | 0.789 |
| 10 | 0.10 | 0.1 | 0.0 | RBF | 10.0 | 0.854 | 2.960 | 0.805 | 3.981 | 0.661 | 0.789 |
| 10 | 0.10 | 0.1 | 1.0 | COS | - | 0.854 | 2.960 | 0.805 | 3.980 | 0.661 | 0.789 |

Continued on next page

TABLE S7 – continued from previous page

| $l$ | $\alpha$ | $\beta$ | $\gamma$ | usim | $\sigma$ | AP@5 | AH@5 | AP@10 | AH@10 | sCI | CI |
|---|---|---|---|---|---|---|---|---|---|---|---|
| 10 | 0.10 | 0.1 | 1.0 | RBF | 10.0 | 0.854 | 2.960 | 0.805 | 3.980 | 0.661 | 0.789 |
| 10 | 0.10 | 0.1 | 10.0 | COS | - | 0.854 | 2.960 | 0.805 | 3.981 | 0.661 | 0.789 |
| 10 | 0.10 | 0.1 | 10.0 | RBF | 10.0 | 0.854 | 2.960 | 0.805 | 3.981 | 0.661 | 0.789 |
| 10 | 0.10 | 0.1 | 100.0 | COS | - | 0.853 | 2.958 | 0.804 | 3.982 | 0.661 | 0.789 |
| 10 | 0.10 | 0.1 | 100.0 | RBF | 10.0 | 0.853 | 2.958 | 0.804 | 3.982 | 0.661 | 0.789 |
| 10 | 0.10 | 1.0 | 0.0 | COS | - | 0.854 | 2.960 | 0.805 | 3.980 | 0.661 | 0.789 |
| 10 | 0.10 | 1.0 | 0.0 | RBF | 10.0 | 0.854 | 2.960 | 0.805 | 3.980 | 0.661 | 0.789 |
| 10 | 0.10 | 1.0 | 1.0 | COS | - | 0.854 | 2.960 | 0.805 | 3.980 | 0.661 | 0.789 |
| 10 | 0.10 | 1.0 | 1.0 | RBF | 10.0 | 0.854 | 2.960 | 0.805 | 3.980 | 0.661 | 0.789 |
| 10 | 0.10 | 1.0 | 10.0 | COS | - | 0.854 | 2.960 | 0.805 | 3.981 | 0.661 | 0.789 |
| 10 | 0.10 | 1.0 | 10.0 | RBF | 10.0 | 0.854 | 2.960 | 0.805 | 3.981 | 0.661 | 0.789 |
| 10 | 0.10 | 1.0 | 100.0 | COS | - | 0.853 | 2.958 | 0.804 | 3.981 | 0.661 | 0.789 |
| 10 | 0.10 | 1.0 | 100.0 | RBF | 10.0 | 0.853 | 2.958 | 0.804 | 3.982 | 0.661 | 0.789 |
| 10 | 0.50 | 0.1 | 0.0 | COS | - | 0.855 | 2.965 | 0.806 | 3.985 | 0.658 | 0.804 |
| 10 | 0.50 | 0.1 | 0.0 | RBF | 10.0 | 0.855 | 2.965 | 0.806 | 3.985 | 0.658 | 0.804 |
| 10 | 0.50 | 0.1 | 1.0 | COS | - | 0.855 | 2.965 | 0.806 | 3.985 | 0.658 | 0.804 |
| 10 | 0.50 | 0.1 | 1.0 | RBF | 10.0 | 0.855 | 2.965 | 0.806 | 3.985 | 0.658 | 0.804 |
| 10 | 0.50 | 0.1 | 10.0 | COS | - | 0.855 | 2.965 | 0.806 | 3.985 | 0.658 | 0.804 |
| 10 | 0.50 | 0.1 | 10.0 | RBF | 10.0 | 0.855 | 2.965 | 0.806 | 3.985 | 0.658 | 0.804 |
| 10 | 0.50 | 0.1 | 100.0 | COS | - | 0.855 | 2.965 | 0.806 | 3.986 | 0.658 | 0.804 |
| 10 | 0.50 | 0.1 | 100.0 | RBF | 10.0 | 0.855 | 2.965 | 0.806 | 3.985 | 0.658 | 0.804 |
| 10 | 0.50 | 1.0 | 0.0 | COS | - | 0.855 | 2.965 | 0.806 | 3.985 | 0.658 | 0.804 |
| 10 | 0.50 | 1.0 | 0.0 | RBF | 10.0 | 0.855 | 2.965 | 0.806 | 3.985 | 0.658 | 0.804 |
| 10 | 0.50 | 1.0 | 1.0 | COS | - | 0.855 | 2.965 | 0.806 | 3.985 | 0.658 | 0.804 |
| 10 | 0.50 | 1.0 | 1.0 | RBF | 10.0 | 0.855 | 2.965 | 0.806 | 3.985 | 0.658 | 0.804 |
| 10 | 0.50 | 1.0 | 10.0 | COS | - | 0.855 | 2.965 | 0.806 | 3.985 | 0.658 | 0.804 |
| 10 | 0.50 | 1.0 | 10.0 | RBF | 10.0 | 0.855 | 2.965 | 0.806 | 3.985 | 0.658 | 0.804 |
| 10 | 0.50 | 1.0 | 100.0 | COS | - | 0.855 | 2.965 | 0.806 | 3.986 | 0.658 | 0.804 |
| 10 | 0.50 | 1.0 | 100.0 | RBF | 10.0 | 0.855 | 2.965 | 0.806 | 3.986 | 0.658 | 0.804 |
| 10 | 1.00 | 0.1 | 0.0 | COS | - | 0.665 | 1.918 | 0.620 | 2.663 | 0.637 | 0.640 |
| 10 | 1.00 | 0.1 | 0.0 | RBF | 10.0 | 0.665 | 1.918 | 0.620 | 2.663 | 0.637 | 0.640 |
| 10 | 1.00 | 0.1 | 1.0 | COS | - | 0.668 | 1.938 | 0.623 | 2.686 | 0.637 | 0.644 |
| 10 | 1.00 | 0.1 | 1.0 | RBF | 10.0 | 0.668 | 1.939 | 0.623 | 2.685 | 0.637 | 0.644 |
| 10 | 1.00 | 0.1 | 10.0 | COS | - | 0.685 | 1.994 | 0.637 | 2.752 | 0.640 | 0.657 |
| 10 | 1.00 | 0.1 | 10.0 | RBF | 10.0 | 0.684 | 2.001 | 0.637 | 2.754 | 0.640 | 0.657 |
| 10 | 1.00 | 0.1 | 100.0 | COS | - | 0.726 | 2.188 | 0.675 | 2.991 | 0.655 | 0.708 |
| 10 | 1.00 | 0.1 | 100.0 | RBF | 10.0 | 0.726 | 2.178 | 0.674 | 2.979 | 0.654 | 0.705 |
| 10 | 1.00 | 1.0 | 0.0 | COS | - | 0.668 | 1.929 | 0.624 | 2.669 | 0.637 | 0.638 |
| 10 | 1.00 | 1.0 | 0.0 | RBF | 10.0 | 0.668 | 1.929 | 0.624 | 2.669 | 0.637 | 0.638 |
| 10 | 1.00 | 1.0 | 1.0 | COS | - | 0.672 | 1.953 | 0.627 | 2.688 | 0.636 | 0.642 |
| 10 | 1.00 | 1.0 | 1.0 | RBF | 10.0 | 0.672 | 1.952 | 0.627 | 2.687 | 0.636 | 0.641 |
| 10 | 1.00 | 1.0 | 10.0 | COS | - | 0.690 | 2.014 | 0.642 | 2.768 | 0.640 | 0.656 |
| 10 | 1.00 | 1.0 | 10.0 | RBF | 10.0 | 0.688 | 2.006 | 0.640 | 2.756 | 0.640 | 0.655 |
| 10 | 1.00 | 1.0 | 100.0 | COS | - | 0.731 | 2.194 | 0.678 | 3.001 | 0.656 | 0.710 |
| 10 | 1.00 | 1.0 | 100.0 | RBF | 10.0 | 0.726 | 2.174 | 0.675 | 2.966 | 0.654 | 0.702 |
| 15 | 0.00 | 0.1 | 0.0 | COS | - | 0.850 | 2.961 | 0.802 | 4.004 | 0.638 | 0.791 |
| 15 | 0.00 | 0.1 | 0.0 | RBF | 10.0 | 0.850 | 2.961 | 0.802 | 4.004 | 0.638 | 0.791 |
| 15 | 0.00 | 0.1 | 1.0 | COS | - | 0.850 | 2.961 | 0.802 | 4.004 | 0.638 | 0.791 |
| 15 | 0.00 | 0.1 | 1.0 | RBF | 10.0 | 0.850 | 2.961 | 0.802 | 4.004 | 0.638 | 0.791 |
| 15 | 0.00 | 0.1 | 10.0 | COS | - | 0.849 | 2.961 | 0.802 | 4.005 | 0.638 | 0.791 |
| 15 | 0.00 | 0.1 | 10.0 | RBF | 10.0 | 0.849 | 2.962 | 0.802 | 4.004 | 0.638 | 0.791 |
| 15 | 0.00 | 0.1 | 100.0 | COS | - | 0.850 | 2.962 | 0.802 | 4.007 | 0.638 | 0.791 |
| 15 | 0.00 | 0.1 | 100.0 | RBF | 10.0 | 0.850 | 2.960 | 0.802 | 4.007 | 0.638 | 0.792 |
| 15 | 0.00 | 1.0 | 0.0 | COS | - | 0.850 | 2.960 | 0.802 | 4.005 | 0.637 | 0.792 |
| 15 | 0.00 | 1.0 | 0.0 | RBF | 10.0 | 0.850 | 2.960 | 0.802 | 4.005 | 0.637 | 0.792 |
| 15 | 0.00 | 1.0 | 1.0 | COS | - | 0.850 | 2.960 | 0.802 | 4.005 | 0.637 | 0.792 |
| 15 | 0.00 | 1.0 | 1.0 | RBF | 10.0 | 0.850 | 2.960 | 0.802 | 4.005 | 0.637 | 0.792 |
| 15 | 0.00 | 1.0 | 10.0 | COS | - | 0.849 | 2.961 | 0.802 | 4.005 | 0.637 | 0.792 |

Continued on next page

TABLE S7 – continued from previous page

| $l$ | $\alpha$ | $\beta$ | $\gamma$ | usim | $\sigma$ | AP@5 | AH@5 | AP@10 | AH@10 | sCI | CI |
|---|---|---|---|---|---|---|---|---|---|---|---|
| 15 | 0.00 | 1.0 | 10.0 | RBF | 10.0 | 0.849 | 2.961 | 0.802 | 4.005 | 0.637 | 0.792 |
| 15 | 0.00 | 1.0 | 100.0 | COS | - | 0.850 | 2.960 | 0.802 | 4.007 | 0.638 | 0.791 |
| 15 | 0.00 | 1.0 | 100.0 | RBF | 10.0 | 0.850 | 2.960 | 0.802 | 4.007 | 0.638 | 0.792 |
| 15 | 0.05 | 0.1 | 0.0 | COS | - | 0.849 | 2.956 | 0.801 | 4.006 | 0.636 | 0.793 |
| 15 | 0.05 | 0.1 | 0.0 | RBF | 10.0 | 0.849 | 2.956 | 0.801 | 4.006 | 0.636 | 0.793 |
| 15 | 0.05 | 0.1 | 1.0 | COS | - | 0.849 | 2.956 | 0.801 | 4.006 | 0.636 | 0.793 |
| 15 | 0.05 | 0.1 | 1.0 | RBF | 10.0 | 0.849 | 2.956 | 0.801 | 4.006 | 0.636 | 0.793 |
| 15 | 0.05 | 0.1 | 10.0 | COS | - | 0.849 | 2.956 | 0.801 | 4.006 | 0.636 | 0.793 |
| 15 | 0.05 | 0.1 | 10.0 | RBF | 10.0 | 0.849 | 2.956 | 0.801 | 4.006 | 0.636 | 0.793 |
| 15 | 0.05 | 0.1 | 100.0 | COS | - | 0.849 | 2.960 | 0.801 | 4.005 | 0.637 | 0.793 |
| 15 | 0.05 | 0.1 | 100.0 | RBF | 10.0 | 0.849 | 2.960 | 0.801 | 4.006 | 0.636 | 0.793 |
| 15 | 0.05 | 1.0 | 0.0 | COS | - | 0.849 | 2.956 | 0.801 | 4.006 | 0.636 | 0.793 |
| 15 | 0.05 | 1.0 | 0.0 | RBF | 10.0 | 0.849 | 2.956 | 0.801 | 4.006 | 0.636 | 0.793 |
| 15 | 0.05 | 1.0 | 1.0 | COS | - | 0.849 | 2.956 | 0.801 | 4.006 | 0.636 | 0.793 |
| 15 | 0.05 | 1.0 | 1.0 | RBF | 10.0 | 0.849 | 2.956 | 0.801 | 4.006 | 0.636 | 0.793 |
| 15 | 0.05 | 1.0 | 10.0 | COS | - | 0.849 | 2.956 | 0.801 | 4.006 | 0.636 | 0.793 |
| 15 | 0.05 | 1.0 | 10.0 | RBF | 10.0 | 0.849 | 2.956 | 0.801 | 4.006 | 0.636 | 0.793 |
| 15 | 0.05 | 1.0 | 100.0 | COS | - | 0.849 | 2.960 | 0.801 | 4.005 | 0.637 | 0.793 |
| 15 | 0.05 | 1.0 | 100.0 | RBF | 10.0 | 0.849 | 2.960 | 0.801 | 4.006 | 0.636 | 0.793 |
| 15 | 0.10 | 0.1 | 0.0 | COS | - | 0.848 | 2.951 | 0.800 | 4.007 | 0.635 | 0.795 |
| 15 | 0.10 | 0.1 | 0.0 | RBF | 10.0 | 0.848 | 2.951 | 0.800 | 4.007 | 0.635 | 0.795 |
| 15 | 0.10 | 0.1 | 1.0 | COS | - | 0.848 | 2.951 | 0.800 | 4.007 | 0.635 | 0.795 |
| 15 | 0.10 | 0.1 | 1.0 | RBF | 10.0 | 0.848 | 2.951 | 0.800 | 4.007 | 0.635 | 0.795 |
| 15 | 0.10 | 0.1 | 10.0 | COS | - | 0.848 | 2.952 | 0.800 | 4.007 | 0.635 | 0.795 |
| 15 | 0.10 | 0.1 | 10.0 | RBF | 10.0 | 0.848 | 2.952 | 0.800 | 4.007 | 0.635 | 0.795 |
| 15 | 0.10 | 0.1 | 100.0 | COS | - | 0.848 | 2.956 | 0.800 | 4.007 | 0.636 | 0.795 |
| 15 | 0.10 | 0.1 | 100.0 | RBF | 10.0 | 0.848 | 2.955 | 0.800 | 4.008 | 0.636 | 0.795 |
| 15 | 0.10 | 1.0 | 0.0 | COS | - | 0.848 | 2.951 | 0.800 | 4.007 | 0.635 | 0.795 |
| 15 | 0.10 | 1.0 | 0.0 | RBF | 10.0 | 0.848 | 2.951 | 0.800 | 4.007 | 0.635 | 0.795 |
| 15 | 0.10 | 1.0 | 1.0 | COS | - | 0.848 | 2.951 | 0.800 | 4.007 | 0.635 | 0.795 |
| 15 | 0.10 | 1.0 | 1.0 | RBF | 10.0 | 0.848 | 2.951 | 0.800 | 4.007 | 0.635 | 0.795 |
| 15 | 0.10 | 1.0 | 10.0 | COS | - | 0.848 | 2.952 | 0.800 | 4.007 | 0.635 | 0.795 |
| 15 | 0.10 | 1.0 | 10.0 | RBF | 10.0 | 0.848 | 2.952 | 0.800 | 4.007 | 0.635 | 0.795 |
| 15 | 0.10 | 1.0 | 100.0 | COS | - | 0.848 | 2.956 | 0.800 | 4.007 | 0.636 | 0.795 |
| 15 | 0.10 | 1.0 | 100.0 | RBF | 10.0 | 0.848 | 2.955 | 0.800 | 4.008 | 0.636 | 0.795 |
| 15 | 0.50 | 0.1 | 0.0 | COS | - | 0.838 | 2.893 | 0.789 | 3.952 | 0.613 | 0.808 |
| 15 | 0.50 | 0.1 | 0.0 | RBF | 10.0 | 0.838 | 2.893 | 0.789 | 3.952 | 0.613 | 0.808 |
| 15 | 0.50 | 0.1 | 1.0 | COS | - | 0.838 | 2.893 | 0.789 | 3.952 | 0.613 | 0.808 |
| 15 | 0.50 | 0.1 | 1.0 | RBF | 10.0 | 0.838 | 2.893 | 0.789 | 3.952 | 0.613 | 0.808 |
| 15 | 0.50 | 0.1 | 10.0 | COS | - | 0.838 | 2.893 | 0.789 | 3.953 | 0.613 | 0.808 |
| 15 | 0.50 | 0.1 | 10.0 | RBF | 10.0 | 0.838 | 2.893 | 0.789 | 3.954 | 0.613 | 0.808 |
| 15 | 0.50 | 0.1 | 100.0 | COS | - | 0.838 | 2.897 | 0.789 | 3.958 | 0.615 | 0.808 |
| 15 | 0.50 | 0.1 | 100.0 | RBF | 10.0 | 0.838 | 2.897 | 0.789 | 3.956 | 0.614 | 0.808 |
| 15 | 0.50 | 1.0 | 0.0 | COS | - | 0.838 | 2.893 | 0.789 | 3.952 | 0.613 | 0.808 |
| 15 | 0.50 | 1.0 | 0.0 | RBF | 10.0 | 0.838 | 2.893 | 0.789 | 3.952 | 0.613 | 0.808 |
| 15 | 0.50 | 1.0 | 1.0 | COS | - | 0.838 | 2.892 | 0.789 | 3.952 | 0.613 | 0.808 |
| 15 | 0.50 | 1.0 | 1.0 | RBF | 10.0 | 0.838 | 2.892 | 0.789 | 3.952 | 0.613 | 0.808 |
| 15 | 0.50 | 1.0 | 10.0 | COS | - | 0.838 | 2.893 | 0.789 | 3.953 | 0.613 | 0.808 |
| 15 | 0.50 | 1.0 | 10.0 | RBF | 10.0 | 0.838 | 2.893 | 0.789 | 3.954 | 0.613 | 0.808 |
| 15 | 0.50 | 1.0 | 100.0 | COS | - | 0.838 | 2.897 | 0.789 | 3.958 | 0.615 | 0.808 |
| 15 | 0.50 | 1.0 | 100.0 | RBF | 10.0 | 0.838 | 2.897 | 0.789 | 3.957 | 0.614 | 0.808 |
| 15 | 1.00 | 0.1 | 0.0 | COS | - | 0.670 | 1.869 | 0.626 | 2.544 | 0.597 | 0.603 |
| 15 | 1.00 | 0.1 | 0.0 | RBF | 10.0 | 0.670 | 1.869 | 0.626 | 2.544 | 0.597 | 0.603 |
| 15 | 1.00 | 0.1 | 1.0 | COS | - | 0.676 | 1.896 | 0.630 | 2.585 | 0.601 | 0.613 |
| 15 | 1.00 | 0.1 | 1.0 | RBF | 10.0 | 0.675 | 1.893 | 0.629 | 2.578 | 0.601 | 0.612 |
| 15 | 1.00 | 0.1 | 10.0 | COS | - | 0.685 | 1.961 | 0.639 | 2.671 | 0.608 | 0.631 |
| 15 | 1.00 | 0.1 | 10.0 | RBF | 10.0 | 0.685 | 1.955 | 0.638 | 2.668 | 0.608 | 0.630 |
| 15 | 1.00 | 0.1 | 100.0 | COS | - | 0.726 | 2.159 | 0.674 | 2.965 | 0.644 | 0.700 |

Continued on next page

TABLE S7 – continued from previous page

| $l$ | $\alpha$ | $\beta$ | $\gamma$ | usim | $\sigma$ | AP@5 | AH@5 | AP@10 | AH@10 | sCI | CI |
|---|---|---|---|---|---|---|---|---|---|---|---|
| 15 | 1.00 | 0.1 | 100.0 | RBF | 10.0 | 0.724 | 2.155 | 0.673 | 2.939 | 0.644 | 0.693 |
| 15 | 1.00 | 1.0 | 0.0 | COS | - | 0.674 | 1.889 | 0.629 | 2.573 | 0.602 | 0.605 |
| 15 | 1.00 | 1.0 | 0.0 | RBF | 10.0 | 0.674 | 1.889 | 0.629 | 2.573 | 0.602 | 0.605 |
| 15 | 1.00 | 1.0 | 1.0 | COS | - | 0.677 | 1.910 | 0.631 | 2.606 | 0.603 | 0.613 |
| 15 | 1.00 | 1.0 | 1.0 | RBF | 10.0 | 0.677 | 1.909 | 0.631 | 2.600 | 0.603 | 0.612 |
| 15 | 1.00 | 1.0 | 10.0 | COS | - | 0.690 | 1.982 | 0.643 | 2.693 | 0.610 | 0.632 |
| 15 | 1.00 | 1.0 | 10.0 | RBF | 10.0 | 0.688 | 1.971 | 0.642 | 2.688 | 0.609 | 0.632 |
| 15 | 1.00 | 1.0 | 100.0 | COS | - | 0.727 | 2.161 | 0.676 | 2.959 | 0.647 | 0.695 |
| 15 | 1.00 | 1.0 | 100.0 | RBF | 10.0 | 0.720 | 2.124 | 0.670 | 2.892 | 0.642 | 0.680 |
| 30 | 0.00 | 0.1 | 0.0 | COS | - | 0.795 | 2.798 | 0.747 | 3.917 | 0.578 | 0.799 |
| 30 | 0.00 | 0.1 | 0.0 | RBF | 10.0 | 0.795 | 2.798 | 0.747 | 3.917 | 0.578 | 0.799 |
| 30 | 0.00 | 0.1 | 1.0 | COS | - | 0.795 | 2.798 | 0.747 | 3.917 | 0.578 | 0.799 |
| 30 | 0.00 | 0.1 | 1.0 | RBF | 10.0 | 0.795 | 2.798 | 0.747 | 3.917 | 0.578 | 0.799 |
| 30 | 0.00 | 0.1 | 10.0 | COS | - | 0.792 | 2.791 | 0.745 | 3.913 | 0.576 | 0.800 |
| 30 | 0.00 | 0.1 | 10.0 | RBF | 10.0 | 0.792 | 2.791 | 0.745 | 3.913 | 0.576 | 0.800 |
| 30 | 0.00 | 0.1 | 100.0 | COS | - | 0.834 | 2.951 | 0.788 | 4.006 | 0.633 | 0.780 |
| 30 | 0.00 | 0.1 | 100.0 | RBF | 10.0 | 0.817 | 2.900 | 0.771 | 3.981 | 0.608 | 0.791 |
| 30 | 0.00 | 1.0 | 0.0 | COS | - | 0.791 | 2.785 | 0.743 | 3.911 | 0.574 | 0.800 |
| 30 | 0.00 | 1.0 | 0.0 | RBF | 10.0 | 0.791 | 2.785 | 0.743 | 3.911 | 0.574 | 0.800 |
| 30 | 0.00 | 1.0 | 1.0 | COS | - | 0.791 | 2.785 | 0.743 | 3.911 | 0.574 | 0.800 |
| 30 | 0.00 | 1.0 | 1.0 | RBF | 10.0 | 0.791 | 2.785 | 0.743 | 3.911 | 0.574 | 0.800 |
| 30 | 0.00 | 1.0 | 10.0 | COS | - | 0.791 | 2.785 | 0.743 | 3.912 | 0.575 | 0.800 |
| 30 | 0.00 | 1.0 | 10.0 | RBF | 10.0 | 0.791 | 2.786 | 0.743 | 3.912 | 0.575 | 0.800 |
| 30 | 0.00 | 1.0 | 100.0 | COS | - | 0.799 | 2.823 | 0.752 | 3.940 | 0.584 | 0.799 |
| 30 | 0.00 | 1.0 | 100.0 | RBF | 10.0 | 0.793 | 2.797 | 0.746 | 3.917 | 0.576 | 0.801 |
| 30 | 0.05 | 0.1 | 0.0 | COS | - | 0.787 | 2.755 | 0.738 | 3.892 | 0.569 | 0.802 |
| 30 | 0.05 | 0.1 | 0.0 | RBF | 10.0 | 0.787 | 2.755 | 0.738 | 3.892 | 0.569 | 0.802 |
| 30 | 0.05 | 0.1 | 1.0 | COS | - | 0.787 | 2.755 | 0.738 | 3.892 | 0.569 | 0.802 |
| 30 | 0.05 | 0.1 | 1.0 | RBF | 10.0 | 0.787 | 2.755 | 0.738 | 3.892 | 0.569 | 0.802 |
| 30 | 0.05 | 0.1 | 10.0 | COS | - | 0.787 | 2.757 | 0.738 | 3.893 | 0.569 | 0.802 |
| 30 | 0.05 | 0.1 | 10.0 | RBF | 10.0 | 0.787 | 2.757 | 0.738 | 3.893 | 0.569 | 0.802 |
| 30 | 0.05 | 0.1 | 100.0 | COS | - | 0.789 | 2.770 | 0.740 | 3.905 | 0.573 | 0.802 |
| 30 | 0.05 | 0.1 | 100.0 | RBF | 10.0 | 0.789 | 2.767 | 0.740 | 3.903 | 0.572 | 0.802 |
| 30 | 0.05 | 1.0 | 0.0 | COS | - | 0.787 | 2.755 | 0.738 | 3.892 | 0.569 | 0.802 |
| 30 | 0.05 | 1.0 | 0.0 | RBF | 10.0 | 0.787 | 2.755 | 0.738 | 3.892 | 0.569 | 0.802 |
| 30 | 0.05 | 1.0 | 1.0 | COS | - | 0.787 | 2.755 | 0.738 | 3.892 | 0.569 | 0.802 |
| 30 | 0.05 | 1.0 | 1.0 | RBF | 10.0 | 0.787 | 2.755 | 0.738 | 3.892 | 0.569 | 0.802 |
| 30 | 0.05 | 1.0 | 10.0 | COS | - | 0.787 | 2.757 | 0.738 | 3.893 | 0.569 | 0.802 |
| 30 | 0.05 | 1.0 | 10.0 | RBF | 10.0 | 0.787 | 2.757 | 0.738 | 3.893 | 0.569 | 0.802 |
| 30 | 0.05 | 1.0 | 100.0 | COS | - | 0.789 | 2.770 | 0.740 | 3.905 | 0.573 | 0.802 |
| 30 | 0.05 | 1.0 | 100.0 | RBF | 10.0 | 0.789 | 2.767 | 0.740 | 3.903 | 0.572 | 0.802 |
| 30 | 0.10 | 0.1 | 0.0 | COS | - | 0.781 | 2.724 | 0.732 | 3.866 | 0.561 | 0.803 |
| 30 | 0.10 | 0.1 | 0.0 | RBF | 10.0 | 0.781 | 2.724 | 0.732 | 3.866 | 0.561 | 0.803 |
| 30 | 0.10 | 0.1 | 1.0 | COS | - | 0.781 | 2.724 | 0.732 | 3.866 | 0.561 | 0.803 |
| 30 | 0.10 | 0.1 | 1.0 | RBF | 10.0 | 0.781 | 2.724 | 0.732 | 3.866 | 0.561 | 0.803 |
| 30 | 0.10 | 0.1 | 10.0 | COS | - | 0.781 | 2.727 | 0.732 | 3.868 | 0.561 | 0.803 |
| 30 | 0.10 | 0.1 | 10.0 | RBF | 10.0 | 0.781 | 2.727 | 0.732 | 3.868 | 0.561 | 0.803 |
| 30 | 0.10 | 0.1 | 100.0 | COS | - | 0.783 | 2.744 | 0.735 | 3.881 | 0.565 | 0.803 |
| 30 | 0.10 | 0.1 | 100.0 | RBF | 10.0 | 0.783 | 2.741 | 0.735 | 3.878 | 0.564 | 0.803 |
| 30 | 0.10 | 1.0 | 0.0 | COS | - | 0.781 | 2.724 | 0.732 | 3.866 | 0.561 | 0.803 |
| 30 | 0.10 | 1.0 | 0.0 | RBF | 10.0 | 0.781 | 2.724 | 0.732 | 3.866 | 0.561 | 0.803 |
| 30 | 0.10 | 1.0 | 1.0 | COS | - | 0.781 | 2.724 | 0.732 | 3.867 | 0.561 | 0.803 |
| 30 | 0.10 | 1.0 | 1.0 | RBF | 10.0 | 0.781 | 2.724 | 0.732 | 3.866 | 0.561 | 0.803 |
| 30 | 0.10 | 1.0 | 10.0 | COS | - | 0.781 | 2.727 | 0.732 | 3.868 | 0.561 | 0.803 |
| 30 | 0.10 | 1.0 | 10.0 | RBF | 10.0 | 0.781 | 2.727 | 0.732 | 3.868 | 0.561 | 0.803 |
| 30 | 0.10 | 1.0 | 100.0 | COS | - | 0.783 | 2.744 | 0.735 | 3.881 | 0.565 | 0.803 |
| 30 | 0.10 | 1.0 | 100.0 | RBF | 10.0 | 0.783 | 2.741 | 0.735 | 3.879 | 0.564 | 0.803 |
| 30 | 0.50 | 0.1 | 0.0 | COS | - | 0.742 | 2.444 | 0.685 | 3.556 | 0.512 | 0.810 |

Continued on next page

TABLE S7 – continued from previous page

| $l$ | $\alpha$ | $\beta$ | $\gamma$ | usim | $\sigma$ | AP@5 | AH@5 | AP@10 | AH@10 | sCI | CI |
|---|---|---|---|---|---|---|---|---|---|---|---|
| 30 | 0.50 | 0.1 | 0.0 | RBF | 10.0 | 0.742 | 2.444 | 0.685 | 3.556 | 0.512 | 0.810 |
| 30 | 0.50 | 0.1 | 1.0 | COS | - | 0.742 | 2.444 | 0.685 | 3.557 | 0.512 | 0.810 |
| 30 | 0.50 | 0.1 | 1.0 | RBF | 10.0 | 0.742 | 2.444 | 0.685 | 3.556 | 0.512 | 0.810 |
| 30 | 0.50 | 0.1 | 10.0 | COS | - | 0.742 | 2.446 | 0.685 | 3.559 | 0.513 | 0.810 |
| 30 | 0.50 | 0.1 | 10.0 | RBF | 10.0 | 0.742 | 2.446 | 0.685 | 3.559 | 0.513 | 0.810 |
| 30 | 0.50 | 0.1 | 100.0 | COS | - | 0.744 | 2.461 | 0.687 | 3.581 | 0.516 | 0.810 |
| 30 | 0.50 | 0.1 | 100.0 | RBF | 10.0 | 0.744 | 2.458 | 0.686 | 3.578 | 0.515 | 0.810 |
| 30 | 0.50 | 1.0 | 0.0 | COS | - | 0.742 | 2.444 | 0.685 | 3.557 | 0.512 | 0.810 |
| 30 | 0.50 | 1.0 | 0.0 | RBF | 10.0 | 0.742 | 2.444 | 0.685 | 3.557 | 0.512 | 0.810 |
| 30 | 0.50 | 1.0 | 1.0 | COS | - | 0.742 | 2.444 | 0.685 | 3.557 | 0.512 | 0.810 |
| 30 | 0.50 | 1.0 | 1.0 | RBF | 10.0 | 0.742 | 2.444 | 0.685 | 3.557 | 0.512 | 0.810 |
| 30 | 0.50 | 1.0 | 10.0 | COS | - | 0.742 | 2.446 | 0.685 | 3.559 | 0.513 | 0.810 |
| 30 | 0.50 | 1.0 | 10.0 | RBF | 10.0 | 0.742 | 2.446 | 0.685 | 3.559 | 0.513 | 0.810 |
| 30 | 0.50 | 1.0 | 100.0 | COS | - | 0.744 | 2.461 | 0.687 | 3.581 | 0.516 | 0.810 |
| 30 | 0.50 | 1.0 | 100.0 | RBF | 10.0 | 0.744 | 2.458 | 0.687 | 3.578 | 0.515 | 0.810 |
| 30 | 1.00 | 0.1 | 0.0 | COS | - | 0.689 | 1.996 | 0.644 | 2.697 | 0.598 | 0.633 |
| 30 | 1.00 | 0.1 | 0.0 | RBF | 10.0 | 0.689 | 1.996 | 0.644 | 2.697 | 0.598 | 0.633 |
| 30 | 1.00 | 0.1 | 1.0 | COS | - | 0.696 | 2.030 | 0.650 | 2.750 | 0.598 | 0.651 |
| 30 | 1.00 | 0.1 | 1.0 | RBF | 10.0 | 0.695 | 2.027 | 0.650 | 2.746 | 0.597 | 0.650 |
| 30 | 1.00 | 0.1 | 10.0 | COS | - | 0.730 | 2.198 | 0.680 | 2.973 | 0.642 | 0.668 |
| 30 | 1.00 | 0.1 | 10.0 | RBF | 10.0 | 0.728 | 2.177 | 0.678 | 2.954 | 0.637 | 0.667 |
| 30 | 1.00 | 0.1 | 100.0 | COS | - | 0.750 | 2.294 | 0.697 | 3.122 | 0.671 | 0.709 |
| 30 | 1.00 | 0.1 | 100.0 | RBF | 10.0 | 0.748 | 2.284 | 0.695 | 3.110 | 0.669 | 0.705 |
| 30 | 1.00 | 1.0 | 0.0 | COS | - | 0.691 | 2.007 | 0.646 | 2.715 | 0.595 | 0.643 |
| 30 | 1.00 | 1.0 | 0.0 | RBF | 10.0 | 0.691 | 2.007 | 0.646 | 2.715 | 0.595 | 0.643 |
| 30 | 1.00 | 1.0 | 1.0 | COS | - | 0.696 | 2.033 | 0.649 | 2.752 | 0.595 | 0.654 |
| 30 | 1.00 | 1.0 | 1.0 | RBF | 10.0 | 0.695 | 2.031 | 0.649 | 2.747 | 0.595 | 0.653 |
| 30 | 1.00 | 1.0 | 10.0 | COS | - | 0.726 | 2.170 | 0.677 | 2.941 | 0.634 | 0.667 |
| 30 | 1.00 | 1.0 | 10.0 | RBF | 10.0 | 0.721 | 2.161 | 0.674 | 2.926 | 0.630 | 0.667 |
| 30 | 1.00 | 1.0 | 100.0 | COS | - | 0.753 | 2.301 | 0.700 | 3.126 | 0.673 | 0.707 |
| 30 | 1.00 | 1.0 | 100.0 | RBF | 10.0 | 0.751 | 2.289 | 0.698 | 3.107 | 0.670 | 0.700 |
| 50 | 0.00 | 0.1 | 0.0 | COS | - | 0.753 | 2.566 | 0.700 | 3.725 | 0.580 | 0.799 |
| 50 | 0.00 | 0.1 | 0.0 | RBF | 10.0 | 0.753 | 2.566 | 0.700 | 3.725 | 0.580 | 0.799 |
| 50 | 0.00 | 0.1 | 1.0 | COS | - | 0.749 | 2.546 | 0.696 | 3.707 | 0.577 | 0.799 |
| 50 | 0.00 | 0.1 | 1.0 | RBF | 10.0 | 0.751 | 2.557 | 0.699 | 3.716 | 0.579 | 0.799 |
| 50 | 0.00 | 0.1 | 10.0 | COS | - | 0.739 | 2.500 | 0.686 | 3.667 | 0.571 | 0.800 |
| 50 | 0.00 | 0.1 | 10.0 | RBF | 10.0 | 0.739 | 2.500 | 0.686 | 3.667 | 0.571 | 0.800 |
| 50 | 0.00 | 0.1 | 100.0 | COS | - | 0.857 | 2.919 | 0.805 | 3.934 | 0.663 | 0.742 |
| 50 | 0.00 | 0.1 | 100.0 | RBF | 10.0 | 0.847 | 2.919 | 0.796 | 3.978 | 0.658 | 0.768 |
| 50 | 0.00 | 1.0 | 0.0 | COS | - | 0.733 | 2.469 | 0.679 | 3.646 | 0.566 | 0.801 |
| 50 | 0.00 | 1.0 | 0.0 | RBF | 10.0 | 0.733 | 2.469 | 0.679 | 3.646 | 0.566 | 0.801 |
| 50 | 0.00 | 1.0 | 1.0 | COS | - | 0.733 | 2.469 | 0.679 | 3.646 | 0.566 | 0.801 |
| 50 | 0.00 | 1.0 | 1.0 | RBF | 10.0 | 0.733 | 2.469 | 0.679 | 3.646 | 0.566 | 0.801 |
| 50 | 0.00 | 1.0 | 10.0 | COS | - | 0.733 | 2.472 | 0.679 | 3.648 | 0.567 | 0.801 |
| 50 | 0.00 | 1.0 | 10.0 | RBF | 10.0 | 0.733 | 2.472 | 0.679 | 3.648 | 0.567 | 0.801 |
| 50 | 0.00 | 1.0 | 100.0 | COS | - | 0.833 | 2.878 | 0.781 | 3.946 | 0.642 | 0.781 |
| 50 | 0.00 | 1.0 | 100.0 | RBF | 10.0 | 0.793 | 2.744 | 0.742 | 3.864 | 0.611 | 0.793 |
| 50 | 0.05 | 0.1 | 0.0 | COS | - | 0.723 | 2.425 | 0.669 | 3.603 | 0.562 | 0.802 |
| 50 | 0.05 | 0.1 | 0.0 | RBF | 10.0 | 0.723 | 2.425 | 0.669 | 3.603 | 0.562 | 0.802 |
| 50 | 0.05 | 0.1 | 1.0 | COS | - | 0.723 | 2.425 | 0.669 | 3.603 | 0.562 | 0.802 |
| 50 | 0.05 | 0.1 | 1.0 | RBF | 10.0 | 0.723 | 2.425 | 0.669 | 3.603 | 0.562 | 0.802 |
| 50 | 0.05 | 0.1 | 10.0 | COS | - | 0.724 | 2.428 | 0.670 | 3.606 | 0.563 | 0.802 |
| 50 | 0.05 | 0.1 | 10.0 | RBF | 10.0 | 0.724 | 2.428 | 0.670 | 3.605 | 0.563 | 0.802 |
| 50 | 0.05 | 0.1 | 100.0 | COS | - | 0.816 | 2.825 | 0.764 | 3.912 | 0.628 | 0.787 |
| 50 | 0.05 | 0.1 | 100.0 | RBF | 10.0 | 0.752 | 2.565 | 0.700 | 3.727 | 0.581 | 0.800 |
| 50 | 0.05 | 1.0 | 0.0 | COS | - | 0.723 | 2.425 | 0.669 | 3.603 | 0.562 | 0.802 |
| 50 | 0.05 | 1.0 | 0.0 | RBF | 10.0 | 0.723 | 2.425 | 0.669 | 3.603 | 0.562 | 0.802 |
| 50 | 0.05 | 1.0 | 1.0 | COS | - | 0.723 | 2.425 | 0.669 | 3.603 | 0.562 | 0.802 |

Continued on next page

TABLE S7 – continued from previous page

| $l$ | $\alpha$ | $\beta$ | $\gamma$ | usim | $\sigma$ | AP@5 | AH@5 | AP@10 | AH@10 | sCI | CI |
|---|---|---|---|---|---|---|---|---|---|---|---|
| 50 | 0.05 | 1.0 | 1.0 | RBF | 10.0 | 0.723 | 2.425 | 0.669 | 3.603 | 0.562 | 0.802 |
| 50 | 0.05 | 1.0 | 10.0 | COS | - | 0.724 | 2.428 | 0.670 | 3.606 | 0.563 | 0.802 |
| 50 | 0.05 | 1.0 | 10.0 | RBF | 10.0 | 0.724 | 2.428 | 0.670 | 3.606 | 0.563 | 0.802 |
| 50 | 0.05 | 1.0 | 100.0 | COS | - | 0.757 | 2.582 | 0.704 | 3.747 | 0.585 | 0.799 |
| 50 | 0.05 | 1.0 | 100.0 | RBF | 10.0 | 0.729 | 2.451 | 0.675 | 3.630 | 0.566 | 0.802 |
| 50 | 0.10 | 0.1 | 0.0 | COS | - | 0.715 | 2.382 | 0.661 | 3.555 | 0.556 | 0.802 |
| 50 | 0.10 | 0.1 | 0.0 | RBF | 10.0 | 0.715 | 2.382 | 0.661 | 3.555 | 0.556 | 0.802 |
| 50 | 0.10 | 0.1 | 1.0 | COS | - | 0.715 | 2.382 | 0.661 | 3.555 | 0.556 | 0.802 |
| 50 | 0.10 | 0.1 | 1.0 | RBF | 10.0 | 0.715 | 2.382 | 0.661 | 3.555 | 0.556 | 0.802 |
| 50 | 0.10 | 0.1 | 10.0 | COS | - | 0.715 | 2.385 | 0.662 | 3.558 | 0.556 | 0.802 |
| 50 | 0.10 | 0.1 | 10.0 | RBF | 10.0 | 0.715 | 2.384 | 0.662 | 3.558 | 0.556 | 0.802 |
| 50 | 0.10 | 0.1 | 100.0 | COS | - | 0.739 | 2.504 | 0.685 | 3.671 | 0.572 | 0.801 |
| 50 | 0.10 | 0.1 | 100.0 | RBF | 10.0 | 0.719 | 2.409 | 0.665 | 3.587 | 0.561 | 0.803 |
| 50 | 0.10 | 1.0 | 0.0 | COS | - | 0.715 | 2.382 | 0.661 | 3.555 | 0.556 | 0.802 |
| 50 | 0.10 | 1.0 | 0.0 | RBF | 10.0 | 0.715 | 2.382 | 0.661 | 3.555 | 0.556 | 0.802 |
| 50 | 0.10 | 1.0 | 1.0 | COS | - | 0.715 | 2.382 | 0.661 | 3.556 | 0.556 | 0.802 |
| 50 | 0.10 | 1.0 | 1.0 | RBF | 10.0 | 0.715 | 2.382 | 0.661 | 3.555 | 0.556 | 0.802 |
| 50 | 0.10 | 1.0 | 10.0 | COS | - | 0.715 | 2.385 | 0.662 | 3.558 | 0.556 | 0.802 |
| 50 | 0.10 | 1.0 | 10.0 | RBF | 10.0 | 0.715 | 2.384 | 0.662 | 3.558 | 0.556 | 0.802 |
| 50 | 0.10 | 1.0 | 100.0 | COS | - | 0.720 | 2.413 | 0.666 | 3.592 | 0.561 | 0.803 |
| 50 | 0.10 | 1.0 | 100.0 | RBF | 10.0 | 0.719 | 2.409 | 0.665 | 3.587 | 0.561 | 0.803 |
| 50 | 0.50 | 0.1 | 0.0 | COS | - | 0.769 | 2.574 | 0.720 | 3.573 | 0.596 | 0.711 |
| 50 | 0.50 | 0.1 | 0.0 | RBF | 10.0 | 0.769 | 2.574 | 0.720 | 3.573 | 0.596 | 0.711 |
| 50 | 0.50 | 0.1 | 1.0 | COS | - | 0.769 | 2.578 | 0.720 | 3.588 | 0.598 | 0.714 |
| 50 | 0.50 | 0.1 | 1.0 | RBF | 10.0 | 0.769 | 2.576 | 0.720 | 3.583 | 0.598 | 0.713 |
| 50 | 0.50 | 0.1 | 10.0 | COS | - | 0.673 | 2.161 | 0.620 | 3.274 | 0.527 | 0.801 |
| 50 | 0.50 | 0.1 | 10.0 | RBF | 10.0 | 0.675 | 2.171 | 0.622 | 3.286 | 0.529 | 0.801 |
| 50 | 0.50 | 0.1 | 100.0 | COS | - | 0.824 | 2.818 | 0.778 | 3.780 | 0.651 | 0.692 |
| 50 | 0.50 | 0.1 | 100.0 | RBF | 10.0 | 0.819 | 2.797 | 0.773 | 3.770 | 0.647 | 0.697 |
| 50 | 0.50 | 1.0 | 0.0 | COS | - | 0.664 | 2.108 | 0.611 | 3.205 | 0.519 | 0.802 |
| 50 | 0.50 | 1.0 | 0.0 | RBF | 10.0 | 0.664 | 2.108 | 0.611 | 3.205 | 0.519 | 0.802 |
| 50 | 0.50 | 1.0 | 1.0 | COS | - | 0.659 | 2.090 | 0.607 | 3.184 | 0.517 | 0.802 |
| 50 | 0.50 | 1.0 | 1.0 | RBF | 10.0 | 0.661 | 2.098 | 0.609 | 3.193 | 0.518 | 0.802 |
| 50 | 0.50 | 1.0 | 10.0 | COS | - | 0.654 | 2.052 | 0.601 | 3.134 | 0.511 | 0.803 |
| 50 | 0.50 | 1.0 | 10.0 | RBF | 10.0 | 0.654 | 2.053 | 0.601 | 3.133 | 0.511 | 0.803 |
| 50 | 0.50 | 1.0 | 100.0 | COS | - | 0.824 | 2.833 | 0.776 | 3.825 | 0.651 | 0.713 |
| 50 | 0.50 | 1.0 | 100.0 | RBF | 10.0 | 0.821 | 2.830 | 0.773 | 3.836 | 0.649 | 0.721 |
| 50 | 1.00 | 0.1 | 0.0 | COS | - | 0.703 | 1.983 | 0.658 | 2.601 | 0.644 | 0.644 |
| 50 | 1.00 | 0.1 | 0.0 | RBF | 10.0 | 0.703 | 1.983 | 0.658 | 2.601 | 0.644 | 0.644 |
| 50 | 1.00 | 0.1 | 1.0 | COS | - | 0.710 | 2.020 | 0.663 | 2.653 | 0.645 | 0.665 |
| 50 | 1.00 | 0.1 | 1.0 | RBF | 10.0 | 0.709 | 2.016 | 0.663 | 2.648 | 0.645 | 0.663 |
| 50 | 1.00 | 0.1 | 10.0 | COS | - | 0.770 | 2.307 | 0.718 | 3.058 | 0.681 | 0.690 |
| 50 | 1.00 | 0.1 | 10.0 | RBF | 10.0 | 0.765 | 2.292 | 0.714 | 3.038 | 0.679 | 0.688 |
| 50 | 1.00 | 0.1 | 100.0 | COS | - | 0.779 | 2.382 | 0.720 | 3.246 | 0.698 | 0.735 |
| 50 | 1.00 | 0.1 | 100.0 | RBF | 10.0 | 0.779 | 2.374 | 0.720 | 3.234 | 0.698 | 0.730 |
| 50 | 1.00 | 1.0 | 0.0 | COS | - | 0.701 | 1.971 | 0.656 | 2.588 | 0.640 | 0.655 |
| 50 | 1.00 | 1.0 | 0.0 | RBF | 10.0 | 0.701 | 1.971 | 0.656 | 2.588 | 0.640 | 0.655 |
| 50 | 1.00 | 1.0 | 1.0 | COS | - | 0.706 | 1.998 | 0.660 | 2.626 | 0.641 | 0.668 |
| 50 | 1.00 | 1.0 | 1.0 | RBF | 10.0 | 0.704 | 1.994 | 0.658 | 2.620 | 0.641 | 0.667 |
| 50 | 1.00 | 1.0 | 10.0 | COS | - | 0.761 | 2.272 | 0.710 | 2.996 | 0.676 | 0.686 |
| 50 | 1.00 | 1.0 | 10.0 | RBF | 10.0 | 0.756 | 2.250 | 0.706 | 2.971 | 0.674 | 0.684 |
| 50 | 1.00 | 1.0 | 100.0 | COS | - | 0.780 | 2.385 | 0.723 | 3.233 | 0.698 | 0.733 |
| 50 | 1.00 | 1.0 | 100.0 | RBF | 10.0 | 0.779 | 2.376 | 0.721 | 3.228 | 0.699 | 0.726 |

The columns corresponding to "$l$", "$\alpha$", "$\beta$", "$\gamma$", "usim", and "$\sigma$" have the latent dimension, weighting factor, latent vector regularization parameter, cell line similarity regularization parameter, cell line similarity function, and parameter for rbf cell line similarity, respectively, for pLETORg.

## S11 Performance on Ranking New and Known Drugs

**TABLE S8:** BMTMKL Performance on New and Known Drugs ($\theta$ = 2)

| $\alpha_b$ | $\beta_b$ | usim | $\sigma$ | AP@5 | AH@5 | AP@10 | AH@10 | AT@5% | AT@10% | NT@5% | NT@10% |
|---|---|---|---|---|---|---|---|---|---|---|---|
| 1e0 | 1e0 | RBF | 10.0 | 0.850 | 0.789 | 3.346 | 5.175 | 48.03 | 54.57 | 47.57 | 54.00 |
| 1e-10 | 1e10 | RBF | 10.0 | 0.850 | 0.789 | 3.347 | 5.174 | 48.03 | 54.55 | 47.61 | 54.00 |
| 1e-10 | 1e-10 | RBF | 10.0 | 0.849 | 0.789 | 3.343 | 5.169 | 47.99 | 54.49 | 47.62 | 54.01 |
| 1e0 | 1e0 | COS | - | 0.836 | 0.776 | 3.169 | 5.022 | 45.49 | 53.01 | 45.41 | 52.47 |
| 1e-10 | 1e10 | COS | - | 0.836 | 0.776 | 3.183 | 5.051 | 45.74 | 53.31 | 45.71 | 52.76 |
| 1e-10 | 1e-10 | COS | - | 0.834 | 0.777 | 3.176 | 5.033 | 45.54 | 53.17 | 45.65 | 52.69 |

The columns corresponding to "$\alpha_b$", "$\beta_b$", "usim", and "$\sigma$" have the two hyperparameters, cell line similarity function, and parameter for RBF cell line similarity, respectively, for BMTMKL.

**TABLE S9:** BMTMKL Performance on New and Known Drugs ($\theta$ = 5)

| $\alpha_b$ | $\beta_b$ | usim | $\sigma$ | AP@5 | AH@5 | AP@10 | AH@10 | AT@5% | AT@10% | NT@5% | NT@10% |
|---|---|---|---|---|---|---|---|---|---|---|---|
| 1e0 | 1e0 | RBF | 10.0 | 0.942 | 0.906 | 4.311 | 7.758 | 48.03 | 54.57 | 47.57 | 54.00 |
| 1e-10 | 1e10 | RBF | 10.0 | 0.942 | 0.906 | 4.312 | 7.758 | 48.03 | 54.55 | 47.61 | 54.00 |
| 1e-10 | 1e-10 | RBF | 10.0 | 0.942 | 0.906 | 4.308 | 7.756 | 47.99 | 54.49 | 47.62 | 54.01 |
| 1e0 | 1e0 | COS | - | 0.935 | 0.898 | 4.183 | 7.539 | 45.49 | 53.01 | 45.41 | 52.47 |
| 1e-10 | 1e10 | COS | - | 0.935 | 0.898 | 4.191 | 7.574 | 45.74 | 53.31 | 45.71 | 52.76 |
| 1e-10 | 1e-10 | COS | - | 0.936 | 0.900 | 4.200 | 7.551 | 45.54 | 53.17 | 45.65 | 52.69 |

The columns corresponding to "$\alpha_b$", "$\beta_b$", "usim", and "$\sigma$" have the two hyperparameters, cell line similarity function, and parameter for RBF cell line similarity, respectively, for BMTMKL.

**TABLE S10:** KRL Performance on New and Known Drugs ($\theta$ = 2)

| $k$ | $\lambda$ | usim | $\sigma$ | AP@5 | AH@5 | AP@10 | AH@10 | AT@5% | AT@10% | NT@5% | NT@10% |
|---|---|---|---|---|---|---|---|---|---|---|---|
| 10 | 0.000001 | LIN | - | 0.667 | 2.229 | 0.606 | 3.779 | 41.174 | 40.814 | 34.874 | 42.071 |
| 10 | 0.000001 | RBF | 0.0001 | 0.839 | 3.206 | 0.770 | 4.940 | 45.632 | 51.881 | 45.546 | 52.282 |
| 10 | 0.000001 | RBF | 0.001 | 0.879 | 3.591 | 0.813 | 5.745 | 55.059 | 59.932 | 43.333 | 51.916 |
| 10 | 0.000001 | RBF | 0.01 | 1.000 | 4.907 | 0.997 | 7.976 | 78.879 | 78.239 | 3.426 | 28.513 |
| 10 | 0.00001 | LIN | - | 0.714 | 2.579 | 0.647 | 4.370 | 43.566 | 46.358 | 40.638 | 46.850 |
| 10 | 0.00001 | RBF | 0.0001 | 0.839 | 3.206 | 0.770 | 4.940 | 45.632 | 51.881 | 45.546 | 52.282 |
| 10 | 0.00001 | RBF | 0.001 | 0.879 | 3.591 | 0.813 | 5.745 | 55.059 | 59.932 | 43.333 | 51.916 |
| 10 | 0.00001 | RBF | 0.01 | 1.000 | 4.906 | 0.997 | 7.957 | 78.821 | 77.973 | 3.339 | 27.476 |
| 10 | 0.0001 | LIN | - | 0.725 | 2.653 | 0.656 | 4.760 | 41.354 | 50.168 | 41.232 | 51.010 |
| 10 | 0.0001 | RBF | 0.0001 | 0.839 | 3.206 | 0.770 | 4.940 | 45.632 | 51.881 | 45.546 | 52.282 |
| 10 | 0.0001 | RBF | 0.001 | 0.879 | 3.591 | 0.813 | 5.745 | 55.059 | 59.932 | 43.333 | 51.916 |
| 10 | 0.0001 | RBF | 0.01 | 1.000 | 4.906 | 0.997 | 7.918 | 78.840 | 77.464 | 3.353 | 25.385 |
| 10 | 0.001 | LIN | - | 0.759 | 2.499 | 0.657 | 4.792 | 37.666 | 50.417 | 37.735 | 51.150 |
| 10 | 0.001 | RBF | 0.0001 | 0.839 | 3.206 | 0.770 | 4.940 | 45.632 | 51.881 | 45.546 | 52.282 |
| 10 | 0.001 | RBF | 0.001 | 0.879 | 3.591 | 0.813 | 5.745 | 55.059 | 59.932 | 43.333 | 51.916 |
| 10 | 0.001 | RBF | 0.01 | 1.000 | 4.905 | 0.998 | 7.860 | 78.801 | 76.673 | 3.280 | 22.605 |
| 10 | 0.01 | LIN | - | 0.783 | 2.664 | 0.686 | 4.831 | 39.669 | 50.853 | 40.088 | 51.364 |
| 10 | 0.01 | RBF | 0.0001 | 0.839 | 3.206 | 0.770 | 4.940 | 45.632 | 51.881 | 45.546 | 52.282 |
| 10 | 0.01 | RBF | 0.001 | 0.879 | 3.591 | 0.813 | 5.745 | 55.059 | 59.932 | 43.333 | 51.916 |
| 10 | 0.01 | RBF | 0.01 | 1.000 | 4.904 | 0.998 | 7.778 | 78.733 | 75.613 | 3.135 | 18.388 |
| 10 | 0.1 | LIN | - | 0.834 | 3.188 | 0.766 | 4.900 | 45.549 | 51.508 | 45.911 | 51.949 |
| 10 | 0.1 | RBF | 0.0001 | 0.839 | 3.206 | 0.770 | 4.940 | 45.632 | 51.881 | 45.546 | 52.282 |
| 10 | 0.1 | RBF | 0.001 | 0.879 | 3.591 | 0.813 | 5.745 | 55.059 | 59.932 | 43.333 | 51.916 |
| 10 | 0.1 | RBF | 0.01 | 1.000 | 4.904 | 0.999 | 7.700 | 78.684 | 74.512 | 3.013 | 14.353 |
| 10 | 0.2 | LIN | - | 0.834 | 3.188 | 0.764 | 4.914 | 45.559 | 51.605 | 45.947 | 51.899 |
| 10 | 0.2 | RBF | 0.0001 | 0.839 | 3.206 | 0.770 | 4.940 | 45.632 | 51.881 | 45.546 | 52.282 |
| 10 | 0.2 | RBF | 0.001 | 0.879 | 3.591 | 0.813 | 5.745 | 55.059 | 59.932 | 43.333 | 51.916 |
| 10 | 0.2 | RBF | 0.01 | 1.000 | 4.904 | 0.999 | 7.670 | 78.675 | 74.112 | 3.007 | 12.668 |
| 10 | 0.4 | LIN | - | 0.834 | 3.188 | 0.764 | 4.914 | 45.559 | 51.605 | 45.947 | 51.899 |
| 10 | 0.4 | RBF | 0.0001 | 0.839 | 3.206 | 0.770 | 4.940 | 45.632 | 51.881 | 45.546 | 52.282 |
| 10 | 0.4 | RBF | 0.001 | 0.879 | 3.591 | 0.813 | 5.745 | 55.059 | 59.932 | 43.333 | 51.916 |
| 10 | 0.4 | RBF | 0.01 | 1.000 | 4.903 | 0.999 | 7.637 | 78.650 | 73.664 | 2.927 | 11.007 |
| 10 | 0.6 | LIN | - | 0.834 | 3.188 | 0.764 | 4.914 | 45.559 | 51.605 | 45.947 | 51.899 |
| 10 | 0.6 | RBF | 0.0001 | 0.839 | 3.206 | 0.770 | 4.940 | 45.632 | 51.881 | 45.546 | 52.282 |
| 10 | 0.6 | RBF | 0.001 | 0.879 | 3.591 | 0.813 | 5.745 | 55.059 | 59.932 | 43.333 | 51.916 |
| 10 | 0.6 | RBF | 0.01 | 1.000 | 4.903 | 0.999 | 7.622 | 78.631 | 73.462 | 2.816 | 10.211 |
| 10 | 0.8 | LIN | - | 0.834 | 3.188 | 0.764 | 4.914 | 45.559 | 51.605 | 45.947 | 51.899 |
| 10 | 0.8 | RBF | 0.0001 | 0.839 | 3.206 | 0.770 | 4.940 | 45.632 | 51.881 | 45.546 | 52.282 |
| 10 | 0.8 | RBF | 0.001 | 0.879 | 3.591 | 0.813 | 5.745 | 55.059 | 59.932 | 43.333 | 51.916 |
| 10 | 0.8 | RBF | 0.01 | 1.000 | 4.902 | 0.999 | 7.614 | 78.616 | 73.320 | 2.779 | 9.660 |
| 10 | 1.0 | LIN | - | 0.834 | 3.188 | 0.764 | 4.914 | 45.559 | 51.605 | 45.947 | 51.899 |
| 10 | 1.0 | RBF | 0.0001 | 0.839 | 3.206 | 0.770 | 4.940 | 45.632 | 51.881 | 45.546 | 52.282 |
| 10 | 1.0 | RBF | 0.001 | 0.879 | 3.591 | 0.813 | 5.745 | 55.059 | 59.932 | 43.333 | 51.916 |
| 10 | 1.0 | RBF | 0.01 | 1.000 | 4.902 | 0.999 | 7.602 | 78.616 | 73.199 | 2.757 | 9.093 |
| 10 | 10 | LIN | - | 0.834 | 3.190 | 0.768 | 4.903 | 45.617 | 51.496 | 45.939 | 51.779 |
| 10 | 10 | RBF | 0.0001 | 0.839 | 3.206 | 0.770 | 4.940 | 45.632 | 51.881 | 45.546 | 52.282 |
| 10 | 10 | RBF | 0.001 | 0.879 | 3.591 | 0.813 | 5.745 | 55.059 | 59.932 | 43.333 | 51.916 |
| 10 | 10 | RBF | 0.01 | 1.000 | 4.900 | 0.999 | 7.551 | 78.533 | 72.512 | 2.500 | 6.188 |
| 10 | 50 | LIN | - | 0.835 | 3.190 | 0.770 | 4.896 | 45.637 | 51.440 | 45.993 | 51.818 |
| 10 | 50 | RBF | 0.0001 | 0.839 | 3.206 | 0.770 | 4.940 | 45.632 | 51.881 | 45.546 | 52.282 |
| 10 | 50 | RBF | 0.001 | 0.879 | 3.591 | 0.813 | 5.745 | 55.059 | 59.937 | 43.333 | 51.916 |
| 10 | 50 | RBF | 0.01 | 1.000 | 4.900 | 0.999 | 7.530 | 78.514 | 72.249 | 2.495 | 5.103 |
| 10 | 100 | LIN | - | 0.835 | 3.190 | 0.770 | 4.896 | 45.637 | 51.440 | 45.993 | 51.809 |
| 10 | 100 | RBF | 0.0001 | 0.839 | 3.206 | 0.770 | 4.940 | 45.632 | 51.881 | 45.546 | 52.282 |
| 10 | 100 | RBF | 0.001 | 0.879 | 3.591 | 0.813 | 5.745 | 55.059 | 59.932 | 43.333 | 51.916 |
| 10 | 100 | RBF | 0.01 | 1.000 | 4.901 | 0.999 | 7.524 | 78.524 | 72.173 | 2.507 | 4.812 |

The columns corresponding to "$k$", "$\lambda$", "usim", and "$\sigma$" have the two hyperparameters, cell line similarity function, and parameter for RBF cell line similarity, respectively, for KRL.

**TABLE S11:** KRL Performance on New and Known Drugs ($\theta$ = 5)

| $k$ | $\lambda$ | usim | $\sigma$ | AP@5 | AH@5 | AP@10 | AH@10 | AT@5% | AT@10% | NT@5% | NT@10% |
|---|---|---|---|---|---|---|---|---|---|---|---|
| 10 | 0.000001 | LIN | - | 0.780 | 3.012 | 0.714 | 5.435 | 48.010 | 47.781 | 36.423 | 41.896 |
| 10 | 0.000001 | RBF | 0.0001 | 0.929 | 4.208 | 0.890 | 7.155 | 45.998 | 52.660 | 45.952 | 53.290 |
| 10 | 0.000001 | RBF | 0.001 | 0.952 | 4.359 | 0.912 | 7.981 | 52.736 | 60.151 | 42.330 | 50.277 |
| 10 | 0.000001 | RBF | 0.01 | 1.000 | 4.970 | 1.000 | 9.833 | 75.971 | 75.065 | 2.641 | 4.135 |
| 10 | 0.00001 | LIN | - | 0.876 | 3.838 | 0.832 | 6.938 | 53.910 | 56.543 | 46.293 | 52.328 |
| 10 | 0.00001 | RBF | 0.0001 | 0.930 | 4.201 | 0.886 | 7.008 | 44.317 | 50.536 | 44.652 | 50.761 |
| 10 | 0.00001 | RBF | 0.001 | 0.952 | 4.359 | 0.912 | 7.981 | 52.736 | 60.151 | 42.330 | 50.277 |
| 10 | 0.00001 | RBF | 0.01 | 1.000 | 4.969 | 1.000 | 9.831 | 75.947 | 75.009 | 2.581 | 4.024 |
| 10 | 0.0001 | LIN | - | 0.894 | 3.935 | 0.849 | 7.211 | 48.254 | 54.543 | 46.424 | 54.512 |
| 10 | 0.0001 | RBF | 0.0001 | 0.930 | 4.201 | 0.886 | 7.008 | 44.317 | 50.536 | 44.652 | 50.761 |
| 10 | 0.0001 | RBF | 0.001 | 0.952 | 4.359 | 0.912 | 7.981 | 52.736 | 60.151 | 42.330 | 50.277 |
| 10 | 0.0001 | RBF | 0.01 | 1.000 | 4.969 | 1.000 | 9.831 | 75.947 | 74.984 | 2.581 | 3.997 |
| 10 | 0.001 | LIN | - | 0.909 | 3.926 | 0.851 | 7.077 | 45.325 | 52.533 | 45.740 | 52.935 |
| 10 | 0.001 | RBF | 0.0001 | 0.930 | 4.201 | 0.886 | 7.008 | 44.317 | 50.536 | 44.652 | 50.761 |
| 10 | 0.001 | RBF | 0.001 | 0.952 | 4.359 | 0.912 | 7.981 | 52.736 | 60.151 | 42.330 | 50.277 |
| 10 | 0.001 | RBF | 0.01 | 1.000 | 4.969 | 1.000 | 9.829 | 75.942 | 74.940 | 2.581 | 3.911 |
| 10 | 0.01 | LIN | - | 0.912 | 4.062 | 0.856 | 7.078 | 45.949 | 52.297 | 46.278 | 52.690 |
| 10 | 0.01 | RBF | 0.0001 | 0.930 | 4.201 | 0.886 | 7.008 | 44.317 | 50.536 | 44.652 | 50.761 |
| 10 | 0.01 | RBF | 0.001 | 0.952 | 4.359 | 0.912 | 7.981 | 52.736 | 60.151 | 42.330 | 50.277 |
| 10 | 0.01 | RBF | 0.01 | 1.000 | 4.968 | 1.000 | 9.827 | 75.927 | 74.904 | 2.544 | 3.768 |
| 10 | 0.1 | LIN | - | 0.929 | 4.201 | 0.886 | 7.111 | 45.657 | 52.224 | 45.475 | 52.227 |
| 10 | 0.1 | RBF | 0.0001 | 0.930 | 4.201 | 0.886 | 7.008 | 44.317 | 50.536 | 44.652 | 50.761 |
| 10 | 0.1 | RBF | 0.001 | 0.952 | 4.359 | 0.912 | 7.981 | 52.736 | 60.151 | 42.330 | 50.277 |
| 10 | 0.1 | RBF | 0.01 | 1.000 | 4.968 | 1.000 | 9.824 | 75.917 | 74.826 | 2.509 | 3.615 |
| 10 | 0.2 | LIN | - | 0.929 | 4.184 | 0.888 | 7.033 | 45.418 | 51.640 | 45.607 | 52.131 |
| 10 | 0.2 | RBF | 0.0001 | 0.930 | 4.201 | 0.886 | 7.008 | 44.317 | 50.536 | 44.652 | 50.761 |
| 10 | 0.2 | RBF | 0.001 | 0.952 | 4.359 | 0.912 | 7.981 | 52.736 | 60.151 | 42.330 | 50.277 |
| 10 | 0.2 | RBF | 0.01 | 1.000 | 4.968 | 1.000 | 9.824 | 75.917 | 74.814 | 2.509 | 3.572 |
| 10 | 0.4 | LIN | - | 0.929 | 4.197 | 0.885 | 6.957 | 44.258 | 50.219 | 44.613 | 50.574 |
| 10 | 0.4 | RBF | 0.0001 | 0.930 | 4.201 | 0.886 | 7.008 | 44.317 | 50.536 | 44.652 | 50.761 |
| 10 | 0.4 | RBF | 0.001 | 0.952 | 4.359 | 0.912 | 7.981 | 52.736 | 60.151 | 42.330 | 50.277 |
| 10 | 0.4 | RBF | 0.01 | 1.000 | 4.968 | 1.000 | 9.823 | 75.922 | 74.814 | 2.509 | 3.559 |
| 10 | 0.6 | LIN | - | 0.929 | 4.197 | 0.885 | 6.925 | 44.253 | 49.737 | 44.613 | 50.098 |
| 10 | 0.6 | RBF | 0.0001 | 0.930 | 4.201 | 0.886 | 7.008 | 44.317 | 50.536 | 44.652 | 50.761 |
| 10 | 0.6 | RBF | 0.001 | 0.952 | 4.359 | 0.912 | 7.981 | 52.736 | 60.151 | 42.330 | 50.277 |
| 10 | 0.6 | RBF | 0.01 | 1.000 | 4.967 | 1.000 | 9.823 | 75.912 | 74.787 | 2.397 | 3.495 |
| 10 | 0.8 | LIN | - | 0.929 | 4.197 | 0.885 | 6.925 | 44.253 | 49.737 | 44.613 | 50.098 |
| 10 | 0.8 | RBF | 0.0001 | 0.930 | 4.201 | 0.886 | 7.008 | 44.317 | 50.536 | 44.652 | 50.761 |
| 10 | 0.8 | RBF | 0.001 | 0.952 | 4.359 | 0.912 | 7.981 | 52.736 | 60.151 | 42.330 | 50.277 |
| 10 | 0.8 | RBF | 0.01 | 1.000 | 4.967 | 1.000 | 9.822 | 75.902 | 74.767 | 2.362 | 3.465 |
| 10 | 1.0 | LIN | - | 0.929 | 4.197 | 0.885 | 6.925 | 44.253 | 49.737 | 44.613 | 50.098 |
| 10 | 1.0 | RBF | 0.0001 | 0.930 | 4.201 | 0.886 | 7.008 | 44.317 | 50.536 | 44.652 | 50.761 |
| 10 | 1.0 | RBF | 0.001 | 0.952 | 4.359 | 0.912 | 7.981 | 52.736 | 60.151 | 42.330 | 50.277 |
| 10 | 1.0 | RBF | 0.01 | 1.000 | 4.967 | 1.000 | 9.823 | 75.907 | 74.746 | 2.362 | 3.451 |
| 10 | 10 | LIN | - | 0.929 | 4.197 | 0.885 | 6.925 | 44.253 | 49.737 | 44.613 | 50.098 |
| 10 | 10 | RBF | 0.0001 | 0.930 | 4.201 | 0.886 | 7.008 | 44.317 | 50.536 | 44.652 | 50.761 |
| 10 | 10 | RBF | 0.001 | 0.952 | 4.359 | 0.912 | 7.981 | 52.736 | 60.151 | 42.330 | 50.277 |
| 10 | 10 | RBF | 0.01 | 1.000 | 4.966 | 1.000 | 9.820 | 75.854 | 74.667 | 2.241 | 3.203 |
| 10 | 50 | LIN | - | 0.929 | 4.197 | 0.885 | 6.925 | 44.253 | 49.737 | 44.613 | 50.098 |
| 10 | 50 | RBF | 0.0001 | 0.930 | 4.201 | 0.886 | 7.008 | 44.317 | 50.536 | 44.652 | 50.761 |
| 10 | 50 | RBF | 0.001 | 0.952 | 4.359 | 0.912 | 7.981 | 52.736 | 60.154 | 42.330 | 50.277 |
| 10 | 50 | RBF | 0.01 | 1.000 | 4.965 | 1.000 | 9.819 | 75.830 | 74.668 | 2.101 | 3.122 |
| 10 | 100 | LIN | - | 0.929 | 4.197 | 0.885 | 6.925 | 44.253 | 49.737 | 44.613 | 50.098 |
| 10 | 100 | RBF | 0.0001 | 0.930 | 4.201 | 0.886 | 7.008 | 44.317 | 50.536 | 44.652 | 50.761 |
| 10 | 100 | RBF | 0.001 | 0.952 | 4.359 | 0.912 | 7.981 | 52.736 | 60.151 | 42.330 | 50.277 |
| 10 | 100 | RBF | 0.01 | 1.000 | 4.965 | 1.000 | 9.819 | 75.820 | 74.672 | 2.101 | 3.156 |

The columns corresponding to "$k$", "$\lambda$", "usim", and "$\sigma$" have the two hyperparameters, cell line similarity function, and parameter for RBF cell line similarity, respectively, for KRL.

**TABLE S12:** `pLETORg` Performance on New and Known Drugs ($\theta$ = 2)

| $l$ | $\alpha$ | $\beta$ | $\gamma$ | usim | $\sigma$ | AP@5 | AH@5 | AP@10 | AH@10 | AT@5% | AT@10% | NT@5% | NT@10% |
|---|---|---|---|---|---|---|---|---|---|---|---|---|---|
| 5 | 0.0 | 0.1 | 0.0 | COS | - | 0.861 | 3.407 | 0.794 | 5.538 | 49.466 | 58.356 | 46.393 | 55.579 |
| 5 | 0.0 | 0.1 | 0.0 | RBF | 10.0 | 0.861 | 3.407 | 0.794 | 5.538 | 49.466 | 58.356 | 46.393 | 55.579 |
| 5 | 0.0 | 0.1 | 1.0 | COS | - | 0.861 | 3.407 | 0.794 | 5.538 | 49.466 | 58.358 | 46.393 | 55.588 |
| 5 | 0.0 | 0.1 | 1.0 | RBF | 10.0 | 0.861 | 3.407 | 0.794 | 5.538 | 49.466 | 58.358 | 46.393 | 55.588 |
| 5 | 0.0 | 0.1 | 10.0 | COS | - | 0.861 | 3.407 | 0.794 | 5.539 | 49.457 | 58.368 | 46.393 | 55.601 |
| 5 | 0.0 | 0.1 | 10.0 | RBF | 10.0 | 0.861 | 3.407 | 0.794 | 5.539 | 49.457 | 58.368 | 46.393 | 55.601 |
| 5 | 0.0 | 0.1 | 100.0 | COS | - | 0.861 | 3.407 | 0.794 | 5.543 | 49.452 | 58.385 | 46.382 | 55.523 |
| 5 | 0.0 | 0.1 | 100.0 | RBF | 10.0 | 0.861 | 3.406 | 0.794 | 5.543 | 49.457 | 58.400 | 46.382 | 55.555 |
| 5 | 0.0 | 1.0 | 0.0 | COS | - | 0.861 | 3.408 | 0.794 | 5.545 | 49.486 | 58.419 | 46.340 | 55.551 |
| 5 | 0.0 | 1.0 | 0.0 | RBF | 10.0 | 0.861 | 3.408 | 0.794 | 5.545 | 49.486 | 58.419 | 46.340 | 55.551 |
| 5 | 0.0 | 1.0 | 1.0 | COS | - | 0.861 | 3.408 | 0.794 | 5.545 | 49.486 | 58.419 | 46.340 | 55.551 |
| 5 | 0.0 | 1.0 | 1.0 | RBF | 10.0 | 0.861 | 3.408 | 0.794 | 5.545 | 49.486 | 58.419 | 46.340 | 55.551 |
| 5 | 0.0 | 1.0 | 10.0 | COS | - | 0.904 | 3.747 | 0.844 | 5.813 | 54.616 | 61.174 | 28.122 | 34.103 |
| 5 | 0.0 | 1.0 | 10.0 | RBF | 10.0 | 0.904 | 3.747 | 0.844 | 5.813 | 54.616 | 61.174 | 28.122 | 34.103 |
| 5 | 0.0 | 1.0 | 100.0 | COS | - | 0.861 | 3.407 | 0.794 | 5.543 | 49.452 | 58.382 | 46.382 | 55.523 |
| 5 | 0.0 | 1.0 | 100.0 | RBF | 10.0 | 0.861 | 3.406 | 0.794 | 5.543 | 49.457 | 58.400 | 46.382 | 55.555 |
| 5 | 0.05 | 0.1 | 0.0 | COS | - | 0.896 | 3.646 | 0.830 | 5.718 | 58.329 | 60.875 | 29.102 | 36.774 |
| 5 | 0.05 | 0.1 | 0.0 | RBF | 10.0 | 0.896 | 3.646 | 0.830 | 5.718 | 58.329 | 60.875 | 29.102 | 36.774 |
| 5 | 0.05 | 0.1 | 1.0 | COS | - | 0.896 | 3.646 | 0.830 | 5.717 | 58.329 | 60.875 | 29.115 | 36.801 |
| 5 | 0.05 | 0.1 | 1.0 | RBF | 10.0 | 0.896 | 3.646 | 0.830 | 5.717 | 58.329 | 60.875 | 29.115 | 36.787 |
| 5 | 0.05 | 0.1 | 10.0 | COS | - | 0.895 | 3.644 | 0.830 | 5.717 | 58.295 | 60.862 | 29.152 | 36.910 |
| 5 | 0.05 | 0.1 | 10.0 | RBF | 10.0 | 0.896 | 3.644 | 0.830 | 5.717 | 58.300 | 60.870 | 29.152 | 36.910 |
| 5 | 0.05 | 0.1 | 100.0 | COS | - | 0.892 | 3.613 | 0.825 | 5.698 | 57.822 | 60.626 | 30.146 | 38.156 |
| 5 | 0.05 | 0.1 | 100.0 | RBF | 10.0 | 0.892 | 3.617 | 0.825 | 5.704 | 57.890 | 60.714 | 30.017 | 38.035 |
| 5 | 0.05 | 1.0 | 0.0 | COS | - | 0.896 | 3.651 | 0.831 | 5.727 | 58.197 | 60.977 | 28.814 | 36.231 |
| 5 | 0.05 | 1.0 | 0.0 | RBF | 10.0 | 0.896 | 3.651 | 0.831 | 5.727 | 58.197 | 60.977 | 28.814 | 36.231 |
| 5 | 0.05 | 1.0 | 1.0 | COS | - | 0.896 | 3.650 | 0.831 | 5.725 | 58.178 | 60.965 | 28.807 | 36.147 |
| 5 | 0.05 | 1.0 | 1.0 | RBF | 10.0 | 0.896 | 3.650 | 0.831 | 5.725 | 58.178 | 60.962 | 28.807 | 36.175 |
| 5 | 0.05 | 1.0 | 10.0 | COS | - | 0.897 | 3.654 | 0.831 | 5.727 | 58.076 | 60.958 | 28.708 | 35.768 |
| 5 | 0.05 | 1.0 | 10.0 | RBF | 10.0 | 0.896 | 3.654 | 0.831 | 5.728 | 58.085 | 60.962 | 28.708 | 35.823 |
| 5 | 0.05 | 1.0 | 100.0 | COS | - | 0.892 | 3.620 | 0.826 | 5.704 | 57.837 | 60.690 | 29.915 | 37.625 |
| 5 | 0.05 | 1.0 | 100.0 | RBF | 10.0 | 0.894 | 3.634 | 0.828 | 5.710 | 57.837 | 60.753 | 29.122 | 36.714 |
| 5 | 0.1 | 0.1 | 0.0 | COS | - | 0.861 | 3.415 | 0.795 | 5.550 | 49.842 | 58.499 | 46.536 | 55.614 |
| 5 | 0.1 | 0.1 | 0.0 | RBF | 10.0 | 0.861 | 3.415 | 0.795 | 5.550 | 49.842 | 58.499 | 46.536 | 55.614 |
| 5 | 0.1 | 0.1 | 1.0 | COS | - | 0.861 | 3.415 | 0.795 | 5.550 | 49.842 | 58.495 | 46.536 | 55.614 |
| 5 | 0.1 | 0.1 | 1.0 | RBF | 10.0 | 0.861 | 3.415 | 0.795 | 5.550 | 49.842 | 58.495 | 46.536 | 55.614 |
| 5 | 0.1 | 0.1 | 10.0 | COS | - | 0.861 | 3.414 | 0.795 | 5.550 | 49.842 | 58.504 | 46.554 | 55.614 |
| 5 | 0.1 | 0.1 | 10.0 | RBF | 10.0 | 0.861 | 3.414 | 0.795 | 5.550 | 49.837 | 58.502 | 46.536 | 55.614 |
| 5 | 0.1 | 0.1 | 100.0 | COS | - | 0.861 | 3.413 | 0.795 | 5.547 | 49.837 | 58.463 | 46.645 | 55.572 |
| 5 | 0.1 | 0.1 | 100.0 | RBF | 10.0 | 0.861 | 3.413 | 0.795 | 5.548 | 49.841 | 58.468 | 46.645 | 55.577 |
| 5 | 0.1 | 1.0 | 0.0 | COS | - | 0.861 | 3.415 | 0.795 | 5.550 | 49.842 | 58.499 | 46.536 | 55.614 |
| 5 | 0.1 | 1.0 | 0.0 | RBF | 10.0 | 0.861 | 3.415 | 0.795 | 5.550 | 49.842 | 58.499 | 46.536 | 55.614 |
| 5 | 0.1 | 1.0 | 1.0 | COS | - | 0.861 | 3.415 | 0.795 | 5.550 | 49.842 | 58.497 | 46.554 | 55.614 |
| 5 | 0.1 | 1.0 | 1.0 | RBF | 10.0 | 0.861 | 3.415 | 0.795 | 5.550 | 49.842 | 58.497 | 46.554 | 55.614 |
| 5 | 0.1 | 1.0 | 10.0 | COS | - | 0.861 | 3.414 | 0.795 | 5.550 | 49.842 | 58.504 | 46.554 | 55.614 |
| 5 | 0.1 | 1.0 | 10.0 | RBF | 10.0 | 0.861 | 3.414 | 0.795 | 5.550 | 49.837 | 58.502 | 46.536 | 55.614 |
| 5 | 0.1 | 1.0 | 100.0 | COS | - | 0.861 | 3.413 | 0.795 | 5.547 | 49.837 | 58.460 | 46.645 | 55.572 |
| 5 | 0.1 | 1.0 | 100.0 | RBF | 10.0 | 0.861 | 3.413 | 0.795 | 5.548 | 49.841 | 58.468 | 46.645 | 55.577 |
| 5 | 0.5 | 0.1 | 0.0 | COS | - | 0.861 | 3.427 | 0.796 | 5.554 | 50.996 | 58.573 | 45.824 | 55.035 |
| 5 | 0.5 | 0.1 | 0.0 | RBF | 10.0 | 0.861 | 3.427 | 0.796 | 5.554 | 50.996 | 58.573 | 45.824 | 55.035 |
| 5 | 0.5 | 0.1 | 1.0 | COS | - | 0.861 | 3.427 | 0.796 | 5.554 | 51.001 | 58.575 | 45.824 | 55.048 |
| 5 | 0.5 | 0.1 | 1.0 | RBF | 10.0 | 0.861 | 3.427 | 0.796 | 5.554 | 51.001 | 58.575 | 45.824 | 55.048 |
| 5 | 0.5 | 0.1 | 10.0 | COS | - | 0.861 | 3.426 | 0.796 | 5.555 | 51.001 | 58.580 | 45.861 | 55.051 |
| 5 | 0.5 | 0.1 | 10.0 | RBF | 10.0 | 0.861 | 3.426 | 0.796 | 5.555 | 50.996 | 58.577 | 45.861 | 55.051 |
| 5 | 0.5 | 0.1 | 100.0 | COS | - | 0.862 | 3.424 | 0.796 | 5.552 | 50.943 | 58.548 | 45.826 | 54.928 |
| 5 | 0.5 | 0.1 | 100.0 | RBF | 10.0 | 0.862 | 3.425 | 0.796 | 5.554 | 50.957 | 58.563 | 45.826 | 54.972 |
| 5 | 0.5 | 1.0 | 0.0 | COS | - | 0.861 | 3.427 | 0.796 | 5.554 | 51.001 | 58.575 | 45.824 | 55.048 |

Continued on next page

TABLE S12 – continued from previous page

| $l$ | $\alpha$ | $\beta$ | $\gamma$ | usim | $\sigma$ | AP@5 | AH@5 | AP@10 | AH@10 | AT@5% | AT@10% | NT@5% | NT@10% |
|---|---|---|---|---|---|---|---|---|---|---|---|---|---|
| 5 | 0.5 | 1.0 | 0.0 | RBF | 10.0 | 0.861 | 3.427 | 0.796 | 5.554 | 51.001 | 58.575 | 45.824 | 55.048 |
| 5 | 0.5 | 1.0 | 1.0 | COS | - | 0.861 | 3.427 | 0.796 | 5.554 | 51.001 | 58.575 | 45.824 | 55.048 |
| 5 | 0.5 | 1.0 | 1.0 | RBF | 10.0 | 0.861 | 3.427 | 0.796 | 5.554 | 51.001 | 58.575 | 45.824 | 55.048 |
| 5 | 0.5 | 1.0 | 10.0 | COS | - | 0.861 | 3.426 | 0.796 | 5.555 | 51.001 | 58.580 | 45.861 | 55.051 |
| 5 | 0.5 | 1.0 | 10.0 | RBF | 10.0 | 0.861 | 3.426 | 0.796 | 5.555 | 50.996 | 58.582 | 45.861 | 55.051 |
| 5 | 0.5 | 1.0 | 100.0 | COS | - | 0.862 | 3.424 | 0.796 | 5.552 | 50.943 | 58.546 | 45.826 | 54.928 |
| 5 | 0.5 | 1.0 | 100.0 | RBF | 10.0 | 0.862 | 3.425 | 0.796 | 5.554 | 50.953 | 58.563 | 45.826 | 54.972 |
| 5 | 1.0 | 0.1 | 0.0 | COS | - | 0.619 | 2.042 | 0.573 | 3.189 | 37.998 | 34.319 | 31.936 | 33.519 |
| 5 | 1.0 | 0.1 | 0.0 | RBF | 10.0 | 0.619 | 2.042 | 0.573 | 3.189 | 37.998 | 34.319 | 31.936 | 33.519 |
| 5 | 1.0 | 0.1 | 1.0 | COS | - | 0.627 | 2.070 | 0.580 | 3.222 | 38.499 | 34.718 | 32.466 | 33.688 |
| 5 | 1.0 | 0.1 | 1.0 | RBF | 10.0 | 0.621 | 2.043 | 0.574 | 3.192 | 37.988 | 34.402 | 32.023 | 33.467 |
| 5 | 1.0 | 0.1 | 10.0 | COS | - | 0.640 | 2.146 | 0.592 | 3.317 | 39.956 | 35.727 | 32.980 | 34.300 |
| 5 | 1.0 | 0.1 | 10.0 | RBF | 10.0 | 0.640 | 2.139 | 0.590 | 3.311 | 39.849 | 35.656 | 32.944 | 34.190 |
| 5 | 1.0 | 0.1 | 100.0 | COS | - | 0.670 | 2.294 | 0.619 | 3.552 | 42.631 | 38.202 | 34.129 | 37.010 |
| 5 | 1.0 | 0.1 | 100.0 | RBF | 10.0 | 0.679 | 2.355 | 0.627 | 3.629 | 43.810 | 39.023 | 34.904 | 37.408 |
| 5 | 1.0 | 1.0 | 0.0 | COS | - | 0.629 | 2.082 | 0.582 | 3.244 | 38.748 | 34.938 | 32.490 | 33.864 |
| 5 | 1.0 | 1.0 | 0.0 | RBF | 10.0 | 0.629 | 2.082 | 0.582 | 3.244 | 38.748 | 34.938 | 32.490 | 33.864 |
| 5 | 1.0 | 1.0 | 1.0 | COS | - | 0.631 | 2.092 | 0.583 | 3.253 | 38.938 | 35.035 | 32.550 | 33.926 |
| 5 | 1.0 | 1.0 | 1.0 | RBF | 10.0 | 0.628 | 2.076 | 0.580 | 3.236 | 38.650 | 34.836 | 32.410 | 33.827 |
| 5 | 1.0 | 1.0 | 10.0 | COS | - | 0.646 | 2.166 | 0.596 | 3.355 | 40.365 | 36.127 | 33.062 | 34.737 |
| 5 | 1.0 | 1.0 | 10.0 | RBF | 10.0 | 0.642 | 2.149 | 0.593 | 3.322 | 40.015 | 35.793 | 32.957 | 34.575 |
| 5 | 1.0 | 1.0 | 100.0 | COS | - | 0.669 | 2.302 | 0.619 | 3.552 | 42.777 | 38.202 | 34.473 | 36.991 |
| 5 | 1.0 | 1.0 | 100.0 | RBF | 10.0 | 0.680 | 2.356 | 0.628 | 3.635 | 43.820 | 39.084 | 34.737 | 37.409 |
| 10 | 0.0 | 0.1 | 0.0 | COS | - | 0.885 | 3.612 | 0.821 | 5.795 | 52.892 | 60.999 | 38.648 | 52.046 |
| 10 | 0.0 | 0.1 | 0.0 | RBF | 10.0 | 0.885 | 3.612 | 0.821 | 5.795 | 52.892 | 60.999 | 38.648 | 52.046 |
| 10 | 0.0 | 0.1 | 1.0 | COS | - | 0.885 | 3.612 | 0.821 | 5.795 | 52.887 | 60.999 | 38.648 | 52.051 |
| 10 | 0.0 | 0.1 | 1.0 | RBF | 10.0 | 0.885 | 3.612 | 0.821 | 5.795 | 52.887 | 60.999 | 38.648 | 52.046 |
| 10 | 0.0 | 0.1 | 10.0 | COS | - | 0.885 | 3.612 | 0.821 | 5.796 | 52.887 | 61.011 | 38.704 | 52.103 |
| 10 | 0.0 | 0.1 | 10.0 | RBF | 10.0 | 0.885 | 3.612 | 0.821 | 5.796 | 52.892 | 61.008 | 38.667 | 52.097 |
| 10 | 0.0 | 0.1 | 100.0 | COS | - | 0.882 | 3.591 | 0.819 | 5.777 | 52.609 | 60.740 | 40.469 | 53.495 |
| 10 | 0.0 | 0.1 | 100.0 | RBF | 10.0 | 0.883 | 3.596 | 0.819 | 5.785 | 52.667 | 60.836 | 39.903 | 53.061 |
| 10 | 0.0 | 1.0 | 0.0 | COS | - | 0.885 | 3.614 | 0.821 | 5.798 | 52.862 | 61.050 | 37.776 | 51.578 |
| 10 | 0.0 | 1.0 | 0.0 | RBF | 10.0 | 0.885 | 3.614 | 0.821 | 5.798 | 52.862 | 61.050 | 37.776 | 51.578 |
| 10 | 0.0 | 1.0 | 1.0 | COS | - | 0.885 | 3.614 | 0.821 | 5.798 | 52.862 | 61.050 | 37.813 | 51.578 |
| 10 | 0.0 | 1.0 | 1.0 | RBF | 10.0 | 0.885 | 3.614 | 0.821 | 5.798 | 52.862 | 61.050 | 37.813 | 51.578 |
| 10 | 0.0 | 1.0 | 10.0 | COS | - | 0.885 | 3.615 | 0.821 | 5.798 | 52.867 | 61.057 | 37.849 | 51.576 |
| 10 | 0.0 | 1.0 | 10.0 | RBF | 10.0 | 0.885 | 3.615 | 0.821 | 5.798 | 52.867 | 61.052 | 37.849 | 51.569 |
| 10 | 0.0 | 1.0 | 100.0 | COS | - | 0.886 | 3.613 | 0.821 | 5.796 | 52.867 | 61.026 | 38.033 | 51.753 |
| 10 | 0.0 | 1.0 | 100.0 | RBF | 10.0 | 0.885 | 3.613 | 0.821 | 5.795 | 52.862 | 61.021 | 37.991 | 51.713 |
| 10 | 0.05 | 0.1 | 0.0 | COS | - | 0.885 | 3.619 | 0.821 | 5.806 | 53.096 | 61.140 | 36.961 | 51.283 |
| 10 | 0.05 | 0.1 | 0.0 | RBF | 10.0 | 0.885 | 3.619 | 0.821 | 5.806 | 53.096 | 61.140 | 36.961 | 51.283 |
| 10 | 0.05 | 0.1 | 1.0 | COS | - | 0.885 | 3.619 | 0.821 | 5.806 | 53.101 | 61.143 | 36.961 | 51.292 |
| 10 | 0.05 | 0.1 | 1.0 | RBF | 10.0 | 0.885 | 3.619 | 0.821 | 5.806 | 53.101 | 61.143 | 36.961 | 51.292 |
| 10 | 0.05 | 0.1 | 10.0 | COS | - | 0.885 | 3.619 | 0.821 | 5.805 | 53.101 | 61.138 | 36.960 | 51.310 |
| 10 | 0.05 | 0.1 | 10.0 | RBF | 10.0 | 0.885 | 3.619 | 0.821 | 5.806 | 53.106 | 61.140 | 36.978 | 51.310 |
| 10 | 0.05 | 0.1 | 100.0 | COS | - | 0.885 | 3.616 | 0.821 | 5.801 | 53.048 | 61.101 | 37.251 | 51.345 |
| 10 | 0.05 | 0.1 | 100.0 | RBF | 10.0 | 0.885 | 3.618 | 0.821 | 5.803 | 53.077 | 61.111 | 37.227 | 51.332 |
| 10 | 0.05 | 1.0 | 0.0 | COS | - | 0.885 | 3.619 | 0.821 | 5.806 | 53.096 | 61.143 | 36.961 | 51.292 |
| 10 | 0.05 | 1.0 | 0.0 | RBF | 10.0 | 0.885 | 3.619 | 0.821 | 5.806 | 53.096 | 61.143 | 36.961 | 51.292 |
| 10 | 0.05 | 1.0 | 1.0 | COS | - | 0.885 | 3.619 | 0.821 | 5.806 | 53.101 | 61.143 | 36.961 | 51.292 |
| 10 | 0.05 | 1.0 | 1.0 | RBF | 10.0 | 0.885 | 3.619 | 0.821 | 5.806 | 53.101 | 61.143 | 36.961 | 51.292 |
| 10 | 0.05 | 1.0 | 10.0 | COS | - | 0.885 | 3.619 | 0.821 | 5.805 | 53.101 | 61.138 | 36.960 | 51.310 |
| 10 | 0.05 | 1.0 | 10.0 | RBF | 10.0 | 0.885 | 3.619 | 0.821 | 5.806 | 53.101 | 61.140 | 36.960 | 51.310 |
| 10 | 0.05 | 1.0 | 100.0 | COS | - | 0.885 | 3.616 | 0.821 | 5.801 | 53.048 | 61.101 | 37.251 | 51.345 |
| 10 | 0.05 | 1.0 | 100.0 | RBF | 10.0 | 0.885 | 3.617 | 0.821 | 5.803 | 53.077 | 61.111 | 37.227 | 51.332 |
| 10 | 0.1 | 0.1 | 0.0 | COS | - | 0.885 | 3.624 | 0.822 | 5.811 | 53.330 | 61.167 | 36.770 | 50.787 |
| 10 | 0.1 | 0.1 | 0.0 | RBF | 10.0 | 0.885 | 3.624 | 0.822 | 5.811 | 53.330 | 61.167 | 36.770 | 50.787 |
| 10 | 0.1 | 0.1 | 1.0 | COS | - | 0.885 | 3.624 | 0.822 | 5.811 | 53.325 | 61.167 | 36.770 | 50.787 |

Continued on next page

TABLE S12 – continued from previous page

| $l$ | $\alpha$ | $\beta$ | $\gamma$ | usim | $\sigma$ | AP@5 | AH@5 | AP@10 | AH@10 | AT@5% | AT@10% | NT@5% | NT@10% |
|---|---|---|---|---|---|---|---|---|---|---|---|---|---|
| 10 | 0.1 | 0.1 | 1.0 | RBF | 10.0 | 0.885 | 3.624 | 0.822 | 5.811 | 53.325 | 61.167 | 36.770 | 50.787 |
| 10 | 0.1 | 0.1 | 10.0 | COS | - | 0.886 | 3.624 | 0.822 | 5.812 | 53.325 | 61.174 | 36.818 | 50.773 |
| 10 | 0.1 | 0.1 | 10.0 | RBF | 10.0 | 0.886 | 3.624 | 0.822 | 5.812 | 53.325 | 61.172 | 36.818 | 50.773 |
| 10 | 0.1 | 0.1 | 100.0 | COS | - | 0.885 | 3.621 | 0.821 | 5.813 | 53.281 | 61.211 | 37.008 | 51.126 |
| 10 | 0.1 | 0.1 | 100.0 | RBF | 10.0 | 0.885 | 3.621 | 0.821 | 5.812 | 53.281 | 61.199 | 37.025 | 51.077 |
| 10 | 0.1 | 1.0 | 0.0 | COS | - | 0.885 | 3.624 | 0.822 | 5.811 | 53.330 | 61.167 | 36.770 | 50.787 |
| 10 | 0.1 | 1.0 | 0.0 | RBF | 10.0 | 0.885 | 3.624 | 0.822 | 5.811 | 53.330 | 61.167 | 36.770 | 50.787 |
| 10 | 0.1 | 1.0 | 1.0 | COS | - | 0.885 | 3.624 | 0.822 | 5.811 | 53.325 | 61.164 | 36.770 | 50.787 |
| 10 | 0.1 | 1.0 | 1.0 | RBF | 10.0 | 0.885 | 3.624 | 0.822 | 5.811 | 53.325 | 61.167 | 36.770 | 50.787 |
| 10 | 0.1 | 1.0 | 10.0 | COS | - | 0.886 | 3.624 | 0.822 | 5.812 | 53.325 | 61.174 | 36.818 | 50.773 |
| 10 | 0.1 | 1.0 | 10.0 | RBF | 10.0 | 0.886 | 3.624 | 0.822 | 5.812 | 53.325 | 61.174 | 36.818 | 50.773 |
| 10 | 0.1 | 1.0 | 100.0 | COS | - | 0.885 | 3.621 | 0.821 | 5.813 | 53.281 | 61.211 | 37.008 | 51.126 |
| 10 | 0.1 | 1.0 | 100.0 | RBF | 10.0 | 0.885 | 3.621 | 0.821 | 5.812 | 53.281 | 61.199 | 37.025 | 51.077 |
| 10 | 0.5 | 0.1 | 0.0 | COS | - | 0.849 | 3.446 | 0.789 | 5.608 | 59.518 | 59.523 | 42.201 | 52.104 |
| 10 | 0.5 | 0.1 | 0.0 | RBF | 10.0 | 0.849 | 3.446 | 0.789 | 5.608 | 59.518 | 59.523 | 42.201 | 52.104 |
| 10 | 0.5 | 0.1 | 1.0 | COS | - | 0.849 | 3.445 | 0.789 | 5.609 | 59.513 | 59.527 | 42.182 | 52.127 |
| 10 | 0.5 | 0.1 | 1.0 | RBF | 10.0 | 0.849 | 3.445 | 0.789 | 5.608 | 59.513 | 59.525 | 42.182 | 52.127 |
| 10 | 0.5 | 0.1 | 10.0 | COS | - | 0.849 | 3.443 | 0.789 | 5.611 | 59.498 | 59.542 | 42.327 | 52.196 |
| 10 | 0.5 | 0.1 | 10.0 | RBF | 10.0 | 0.849 | 3.443 | 0.789 | 5.610 | 59.508 | 59.537 | 42.315 | 52.175 |
| 10 | 0.5 | 0.1 | 100.0 | COS | - | 0.850 | 3.441 | 0.790 | 5.590 | 59.508 | 59.369 | 43.655 | 53.130 |
| 10 | 0.5 | 0.1 | 100.0 | RBF | 10.0 | 0.850 | 3.439 | 0.790 | 5.592 | 59.445 | 59.401 | 43.290 | 53.031 |
| 10 | 0.5 | 1.0 | 0.0 | COS | - | 0.863 | 3.524 | 0.801 | 5.738 | 58.426 | 60.665 | 41.128 | 52.252 |
| 10 | 0.5 | 1.0 | 0.0 | RBF | 10.0 | 0.863 | 3.524 | 0.801 | 5.738 | 58.426 | 60.665 | 41.128 | 52.252 |
| 10 | 0.5 | 1.0 | 1.0 | COS | - | 0.863 | 3.526 | 0.801 | 5.738 | 58.426 | 60.663 | 41.110 | 52.183 |
| 10 | 0.5 | 1.0 | 1.0 | RBF | 10.0 | 0.863 | 3.526 | 0.801 | 5.737 | 58.426 | 60.663 | 41.110 | 52.169 |
| 10 | 0.5 | 1.0 | 10.0 | COS | - | 0.863 | 3.530 | 0.802 | 5.740 | 58.378 | 60.699 | 41.116 | 52.399 |
| 10 | 0.5 | 1.0 | 10.0 | RBF | 10.0 | 0.863 | 3.529 | 0.802 | 5.740 | 58.358 | 60.694 | 41.049 | 52.354 |
| 10 | 0.5 | 1.0 | 100.0 | COS | - | 0.863 | 3.521 | 0.802 | 5.726 | 58.232 | 60.575 | 41.573 | 53.013 |
| 10 | 0.5 | 1.0 | 100.0 | RBF | 10.0 | 0.864 | 3.527 | 0.803 | 5.731 | 58.231 | 60.609 | 41.366 | 52.694 |
| 10 | 1.0 | 0.1 | 0.0 | COS | - | 0.760 | 2.677 | 0.695 | 3.905 | 51.035 | 42.085 | 30.628 | 35.463 |
| 10 | 1.0 | 0.1 | 0.0 | RBF | 10.0 | 0.760 | 2.677 | 0.695 | 3.905 | 51.035 | 42.085 | 30.628 | 35.463 |
| 10 | 1.0 | 0.1 | 1.0 | COS | - | 0.759 | 2.682 | 0.695 | 3.907 | 51.089 | 42.122 | 30.969 | 35.668 |
| 10 | 1.0 | 0.1 | 1.0 | RBF | 10.0 | 0.760 | 2.681 | 0.695 | 3.908 | 51.074 | 42.127 | 30.933 | 35.637 |
| 10 | 1.0 | 0.1 | 10.0 | COS | - | 0.757 | 2.669 | 0.691 | 3.918 | 50.933 | 42.270 | 31.768 | 37.088 |
| 10 | 1.0 | 0.1 | 10.0 | RBF | 10.0 | 0.758 | 2.673 | 0.692 | 3.926 | 50.987 | 42.321 | 31.492 | 37.066 |
| 10 | 1.0 | 0.1 | 100.0 | COS | - | 0.759 | 2.653 | 0.689 | 3.978 | 50.572 | 42.916 | 33.244 | 39.584 |
| 10 | 1.0 | 0.1 | 100.0 | RBF | 10.0 | 0.760 | 2.670 | 0.691 | 3.986 | 50.899 | 43.030 | 33.210 | 39.339 |
| 10 | 1.0 | 1.0 | 0.0 | COS | - | 0.760 | 2.679 | 0.695 | 3.900 | 51.045 | 42.022 | 30.433 | 35.478 |
| 10 | 1.0 | 1.0 | 0.0 | RBF | 10.0 | 0.760 | 2.679 | 0.695 | 3.900 | 51.045 | 42.022 | 30.433 | 35.478 |
| 10 | 1.0 | 1.0 | 1.0 | COS | - | 0.762 | 2.687 | 0.696 | 3.919 | 51.206 | 42.239 | 30.793 | 35.838 |
| 10 | 1.0 | 1.0 | 1.0 | RBF | 10.0 | 0.761 | 2.686 | 0.696 | 3.918 | 51.186 | 42.222 | 30.781 | 35.788 |
| 10 | 1.0 | 1.0 | 10.0 | COS | - | 0.757 | 2.664 | 0.691 | 3.904 | 50.894 | 42.107 | 31.413 | 36.827 |
| 10 | 1.0 | 1.0 | 10.0 | RBF | 10.0 | 0.759 | 2.671 | 0.693 | 3.910 | 50.957 | 42.144 | 31.082 | 36.719 |
| 10 | 1.0 | 1.0 | 100.0 | COS | - | 0.761 | 2.670 | 0.692 | 3.983 | 50.865 | 42.967 | 33.207 | 39.703 |
| 10 | 1.0 | 1.0 | 100.0 | RBF | 10.0 | 0.760 | 2.666 | 0.691 | 3.971 | 50.797 | 42.845 | 33.421 | 39.305 |
| 15 | 0.0 | 0.1 | 0.0 | COS | - | 0.904 | 3.700 | 0.836 | 5.863 | 53.476 | 61.618 | 19.808 | 40.378 |
| 15 | 0.0 | 0.1 | 0.0 | RBF | 10.0 | 0.904 | 3.700 | 0.836 | 5.863 | 53.476 | 61.618 | 19.808 | 40.378 |
| 15 | 0.0 | 0.1 | 1.0 | COS | - | 0.904 | 3.700 | 0.836 | 5.864 | 53.476 | 61.622 | 19.808 | 40.387 |
| 15 | 0.0 | 0.1 | 1.0 | RBF | 10.0 | 0.904 | 3.700 | 0.836 | 5.864 | 53.476 | 61.622 | 19.808 | 40.387 |
| 15 | 0.0 | 0.1 | 10.0 | COS | - | 0.904 | 3.703 | 0.837 | 5.862 | 53.545 | 61.598 | 19.471 | 39.672 |
| 15 | 0.0 | 0.1 | 10.0 | RBF | 10.0 | 0.904 | 3.703 | 0.837 | 5.862 | 53.545 | 61.598 | 19.471 | 39.673 |
| 15 | 0.0 | 0.1 | 100.0 | COS | - | 0.898 | 3.676 | 0.832 | 5.868 | 53.335 | 61.642 | 25.486 | 45.951 |
| 15 | 0.0 | 0.1 | 100.0 | RBF | 10.0 | 0.899 | 3.687 | 0.833 | 5.872 | 53.442 | 61.693 | 23.872 | 44.381 |
| 15 | 0.0 | 1.0 | 0.0 | COS | - | 0.906 | 3.710 | 0.838 | 5.839 | 53.476 | 61.362 | 17.166 | 36.667 |
| 15 | 0.0 | 1.0 | 0.0 | RBF | 10.0 | 0.906 | 3.710 | 0.838 | 5.839 | 53.476 | 61.362 | 17.166 | 36.667 |
| 15 | 0.0 | 1.0 | 1.0 | COS | - | 0.906 | 3.710 | 0.838 | 5.839 | 53.476 | 61.359 | 17.166 | 36.660 |
| 15 | 0.0 | 1.0 | 1.0 | RBF | 10.0 | 0.906 | 3.710 | 0.838 | 5.839 | 53.476 | 61.359 | 17.166 | 36.660 |
| 15 | 0.0 | 1.0 | 10.0 | COS | - | 0.906 | 3.710 | 0.838 | 5.839 | 53.462 | 61.369 | 17.203 | 36.488 |

Continued on next page

TABLE S12 – continued from previous page

| $l$ | $\alpha$ | $\beta$ | $\gamma$ | usim | $\sigma$ | AP@5 | AH@5 | AP@10 | AH@10 | AT@5% | AT@10% | NT@5% | NT@10% |
|---|---|---|---|---|---|---|---|---|---|---|---|---|---|
| 15 | 0.0 | 1.0 | 10.0 | RBF | 10.0 | 0.906 | 3.710 | 0.838 | 5.840 | 53.467 | 61.372 | 17.203 | 36.488 |
| 15 | 0.0 | 1.0 | 100.0 | COS | - | 0.905 | 3.701 | 0.837 | 5.850 | 53.408 | 61.479 | 18.273 | 38.211 |
| 15 | 0.0 | 1.0 | 100.0 | RBF | 10.0 | 0.906 | 3.704 | 0.838 | 5.844 | 53.389 | 61.403 | 17.135 | 36.886 |
| 15 | 0.05 | 0.1 | 0.0 | COS | - | 0.907 | 3.711 | 0.839 | 5.841 | 53.671 | 61.371 | 16.510 | 35.453 |
| 15 | 0.05 | 0.1 | 0.0 | RBF | 10.0 | 0.907 | 3.711 | 0.839 | 5.841 | 53.671 | 61.371 | 16.510 | 35.453 |
| 15 | 0.05 | 0.1 | 1.0 | COS | - | 0.907 | 3.712 | 0.839 | 5.841 | 53.671 | 61.369 | 16.528 | 35.453 |
| 15 | 0.05 | 0.1 | 1.0 | RBF | 10.0 | 0.907 | 3.711 | 0.839 | 5.841 | 53.666 | 61.369 | 16.510 | 35.453 |
| 15 | 0.05 | 0.1 | 10.0 | COS | - | 0.907 | 3.711 | 0.839 | 5.840 | 53.676 | 61.364 | 16.583 | 35.453 |
| 15 | 0.05 | 0.1 | 10.0 | RBF | 10.0 | 0.907 | 3.711 | 0.839 | 5.840 | 53.671 | 61.362 | 16.546 | 35.453 |
| 15 | 0.05 | 0.1 | 100.0 | COS | - | 0.906 | 3.710 | 0.838 | 5.839 | 53.632 | 61.347 | 16.715 | 35.742 |
| 15 | 0.05 | 0.1 | 100.0 | RBF | 10.0 | 0.906 | 3.709 | 0.839 | 5.838 | 53.627 | 61.354 | 16.697 | 35.646 |
| 15 | 0.05 | 1.0 | 0.0 | COS | - | 0.907 | 3.711 | 0.839 | 5.841 | 53.666 | 61.371 | 16.510 | 35.453 |
| 15 | 0.05 | 1.0 | 0.0 | RBF | 10.0 | 0.907 | 3.711 | 0.839 | 5.841 | 53.666 | 61.371 | 16.510 | 35.453 |
| 15 | 0.05 | 1.0 | 1.0 | COS | - | 0.907 | 3.711 | 0.839 | 5.841 | 53.676 | 61.369 | 16.546 | 35.453 |
| 15 | 0.05 | 1.0 | 1.0 | RBF | 10.0 | 0.907 | 3.711 | 0.839 | 5.841 | 53.671 | 61.369 | 16.528 | 35.453 |
| 15 | 0.05 | 1.0 | 10.0 | COS | - | 0.907 | 3.711 | 0.839 | 5.840 | 53.676 | 61.364 | 16.583 | 35.453 |
| 15 | 0.05 | 1.0 | 10.0 | RBF | 10.0 | 0.907 | 3.711 | 0.839 | 5.840 | 53.671 | 61.362 | 16.546 | 35.453 |
| 15 | 0.05 | 1.0 | 100.0 | COS | - | 0.906 | 3.709 | 0.838 | 5.837 | 53.617 | 61.340 | 16.715 | 35.639 |
| 15 | 0.05 | 1.0 | 100.0 | RBF | 10.0 | 0.906 | 3.709 | 0.839 | 5.838 | 53.627 | 61.354 | 16.697 | 35.646 |
| 15 | 0.1 | 0.1 | 0.0 | COS | - | 0.907 | 3.713 | 0.839 | 5.839 | 53.832 | 61.342 | 15.856 | 34.516 |
| 15 | 0.1 | 0.1 | 0.0 | RBF | 10.0 | 0.907 | 3.713 | 0.839 | 5.839 | 53.832 | 61.342 | 15.856 | 34.516 |
| 15 | 0.1 | 0.1 | 1.0 | COS | - | 0.907 | 3.713 | 0.839 | 5.839 | 53.827 | 61.342 | 15.856 | 34.516 |
| 15 | 0.1 | 0.1 | 1.0 | RBF | 10.0 | 0.907 | 3.713 | 0.839 | 5.839 | 53.827 | 61.342 | 15.856 | 34.516 |
| 15 | 0.1 | 0.1 | 10.0 | COS | - | 0.907 | 3.712 | 0.839 | 5.839 | 53.807 | 61.349 | 15.783 | 34.598 |
| 15 | 0.1 | 0.1 | 10.0 | RBF | 10.0 | 0.907 | 3.712 | 0.839 | 5.839 | 53.807 | 61.347 | 15.783 | 34.571 |
| 15 | 0.1 | 0.1 | 100.0 | COS | - | 0.907 | 3.710 | 0.839 | 5.839 | 53.803 | 61.335 | 16.245 | 34.822 |
| 15 | 0.1 | 0.1 | 100.0 | RBF | 10.0 | 0.907 | 3.712 | 0.839 | 5.840 | 53.827 | 61.347 | 16.208 | 34.906 |
| 15 | 0.1 | 1.0 | 0.0 | COS | - | 0.907 | 3.713 | 0.839 | 5.839 | 53.827 | 61.342 | 15.856 | 34.516 |
| 15 | 0.1 | 1.0 | 0.0 | RBF | 10.0 | 0.907 | 3.713 | 0.839 | 5.839 | 53.827 | 61.342 | 15.856 | 34.516 |
| 15 | 0.1 | 1.0 | 1.0 | COS | - | 0.907 | 3.713 | 0.839 | 5.839 | 53.822 | 61.342 | 15.820 | 34.516 |
| 15 | 0.1 | 1.0 | 1.0 | RBF | 10.0 | 0.907 | 3.713 | 0.839 | 5.839 | 53.822 | 61.342 | 15.820 | 34.516 |
| 15 | 0.1 | 1.0 | 10.0 | COS | - | 0.907 | 3.713 | 0.839 | 5.839 | 53.812 | 61.349 | 15.783 | 34.598 |
| 15 | 0.1 | 1.0 | 10.0 | RBF | 10.0 | 0.907 | 3.712 | 0.839 | 5.839 | 53.807 | 61.349 | 15.783 | 34.598 |
| 15 | 0.1 | 1.0 | 100.0 | COS | - | 0.907 | 3.710 | 0.839 | 5.839 | 53.798 | 61.337 | 16.245 | 34.831 |
| 15 | 0.1 | 1.0 | 100.0 | RBF | 10.0 | 0.907 | 3.712 | 0.839 | 5.840 | 53.827 | 61.347 | 16.208 | 34.906 |
| 15 | 0.5 | 0.1 | 0.0 | COS | - | 0.875 | 3.519 | 0.808 | 5.710 | 62.485 | 60.826 | 28.910 | 43.998 |
| 15 | 0.5 | 0.1 | 0.0 | RBF | 10.0 | 0.875 | 3.519 | 0.808 | 5.710 | 62.485 | 60.826 | 28.910 | 43.998 |
| 15 | 0.5 | 0.1 | 1.0 | COS | - | 0.875 | 3.518 | 0.808 | 5.711 | 62.485 | 60.835 | 28.855 | 44.043 |
| 15 | 0.5 | 0.1 | 1.0 | RBF | 10.0 | 0.875 | 3.518 | 0.808 | 5.711 | 62.475 | 60.835 | 28.855 | 44.043 |
| 15 | 0.5 | 0.1 | 10.0 | COS | - | 0.875 | 3.519 | 0.808 | 5.707 | 62.490 | 60.799 | 29.012 | 44.269 |
| 15 | 0.5 | 0.1 | 10.0 | RBF | 10.0 | 0.875 | 3.519 | 0.808 | 5.708 | 62.509 | 60.802 | 29.025 | 44.246 |
| 15 | 0.5 | 0.1 | 100.0 | COS | - | 0.871 | 3.506 | 0.805 | 5.684 | 62.363 | 60.497 | 31.477 | 45.924 |
| 15 | 0.5 | 0.1 | 100.0 | RBF | 10.0 | 0.872 | 3.508 | 0.805 | 5.693 | 62.407 | 60.606 | 31.106 | 45.633 |
| 15 | 0.5 | 1.0 | 0.0 | COS | - | 0.878 | 3.552 | 0.811 | 5.762 | 61.505 | 61.174 | 25.845 | 41.923 |
| 15 | 0.5 | 1.0 | 0.0 | RBF | 10.0 | 0.878 | 3.552 | 0.811 | 5.762 | 61.505 | 61.174 | 25.845 | 41.923 |
| 15 | 0.5 | 1.0 | 1.0 | COS | - | 0.878 | 3.552 | 0.812 | 5.765 | 61.452 | 61.189 | 25.652 | 41.852 |
| 15 | 0.5 | 1.0 | 1.0 | RBF | 10.0 | 0.879 | 3.552 | 0.812 | 5.764 | 61.452 | 61.189 | 25.652 | 41.838 |
| 15 | 0.5 | 1.0 | 10.0 | COS | - | 0.879 | 3.561 | 0.812 | 5.770 | 61.345 | 61.240 | 25.607 | 41.590 |
| 15 | 0.5 | 1.0 | 10.0 | RBF | 10.0 | 0.879 | 3.560 | 0.812 | 5.770 | 61.355 | 61.249 | 25.540 | 41.713 |
| 15 | 0.5 | 1.0 | 100.0 | COS | - | 0.877 | 3.548 | 0.809 | 5.762 | 61.160 | 61.162 | 27.027 | 43.266 |
| 15 | 0.5 | 1.0 | 100.0 | RBF | 10.0 | 0.877 | 3.552 | 0.809 | 5.767 | 61.155 | 61.216 | 26.811 | 43.041 |
| 15 | 1.0 | 0.1 | 0.0 | COS | - | 0.847 | 3.096 | 0.776 | 4.347 | 59.313 | 46.894 | 23.980 | 32.683 |
| 15 | 1.0 | 0.1 | 0.0 | RBF | 10.0 | 0.847 | 3.096 | 0.776 | 4.347 | 59.313 | 46.894 | 23.980 | 32.683 |
| 15 | 1.0 | 0.1 | 1.0 | COS | - | 0.848 | 3.096 | 0.776 | 4.348 | 59.318 | 46.911 | 24.503 | 32.995 |
| 15 | 1.0 | 0.1 | 1.0 | RBF | 10.0 | 0.847 | 3.096 | 0.776 | 4.347 | 59.323 | 46.899 | 24.394 | 32.948 |
| 15 | 1.0 | 0.1 | 10.0 | COS | - | 0.841 | 3.038 | 0.769 | 4.297 | 58.266 | 46.446 | 28.279 | 36.290 |
| 15 | 1.0 | 0.1 | 10.0 | RBF | 10.0 | 0.842 | 3.051 | 0.771 | 4.308 | 58.499 | 46.553 | 28.000 | 35.883 |
| 15 | 1.0 | 0.1 | 100.0 | COS | - | 0.821 | 2.858 | 0.742 | 4.165 | 54.943 | 44.972 | 32.395 | 40.372 |

Continued on next page

TABLE S12 – continued from previous page

| $l$ | $\alpha$ | $\beta$ | $\gamma$ | usim | $\sigma$ | AP@5 | AH@5 | AP@10 | AH@10 | AT@5% | AT@10% | NT@5% | NT@10% |
|---|---|---|---|---|---|---|---|---|---|---|---|---|---|
| 15 | 1.0 | 0.1 | 100.0 | RBF | 10.0 | 0.817 | 2.845 | 0.740 | 4.147 | 54.753 | 44.741 | 32.496 | 40.427 |
| 15 | 1.0 | 1.0 | 0.0 | COS | - | 0.849 | 3.093 | 0.777 | 4.345 | 59.220 | 46.870 | 23.888 | 32.781 |
| 15 | 1.0 | 1.0 | 0.0 | RBF | 10.0 | 0.849 | 3.093 | 0.777 | 4.345 | 59.220 | 46.870 | 23.888 | 32.781 |
| 15 | 1.0 | 1.0 | 1.0 | COS | - | 0.849 | 3.097 | 0.777 | 4.353 | 59.313 | 46.965 | 24.470 | 33.114 |
| 15 | 1.0 | 1.0 | 1.0 | RBF | 10.0 | 0.849 | 3.096 | 0.777 | 4.353 | 59.308 | 46.962 | 24.432 | 33.109 |
| 15 | 1.0 | 1.0 | 10.0 | COS | - | 0.842 | 3.033 | 0.770 | 4.278 | 58.197 | 46.207 | 28.183 | 36.032 |
| 15 | 1.0 | 1.0 | 10.0 | RBF | 10.0 | 0.844 | 3.043 | 0.771 | 4.287 | 58.373 | 46.317 | 28.015 | 35.694 |
| 15 | 1.0 | 1.0 | 100.0 | COS | - | 0.817 | 2.839 | 0.739 | 4.145 | 54.631 | 44.716 | 33.076 | 40.777 |
| 15 | 1.0 | 1.0 | 100.0 | RBF | 10.0 | 0.825 | 2.894 | 0.748 | 4.192 | 55.679 | 45.272 | 32.245 | 40.015 |
| 30 | 0.0 | 0.1 | 0.0 | COS | - | 0.938 | 3.930 | 0.873 | 5.958 | 55.898 | 62.253 | 4.707 | 13.993 |
| 30 | 0.0 | 0.1 | 0.0 | RBF | 10.0 | 0.938 | 3.930 | 0.873 | 5.958 | 55.898 | 62.253 | 4.707 | 13.993 |
| 30 | 0.0 | 0.1 | 1.0 | COS | - | 0.938 | 3.931 | 0.873 | 5.957 | 55.898 | 62.249 | 4.594 | 13.668 |
| 30 | 0.0 | 0.1 | 1.0 | RBF | 10.0 | 0.938 | 3.931 | 0.873 | 5.956 | 55.898 | 62.246 | 4.594 | 13.668 |
| 30 | 0.0 | 0.1 | 10.0 | COS | - | 0.940 | 3.949 | 0.876 | 5.950 | 56.180 | 62.183 | 3.856 | 12.249 |
| 30 | 0.0 | 0.1 | 10.0 | RBF | 10.0 | 0.940 | 3.948 | 0.875 | 5.953 | 56.141 | 62.212 | 3.911 | 12.320 |
| 30 | 0.0 | 0.1 | 100.0 | COS | - | 0.905 | 3.747 | 0.839 | 5.930 | 54.173 | 62.046 | 24.055 | 37.370 |
| 30 | 0.0 | 0.1 | 100.0 | RBF | 10.0 | 0.915 | 3.800 | 0.849 | 5.969 | 54.650 | 62.434 | 16.795 | 30.313 |
| 30 | 0.0 | 1.0 | 0.0 | COS | - | 0.947 | 4.006 | 0.885 | 5.917 | 56.926 | 61.944 | 2.663 | 7.854 |
| 30 | 0.0 | 1.0 | 0.0 | RBF | 10.0 | 0.947 | 4.006 | 0.885 | 5.917 | 56.926 | 61.944 | 2.663 | 7.854 |
| 30 | 0.0 | 1.0 | 1.0 | COS | - | 0.947 | 4.011 | 0.886 | 5.917 | 56.994 | 61.939 | 2.602 | 7.742 |
| 30 | 0.0 | 1.0 | 1.0 | RBF | 10.0 | 0.947 | 4.011 | 0.886 | 5.917 | 56.994 | 61.939 | 2.602 | 7.742 |
| 30 | 0.0 | 1.0 | 10.0 | COS | - | 0.948 | 4.010 | 0.886 | 5.917 | 56.970 | 61.932 | 2.602 | 7.710 |
| 30 | 0.0 | 1.0 | 10.0 | RBF | 10.0 | 0.948 | 4.010 | 0.886 | 5.917 | 56.970 | 61.932 | 2.602 | 7.710 |
| 30 | 0.0 | 1.0 | 100.0 | COS | - | 0.930 | 3.890 | 0.865 | 5.961 | 55.503 | 62.300 | 6.932 | 18.147 |
| 30 | 0.0 | 1.0 | 100.0 | RBF | 10.0 | 0.938 | 3.933 | 0.874 | 5.947 | 55.956 | 62.163 | 4.210 | 12.839 |
| 30 | 0.05 | 0.1 | 0.0 | COS | - | 0.948 | 4.018 | 0.887 | 5.925 | 57.418 | 62.032 | 2.504 | 7.491 |
| 30 | 0.05 | 0.1 | 0.0 | RBF | 10.0 | 0.948 | 4.018 | 0.887 | 5.925 | 57.418 | 62.032 | 2.504 | 7.491 |
| 30 | 0.05 | 0.1 | 1.0 | COS | - | 0.948 | 4.018 | 0.887 | 5.926 | 57.418 | 62.029 | 2.504 | 7.463 |
| 30 | 0.05 | 0.1 | 1.0 | RBF | 10.0 | 0.948 | 4.018 | 0.887 | 5.926 | 57.418 | 62.029 | 2.504 | 7.463 |
| 30 | 0.05 | 0.1 | 10.0 | COS | - | 0.948 | 4.018 | 0.887 | 5.926 | 57.403 | 62.034 | 2.521 | 7.477 |
| 30 | 0.05 | 0.1 | 10.0 | RBF | 10.0 | 0.948 | 4.018 | 0.887 | 5.926 | 57.403 | 62.034 | 2.521 | 7.477 |
| 30 | 0.05 | 0.1 | 100.0 | COS | - | 0.933 | 3.906 | 0.868 | 5.963 | 56.185 | 62.326 | 6.110 | 16.455 |
| 30 | 0.05 | 0.1 | 100.0 | RBF | 10.0 | 0.940 | 3.956 | 0.877 | 5.951 | 56.765 | 62.192 | 3.618 | 11.409 |
| 30 | 0.05 | 1.0 | 0.0 | COS | - | 0.948 | 4.018 | 0.887 | 5.925 | 57.418 | 62.032 | 2.504 | 7.491 |
| 30 | 0.05 | 1.0 | 0.0 | RBF | 10.0 | 0.948 | 4.018 | 0.887 | 5.925 | 57.418 | 62.032 | 2.504 | 7.491 |
| 30 | 0.05 | 1.0 | 1.0 | COS | - | 0.948 | 4.018 | 0.887 | 5.926 | 57.418 | 62.029 | 2.504 | 7.463 |
| 30 | 0.05 | 1.0 | 1.0 | RBF | 10.0 | 0.948 | 4.018 | 0.887 | 5.926 | 57.418 | 62.029 | 2.504 | 7.463 |
| 30 | 0.05 | 1.0 | 10.0 | COS | - | 0.948 | 4.018 | 0.887 | 5.926 | 57.408 | 62.032 | 2.521 | 7.450 |
| 30 | 0.05 | 1.0 | 10.0 | RBF | 10.0 | 0.948 | 4.018 | 0.887 | 5.926 | 57.403 | 62.034 | 2.521 | 7.477 |
| 30 | 0.05 | 1.0 | 100.0 | COS | - | 0.943 | 3.979 | 0.880 | 5.942 | 56.955 | 62.107 | 3.038 | 9.726 |
| 30 | 0.05 | 1.0 | 100.0 | RBF | 10.0 | 0.947 | 4.010 | 0.886 | 5.923 | 57.262 | 62.002 | 2.559 | 7.750 |
| 30 | 0.1 | 0.1 | 0.0 | COS | - | 0.948 | 4.023 | 0.887 | 5.938 | 57.793 | 62.156 | 2.487 | 7.416 |
| 30 | 0.1 | 0.1 | 0.0 | RBF | 10.0 | 0.948 | 4.023 | 0.887 | 5.938 | 57.793 | 62.156 | 2.487 | 7.416 |
| 30 | 0.1 | 0.1 | 1.0 | COS | - | 0.948 | 4.023 | 0.887 | 5.938 | 57.793 | 62.153 | 2.487 | 7.416 |
| 30 | 0.1 | 0.1 | 1.0 | RBF | 10.0 | 0.948 | 4.023 | 0.887 | 5.938 | 57.793 | 62.153 | 2.487 | 7.416 |
| 30 | 0.1 | 0.1 | 10.0 | COS | - | 0.948 | 4.023 | 0.887 | 5.937 | 57.798 | 62.141 | 2.487 | 7.408 |
| 30 | 0.1 | 0.1 | 10.0 | RBF | 10.0 | 0.948 | 4.023 | 0.887 | 5.937 | 57.803 | 62.139 | 2.487 | 7.408 |
| 30 | 0.1 | 0.1 | 100.0 | COS | - | 0.938 | 3.954 | 0.875 | 5.967 | 57.282 | 62.363 | 4.427 | 12.491 |
| 30 | 0.1 | 0.1 | 100.0 | RBF | 10.0 | 0.945 | 4.003 | 0.884 | 5.942 | 57.564 | 62.180 | 2.782 | 8.541 |
| 30 | 0.1 | 1.0 | 0.0 | COS | - | 0.948 | 4.023 | 0.887 | 5.937 | 57.808 | 62.144 | 2.487 | 7.403 |
| 30 | 0.1 | 1.0 | 0.0 | RBF | 10.0 | 0.948 | 4.023 | 0.887 | 5.937 | 57.808 | 62.144 | 2.487 | 7.403 |
| 30 | 0.1 | 1.0 | 1.0 | COS | - | 0.948 | 4.023 | 0.887 | 5.937 | 57.808 | 62.144 | 2.487 | 7.403 |
| 30 | 0.1 | 1.0 | 1.0 | RBF | 10.0 | 0.948 | 4.023 | 0.887 | 5.937 | 57.808 | 62.144 | 2.487 | 7.403 |
| 30 | 0.1 | 1.0 | 10.0 | COS | - | 0.948 | 4.023 | 0.887 | 5.937 | 57.798 | 62.141 | 2.487 | 7.408 |
| 30 | 0.1 | 1.0 | 10.0 | RBF | 10.0 | 0.948 | 4.023 | 0.887 | 5.937 | 57.803 | 62.141 | 2.487 | 7.408 |
| 30 | 0.1 | 1.0 | 100.0 | COS | - | 0.945 | 4.003 | 0.883 | 5.942 | 57.535 | 62.185 | 2.782 | 8.591 |
| 30 | 0.1 | 1.0 | 100.0 | RBF | 10.0 | 0.948 | 4.018 | 0.886 | 5.935 | 57.725 | 62.134 | 2.486 | 7.571 |
| 30 | 0.5 | 0.1 | 0.0 | COS | - | 0.922 | 3.755 | 0.850 | 5.816 | 67.459 | 62.148 | 9.985 | 19.554 |

Continued on next page

TABLE S12 – continued from previous page

| $l$ | $\alpha$ | $\beta$ | $\gamma$ | usim | $\sigma$ | AP@5 | AH@5 | AP@10 | AH@10 | AT@5% | AT@10% | NT@5% | NT@10% |
|---|---|---|---|---|---|---|---|---|---|---|---|---|---|
| 30 | 0.5 | 0.1 | 0.0 | RBF | 10.0 | 0.922 | 3.755 | 0.850 | 5.816 | 67.459 | 62.148 | 9.985 | 19.554 |
| 30 | 0.5 | 0.1 | 1.0 | COS | - | 0.922 | 3.755 | 0.850 | 5.814 | 67.469 | 62.139 | 9.985 | 19.593 |
| 30 | 0.5 | 0.1 | 1.0 | RBF | 10.0 | 0.922 | 3.755 | 0.850 | 5.814 | 67.469 | 62.134 | 9.985 | 19.573 |
| 30 | 0.5 | 0.1 | 10.0 | COS | - | 0.921 | 3.751 | 0.849 | 5.808 | 67.406 | 62.102 | 10.124 | 19.859 |
| 30 | 0.5 | 0.1 | 10.0 | RBF | 10.0 | 0.921 | 3.751 | 0.849 | 5.810 | 67.401 | 62.117 | 10.087 | 19.844 |
| 30 | 0.5 | 0.1 | 100.0 | COS | - | 0.913 | 3.707 | 0.841 | 5.767 | 66.738 | 61.691 | 12.476 | 23.133 |
| 30 | 0.5 | 0.1 | 100.0 | RBF | 10.0 | 0.914 | 3.713 | 0.842 | 5.775 | 66.816 | 61.766 | 12.146 | 22.590 |
| 30 | 0.5 | 1.0 | 0.0 | COS | - | 0.923 | 3.772 | 0.851 | 5.837 | 67.001 | 62.273 | 8.414 | 17.279 |
| 30 | 0.5 | 1.0 | 0.0 | RBF | 10.0 | 0.923 | 3.772 | 0.851 | 5.837 | 67.001 | 62.273 | 8.414 | 17.279 |
| 30 | 0.5 | 1.0 | 1.0 | COS | - | 0.923 | 3.772 | 0.851 | 5.837 | 66.957 | 62.275 | 8.386 | 17.187 |
| 30 | 0.5 | 1.0 | 1.0 | RBF | 10.0 | 0.923 | 3.773 | 0.851 | 5.838 | 66.962 | 62.278 | 8.368 | 17.187 |
| 30 | 0.5 | 1.0 | 10.0 | COS | - | 0.923 | 3.774 | 0.852 | 5.842 | 66.704 | 62.302 | 8.057 | 16.705 |
| 30 | 0.5 | 1.0 | 10.0 | RBF | 10.0 | 0.923 | 3.773 | 0.852 | 5.841 | 66.719 | 62.290 | 8.044 | 16.701 |
| 30 | 0.5 | 1.0 | 100.0 | COS | - | 0.917 | 3.736 | 0.845 | 5.799 | 66.300 | 61.868 | 9.872 | 19.434 |
| 30 | 0.5 | 1.0 | 100.0 | RBF | 10.0 | 0.919 | 3.746 | 0.848 | 5.810 | 66.222 | 61.942 | 9.179 | 18.183 |
| 30 | 1.0 | 0.1 | 0.0 | COS | - | 0.937 | 3.591 | 0.871 | 4.673 | 67.508 | 50.902 | 9.615 | 19.160 |
| 30 | 1.0 | 0.1 | 0.0 | RBF | 10.0 | 0.937 | 3.591 | 0.871 | 4.673 | 67.508 | 50.902 | 9.615 | 19.160 |
| 30 | 1.0 | 0.1 | 1.0 | COS | - | 0.936 | 3.582 | 0.869 | 4.681 | 67.406 | 51.006 | 10.368 | 19.829 |
| 30 | 1.0 | 0.1 | 1.0 | RBF | 10.0 | 0.936 | 3.584 | 0.869 | 4.680 | 67.415 | 50.991 | 10.301 | 19.770 |
| 30 | 1.0 | 0.1 | 10.0 | COS | - | 0.921 | 3.489 | 0.850 | 4.672 | 66.568 | 50.731 | 20.160 | 30.674 |
| 30 | 1.0 | 0.1 | 10.0 | RBF | 10.0 | 0.924 | 3.508 | 0.853 | 4.685 | 66.782 | 50.896 | 18.566 | 29.390 |
| 30 | 1.0 | 0.1 | 100.0 | COS | - | 0.892 | 3.108 | 0.802 | 4.435 | 60.029 | 47.766 | 30.481 | 42.831 |
| 30 | 1.0 | 0.1 | 100.0 | RBF | 10.0 | 0.891 | 3.141 | 0.803 | 4.459 | 60.658 | 48.085 | 30.903 | 42.882 |
| 30 | 1.0 | 1.0 | 0.0 | COS | - | 0.936 | 3.587 | 0.871 | 4.667 | 67.435 | 50.855 | 9.743 | 19.325 |
| 30 | 1.0 | 1.0 | 0.0 | RBF | 10.0 | 0.936 | 3.587 | 0.871 | 4.667 | 67.435 | 50.855 | 9.743 | 19.325 |
| 30 | 1.0 | 1.0 | 1.0 | COS | - | 0.936 | 3.581 | 0.869 | 4.681 | 67.381 | 51.033 | 10.252 | 19.627 |
| 30 | 1.0 | 1.0 | 1.0 | RBF | 10.0 | 0.936 | 3.582 | 0.869 | 4.683 | 67.401 | 51.040 | 10.187 | 19.609 |
| 30 | 1.0 | 1.0 | 10.0 | COS | - | 0.922 | 3.484 | 0.851 | 4.649 | 66.480 | 50.451 | 20.550 | 31.313 |
| 30 | 1.0 | 1.0 | 10.0 | RBF | 10.0 | 0.925 | 3.501 | 0.854 | 4.658 | 66.704 | 50.585 | 19.399 | 29.842 |
| 30 | 1.0 | 1.0 | 100.0 | COS | - | 0.889 | 3.125 | 0.802 | 4.434 | 60.322 | 47.766 | 31.508 | 42.788 |
| 30 | 1.0 | 1.0 | 100.0 | RBF | 10.0 | 0.892 | 3.153 | 0.805 | 4.468 | 60.853 | 48.132 | 31.375 | 42.962 |
| 50 | 0.0 | 0.1 | 0.0 | COS | - | 0.949 | 4.111 | 0.894 | 6.194 | 58.821 | 64.638 | 2.102 | 7.198 |
| 50 | 0.0 | 0.1 | 0.0 | RBF | 10.0 | 0.949 | 4.111 | 0.894 | 6.194 | 58.821 | 64.638 | 2.102 | 7.198 |
| 50 | 0.0 | 0.1 | 1.0 | COS | - | 0.953 | 4.133 | 0.898 | 6.189 | 59.143 | 64.628 | 1.537 | 5.928 |
| 50 | 0.0 | 0.1 | 1.0 | RBF | 10.0 | 0.953 | 4.133 | 0.898 | 6.189 | 59.143 | 64.628 | 1.537 | 5.928 |
| 50 | 0.0 | 0.1 | 10.0 | COS | - | 0.958 | 4.183 | 0.905 | 6.197 | 59.902 | 64.709 | 0.857 | 3.756 |
| 50 | 0.0 | 0.1 | 10.0 | RBF | 10.0 | 0.958 | 4.176 | 0.904 | 6.194 | 59.820 | 64.680 | 0.884 | 3.903 |
| 50 | 0.0 | 0.1 | 100.0 | COS | - | 0.904 | 3.760 | 0.838 | 6.001 | 54.348 | 62.731 | 27.350 | 39.077 |
| 50 | 0.0 | 0.1 | 100.0 | RBF | 10.0 | 0.911 | 3.832 | 0.848 | 6.078 | 55.420 | 63.518 | 21.996 | 31.845 |
| 50 | 0.0 | 1.0 | 0.0 | COS | - | 0.967 | 4.271 | 0.917 | 6.217 | 61.184 | 64.984 | 0.609 | 2.156 |
| 50 | 0.0 | 1.0 | 0.0 | RBF | 10.0 | 0.967 | 4.271 | 0.917 | 6.217 | 61.184 | 64.984 | 0.609 | 2.156 |
| 50 | 0.0 | 1.0 | 1.0 | COS | - | 0.967 | 4.271 | 0.917 | 6.216 | 61.179 | 64.982 | 0.609 | 2.156 |
| 50 | 0.0 | 1.0 | 1.0 | RBF | 10.0 | 0.967 | 4.271 | 0.917 | 6.216 | 61.179 | 64.982 | 0.609 | 2.156 |
| 50 | 0.0 | 1.0 | 10.0 | COS | - | 0.969 | 4.293 | 0.920 | 6.222 | 61.627 | 65.079 | 0.588 | 1.968 |
| 50 | 0.0 | 1.0 | 10.0 | RBF | 10.0 | 0.969 | 4.291 | 0.920 | 6.222 | 61.583 | 65.069 | 0.588 | 1.983 |
| 50 | 0.0 | 1.0 | 100.0 | COS | - | 0.926 | 3.933 | 0.865 | 6.168 | 56.658 | 64.358 | 10.464 | 19.709 |
| 50 | 0.0 | 1.0 | 100.0 | RBF | 10.0 | 0.940 | 4.031 | 0.882 | 6.180 | 57.871 | 64.429 | 4.482 | 11.708 |
| 50 | 0.05 | 0.1 | 0.0 | COS | - | 0.968 | 4.293 | 0.920 | 6.230 | 62.100 | 65.165 | 0.588 | 2.013 |
| 50 | 0.05 | 0.1 | 0.0 | RBF | 10.0 | 0.968 | 4.293 | 0.920 | 6.230 | 62.100 | 65.165 | 0.588 | 2.013 |
| 50 | 0.05 | 0.1 | 1.0 | COS | - | 0.968 | 4.293 | 0.919 | 6.230 | 62.095 | 65.165 | 0.588 | 2.013 |
| 50 | 0.05 | 0.1 | 1.0 | RBF | 10.0 | 0.968 | 4.293 | 0.919 | 6.230 | 62.095 | 65.165 | 0.588 | 2.013 |
| 50 | 0.05 | 0.1 | 10.0 | COS | - | 0.969 | 4.307 | 0.921 | 6.233 | 62.300 | 65.223 | 0.580 | 1.954 |
| 50 | 0.05 | 0.1 | 10.0 | RBF | 10.0 | 0.969 | 4.306 | 0.921 | 6.233 | 62.295 | 65.223 | 0.580 | 1.961 |
| 50 | 0.05 | 0.1 | 100.0 | COS | - | 0.918 | 3.898 | 0.857 | 6.123 | 58.100 | 63.990 | 18.299 | 28.140 |
| 50 | 0.05 | 0.1 | 100.0 | RBF | 10.0 | 0.934 | 4.006 | 0.876 | 6.181 | 58.791 | 64.546 | 7.393 | 16.115 |
| 50 | 0.05 | 1.0 | 0.0 | COS | - | 0.969 | 4.310 | 0.922 | 6.233 | 62.353 | 65.245 | 0.580 | 1.906 |
| 50 | 0.05 | 1.0 | 0.0 | RBF | 10.0 | 0.969 | 4.310 | 0.922 | 6.233 | 62.353 | 65.245 | 0.580 | 1.906 |
| 50 | 0.05 | 1.0 | 1.0 | COS | - | 0.969 | 4.310 | 0.922 | 6.233 | 62.348 | 65.242 | 0.580 | 1.906 |

Continued on next page

TABLE S12 – continued from previous page

| $l$ | $\alpha$ | $\beta$ | $\gamma$ | usim | $\sigma$ | AP@5 | AH@5 | AP@10 | AH@10 | AT@5% | AT@10% | NT@5% | NT@10% |
|---|---|---|---|---|---|---|---|---|---|---|---|---|---|
| 50 | 0.05 | 1.0 | 1.0 | RBF | 10.0 | 0.969 | 4.310 | 0.922 | 6.233 | 62.348 | 65.242 | 0.580 | 1.906 |
| 50 | 0.05 | 1.0 | 10.0 | COS | - | 0.969 | 4.310 | 0.922 | 6.234 | 62.348 | 65.255 | 0.580 | 1.898 |
| 50 | 0.05 | 1.0 | 10.0 | RBF | 10.0 | 0.969 | 4.310 | 0.922 | 6.234 | 62.344 | 65.255 | 0.580 | 1.898 |
| 50 | 0.05 | 1.0 | 100.0 | COS | - | 0.942 | 4.055 | 0.885 | 6.184 | 59.118 | 64.546 | 4.104 | 11.075 |
| 50 | 0.05 | 1.0 | 100.0 | RBF | 10.0 | 0.956 | 4.166 | 0.902 | 6.191 | 60.404 | 64.670 | 1.091 | 4.507 |
| 50 | 0.1 | 0.1 | 0.0 | COS | - | 0.926 | 3.960 | 0.870 | 5.972 | 57.554 | 62.553 | 18.816 | 23.479 |
| 50 | 0.1 | 0.1 | 0.0 | RBF | 10.0 | 0.926 | 3.961 | 0.870 | 5.972 | 57.554 | 62.553 | 18.816 | 23.479 |
| 50 | 0.1 | 0.1 | 1.0 | COS | - | 0.969 | 4.298 | 0.920 | 6.241 | 62.675 | 65.313 | 0.598 | 2.041 |
| 50 | 0.1 | 0.1 | 1.0 | RBF | 10.0 | 0.969 | 4.298 | 0.920 | 6.241 | 62.675 | 65.313 | 0.598 | 2.041 |
| 50 | 0.1 | 0.1 | 10.0 | COS | - | 0.969 | 4.312 | 0.921 | 6.245 | 62.787 | 65.389 | 0.616 | 2.010 |
| 50 | 0.1 | 0.1 | 10.0 | RBF | 10.0 | 0.969 | 4.310 | 0.921 | 6.244 | 62.772 | 65.374 | 0.616 | 2.017 |
| 50 | 0.1 | 0.1 | 100.0 | COS | - | 0.924 | 3.939 | 0.863 | 6.182 | 61.880 | 64.675 | 16.814 | 25.781 |
| 50 | 0.1 | 0.1 | 100.0 | RBF | 10.0 | 0.931 | 3.994 | 0.872 | 6.183 | 61.120 | 64.643 | 10.606 | 19.454 |
| 50 | 0.1 | 1.0 | 0.0 | COS | - | 0.970 | 4.317 | 0.922 | 6.245 | 62.904 | 65.393 | 0.615 | 1.948 |
| 50 | 0.1 | 1.0 | 0.0 | RBF | 10.0 | 0.970 | 4.317 | 0.922 | 6.245 | 62.904 | 65.393 | 0.615 | 1.948 |
| 50 | 0.1 | 1.0 | 1.0 | COS | - | 0.970 | 4.317 | 0.922 | 6.245 | 62.904 | 65.396 | 0.615 | 1.948 |
| 50 | 0.1 | 1.0 | 1.0 | RBF | 10.0 | 0.970 | 4.317 | 0.922 | 6.245 | 62.904 | 65.396 | 0.615 | 1.948 |
| 50 | 0.1 | 1.0 | 10.0 | COS | - | 0.970 | 4.319 | 0.922 | 6.247 | 62.918 | 65.410 | 0.615 | 1.948 |
| 50 | 0.1 | 1.0 | 10.0 | RBF | 10.0 | 0.970 | 4.318 | 0.922 | 6.247 | 62.913 | 65.408 | 0.615 | 1.948 |
| 50 | 0.1 | 1.0 | 100.0 | COS | - | 0.943 | 4.075 | 0.887 | 6.193 | 60.726 | 64.704 | 4.003 | 10.863 |
| 50 | 0.1 | 1.0 | 100.0 | RBF | 10.0 | 0.956 | 4.186 | 0.904 | 6.207 | 61.535 | 64.891 | 0.977 | 4.121 |
| 50 | 0.5 | 0.1 | 0.0 | COS | - | 0.915 | 3.796 | 0.851 | 5.820 | 62.767 | 61.893 | 21.142 | 28.107 |
| 50 | 0.5 | 0.1 | 0.0 | RBF | 10.0 | 0.915 | 3.796 | 0.851 | 5.820 | 62.767 | 61.893 | 21.142 | 28.107 |
| 50 | 0.5 | 0.1 | 1.0 | COS | - | 0.915 | 3.795 | 0.851 | 5.820 | 62.762 | 61.888 | 21.142 | 28.107 |
| 50 | 0.5 | 0.1 | 1.0 | RBF | 10.0 | 0.915 | 3.795 | 0.850 | 5.820 | 62.762 | 61.893 | 21.142 | 28.107 |
| 50 | 0.5 | 0.1 | 10.0 | COS | - | 0.914 | 3.793 | 0.850 | 5.819 | 62.733 | 61.885 | 21.190 | 28.264 |
| 50 | 0.5 | 0.1 | 10.0 | RBF | 10.0 | 0.914 | 3.793 | 0.850 | 5.819 | 62.733 | 61.890 | 21.190 | 28.257 |
| 50 | 0.5 | 0.1 | 100.0 | COS | - | 0.910 | 3.742 | 0.843 | 5.789 | 62.134 | 61.518 | 22.382 | 30.222 |
| 50 | 0.5 | 0.1 | 100.0 | RBF | 10.0 | 0.910 | 3.751 | 0.844 | 5.792 | 62.246 | 61.557 | 22.119 | 29.947 |
| 50 | 0.5 | 1.0 | 0.0 | COS | - | 0.916 | 3.801 | 0.851 | 5.828 | 62.567 | 61.988 | 20.746 | 27.172 |
| 50 | 0.5 | 1.0 | 0.0 | RBF | 10.0 | 0.916 | 3.801 | 0.851 | 5.828 | 62.567 | 61.988 | 20.746 | 27.172 |
| 50 | 0.5 | 1.0 | 1.0 | COS | - | 0.916 | 3.802 | 0.852 | 5.830 | 62.543 | 61.988 | 20.698 | 27.020 |
| 50 | 0.5 | 1.0 | 1.0 | RBF | 10.0 | 0.916 | 3.800 | 0.851 | 5.828 | 62.538 | 61.978 | 20.710 | 27.118 |
| 50 | 0.5 | 1.0 | 10.0 | COS | - | 0.917 | 3.808 | 0.852 | 5.841 | 62.358 | 62.034 | 20.285 | 26.573 |
| 50 | 0.5 | 1.0 | 10.0 | RBF | 10.0 | 0.917 | 3.807 | 0.852 | 5.842 | 62.416 | 62.056 | 20.374 | 26.645 |
| 50 | 0.5 | 1.0 | 100.0 | COS | - | 0.911 | 3.756 | 0.844 | 5.795 | 62.075 | 61.583 | 21.533 | 29.392 |
| 50 | 0.5 | 1.0 | 100.0 | RBF | 10.0 | 0.913 | 3.772 | 0.847 | 5.807 | 62.037 | 61.693 | 20.867 | 28.119 |
| 50 | 1.0 | 0.1 | 0.0 | COS | - | 0.967 | 3.854 | 0.910 | 4.851 | 71.235 | 53.369 | 7.623 | 13.961 |
| 50 | 1.0 | 0.1 | 0.0 | RBF | 10.0 | 0.967 | 3.854 | 0.910 | 4.851 | 71.235 | 53.369 | 7.623 | 13.961 |
| 50 | 1.0 | 0.1 | 1.0 | COS | - | 0.965 | 3.839 | 0.907 | 4.864 | 71.109 | 53.513 | 8.285 | 14.805 |
| 50 | 1.0 | 0.1 | 1.0 | RBF | 10.0 | 0.965 | 3.841 | 0.907 | 4.863 | 71.103 | 53.498 | 8.172 | 14.693 |
| 50 | 1.0 | 0.1 | 10.0 | COS | - | 0.948 | 3.704 | 0.882 | 4.869 | 69.998 | 53.091 | 18.854 | 28.549 |
| 50 | 1.0 | 0.1 | 10.0 | RBF | 10.0 | 0.951 | 3.723 | 0.886 | 4.878 | 70.246 | 53.250 | 17.628 | 26.520 |
| 50 | 1.0 | 0.1 | 100.0 | COS | - | 0.909 | 3.216 | 0.819 | 4.599 | 62.149 | 49.603 | 30.909 | 44.194 |
| 50 | 1.0 | 0.1 | 100.0 | RBF | 10.0 | 0.915 | 3.275 | 0.827 | 4.644 | 63.264 | 50.166 | 29.751 | 42.998 |
| 50 | 1.0 | 1.0 | 0.0 | COS | - | 0.966 | 3.848 | 0.909 | 4.856 | 71.172 | 53.415 | 7.726 | 14.200 |
| 50 | 1.0 | 1.0 | 0.0 | RBF | 10.0 | 0.966 | 3.848 | 0.909 | 4.856 | 71.172 | 53.415 | 7.726 | 14.200 |
| 50 | 1.0 | 1.0 | 1.0 | COS | - | 0.964 | 3.838 | 0.906 | 4.865 | 71.089 | 53.520 | 8.249 | 14.718 |
| 50 | 1.0 | 1.0 | 1.0 | RBF | 10.0 | 0.964 | 3.840 | 0.907 | 4.866 | 71.099 | 53.525 | 8.149 | 14.661 |
| 50 | 1.0 | 1.0 | 10.0 | COS | - | 0.948 | 3.698 | 0.883 | 4.850 | 69.920 | 52.845 | 19.415 | 29.478 |
| 50 | 1.0 | 1.0 | 10.0 | RBF | 10.0 | 0.951 | 3.720 | 0.887 | 4.862 | 70.246 | 53.047 | 18.395 | 27.633 |
| 50 | 1.0 | 1.0 | 100.0 | COS | - | 0.912 | 3.243 | 0.822 | 4.623 | 62.723 | 49.890 | 30.505 | 43.681 |
| 50 | 1.0 | 1.0 | 100.0 | RBF | 10.0 | 0.914 | 3.263 | 0.825 | 4.633 | 63.099 | 50.051 | 30.070 | 43.690 |

The columns corresponding to "$l$", "$\alpha$", "$\beta$", "$\gamma$", "usim", and "$\sigma$" have the latent dimension, weighting factor, latent vector regularization parameter, cell line similarity regularization parameter, cell line similarity function, and parameter for rbf cell line similarity, respectively, for pLETORg.

**TABLE S13:** pLETORg Performance on New and Known Drugs ($\theta$ = 5)

| $l$ | $\alpha$ | $\beta$ | $\gamma$ | usim | $\sigma$ | AP@5 | AH@5 | AP@10 | AH@10 | AT@5% | AT@10% | NT@5% | NT@10% |
|---|---|---|---|---|---|---|---|---|---|---|---|---|---|
| 5 | 0.0 | 0.1 | 0.0 | COS | - | 0.996 | 4.965 | 0.995 | 9.914 | 47.800 | 56.938 | 44.523 | 54.579 |
| 5 | 0.0 | 0.1 | 0.0 | RBF | 10.0 | 0.996 | 4.965 | 0.995 | 9.914 | 47.800 | 56.938 | 44.523 | 54.579 |
| 5 | 0.0 | 0.1 | 1.0 | COS | - | 0.996 | 4.965 | 0.995 | 9.914 | 47.800 | 56.938 | 44.542 | 54.579 |
| 5 | 0.0 | 0.1 | 1.0 | RBF | 10.0 | 0.996 | 4.965 | 0.995 | 9.914 | 47.800 | 56.938 | 44.542 | 54.579 |
| 5 | 0.0 | 0.1 | 10.0 | COS | - | 0.996 | 4.965 | 0.995 | 9.914 | 47.790 | 56.928 | 44.542 | 54.569 |
| 5 | 0.0 | 0.1 | 10.0 | RBF | 10.0 | 0.996 | 4.965 | 0.995 | 9.914 | 47.790 | 56.926 | 44.542 | 54.560 |
| 5 | 0.0 | 0.1 | 100.0 | COS | - | 0.996 | 4.965 | 0.995 | 9.913 | 47.747 | 56.865 | 44.429 | 54.453 |
| 5 | 0.0 | 0.1 | 100.0 | RBF | 10.0 | 0.996 | 4.965 | 0.995 | 9.913 | 47.737 | 56.867 | 44.429 | 54.464 |
| 5 | 0.0 | 1.0 | 0.0 | COS | - | 0.996 | 4.965 | 0.995 | 9.914 | 47.796 | 56.936 | 44.523 | 54.565 |
| 5 | 0.0 | 1.0 | 0.0 | RBF | 10.0 | 0.996 | 4.965 | 0.995 | 9.914 | 47.796 | 56.936 | 44.523 | 54.565 |
| 5 | 0.0 | 1.0 | 1.0 | COS | - | 0.996 | 4.965 | 0.995 | 9.914 | 47.800 | 56.938 | 44.542 | 54.579 |
| 5 | 0.0 | 1.0 | 1.0 | RBF | 10.0 | 0.996 | 4.965 | 0.995 | 9.914 | 47.800 | 56.936 | 44.542 | 54.565 |
| 5 | 0.0 | 1.0 | 10.0 | COS | - | 0.997 | 4.977 | 0.997 | 9.937 | 52.906 | 59.764 | 27.191 | 33.642 |
| 5 | 0.0 | 1.0 | 10.0 | RBF | 10.0 | 0.997 | 4.977 | 0.997 | 9.937 | 52.906 | 59.761 | 27.191 | 33.633 |
| 5 | 0.0 | 1.0 | 100.0 | COS | - | 0.996 | 4.965 | 0.995 | 9.913 | 47.747 | 56.865 | 44.429 | 54.453 |
| 5 | 0.0 | 1.0 | 100.0 | RBF | 10.0 | 0.996 | 4.965 | 0.995 | 9.913 | 47.737 | 56.867 | 44.429 | 54.464 |
| 5 | 0.05 | 0.1 | 0.0 | COS | - | 0.997 | 4.976 | 0.996 | 9.935 | 56.365 | 62.799 | 27.662 | 35.451 |
| 5 | 0.05 | 0.1 | 0.0 | RBF | 10.0 | 0.997 | 4.976 | 0.996 | 9.935 | 56.365 | 62.799 | 27.662 | 35.451 |
| 5 | 0.05 | 0.1 | 1.0 | COS | - | 0.997 | 4.976 | 0.996 | 9.935 | 56.268 | 62.721 | 27.624 | 35.344 |
| 5 | 0.05 | 0.1 | 1.0 | RBF | 10.0 | 0.997 | 4.976 | 0.996 | 9.935 | 56.302 | 62.748 | 27.662 | 35.426 |
| 5 | 0.05 | 0.1 | 10.0 | COS | - | 0.997 | 4.977 | 0.997 | 9.936 | 54.080 | 60.597 | 27.210 | 33.641 |
| 5 | 0.05 | 0.1 | 10.0 | RBF | 10.0 | 0.997 | 4.977 | 0.997 | 9.936 | 54.075 | 60.609 | 27.210 | 33.647 |
| 5 | 0.05 | 0.1 | 100.0 | COS | - | 0.997 | 4.976 | 0.996 | 9.933 | 58.733 | 65.109 | 28.793 | 39.563 |
| 5 | 0.05 | 0.1 | 100.0 | RBF | 10.0 | 0.997 | 4.976 | 0.996 | 9.934 | 58.577 | 64.894 | 28.725 | 38.953 |
| 5 | 0.05 | 1.0 | 0.0 | COS | - | 0.997 | 4.977 | 0.997 | 9.936 | 54.061 | 60.599 | 27.192 | 33.620 |
| 5 | 0.05 | 1.0 | 0.0 | RBF | 10.0 | 0.997 | 4.977 | 0.997 | 9.936 | 54.061 | 60.599 | 27.192 | 33.620 |
| 5 | 0.05 | 1.0 | 1.0 | COS | - | 0.997 | 4.977 | 0.997 | 9.936 | 54.056 | 60.599 | 27.192 | 33.620 |
| 5 | 0.05 | 1.0 | 1.0 | RBF | 10.0 | 0.997 | 4.977 | 0.997 | 9.936 | 54.056 | 60.599 | 27.192 | 33.620 |
| 5 | 0.05 | 1.0 | 10.0 | COS | - | 0.997 | 4.977 | 0.997 | 9.936 | 54.022 | 60.589 | 27.192 | 33.616 |
| 5 | 0.05 | 1.0 | 10.0 | RBF | 10.0 | 0.997 | 4.977 | 0.997 | 9.936 | 54.027 | 60.587 | 27.192 | 33.616 |
| 5 | 0.05 | 1.0 | 100.0 | COS | - | 0.997 | 4.976 | 0.996 | 9.932 | 57.876 | 64.200 | 28.564 | 38.644 |
| 5 | 0.05 | 1.0 | 100.0 | RBF | 10.0 | 0.997 | 4.976 | 0.996 | 9.932 | 57.442 | 63.868 | 28.400 | 38.049 |
| 5 | 0.1 | 0.1 | 0.0 | COS | - | 0.996 | 4.965 | 0.995 | 9.913 | 48.185 | 57.137 | 44.518 | 54.518 |
| 5 | 0.1 | 0.1 | 0.0 | RBF | 10.0 | 0.996 | 4.965 | 0.995 | 9.913 | 48.185 | 57.137 | 44.518 | 54.518 |
| 5 | 0.1 | 0.1 | 1.0 | COS | - | 0.996 | 4.965 | 0.995 | 9.913 | 48.180 | 57.137 | 44.500 | 54.518 |
| 5 | 0.1 | 0.1 | 1.0 | RBF | 10.0 | 0.996 | 4.965 | 0.995 | 9.913 | 48.180 | 57.137 | 44.500 | 54.518 |
| 5 | 0.1 | 0.1 | 10.0 | COS | - | 0.996 | 4.965 | 0.995 | 9.914 | 48.166 | 57.140 | 44.518 | 54.507 |
| 5 | 0.1 | 0.1 | 10.0 | RBF | 10.0 | 0.996 | 4.965 | 0.995 | 9.914 | 48.161 | 57.140 | 44.500 | 54.507 |
| 5 | 0.1 | 0.1 | 100.0 | COS | - | 0.996 | 4.965 | 0.995 | 9.913 | 48.161 | 57.091 | 44.692 | 54.537 |
| 5 | 0.1 | 0.1 | 100.0 | RBF | 10.0 | 0.996 | 4.965 | 0.995 | 9.913 | 48.166 | 57.096 | 44.692 | 54.542 |
| 5 | 0.1 | 1.0 | 0.0 | COS | - | 0.996 | 4.965 | 0.995 | 9.913 | 48.185 | 57.137 | 44.518 | 54.518 |
| 5 | 0.1 | 1.0 | 0.0 | RBF | 10.0 | 0.996 | 4.965 | 0.995 | 9.913 | 48.185 | 57.137 | 44.518 | 54.518 |
| 5 | 0.1 | 1.0 | 1.0 | COS | - | 0.996 | 4.965 | 0.995 | 9.913 | 48.180 | 57.137 | 44.500 | 54.518 |
| 5 | 0.1 | 1.0 | 1.0 | RBF | 10.0 | 0.996 | 4.965 | 0.995 | 9.913 | 48.180 | 57.137 | 44.500 | 54.518 |
| 5 | 0.1 | 1.0 | 10.0 | COS | - | 0.996 | 4.965 | 0.995 | 9.914 | 48.166 | 57.140 | 44.518 | 54.507 |
| 5 | 0.1 | 1.0 | 10.0 | RBF | 10.0 | 0.996 | 4.965 | 0.995 | 9.914 | 48.161 | 57.140 | 44.500 | 54.513 |
| 5 | 0.1 | 1.0 | 100.0 | COS | - | 0.996 | 4.965 | 0.995 | 9.913 | 48.161 | 57.089 | 44.692 | 54.537 |
| 5 | 0.1 | 1.0 | 100.0 | RBF | 10.0 | 0.996 | 4.965 | 0.995 | 9.913 | 48.166 | 57.096 | 44.692 | 54.542 |
| 5 | 0.5 | 0.1 | 0.0 | COS | - | 0.996 | 4.965 | 0.995 | 9.912 | 49.822 | 57.968 | 45.399 | 54.836 |
| 5 | 0.5 | 0.1 | 0.0 | RBF | 10.0 | 0.996 | 4.965 | 0.995 | 9.912 | 49.822 | 57.968 | 45.399 | 54.836 |
| 5 | 0.5 | 0.1 | 1.0 | COS | - | 0.996 | 4.965 | 0.995 | 9.912 | 49.822 | 57.961 | 45.399 | 54.836 |
| 5 | 0.5 | 0.1 | 1.0 | RBF | 10.0 | 0.996 | 4.965 | 0.995 | 9.912 | 49.822 | 57.961 | 45.399 | 54.836 |
| 5 | 0.5 | 0.1 | 10.0 | COS | - | 0.996 | 4.965 | 0.995 | 9.911 | 49.842 | 57.966 | 45.465 | 54.836 |
| 5 | 0.5 | 0.1 | 10.0 | RBF | 10.0 | 0.996 | 4.965 | 0.995 | 9.911 | 49.842 | 57.966 | 45.465 | 54.836 |
| 5 | 0.5 | 0.1 | 100.0 | COS | - | 0.996 | 4.965 | 0.995 | 9.910 | 49.817 | 57.920 | 45.443 | 54.707 |
| 5 | 0.5 | 0.1 | 100.0 | RBF | 10.0 | 0.996 | 4.965 | 0.995 | 9.910 | 49.817 | 57.929 | 45.407 | 54.748 |
| 5 | 0.5 | 1.0 | 0.0 | COS | - | 0.996 | 4.965 | 0.995 | 9.912 | 49.822 | 57.966 | 45.399 | 54.836 |

Continued on next page

TABLE S13 – continued from previous page

| $l$ | $\alpha$ | $\beta$ | $\gamma$ | usim | $\sigma$ | AP@5 | AH@5 | AP@10 | AH@10 | AT@5% | AT@10% | NT@5% | NT@10% |
|---|---|---|---|---|---|---|---|---|---|---|---|---|---|
| 5 | 0.5 | 1.0 | 0.0 | RBF | 10.0 | 0.996 | 4.965 | 0.995 | 9.912 | 49.822 | 57.966 | 45.399 | 54.836 |
| 5 | 0.5 | 1.0 | 1.0 | COS | - | 0.996 | 4.965 | 0.995 | 9.912 | 49.822 | 57.961 | 45.399 | 54.836 |
| 5 | 0.5 | 1.0 | 1.0 | RBF | 10.0 | 0.996 | 4.965 | 0.995 | 9.912 | 49.822 | 57.961 | 45.399 | 54.836 |
| 5 | 0.5 | 1.0 | 10.0 | COS | - | 0.996 | 4.965 | 0.995 | 9.911 | 49.842 | 57.966 | 45.465 | 54.836 |
| 5 | 0.5 | 1.0 | 10.0 | RBF | 10.0 | 0.996 | 4.965 | 0.995 | 9.911 | 49.842 | 57.966 | 45.465 | 54.836 |
| 5 | 0.5 | 1.0 | 100.0 | COS | - | 0.996 | 4.965 | 0.995 | 9.910 | 49.817 | 57.920 | 45.443 | 54.707 |
| 5 | 0.5 | 1.0 | 100.0 | RBF | 10.0 | 0.996 | 4.965 | 0.995 | 9.910 | 49.817 | 57.929 | 45.407 | 54.748 |
| 5 | 1.0 | 0.1 | 0.0 | COS | - | 0.960 | 4.659 | 0.946 | 9.129 | 47.766 | 50.965 | 40.496 | 45.096 |
| 5 | 1.0 | 0.1 | 0.0 | RBF | 10.0 | 0.960 | 4.659 | 0.946 | 9.129 | 47.766 | 50.965 | 40.496 | 45.096 |
| 5 | 1.0 | 0.1 | 1.0 | COS | - | 0.962 | 4.670 | 0.948 | 9.152 | 48.073 | 51.274 | 40.583 | 45.399 |
| 5 | 1.0 | 0.1 | 1.0 | RBF | 10.0 | 0.961 | 4.669 | 0.948 | 9.149 | 48.049 | 51.213 | 40.583 | 45.333 |
| 5 | 1.0 | 0.1 | 10.0 | COS | - | 0.968 | 4.718 | 0.955 | 9.222 | 49.067 | 52.246 | 41.149 | 46.280 |
| 5 | 1.0 | 0.1 | 10.0 | RBF | 10.0 | 0.967 | 4.712 | 0.954 | 9.213 | 48.994 | 52.151 | 41.024 | 46.130 |
| 5 | 1.0 | 0.1 | 100.0 | COS | - | 0.980 | 4.833 | 0.973 | 9.501 | 52.521 | 55.756 | 44.319 | 48.895 |
| 5 | 1.0 | 0.1 | 100.0 | RBF | 10.0 | 0.980 | 4.831 | 0.972 | 9.473 | 52.307 | 55.340 | 44.207 | 48.730 |
| 5 | 1.0 | 1.0 | 0.0 | COS | - | 0.963 | 4.676 | 0.949 | 9.155 | 48.292 | 51.384 | 40.704 | 45.492 |
| 5 | 1.0 | 1.0 | 0.0 | RBF | 10.0 | 0.963 | 4.676 | 0.949 | 9.155 | 48.292 | 51.384 | 40.704 | 45.492 |
| 5 | 1.0 | 1.0 | 1.0 | COS | - | 0.964 | 4.683 | 0.950 | 9.166 | 48.395 | 51.525 | 40.861 | 45.618 |
| 5 | 1.0 | 1.0 | 1.0 | RBF | 10.0 | 0.963 | 4.683 | 0.950 | 9.166 | 48.400 | 51.515 | 40.861 | 45.602 |
| 5 | 1.0 | 1.0 | 10.0 | COS | - | 0.969 | 4.729 | 0.956 | 9.240 | 49.408 | 52.558 | 41.399 | 46.530 |
| 5 | 1.0 | 1.0 | 10.0 | RBF | 10.0 | 0.968 | 4.724 | 0.956 | 9.232 | 49.272 | 52.438 | 41.215 | 46.418 |
| 5 | 1.0 | 1.0 | 100.0 | COS | - | 0.981 | 4.835 | 0.973 | 9.503 | 52.667 | 55.822 | 44.323 | 49.057 |
| 5 | 1.0 | 1.0 | 100.0 | RBF | 10.0 | 0.980 | 4.830 | 0.973 | 9.474 | 52.321 | 55.420 | 44.134 | 48.756 |
| 10 | 0.0 | 0.1 | 0.0 | COS | - | 0.998 | 4.976 | 0.997 | 9.935 | 51.177 | 59.739 | 34.656 | 50.379 |
| 10 | 0.0 | 0.1 | 0.0 | RBF | 10.0 | 0.998 | 4.976 | 0.997 | 9.935 | 51.177 | 59.739 | 34.656 | 50.379 |
| 10 | 0.0 | 0.1 | 1.0 | COS | - | 0.998 | 4.976 | 0.997 | 9.934 | 51.186 | 59.732 | 34.730 | 50.379 |
| 10 | 0.0 | 0.1 | 1.0 | RBF | 10.0 | 0.998 | 4.976 | 0.997 | 9.934 | 51.186 | 59.734 | 34.730 | 50.379 |
| 10 | 0.0 | 0.1 | 10.0 | COS | - | 0.998 | 4.976 | 0.997 | 9.934 | 51.186 | 59.715 | 34.804 | 50.386 |
| 10 | 0.0 | 0.1 | 10.0 | RBF | 10.0 | 0.998 | 4.976 | 0.997 | 9.934 | 51.177 | 59.718 | 34.786 | 50.386 |
| 10 | 0.0 | 0.1 | 100.0 | COS | - | 0.998 | 4.977 | 0.997 | 9.934 | 51.172 | 59.705 | 34.988 | 50.570 |
| 10 | 0.0 | 0.1 | 100.0 | RBF | 10.0 | 0.998 | 4.977 | 0.997 | 9.934 | 51.176 | 59.708 | 34.988 | 50.505 |
| 10 | 0.0 | 1.0 | 0.0 | COS | - | 0.998 | 4.976 | 0.997 | 9.934 | 51.181 | 59.734 | 34.693 | 50.379 |
| 10 | 0.0 | 1.0 | 0.0 | RBF | 10.0 | 0.998 | 4.976 | 0.997 | 9.934 | 51.181 | 59.734 | 34.693 | 50.379 |
| 10 | 0.0 | 1.0 | 1.0 | COS | - | 0.998 | 4.976 | 0.997 | 9.934 | 51.186 | 59.732 | 34.730 | 50.379 |
| 10 | 0.0 | 1.0 | 1.0 | RBF | 10.0 | 0.998 | 4.976 | 0.997 | 9.934 | 51.186 | 59.732 | 34.730 | 50.379 |
| 10 | 0.0 | 1.0 | 10.0 | COS | - | 0.998 | 4.976 | 0.997 | 9.934 | 51.186 | 59.715 | 34.804 | 50.386 |
| 10 | 0.0 | 1.0 | 10.0 | RBF | 10.0 | 0.998 | 4.976 | 0.997 | 9.934 | 51.181 | 59.715 | 34.804 | 50.386 |
| 10 | 0.0 | 1.0 | 100.0 | COS | - | 0.998 | 4.977 | 0.997 | 9.934 | 51.172 | 59.705 | 34.988 | 50.570 |
| 10 | 0.0 | 1.0 | 100.0 | RBF | 10.0 | 0.998 | 4.977 | 0.997 | 9.934 | 51.176 | 59.708 | 34.988 | 50.505 |
| 10 | 0.05 | 0.1 | 0.0 | COS | - | 0.998 | 4.977 | 0.997 | 9.936 | 51.299 | 59.876 | 34.548 | 50.211 |
| 10 | 0.05 | 0.1 | 0.0 | RBF | 10.0 | 0.998 | 4.977 | 0.997 | 9.936 | 51.299 | 59.876 | 34.548 | 50.211 |
| 10 | 0.05 | 0.1 | 1.0 | COS | - | 0.998 | 4.977 | 0.997 | 9.936 | 51.303 | 59.876 | 34.585 | 50.211 |
| 10 | 0.05 | 0.1 | 1.0 | RBF | 10.0 | 0.998 | 4.977 | 0.997 | 9.936 | 51.303 | 59.876 | 34.585 | 50.211 |
| 10 | 0.05 | 0.1 | 10.0 | COS | - | 0.998 | 4.977 | 0.997 | 9.936 | 51.304 | 59.859 | 34.696 | 50.211 |
| 10 | 0.05 | 0.1 | 10.0 | RBF | 10.0 | 0.998 | 4.977 | 0.997 | 9.936 | 51.304 | 59.859 | 34.696 | 50.211 |
| 10 | 0.05 | 0.1 | 100.0 | COS | - | 0.998 | 4.977 | 0.997 | 9.934 | 51.318 | 59.825 | 34.833 | 50.363 |
| 10 | 0.05 | 0.1 | 100.0 | RBF | 10.0 | 0.998 | 4.977 | 0.997 | 9.934 | 51.323 | 59.839 | 34.850 | 50.338 |
| 10 | 0.05 | 1.0 | 0.0 | COS | - | 0.998 | 4.977 | 0.997 | 9.936 | 51.303 | 59.876 | 34.585 | 50.211 |
| 10 | 0.05 | 1.0 | 0.0 | RBF | 10.0 | 0.998 | 4.977 | 0.997 | 9.936 | 51.303 | 59.876 | 34.585 | 50.211 |
| 10 | 0.05 | 1.0 | 1.0 | COS | - | 0.998 | 4.977 | 0.997 | 9.936 | 51.303 | 59.876 | 34.585 | 50.211 |
| 10 | 0.05 | 1.0 | 1.0 | RBF | 10.0 | 0.998 | 4.977 | 0.997 | 9.936 | 51.303 | 59.876 | 34.585 | 50.211 |
| 10 | 0.05 | 1.0 | 10.0 | COS | - | 0.998 | 4.977 | 0.997 | 9.936 | 51.304 | 59.859 | 34.696 | 50.211 |
| 10 | 0.05 | 1.0 | 10.0 | RBF | 10.0 | 0.998 | 4.977 | 0.997 | 9.936 | 51.304 | 59.859 | 34.696 | 50.211 |
| 10 | 0.05 | 1.0 | 100.0 | COS | - | 0.998 | 4.977 | 0.997 | 9.934 | 51.318 | 59.825 | 34.833 | 50.377 |
| 10 | 0.05 | 1.0 | 100.0 | RBF | 10.0 | 0.998 | 4.977 | 0.997 | 9.934 | 51.323 | 59.839 | 34.850 | 50.338 |
| 10 | 0.1 | 0.1 | 0.0 | COS | - | 0.998 | 4.977 | 0.997 | 9.937 | 51.459 | 60.005 | 34.310 | 50.096 |
| 10 | 0.1 | 0.1 | 0.0 | RBF | 10.0 | 0.998 | 4.977 | 0.997 | 9.937 | 51.459 | 60.005 | 34.310 | 50.096 |
| 10 | 0.1 | 0.1 | 1.0 | COS | - | 0.998 | 4.977 | 0.997 | 9.937 | 51.464 | 60.002 | 34.345 | 50.109 |

Continued on next page

TABLE S13 – continued from previous page

| $l$ | $\alpha$ | $\beta$ | $\gamma$ | usim | $\sigma$ | AP@5 | AH@5 | AP@10 | AH@10 | AT@5% | AT@10% | NT@5% | NT@10% |
|---|---|---|---|---|---|---|---|---|---|---|---|---|---|
| 10 | 0.1 | 0.1 | 1.0 | RBF | 10.0 | 0.998 | 4.977 | 0.997 | 9.937 | 51.464 | 60.002 | 34.345 | 50.096 |
| 10 | 0.1 | 0.1 | 10.0 | COS | - | 0.998 | 4.977 | 0.997 | 9.937 | 51.479 | 59.995 | 34.413 | 50.129 |
| 10 | 0.1 | 0.1 | 10.0 | RBF | 10.0 | 0.998 | 4.977 | 0.997 | 9.937 | 51.474 | 59.995 | 34.376 | 50.129 |
| 10 | 0.1 | 0.1 | 100.0 | COS | - | 0.998 | 4.977 | 0.997 | 9.936 | 51.450 | 59.963 | 34.744 | 50.187 |
| 10 | 0.1 | 0.1 | 100.0 | RBF | 10.0 | 0.998 | 4.977 | 0.997 | 9.936 | 51.440 | 59.973 | 34.678 | 50.165 |
| 10 | 0.1 | 1.0 | 0.0 | COS | - | 0.998 | 4.977 | 0.997 | 9.937 | 51.464 | 60.002 | 34.345 | 50.096 |
| 10 | 0.1 | 1.0 | 0.0 | RBF | 10.0 | 0.998 | 4.977 | 0.997 | 9.937 | 51.464 | 60.002 | 34.345 | 50.096 |
| 10 | 0.1 | 1.0 | 1.0 | COS | - | 0.998 | 4.977 | 0.997 | 9.937 | 51.464 | 60.002 | 34.345 | 50.109 |
| 10 | 0.1 | 1.0 | 1.0 | RBF | 10.0 | 0.998 | 4.977 | 0.997 | 9.937 | 51.464 | 60.002 | 34.345 | 50.096 |
| 10 | 0.1 | 1.0 | 10.0 | COS | - | 0.998 | 4.977 | 0.997 | 9.937 | 51.474 | 59.993 | 34.413 | 50.129 |
| 10 | 0.1 | 1.0 | 10.0 | RBF | 10.0 | 0.998 | 4.977 | 0.997 | 9.937 | 51.474 | 59.995 | 34.376 | 50.129 |
| 10 | 0.1 | 1.0 | 100.0 | COS | - | 0.998 | 4.977 | 0.997 | 9.936 | 51.450 | 59.961 | 34.744 | 50.187 |
| 10 | 0.1 | 1.0 | 100.0 | RBF | 10.0 | 0.998 | 4.977 | 0.997 | 9.936 | 51.440 | 59.973 | 34.678 | 50.165 |
| 10 | 0.5 | 0.1 | 0.0 | COS | - | 0.998 | 4.979 | 0.997 | 9.935 | 52.872 | 60.933 | 33.078 | 48.144 |
| 10 | 0.5 | 0.1 | 0.0 | RBF | 10.0 | 0.998 | 4.979 | 0.997 | 9.935 | 52.872 | 60.933 | 33.078 | 48.144 |
| 10 | 0.5 | 0.1 | 1.0 | COS | - | 0.998 | 4.979 | 0.997 | 9.935 | 52.872 | 60.936 | 33.078 | 48.144 |
| 10 | 0.5 | 0.1 | 1.0 | RBF | 10.0 | 0.998 | 4.979 | 0.997 | 9.935 | 52.872 | 60.936 | 33.078 | 48.144 |
| 10 | 0.5 | 0.1 | 10.0 | COS | - | 0.998 | 4.979 | 0.997 | 9.936 | 52.872 | 60.930 | 33.142 | 48.153 |
| 10 | 0.5 | 0.1 | 10.0 | RBF | 10.0 | 0.998 | 4.979 | 0.997 | 9.936 | 52.877 | 60.928 | 33.142 | 48.153 |
| 10 | 0.5 | 0.1 | 100.0 | COS | - | 0.998 | 4.979 | 0.997 | 9.936 | 52.833 | 60.906 | 33.391 | 48.236 |
| 10 | 0.5 | 0.1 | 100.0 | RBF | 10.0 | 0.998 | 4.979 | 0.997 | 9.935 | 52.833 | 60.914 | 33.355 | 48.223 |
| 10 | 0.5 | 1.0 | 0.0 | COS | - | 0.998 | 4.979 | 0.997 | 9.935 | 52.872 | 60.933 | 33.078 | 48.144 |
| 10 | 0.5 | 1.0 | 0.0 | RBF | 10.0 | 0.998 | 4.979 | 0.997 | 9.935 | 52.872 | 60.933 | 33.078 | 48.144 |
| 10 | 0.5 | 1.0 | 1.0 | COS | - | 0.998 | 4.979 | 0.997 | 9.935 | 52.872 | 60.936 | 33.078 | 48.144 |
| 10 | 0.5 | 1.0 | 1.0 | RBF | 10.0 | 0.998 | 4.979 | 0.997 | 9.935 | 52.872 | 60.936 | 33.078 | 48.144 |
| 10 | 0.5 | 1.0 | 10.0 | COS | - | 0.998 | 4.979 | 0.997 | 9.936 | 52.872 | 60.930 | 33.142 | 48.153 |
| 10 | 0.5 | 1.0 | 10.0 | RBF | 10.0 | 0.998 | 4.979 | 0.997 | 9.936 | 52.877 | 60.930 | 33.142 | 48.153 |
| 10 | 0.5 | 1.0 | 100.0 | COS | - | 0.998 | 4.979 | 0.997 | 9.936 | 52.838 | 60.906 | 33.391 | 48.243 |
| 10 | 0.5 | 1.0 | 100.0 | RBF | 10.0 | 0.998 | 4.979 | 0.997 | 9.935 | 52.833 | 60.914 | 33.355 | 48.223 |
| 10 | 1.0 | 0.1 | 0.0 | COS | - | 0.964 | 4.688 | 0.952 | 9.221 | 48.171 | 48.097 | 36.147 | 40.119 |
| 10 | 1.0 | 0.1 | 0.0 | RBF | 10.0 | 0.964 | 4.688 | 0.952 | 9.221 | 48.171 | 48.097 | 36.147 | 40.119 |
| 10 | 1.0 | 0.1 | 1.0 | COS | - | 0.967 | 4.700 | 0.954 | 9.247 | 48.828 | 48.833 | 36.451 | 40.566 |
| 10 | 1.0 | 0.1 | 1.0 | RBF | 10.0 | 0.966 | 4.699 | 0.954 | 9.244 | 48.823 | 48.828 | 36.461 | 40.550 |
| 10 | 1.0 | 0.1 | 10.0 | COS | - | 0.973 | 4.748 | 0.961 | 9.330 | 51.259 | 51.225 | 37.423 | 41.744 |
| 10 | 1.0 | 0.1 | 10.0 | RBF | 10.0 | 0.973 | 4.747 | 0.961 | 9.328 | 51.206 | 51.191 | 37.429 | 41.705 |
| 10 | 1.0 | 0.1 | 100.0 | COS | - | 0.983 | 4.842 | 0.975 | 9.546 | 57.233 | 57.591 | 39.206 | 45.555 |
| 10 | 1.0 | 0.1 | 100.0 | RBF | 10.0 | 0.983 | 4.841 | 0.975 | 9.537 | 57.004 | 57.330 | 39.157 | 45.410 |
| 10 | 1.0 | 1.0 | 0.0 | COS | - | 0.967 | 4.703 | 0.954 | 9.245 | 48.979 | 48.860 | 36.186 | 40.491 |
| 10 | 1.0 | 1.0 | 0.0 | RBF | 10.0 | 0.967 | 4.703 | 0.954 | 9.245 | 48.979 | 48.860 | 36.186 | 40.491 |
| 10 | 1.0 | 1.0 | 1.0 | COS | - | 0.968 | 4.715 | 0.956 | 9.265 | 49.676 | 49.530 | 36.763 | 40.747 |
| 10 | 1.0 | 1.0 | 1.0 | RBF | 10.0 | 0.968 | 4.713 | 0.956 | 9.264 | 49.632 | 49.476 | 36.700 | 40.797 |
| 10 | 1.0 | 1.0 | 10.0 | COS | - | 0.975 | 4.761 | 0.963 | 9.350 | 51.971 | 51.976 | 37.879 | 41.993 |
| 10 | 1.0 | 1.0 | 10.0 | RBF | 10.0 | 0.974 | 4.756 | 0.962 | 9.344 | 51.737 | 51.739 | 37.721 | 41.943 |
| 10 | 1.0 | 1.0 | 100.0 | COS | - | 0.984 | 4.854 | 0.977 | 9.564 | 57.598 | 57.988 | 39.404 | 45.730 |
| 10 | 1.0 | 1.0 | 100.0 | RBF | 10.0 | 0.983 | 4.844 | 0.975 | 9.537 | 57.033 | 57.386 | 39.109 | 45.325 |
| 15 | 0.0 | 0.1 | 0.0 | COS | - | 0.999 | 4.987 | 0.999 | 9.955 | 51.864 | 59.956 | 15.553 | 36.200 |
| 15 | 0.0 | 0.1 | 0.0 | RBF | 10.0 | 0.999 | 4.987 | 0.999 | 9.955 | 51.864 | 59.956 | 15.553 | 36.200 |
| 15 | 0.0 | 0.1 | 1.0 | COS | - | 0.999 | 4.987 | 0.999 | 9.955 | 51.864 | 59.959 | 15.553 | 36.200 |
| 15 | 0.0 | 0.1 | 1.0 | RBF | 10.0 | 0.999 | 4.987 | 0.999 | 9.955 | 51.864 | 59.959 | 15.553 | 36.200 |
| 15 | 0.0 | 0.1 | 10.0 | COS | - | 0.999 | 4.987 | 0.999 | 9.955 | 51.854 | 59.961 | 15.588 | 36.213 |
| 15 | 0.0 | 0.1 | 10.0 | RBF | 10.0 | 0.999 | 4.987 | 0.999 | 9.955 | 51.864 | 59.966 | 15.588 | 36.213 |
| 15 | 0.0 | 0.1 | 100.0 | COS | - | 0.999 | 4.988 | 0.999 | 9.954 | 51.795 | 59.912 | 15.802 | 36.447 |
| 15 | 0.0 | 0.1 | 100.0 | RBF | 10.0 | 0.999 | 4.988 | 0.999 | 9.954 | 51.834 | 59.920 | 15.755 | 36.299 |
| 15 | 0.0 | 1.0 | 0.0 | COS | - | 0.999 | 4.987 | 0.999 | 9.955 | 51.854 | 59.956 | 15.413 | 36.076 |
| 15 | 0.0 | 1.0 | 0.0 | RBF | 10.0 | 0.999 | 4.987 | 0.999 | 9.955 | 51.854 | 59.956 | 15.413 | 36.076 |
| 15 | 0.0 | 1.0 | 1.0 | COS | - | 0.999 | 4.987 | 0.999 | 9.955 | 51.854 | 59.961 | 15.413 | 36.076 |
| 15 | 0.0 | 1.0 | 1.0 | RBF | 10.0 | 0.999 | 4.987 | 0.999 | 9.955 | 51.854 | 59.961 | 15.413 | 36.076 |
| 15 | 0.0 | 1.0 | 10.0 | COS | - | 0.999 | 4.987 | 0.999 | 9.955 | 51.854 | 59.961 | 15.460 | 36.076 |

Continued on next page

TABLE S13 – continued from previous page

| $l$ | $\alpha$ | $\beta$ | $\gamma$ | usim | $\sigma$ | AP@5 | AH@5 | AP@10 | AH@10 | AT@5% | AT@10% | NT@5% | NT@10% |
|---|---|---|---|---|---|---|---|---|---|---|---|---|---|
| 15 | 0.0 | 1.0 | 10.0 | RBF | 10.0 | 0.999 | 4.987 | 0.999 | 9.955 | 51.859 | 59.963 | 15.460 | 36.076 |
| 15 | 0.0 | 1.0 | 100.0 | COS | - | 0.999 | 4.988 | 0.999 | 9.954 | 51.849 | 59.912 | 15.774 | 36.317 |
| 15 | 0.0 | 1.0 | 100.0 | RBF | 10.0 | 0.999 | 4.988 | 0.999 | 9.954 | 51.834 | 59.917 | 15.755 | 36.299 |
| 15 | 0.05 | 0.1 | 0.0 | COS | - | 0.999 | 4.988 | 0.999 | 9.955 | 51.995 | 60.000 | 15.277 | 35.564 |
| 15 | 0.05 | 0.1 | 0.0 | RBF | 10.0 | 0.999 | 4.988 | 0.999 | 9.955 | 51.995 | 60.000 | 15.277 | 35.564 |
| 15 | 0.05 | 0.1 | 1.0 | COS | - | 0.999 | 4.988 | 0.999 | 9.955 | 52.000 | 59.997 | 15.277 | 35.554 |
| 15 | 0.05 | 0.1 | 1.0 | RBF | 10.0 | 0.999 | 4.988 | 0.999 | 9.955 | 52.000 | 59.997 | 15.277 | 35.554 |
| 15 | 0.05 | 0.1 | 10.0 | COS | - | 0.999 | 4.988 | 0.999 | 9.955 | 52.020 | 59.998 | 15.379 | 35.581 |
| 15 | 0.05 | 0.1 | 10.0 | RBF | 10.0 | 0.999 | 4.988 | 0.999 | 9.955 | 52.020 | 59.998 | 15.379 | 35.581 |
| 15 | 0.05 | 0.1 | 100.0 | COS | - | 0.999 | 4.988 | 0.999 | 9.954 | 51.980 | 59.983 | 15.628 | 35.861 |
| 15 | 0.05 | 0.1 | 100.0 | RBF | 10.0 | 0.999 | 4.988 | 0.999 | 9.954 | 51.985 | 59.978 | 15.606 | 35.787 |
| 15 | 0.05 | 1.0 | 0.0 | COS | - | 0.999 | 4.988 | 0.999 | 9.955 | 51.995 | 59.997 | 15.277 | 35.554 |
| 15 | 0.05 | 1.0 | 0.0 | RBF | 10.0 | 0.999 | 4.988 | 0.999 | 9.955 | 51.995 | 59.997 | 15.277 | 35.554 |
| 15 | 0.05 | 1.0 | 1.0 | COS | - | 0.999 | 4.988 | 0.999 | 9.955 | 52.000 | 59.997 | 15.277 | 35.554 |
| 15 | 0.05 | 1.0 | 1.0 | RBF | 10.0 | 0.999 | 4.988 | 0.999 | 9.955 | 52.000 | 59.997 | 15.277 | 35.554 |
| 15 | 0.05 | 1.0 | 10.0 | COS | - | 0.999 | 4.988 | 0.999 | 9.955 | 52.020 | 59.998 | 15.379 | 35.581 |
| 15 | 0.05 | 1.0 | 10.0 | RBF | 10.0 | 0.999 | 4.988 | 0.999 | 9.955 | 52.020 | 59.998 | 15.379 | 35.581 |
| 15 | 0.05 | 1.0 | 100.0 | COS | - | 0.999 | 4.988 | 0.999 | 9.954 | 51.980 | 59.983 | 15.628 | 35.875 |
| 15 | 0.05 | 1.0 | 100.0 | RBF | 10.0 | 0.999 | 4.988 | 0.999 | 9.954 | 51.985 | 59.978 | 15.606 | 35.787 |
| 15 | 0.1 | 0.1 | 0.0 | COS | - | 0.999 | 4.988 | 0.999 | 9.955 | 52.112 | 60.110 | 14.902 | 35.024 |
| 15 | 0.1 | 0.1 | 0.0 | RBF | 10.0 | 0.999 | 4.988 | 0.999 | 9.955 | 52.112 | 60.110 | 14.902 | 35.024 |
| 15 | 0.1 | 0.1 | 1.0 | COS | - | 0.999 | 4.988 | 0.999 | 9.955 | 52.112 | 60.105 | 14.902 | 34.988 |
| 15 | 0.1 | 0.1 | 1.0 | RBF | 10.0 | 0.999 | 4.988 | 0.999 | 9.955 | 52.112 | 60.105 | 14.902 | 34.988 |
| 15 | 0.1 | 0.1 | 10.0 | COS | - | 0.999 | 4.988 | 0.999 | 9.956 | 52.117 | 60.095 | 14.957 | 34.999 |
| 15 | 0.1 | 0.1 | 10.0 | RBF | 10.0 | 0.999 | 4.988 | 0.999 | 9.956 | 52.117 | 60.100 | 14.957 | 34.992 |
| 15 | 0.1 | 0.1 | 100.0 | COS | - | 0.999 | 4.988 | 0.999 | 9.955 | 52.097 | 60.058 | 15.405 | 35.248 |
| 15 | 0.1 | 0.1 | 100.0 | RBF | 10.0 | 0.999 | 4.988 | 0.999 | 9.955 | 52.107 | 60.049 | 15.286 | 35.211 |
| 15 | 0.1 | 1.0 | 0.0 | COS | - | 0.999 | 4.988 | 0.999 | 9.955 | 52.112 | 60.110 | 14.902 | 35.024 |
| 15 | 0.1 | 1.0 | 0.0 | RBF | 10.0 | 0.999 | 4.988 | 0.999 | 9.955 | 52.112 | 60.110 | 14.902 | 35.024 |
| 15 | 0.1 | 1.0 | 1.0 | COS | - | 0.999 | 4.988 | 0.999 | 9.955 | 52.107 | 60.105 | 14.902 | 34.988 |
| 15 | 0.1 | 1.0 | 1.0 | RBF | 10.0 | 0.999 | 4.988 | 0.999 | 9.955 | 52.107 | 60.105 | 14.902 | 34.988 |
| 15 | 0.1 | 1.0 | 10.0 | COS | - | 0.999 | 4.988 | 0.999 | 9.956 | 52.117 | 60.095 | 14.957 | 34.999 |
| 15 | 0.1 | 1.0 | 10.0 | RBF | 10.0 | 0.999 | 4.988 | 0.999 | 9.956 | 52.117 | 60.100 | 14.957 | 34.999 |
| 15 | 0.1 | 1.0 | 100.0 | COS | - | 0.999 | 4.988 | 0.999 | 9.955 | 52.097 | 60.056 | 15.405 | 35.248 |
| 15 | 0.1 | 1.0 | 100.0 | RBF | 10.0 | 0.999 | 4.988 | 0.999 | 9.955 | 52.112 | 60.049 | 15.298 | 35.211 |
| 15 | 0.5 | 0.1 | 0.0 | COS | - | 0.999 | 4.987 | 0.999 | 9.955 | 53.622 | 60.816 | 13.751 | 30.763 |
| 15 | 0.5 | 0.1 | 0.0 | RBF | 10.0 | 0.999 | 4.987 | 0.999 | 9.955 | 53.622 | 60.816 | 13.751 | 30.763 |
| 15 | 0.5 | 0.1 | 1.0 | COS | - | 0.999 | 4.987 | 0.999 | 9.955 | 53.622 | 60.821 | 13.751 | 30.799 |
| 15 | 0.5 | 0.1 | 1.0 | RBF | 10.0 | 0.999 | 4.987 | 0.999 | 9.955 | 53.622 | 60.821 | 13.751 | 30.799 |
| 15 | 0.5 | 0.1 | 10.0 | COS | - | 0.999 | 4.987 | 0.999 | 9.955 | 53.622 | 60.818 | 13.713 | 30.817 |
| 15 | 0.5 | 0.1 | 10.0 | RBF | 10.0 | 0.999 | 4.987 | 0.999 | 9.955 | 53.622 | 60.821 | 13.751 | 30.826 |
| 15 | 0.5 | 0.1 | 100.0 | COS | - | 0.999 | 4.987 | 0.999 | 9.956 | 53.647 | 60.821 | 13.871 | 30.864 |
| 15 | 0.5 | 0.1 | 100.0 | RBF | 10.0 | 0.999 | 4.987 | 0.999 | 9.956 | 53.647 | 60.816 | 13.871 | 30.845 |
| 15 | 0.5 | 1.0 | 0.0 | COS | - | 0.999 | 4.987 | 0.999 | 9.955 | 53.622 | 60.818 | 13.751 | 30.790 |
| 15 | 0.5 | 1.0 | 0.0 | RBF | 10.0 | 0.999 | 4.987 | 0.999 | 9.955 | 53.622 | 60.818 | 13.751 | 30.790 |
| 15 | 0.5 | 1.0 | 1.0 | COS | - | 0.999 | 4.987 | 0.999 | 9.955 | 53.627 | 60.819 | 13.751 | 30.799 |
| 15 | 0.5 | 1.0 | 1.0 | RBF | 10.0 | 0.999 | 4.987 | 0.999 | 9.955 | 53.622 | 60.819 | 13.751 | 30.799 |
| 15 | 0.5 | 1.0 | 10.0 | COS | - | 0.999 | 4.987 | 0.999 | 9.955 | 53.622 | 60.816 | 13.713 | 30.817 |
| 15 | 0.5 | 1.0 | 10.0 | RBF | 10.0 | 0.999 | 4.987 | 0.999 | 9.955 | 53.622 | 60.818 | 13.713 | 30.817 |
| 15 | 0.5 | 1.0 | 100.0 | COS | - | 0.999 | 4.987 | 0.999 | 9.956 | 53.647 | 60.818 | 13.871 | 30.864 |
| 15 | 0.5 | 1.0 | 100.0 | RBF | 10.0 | 0.999 | 4.987 | 0.999 | 9.956 | 53.647 | 60.816 | 13.871 | 30.845 |
| 15 | 1.0 | 0.1 | 0.0 | COS | - | 0.980 | 4.807 | 0.969 | 9.452 | 50.743 | 49.259 | 31.667 | 37.397 |
| 15 | 1.0 | 0.1 | 0.0 | RBF | 10.0 | 0.980 | 4.807 | 0.969 | 9.452 | 50.743 | 49.259 | 31.667 | 37.397 |
| 15 | 1.0 | 0.1 | 1.0 | COS | - | 0.981 | 4.815 | 0.971 | 9.475 | 52.322 | 50.526 | 32.346 | 37.624 |
| 15 | 1.0 | 0.1 | 1.0 | RBF | 10.0 | 0.981 | 4.814 | 0.971 | 9.471 | 52.131 | 50.412 | 32.232 | 37.572 |
| 15 | 1.0 | 0.1 | 10.0 | COS | - | 0.983 | 4.836 | 0.974 | 9.515 | 54.382 | 52.446 | 33.719 | 39.044 |
| 15 | 1.0 | 0.1 | 10.0 | RBF | 10.0 | 0.983 | 4.838 | 0.974 | 9.512 | 54.266 | 52.346 | 33.671 | 38.723 |
| 15 | 1.0 | 0.1 | 100.0 | COS | - | 0.987 | 4.873 | 0.980 | 9.612 | 61.671 | 59.681 | 37.358 | 43.800 |

Continued on next page

TABLE S13 – continued from previous page

| $l$ | $\alpha$ | $\beta$ | $\gamma$ | usim | $\sigma$ | AP@5 | AH@5 | AP@10 | AH@10 | AT@5% | AT@10% | NT@5% | NT@10% |
|---|---|---|---|---|---|---|---|---|---|---|---|---|---|
| 15 | 1.0 | 0.1 | 100.0 | RBF | 10.0 | 0.986 | 4.871 | 0.980 | 9.607 | 61.315 | 59.160 | 37.678 | 43.743 |
| 15 | 1.0 | 1.0 | 0.0 | COS | - | 0.982 | 4.822 | 0.972 | 9.478 | 52.867 | 50.943 | 32.329 | 37.380 |
| 15 | 1.0 | 1.0 | 0.0 | RBF | 10.0 | 0.982 | 4.822 | 0.972 | 9.478 | 52.867 | 50.943 | 32.329 | 37.380 |
| 15 | 1.0 | 1.0 | 1.0 | COS | - | 0.982 | 4.829 | 0.973 | 9.495 | 53.822 | 51.871 | 32.445 | 37.933 |
| 15 | 1.0 | 1.0 | 1.0 | RBF | 10.0 | 0.982 | 4.828 | 0.973 | 9.493 | 53.710 | 51.803 | 32.462 | 37.939 |
| 15 | 1.0 | 1.0 | 10.0 | COS | - | 0.984 | 4.850 | 0.976 | 9.541 | 55.932 | 53.942 | 34.013 | 39.266 |
| 15 | 1.0 | 1.0 | 10.0 | RBF | 10.0 | 0.984 | 4.848 | 0.976 | 9.540 | 55.917 | 53.937 | 33.798 | 39.049 |
| 15 | 1.0 | 1.0 | 100.0 | COS | - | 0.987 | 4.874 | 0.980 | 9.614 | 61.720 | 59.800 | 37.300 | 43.938 |
| 15 | 1.0 | 1.0 | 100.0 | RBF | 10.0 | 0.985 | 4.866 | 0.979 | 9.595 | 60.692 | 58.572 | 37.110 | 43.416 |
| 30 | 0.0 | 0.1 | 0.0 | COS | - | 1.000 | 4.994 | 0.999 | 9.972 | 55.026 | 60.463 | 2.336 | 8.114 |
| 30 | 0.0 | 0.1 | 0.0 | RBF | 10.0 | 1.000 | 4.994 | 0.999 | 9.972 | 55.026 | 60.463 | 2.336 | 8.114 |
| 30 | 0.0 | 0.1 | 1.0 | COS | - | 1.000 | 4.994 | 0.999 | 9.972 | 55.021 | 60.460 | 2.336 | 8.107 |
| 30 | 0.0 | 0.1 | 1.0 | RBF | 10.0 | 1.000 | 4.994 | 0.999 | 9.972 | 55.026 | 60.460 | 2.336 | 8.107 |
| 30 | 0.0 | 0.1 | 10.0 | COS | - | 1.000 | 4.994 | 0.999 | 9.972 | 55.060 | 60.456 | 2.299 | 7.920 |
| 30 | 0.0 | 0.1 | 10.0 | RBF | 10.0 | 1.000 | 4.994 | 0.999 | 9.972 | 55.060 | 60.458 | 2.299 | 7.913 |
| 30 | 0.0 | 0.1 | 100.0 | COS | - | 1.000 | 4.993 | 0.999 | 9.970 | 53.160 | 60.085 | 3.970 | 14.969 |
| 30 | 0.0 | 0.1 | 100.0 | RBF | 10.0 | 1.000 | 4.994 | 0.999 | 9.971 | 54.265 | 60.192 | 2.971 | 10.651 |
| 30 | 0.0 | 1.0 | 0.0 | COS | - | 1.000 | 4.994 | 0.999 | 9.972 | 55.104 | 60.475 | 2.257 | 7.860 |
| 30 | 0.0 | 1.0 | 0.0 | RBF | 10.0 | 1.000 | 4.994 | 0.999 | 9.972 | 55.104 | 60.475 | 2.257 | 7.860 |
| 30 | 0.0 | 1.0 | 1.0 | COS | - | 1.000 | 4.994 | 0.999 | 9.972 | 55.104 | 60.470 | 2.257 | 7.854 |
| 30 | 0.0 | 1.0 | 1.0 | RBF | 10.0 | 1.000 | 4.994 | 0.999 | 9.972 | 55.104 | 60.470 | 2.257 | 7.854 |
| 30 | 0.0 | 1.0 | 10.0 | COS | - | 1.000 | 4.994 | 0.999 | 9.972 | 55.084 | 60.458 | 2.287 | 7.877 |
| 30 | 0.0 | 1.0 | 10.0 | RBF | 10.0 | 1.000 | 4.994 | 0.999 | 9.972 | 55.084 | 60.460 | 2.287 | 7.877 |
| 30 | 0.0 | 1.0 | 100.0 | COS | - | 1.000 | 4.994 | 0.999 | 9.972 | 54.816 | 60.363 | 2.302 | 8.422 |
| 30 | 0.0 | 1.0 | 100.0 | RBF | 10.0 | 1.000 | 4.994 | 0.999 | 9.972 | 54.967 | 60.424 | 2.263 | 7.960 |
| 30 | 0.05 | 0.1 | 0.0 | COS | - | 1.000 | 4.994 | 0.999 | 9.972 | 55.508 | 60.624 | 2.299 | 7.636 |
| 30 | 0.05 | 0.1 | 0.0 | RBF | 10.0 | 1.000 | 4.994 | 0.999 | 9.972 | 55.508 | 60.624 | 2.299 | 7.636 |
| 30 | 0.05 | 0.1 | 1.0 | COS | - | 1.000 | 4.994 | 0.999 | 9.972 | 55.508 | 60.624 | 2.299 | 7.636 |
| 30 | 0.05 | 0.1 | 1.0 | RBF | 10.0 | 1.000 | 4.994 | 0.999 | 9.972 | 55.508 | 60.624 | 2.299 | 7.636 |
| 30 | 0.05 | 0.1 | 10.0 | COS | - | 1.000 | 4.994 | 0.999 | 9.972 | 55.474 | 60.619 | 2.299 | 7.636 |
| 30 | 0.05 | 0.1 | 10.0 | RBF | 10.0 | 1.000 | 4.994 | 0.999 | 9.972 | 55.488 | 60.619 | 2.299 | 7.636 |
| 30 | 0.05 | 0.1 | 100.0 | COS | - | 1.000 | 4.994 | 0.999 | 9.972 | 55.367 | 60.553 | 2.305 | 7.727 |
| 30 | 0.05 | 0.1 | 100.0 | RBF | 10.0 | 1.000 | 4.994 | 0.999 | 9.972 | 55.372 | 60.551 | 2.322 | 7.707 |
| 30 | 0.05 | 1.0 | 0.0 | COS | - | 1.000 | 4.994 | 0.999 | 9.972 | 55.508 | 60.624 | 2.299 | 7.636 |
| 30 | 0.05 | 1.0 | 0.0 | RBF | 10.0 | 1.000 | 4.994 | 0.999 | 9.972 | 55.508 | 60.624 | 2.299 | 7.636 |
| 30 | 0.05 | 1.0 | 1.0 | COS | - | 1.000 | 4.994 | 0.999 | 9.972 | 55.508 | 60.624 | 2.299 | 7.636 |
| 30 | 0.05 | 1.0 | 1.0 | RBF | 10.0 | 1.000 | 4.994 | 0.999 | 9.972 | 55.508 | 60.624 | 2.299 | 7.636 |
| 30 | 0.05 | 1.0 | 10.0 | COS | - | 1.000 | 4.994 | 0.999 | 9.972 | 55.474 | 60.621 | 2.299 | 7.641 |
| 30 | 0.05 | 1.0 | 10.0 | RBF | 10.0 | 1.000 | 4.994 | 0.999 | 9.972 | 55.484 | 60.619 | 2.299 | 7.636 |
| 30 | 0.05 | 1.0 | 100.0 | COS | - | 1.000 | 4.994 | 0.999 | 9.972 | 55.367 | 60.551 | 2.305 | 7.727 |
| 30 | 0.05 | 1.0 | 100.0 | RBF | 10.0 | 1.000 | 4.994 | 0.999 | 9.972 | 55.372 | 60.548 | 2.322 | 7.698 |
| 30 | 0.1 | 0.1 | 0.0 | COS | - | 1.000 | 4.994 | 0.999 | 9.972 | 55.810 | 60.840 | 2.313 | 7.571 |
| 30 | 0.1 | 0.1 | 0.0 | RBF | 10.0 | 1.000 | 4.994 | 0.999 | 9.972 | 55.810 | 60.840 | 2.313 | 7.571 |
| 30 | 0.1 | 0.1 | 1.0 | COS | - | 1.000 | 4.994 | 0.999 | 9.972 | 55.810 | 60.833 | 2.313 | 7.571 |
| 30 | 0.1 | 0.1 | 1.0 | RBF | 10.0 | 1.000 | 4.994 | 0.999 | 9.972 | 55.810 | 60.836 | 2.313 | 7.571 |
| 30 | 0.1 | 0.1 | 10.0 | COS | - | 1.000 | 4.994 | 0.999 | 9.972 | 55.771 | 60.833 | 2.313 | 7.635 |
| 30 | 0.1 | 0.1 | 10.0 | RBF | 10.0 | 1.000 | 4.994 | 0.999 | 9.972 | 55.776 | 60.833 | 2.313 | 7.607 |
| 30 | 0.1 | 0.1 | 100.0 | COS | - | 1.000 | 4.994 | 0.999 | 9.972 | 55.683 | 60.762 | 2.311 | 7.605 |
| 30 | 0.1 | 0.1 | 100.0 | RBF | 10.0 | 1.000 | 4.994 | 0.999 | 9.972 | 55.698 | 60.762 | 2.311 | 7.606 |
| 30 | 0.1 | 1.0 | 0.0 | COS | - | 1.000 | 4.994 | 0.999 | 9.972 | 55.810 | 60.838 | 2.313 | 7.571 |
| 30 | 0.1 | 1.0 | 0.0 | RBF | 10.0 | 1.000 | 4.994 | 0.999 | 9.972 | 55.810 | 60.838 | 2.313 | 7.571 |
| 30 | 0.1 | 1.0 | 1.0 | COS | - | 1.000 | 4.994 | 0.999 | 9.972 | 55.810 | 60.833 | 2.313 | 7.571 |
| 30 | 0.1 | 1.0 | 1.0 | RBF | 10.0 | 1.000 | 4.994 | 0.999 | 9.972 | 55.810 | 60.833 | 2.313 | 7.571 |
| 30 | 0.1 | 1.0 | 10.0 | COS | - | 1.000 | 4.994 | 0.999 | 9.972 | 55.771 | 60.833 | 2.313 | 7.635 |
| 30 | 0.1 | 1.0 | 10.0 | RBF | 10.0 | 1.000 | 4.994 | 0.999 | 9.972 | 55.776 | 60.833 | 2.313 | 7.607 |
| 30 | 0.1 | 1.0 | 100.0 | COS | - | 1.000 | 4.994 | 0.999 | 9.972 | 55.683 | 60.760 | 2.311 | 7.605 |
| 30 | 0.1 | 1.0 | 100.0 | RBF | 10.0 | 1.000 | 4.994 | 0.999 | 9.972 | 55.698 | 60.762 | 2.311 | 7.606 |
| 30 | 0.5 | 0.1 | 0.0 | COS | - | 1.000 | 4.994 | 0.999 | 9.972 | 58.207 | 62.273 | 2.309 | 6.954 |

Continued on next page

TABLE S13 – continued from previous page

| $l$ | $\alpha$ | $\beta$ | $\gamma$ | usim | $\sigma$ | AP@5 | AH@5 | AP@10 | AH@10 | AT@5% | AT@10% | NT@5% | NT@10% |
|---|---|---|---|---|---|---|---|---|---|---|---|---|---|
| 30 | 0.5 | 0.1 | 0.0 | RBF | 10.0 | 1.000 | 4.994 | 0.999 | 9.972 | 58.207 | 62.273 | 2.309 | 6.954 |
| 30 | 0.5 | 0.1 | 1.0 | COS | - | 1.000 | 4.994 | 0.999 | 9.972 | 58.207 | 62.273 | 2.309 | 6.954 |
| 30 | 0.5 | 0.1 | 1.0 | RBF | 10.0 | 1.000 | 4.994 | 0.999 | 9.972 | 58.207 | 62.273 | 2.309 | 6.954 |
| 30 | 0.5 | 0.1 | 10.0 | COS | - | 1.000 | 4.994 | 0.999 | 9.972 | 58.197 | 62.275 | 2.309 | 6.954 |
| 30 | 0.5 | 0.1 | 10.0 | RBF | 10.0 | 1.000 | 4.994 | 0.999 | 9.972 | 58.197 | 62.275 | 2.309 | 6.954 |
| 30 | 0.5 | 0.1 | 100.0 | COS | - | 1.000 | 4.994 | 0.999 | 9.972 | 58.149 | 62.229 | 2.328 | 6.999 |
| 30 | 0.5 | 0.1 | 100.0 | RBF | 10.0 | 1.000 | 4.994 | 0.999 | 9.972 | 58.173 | 62.236 | 2.328 | 6.990 |
| 30 | 0.5 | 1.0 | 0.0 | COS | - | 1.000 | 4.994 | 0.999 | 9.972 | 58.207 | 62.273 | 2.309 | 6.954 |
| 30 | 0.5 | 1.0 | 0.0 | RBF | 10.0 | 1.000 | 4.994 | 0.999 | 9.972 | 58.207 | 62.273 | 2.309 | 6.954 |
| 30 | 0.5 | 1.0 | 1.0 | COS | - | 1.000 | 4.994 | 0.999 | 9.972 | 58.207 | 62.273 | 2.309 | 6.954 |
| 30 | 0.5 | 1.0 | 1.0 | RBF | 10.0 | 1.000 | 4.994 | 0.999 | 9.972 | 58.207 | 62.273 | 2.309 | 6.954 |
| 30 | 0.5 | 1.0 | 10.0 | COS | - | 1.000 | 4.994 | 0.999 | 9.972 | 58.193 | 62.275 | 2.309 | 6.954 |
| 30 | 0.5 | 1.0 | 10.0 | RBF | 10.0 | 1.000 | 4.994 | 0.999 | 9.972 | 58.197 | 62.278 | 2.309 | 6.954 |
| 30 | 0.5 | 1.0 | 100.0 | COS | - | 1.000 | 4.994 | 0.999 | 9.972 | 58.149 | 62.229 | 2.328 | 6.999 |
| 30 | 0.5 | 1.0 | 100.0 | RBF | 10.0 | 1.000 | 4.994 | 0.999 | 9.972 | 58.173 | 62.236 | 2.328 | 6.990 |
| 30 | 1.0 | 0.1 | 0.0 | COS | - | 0.997 | 4.968 | 0.994 | 9.854 | 74.889 | 70.911 | 10.980 | 24.665 |
| 30 | 1.0 | 0.1 | 0.0 | RBF | 10.0 | 0.997 | 4.968 | 0.994 | 9.854 | 74.889 | 70.911 | 10.980 | 24.665 |
| 30 | 1.0 | 0.1 | 1.0 | COS | - | 0.997 | 4.969 | 0.995 | 9.856 | 74.982 | 71.104 | 11.421 | 25.163 |
| 30 | 1.0 | 0.1 | 1.0 | RBF | 10.0 | 0.997 | 4.968 | 0.995 | 9.856 | 74.943 | 71.094 | 11.227 | 25.056 |
| 30 | 1.0 | 0.1 | 10.0 | COS | - | 0.997 | 4.957 | 0.993 | 9.810 | 74.022 | 69.583 | 20.520 | 35.115 |
| 30 | 1.0 | 0.1 | 10.0 | RBF | 10.0 | 0.997 | 4.959 | 0.993 | 9.822 | 74.261 | 69.900 | 19.283 | 34.006 |
| 30 | 1.0 | 0.1 | 100.0 | COS | - | 0.994 | 4.921 | 0.987 | 9.706 | 71.547 | 66.358 | 32.438 | 44.142 |
| 30 | 1.0 | 0.1 | 100.0 | RBF | 10.0 | 0.993 | 4.920 | 0.987 | 9.712 | 71.664 | 66.390 | 32.060 | 43.777 |
| 30 | 1.0 | 1.0 | 0.0 | COS | - | 0.998 | 4.968 | 0.995 | 9.860 | 75.099 | 71.193 | 10.921 | 24.676 |
| 30 | 1.0 | 1.0 | 0.0 | RBF | 10.0 | 0.998 | 4.968 | 0.995 | 9.860 | 75.099 | 71.193 | 10.921 | 24.676 |
| 30 | 1.0 | 1.0 | 1.0 | COS | - | 0.997 | 4.968 | 0.995 | 9.861 | 75.167 | 71.337 | 11.360 | 24.808 |
| 30 | 1.0 | 1.0 | 1.0 | RBF | 10.0 | 0.997 | 4.968 | 0.995 | 9.860 | 75.162 | 71.333 | 11.326 | 24.803 |
| 30 | 1.0 | 1.0 | 10.0 | COS | - | 0.997 | 4.962 | 0.994 | 9.832 | 74.543 | 70.375 | 17.864 | 32.639 |
| 30 | 1.0 | 1.0 | 10.0 | RBF | 10.0 | 0.997 | 4.964 | 0.994 | 9.842 | 74.616 | 70.619 | 16.351 | 31.469 |
| 30 | 1.0 | 1.0 | 100.0 | COS | - | 0.993 | 4.921 | 0.988 | 9.716 | 71.834 | 66.721 | 32.605 | 44.346 |
| 30 | 1.0 | 1.0 | 100.0 | RBF | 10.0 | 0.994 | 4.922 | 0.988 | 9.718 | 71.961 | 66.679 | 32.066 | 43.754 |
| 50 | 0.0 | 0.1 | 0.0 | COS | - | 1.000 | 4.996 | 1.000 | 9.980 | 59.196 | 63.160 | 0.604 | 2.064 |
| 50 | 0.0 | 0.1 | 0.0 | RBF | 10.0 | 1.000 | 4.996 | 1.000 | 9.980 | 59.196 | 63.160 | 0.604 | 2.064 |
| 50 | 0.0 | 0.1 | 1.0 | COS | - | 1.000 | 4.996 | 1.000 | 9.980 | 59.298 | 63.216 | 0.587 | 2.037 |
| 50 | 0.0 | 0.1 | 1.0 | RBF | 10.0 | 1.000 | 4.996 | 1.000 | 9.980 | 59.250 | 63.184 | 0.587 | 2.051 |
| 50 | 0.0 | 0.1 | 10.0 | COS | - | 1.000 | 4.996 | 1.000 | 9.979 | 59.542 | 63.345 | 0.587 | 1.995 |
| 50 | 0.0 | 0.1 | 10.0 | RBF | 10.0 | 1.000 | 4.996 | 1.000 | 9.979 | 59.542 | 63.347 | 0.587 | 1.995 |
| 50 | 0.0 | 0.1 | 100.0 | COS | - | 1.000 | 4.994 | 0.999 | 9.970 | 52.521 | 61.111 | 9.252 | 22.422 |
| 50 | 0.0 | 0.1 | 100.0 | RBF | 10.0 | 1.000 | 4.995 | 1.000 | 9.976 | 54.548 | 61.501 | 2.741 | 10.398 |
| 50 | 0.0 | 1.0 | 0.0 | COS | - | 1.000 | 4.996 | 1.000 | 9.979 | 59.776 | 63.437 | 0.550 | 1.900 |
| 50 | 0.0 | 1.0 | 0.0 | RBF | 10.0 | 1.000 | 4.996 | 1.000 | 9.979 | 59.776 | 63.437 | 0.550 | 1.900 |
| 50 | 0.0 | 1.0 | 1.0 | COS | - | 1.000 | 4.996 | 1.000 | 9.979 | 59.771 | 63.437 | 0.550 | 1.900 |
| 50 | 0.0 | 1.0 | 1.0 | RBF | 10.0 | 1.000 | 4.996 | 1.000 | 9.979 | 59.771 | 63.437 | 0.550 | 1.900 |
| 50 | 0.0 | 1.0 | 10.0 | COS | - | 1.000 | 4.996 | 1.000 | 9.979 | 59.757 | 63.423 | 0.550 | 1.900 |
| 50 | 0.0 | 1.0 | 10.0 | RBF | 10.0 | 1.000 | 4.996 | 1.000 | 9.979 | 59.766 | 63.428 | 0.550 | 1.900 |
| 50 | 0.0 | 1.0 | 100.0 | COS | - | 1.000 | 4.996 | 1.000 | 9.977 | 56.034 | 61.849 | 1.140 | 5.142 |
| 50 | 0.0 | 1.0 | 100.0 | RBF | 10.0 | 1.000 | 4.996 | 1.000 | 9.979 | 57.895 | 62.519 | 0.835 | 2.680 |
| 50 | 0.05 | 0.1 | 0.0 | COS | - | 1.000 | 4.996 | 1.000 | 9.979 | 60.175 | 63.684 | 0.598 | 1.873 |
| 50 | 0.05 | 0.1 | 0.0 | RBF | 10.0 | 1.000 | 4.996 | 1.000 | 9.979 | 60.175 | 63.684 | 0.598 | 1.873 |
| 50 | 0.05 | 0.1 | 1.0 | COS | - | 1.000 | 4.996 | 1.000 | 9.979 | 60.170 | 63.676 | 0.598 | 1.873 |
| 50 | 0.05 | 0.1 | 1.0 | RBF | 10.0 | 1.000 | 4.996 | 1.000 | 9.979 | 60.170 | 63.679 | 0.598 | 1.873 |
| 50 | 0.05 | 0.1 | 10.0 | COS | - | 1.000 | 4.996 | 1.000 | 9.979 | 60.151 | 63.659 | 0.598 | 1.873 |
| 50 | 0.05 | 0.1 | 10.0 | RBF | 10.0 | 1.000 | 4.996 | 1.000 | 9.979 | 60.151 | 63.666 | 0.598 | 1.873 |
| 50 | 0.05 | 0.1 | 100.0 | COS | - | 1.000 | 4.996 | 1.000 | 9.978 | 57.408 | 62.414 | 0.926 | 3.766 |
| 50 | 0.05 | 0.1 | 100.0 | RBF | 10.0 | 1.000 | 4.996 | 1.000 | 9.979 | 59.362 | 63.262 | 0.604 | 2.162 |
| 50 | 0.05 | 1.0 | 0.0 | COS | - | 1.000 | 4.996 | 1.000 | 9.979 | 60.170 | 63.684 | 0.598 | 1.873 |
| 50 | 0.05 | 1.0 | 0.0 | RBF | 10.0 | 1.000 | 4.996 | 1.000 | 9.979 | 60.170 | 63.684 | 0.598 | 1.873 |
| 50 | 0.05 | 1.0 | 1.0 | COS | - | 1.000 | 4.996 | 1.000 | 9.979 | 60.166 | 63.676 | 0.598 | 1.873 |

Continued on next page

TABLE S13 – continued from previous page

| $l$ | $\alpha$ | $\beta$ | $\gamma$ | usim | $\sigma$ | AP@5 | AH@5 | AP@10 | AH@10 | AT@5% | AT@10% | NT@5% | NT@10% |
|---|---|---|---|---|---|---|---|---|---|---|---|---|---|
| 50 | 0.05 | 1.0 | 1.0 | RBF | 10.0 | 1.000 | 4.996 | 1.000 | 9.979 | 60.166 | 63.676 | 0.598 | 1.873 |
| 50 | 0.05 | 1.0 | 10.0 | COS | - | 1.000 | 4.996 | 1.000 | 9.979 | 60.146 | 63.656 | 0.598 | 1.873 |
| 50 | 0.05 | 1.0 | 10.0 | RBF | 10.0 | 1.000 | 4.996 | 1.000 | 9.979 | 60.151 | 63.666 | 0.598 | 1.873 |
| 50 | 0.05 | 1.0 | 100.0 | COS | - | 1.000 | 4.996 | 1.000 | 9.980 | 59.255 | 63.172 | 0.623 | 2.186 |
| 50 | 0.05 | 1.0 | 100.0 | RBF | 10.0 | 1.000 | 4.996 | 1.000 | 9.979 | 59.947 | 63.581 | 0.568 | 1.887 |
| 50 | 0.1 | 0.1 | 0.0 | COS | - | 0.999 | 4.984 | 0.998 | 9.957 | 55.445 | 61.065 | 17.949 | 22.838 |
| 50 | 0.1 | 0.1 | 0.0 | RBF | 10.0 | 0.999 | 4.984 | 0.998 | 9.957 | 55.445 | 61.065 | 17.949 | 22.838 |
| 50 | 0.1 | 0.1 | 1.0 | COS | - | 1.000 | 4.996 | 1.000 | 9.979 | 60.560 | 63.900 | 0.598 | 1.910 |
| 50 | 0.1 | 0.1 | 1.0 | RBF | 10.0 | 1.000 | 4.996 | 1.000 | 9.979 | 60.560 | 63.900 | 0.598 | 1.910 |
| 50 | 0.1 | 0.1 | 10.0 | COS | - | 1.000 | 4.996 | 1.000 | 9.979 | 60.521 | 63.890 | 0.598 | 1.910 |
| 50 | 0.1 | 0.1 | 10.0 | RBF | 10.0 | 1.000 | 4.996 | 1.000 | 9.979 | 60.531 | 63.898 | 0.598 | 1.910 |
| 50 | 0.1 | 0.1 | 100.0 | COS | - | 1.000 | 4.996 | 1.000 | 9.979 | 59.927 | 63.596 | 0.616 | 2.003 |
| 50 | 0.1 | 0.1 | 100.0 | RBF | 10.0 | 1.000 | 4.996 | 1.000 | 9.979 | 60.399 | 63.820 | 0.598 | 1.896 |
| 50 | 0.1 | 1.0 | 0.0 | COS | - | 1.000 | 4.996 | 1.000 | 9.979 | 60.560 | 63.900 | 0.598 | 1.910 |
| 50 | 0.1 | 1.0 | 0.0 | RBF | 10.0 | 1.000 | 4.996 | 1.000 | 9.979 | 60.560 | 63.900 | 0.598 | 1.910 |
| 50 | 0.1 | 1.0 | 1.0 | COS | - | 1.000 | 4.996 | 1.000 | 9.979 | 60.560 | 63.903 | 0.598 | 1.910 |
| 50 | 0.1 | 1.0 | 1.0 | RBF | 10.0 | 1.000 | 4.996 | 1.000 | 9.979 | 60.560 | 63.903 | 0.598 | 1.910 |
| 50 | 0.1 | 1.0 | 10.0 | COS | - | 1.000 | 4.996 | 1.000 | 9.979 | 60.517 | 63.890 | 0.598 | 1.910 |
| 50 | 0.1 | 1.0 | 10.0 | RBF | 10.0 | 1.000 | 4.996 | 1.000 | 9.979 | 60.531 | 63.895 | 0.598 | 1.910 |
| 50 | 0.1 | 1.0 | 100.0 | COS | - | 1.000 | 4.996 | 1.000 | 9.979 | 60.395 | 63.798 | 0.598 | 1.889 |
| 50 | 0.1 | 1.0 | 100.0 | RBF | 10.0 | 1.000 | 4.996 | 1.000 | 9.979 | 60.399 | 63.820 | 0.598 | 1.896 |
| 50 | 0.5 | 0.1 | 0.0 | COS | - | 0.998 | 4.982 | 0.998 | 9.949 | 63.834 | 68.631 | 20.091 | 28.507 |
| 50 | 0.5 | 0.1 | 0.0 | RBF | 10.0 | 0.998 | 4.982 | 0.998 | 9.949 | 63.834 | 68.631 | 20.091 | 28.507 |
| 50 | 0.5 | 0.1 | 1.0 | COS | - | 0.998 | 4.982 | 0.998 | 9.949 | 63.698 | 68.494 | 20.062 | 28.385 |
| 50 | 0.5 | 0.1 | 1.0 | RBF | 10.0 | 0.998 | 4.982 | 0.998 | 9.949 | 63.712 | 68.516 | 20.062 | 28.405 |
| 50 | 0.5 | 0.1 | 10.0 | COS | - | 0.998 | 4.984 | 0.998 | 9.956 | 57.223 | 62.297 | 17.965 | 23.094 |
| 50 | 0.5 | 0.1 | 10.0 | RBF | 10.0 | 0.998 | 4.984 | 0.998 | 9.956 | 57.237 | 62.295 | 17.965 | 23.094 |
| 50 | 0.5 | 0.1 | 100.0 | COS | - | 0.998 | 4.982 | 0.998 | 9.948 | 64.136 | 69.228 | 21.314 | 32.323 |
| 50 | 0.5 | 0.1 | 100.0 | RBF | 10.0 | 0.998 | 4.982 | 0.998 | 9.949 | 63.786 | 68.914 | 20.947 | 31.269 |
| 50 | 0.5 | 1.0 | 0.0 | COS | - | 0.998 | 4.984 | 0.998 | 9.956 | 57.252 | 62.287 | 17.918 | 23.062 |
| 50 | 0.5 | 1.0 | 0.0 | RBF | 10.0 | 0.998 | 4.984 | 0.998 | 9.956 | 57.252 | 62.287 | 17.918 | 23.062 |
| 50 | 0.5 | 1.0 | 1.0 | COS | - | 0.998 | 4.984 | 0.998 | 9.956 | 57.291 | 62.248 | 17.918 | 23.057 |
| 50 | 0.5 | 1.0 | 1.0 | RBF | 10.0 | 0.998 | 4.984 | 0.998 | 9.956 | 57.276 | 62.268 | 17.918 | 23.057 |
| 50 | 0.5 | 1.0 | 10.0 | COS | - | 0.998 | 4.984 | 0.998 | 9.956 | 57.286 | 62.202 | 17.918 | 22.959 |
| 50 | 0.5 | 1.0 | 10.0 | RBF | 10.0 | 0.998 | 4.984 | 0.998 | 9.956 | 57.291 | 62.202 | 17.918 | 22.959 |
| 50 | 0.5 | 1.0 | 100.0 | COS | - | 0.998 | 4.982 | 0.998 | 9.949 | 62.665 | 67.963 | 20.868 | 30.726 |
| 50 | 0.5 | 1.0 | 100.0 | RBF | 10.0 | 0.998 | 4.983 | 0.998 | 9.951 | 62.080 | 67.355 | 20.395 | 29.911 |
| 50 | 1.0 | 0.1 | 0.0 | COS | - | 0.999 | 4.987 | 0.998 | 9.934 | 78.777 | 77.235 | 3.659 | 16.645 |
| 50 | 1.0 | 0.1 | 0.0 | RBF | 10.0 | 0.999 | 4.987 | 0.998 | 9.934 | 78.777 | 77.235 | 3.659 | 16.645 |
| 50 | 1.0 | 0.1 | 1.0 | COS | - | 0.999 | 4.987 | 0.998 | 9.938 | 78.728 | 77.230 | 3.735 | 16.302 |
| 50 | 1.0 | 0.1 | 1.0 | RBF | 10.0 | 0.999 | 4.987 | 0.998 | 9.938 | 78.719 | 77.233 | 3.716 | 16.335 |
| 50 | 1.0 | 0.1 | 10.0 | COS | - | 0.998 | 4.978 | 0.997 | 9.893 | 79.415 | 76.489 | 16.928 | 36.025 |
| 50 | 1.0 | 0.1 | 10.0 | RBF | 10.0 | 0.999 | 4.979 | 0.997 | 9.904 | 79.367 | 76.772 | 14.694 | 33.769 |
| 50 | 1.0 | 0.1 | 100.0 | COS | - | 0.996 | 4.946 | 0.991 | 9.770 | 77.096 | 71.152 | 32.855 | 46.931 |
| 50 | 1.0 | 0.1 | 100.0 | RBF | 10.0 | 0.996 | 4.946 | 0.991 | 9.769 | 77.228 | 71.274 | 32.806 | 46.652 |
| 50 | 1.0 | 1.0 | 0.0 | COS | - | 0.999 | 4.987 | 0.998 | 9.937 | 78.767 | 77.199 | 3.445 | 15.456 |
| 50 | 1.0 | 1.0 | 0.0 | RBF | 10.0 | 0.999 | 4.987 | 0.998 | 9.937 | 78.767 | 77.199 | 3.445 | 15.456 |
| 50 | 1.0 | 1.0 | 1.0 | COS | - | 0.999 | 4.987 | 0.998 | 9.937 | 78.762 | 77.160 | 3.569 | 15.290 |
| 50 | 1.0 | 1.0 | 1.0 | RBF | 10.0 | 0.999 | 4.987 | 0.998 | 9.937 | 78.762 | 77.162 | 3.557 | 15.161 |
| 50 | 1.0 | 1.0 | 10.0 | COS | - | 0.999 | 4.982 | 0.997 | 9.912 | 79.284 | 76.984 | 12.646 | 31.247 |
| 50 | 1.0 | 1.0 | 10.0 | RBF | 10.0 | 0.999 | 4.983 | 0.997 | 9.921 | 79.220 | 77.191 | 11.008 | 29.370 |
| 50 | 1.0 | 1.0 | 100.0 | COS | - | 0.996 | 4.948 | 0.991 | 9.778 | 77.198 | 71.425 | 32.661 | 46.862 |
| 50 | 1.0 | 1.0 | 100.0 | RBF | 10.0 | 0.996 | 4.950 | 0.992 | 9.777 | 77.413 | 71.766 | 31.886 | 46.296 |

The columns corresponding to "$l$", "$\alpha$", "$\beta$", "$\gamma$", "usim", and "$\sigma$" have the latent dimension, weighting factor, latent vector regularization parameter, cell line similarity regularization parameter, cell line similarity function, and parameter for rbf cell line similarity, respectively, for pLETORg.

# S12 Performance on Ranking Drugs in New Cell Lines

**TABLE S14:** BMTMKL Performance on New Cell Lines ($\theta$ = 2)

| n | $\alpha_b$ | $\beta_b$ | usim | $\sigma$ | AP@5 | AP@10 | sCI | CI |
|---|---|---|---|---|---|---|---|---|
| 100 | 1 | 1 | RBF | 10.0 | 0.838 | 0.782 | 0.613 | 0.800 |
| 100 | 1e-10 | 1e-10 | RBF | 10.0 | 0.842 | 0.783 | 0.612 | 0.800 |
| 100 | 1e-10 | 1e+10 | RBF | 10.0 | 0.837 | 0.782 | 0.613 | 0.800 |
| 150 | 1 | 1 | RBF | 10.0 | 0.844 | 0.783 | 0.619 | 0.800 |
| 150 | 1e-10 | 1e-10 | RBF | 10.0 | 0.840 | 0.783 | 0.619 | 0.800 |
| 150 | 1e-10 | 1e+10 | RBF | 10.0 | 0.844 | 0.783 | 0.619 | 0.800 |
| 200 | 1 | 1 | RBF | 10.0 | 0.834 | 0.778 | 0.625 | 0.800 |
| 200 | 1e-10 | 1e-10 | RBF | 10.0 | 0.833 | 0.777 | 0.626 | 0.800 |
| 200 | 1e-10 | 1e+10 | RBF | 10.0 | 0.834 | 0.778 | 0.625 | 0.800 |
| 250 | 1 | 1 | RBF | 10.0 | 0.833 | 0.774 | 0.622 | 0.802 |
| 250 | 1e-10 | 1e-10 | RBF | 10.0 | 0.833 | 0.774 | 0.621 | 0.802 |
| 250 | 1e-10 | 1e+10 | RBF | 10.0 | 0.831 | 0.774 | 0.621 | 0.802 |
| 300 | 1 | 1 | RBF | 10.0 | 0.829 | 0.768 | 0.621 | 0.801 |
| 300 | 1e-10 | 1e-10 | RBF | 10.0 | 0.829 | 0.768 | 0.621 | 0.802 |
| 300 | 1e-10 | 1e+10 | RBF | 10.0 | 0.829 | 0.768 | 0.621 | 0.801 |
| 350 | 1 | 1 | RBF | 10.0 | 0.823 | 0.763 | 0.621 | 0.800 |
| 350 | 1e-10 | 1e-10 | RBF | 10.0 | 0.823 | 0.763 | 0.621 | 0.799 |
| 350 | 1e-10 | 1e+10 | RBF | 10.0 | 0.823 | 0.763 | 0.621 | 0.800 |
| 400 | 1 | 1 | RBF | 10.0 | 0.829 | 0.768 | 0.626 | 0.800 |
| 400 | 1e-10 | 1e-10 | RBF | 10.0 | 0.828 | 0.769 | 0.626 | 0.800 |
| 400 | 1e-10 | 1e+10 | RBF | 10.0 | 0.828 | 0.769 | 0.627 | 0.800 |
| 50 | 1 | 1 | RBF | 10.0 | 0.855 | 0.792 | 0.617 | 0.804 |
| 50 | 1e-10 | 1e-10 | RBF | 10.0 | 0.855 | 0.792 | 0.616 | 0.804 |
| 50 | 1e-10 | 1e+10 | RBF | 10.0 | 0.855 | 0.792 | 0.617 | 0.804 |

The columns corresponding to "$\alpha_b$", "$\beta_b$", "usim", and "$\sigma$" have the two hyperparameters, cell line similarity function, and parameter for RBF cell line similarity, respectively, for BMTMKL.

**TABLE S15:** BMTMKL Performance on New Cell Lines ($\theta$ = 5)

| n | $\alpha_b$ | $\beta_b$ | usim | $\sigma$ | AP@5 | AP@10 | sCI | CI |
|---|---|---|---|---|---|---|---|---|
| 100 | 1 | 1 | RBF | 10.0 | 0.943 | 0.909 | 0.646 | 0.800 |
| 100 | 1e-10 | 1e-10 | RBF | 10.0 | 0.945 | 0.908 | 0.646 | 0.800 |
| 100 | 1e-10 | 1e+10 | RBF | 10.0 | 0.943 | 0.909 | 0.646 | 0.800 |
| 150 | 1 | 1 | RBF | 10.0 | 0.946 | 0.911 | 0.649 | 0.800 |
| 150 | 1e-10 | 1e-10 | RBF | 10.0 | 0.944 | 0.912 | 0.649 | 0.800 |
| 150 | 1e-10 | 1e+10 | RBF | 10.0 | 0.945 | 0.912 | 0.649 | 0.800 |
| 200 | 1 | 1 | RBF | 10.0 | 0.937 | 0.907 | 0.650 | 0.800 |
| 200 | 1e-10 | 1e-10 | RBF | 10.0 | 0.936 | 0.907 | 0.650 | 0.800 |
| 200 | 1e-10 | 1e+10 | RBF | 10.0 | 0.937 | 0.907 | 0.650 | 0.800 |
| 250 | 1 | 1 | RBF | 10.0 | 0.939 | 0.908 | 0.653 | 0.802 |
| 250 | 1e-10 | 1e-10 | RBF | 10.0 | 0.939 | 0.908 | 0.653 | 0.802 |
| 250 | 1e-10 | 1e+10 | RBF | 10.0 | 0.940 | 0.908 | 0.653 | 0.802 |
| 300 | 1 | 1 | RBF | 10.0 | 0.937 | 0.906 | 0.652 | 0.801 |
| 300 | 1e-10 | 1e-10 | RBF | 10.0 | 0.937 | 0.906 | 0.651 | 0.802 |
| 300 | 1e-10 | 1e+10 | RBF | 10.0 | 0.937 | 0.906 | 0.651 | 0.801 |
| 350 | 1 | 1 | RBF | 10.0 | 0.935 | 0.903 | 0.648 | 0.800 |
| 350 | 1e-10 | 1e-10 | RBF | 10.0 | 0.935 | 0.903 | 0.648 | 0.799 |
| 350 | 1e-10 | 1e+10 | RBF | 10.0 | 0.935 | 0.903 | 0.648 | 0.800 |
| 400 | 1 | 1 | RBF | 10.0 | 0.938 | 0.905 | 0.651 | 0.800 |
| 400 | 1e-10 | 1e-10 | RBF | 10.0 | 0.938 | 0.906 | 0.651 | 0.800 |
| 400 | 1e-10 | 1e+10 | RBF | 10.0 | 0.938 | 0.906 | 0.651 | 0.800 |
| 50 | 1 | 1 | RBF | 10.0 | 0.951 | 0.903 | 0.637 | 0.804 |
| 50 | 1e-10 | 1e-10 | RBF | 10.0 | 0.951 | 0.903 | 0.637 | 0.804 |
| 50 | 1e-10 | 1e+10 | RBF | 10.0 | 0.951 | 0.903 | 0.636 | 0.804 |

The columns corresponding to "$\alpha_b$", "$\beta_b$", "usim", and "$\sigma$" have the two hyperparameters, cell line similarity function, and parameter for RBF cell line similarity, respectively, for BMTMKL.

**TABLE S16:** KRL Performance on New Cell Lines ($\theta$ = 2)

| n | $k$ | $\lambda$ | usim | $\sigma$ | AP@5 | AP@10 | sCI | CI |
|---|---|---|---|---|---|---|---|---|
| 50 | 5 | 0.000001 | RBF | 0.0001 | 0.322 | 0.330 | 0.541 | 0.747 |
| 50 | 5 | 0.000001 | RBF | 0.001 | 0.283 | 0.295 | 0.559 | 0.725 |
| 50 | 5 | 0.000001 | RBF | 0.01 | 0.138 | 0.170 | 0.534 | 0.604 |
| 50 | 5 | 0.00001 | LIN | - | 0.111 | 0.149 | 0.542 | 0.706 |
| 50 | 5 | 0.00001 | RBF | 0.0001 | 0.425 | 0.419 | 0.550 | 0.755 |
| 50 | 5 | 0.00001 | RBF | 0.01 | 0.124 | 0.175 | 0.537 | 0.616 |
| 50 | 5 | 0.0001 | LIN | - | 0.189 | 0.217 | 0.509 | 0.717 |
| 50 | 5 | 0.0001 | RBF | 0.0001 | 0.436 | 0.423 | 0.557 | 0.764 |
| 50 | 5 | 0.0001 | RBF | 0.001 | 0.446 | 0.410 | 0.546 | 0.754 |
| 50 | 5 | 0.0001 | RBF | 0.01 | 0.132 | 0.184 | 0.543 | 0.576 |
| 50 | 5 | 0.001 | LIN | - | 0.195 | 0.238 | 0.511 | 0.698 |
| 50 | 5 | 0.001 | RBF | 0.0001 | 0.436 | 0.423 | 0.557 | 0.764 |
| 50 | 5 | 0.001 | RBF | 0.001 | 0.446 | 0.410 | 0.546 | 0.754 |
| 50 | 5 | 0.001 | RBF | 0.01 | 0.112 | 0.165 | 0.549 | 0.530 |
| 50 | 5 | 0.01 | LIN | - | 0.307 | 0.298 | 0.535 | 0.747 |
| 50 | 5 | 0.01 | RBF | 0.0001 | 0.436 | 0.423 | 0.557 | 0.764 |
| 50 | 5 | 0.01 | RBF | 0.001 | 0.446 | 0.410 | 0.546 | 0.754 |
| 50 | 5 | 0.01 | RBF | 0.01 | 0.106 | 0.147 | 0.516 | 0.490 |
| 50 | 5 | 0.1 | LIN | - | 0.421 | 0.424 | 0.555 | 0.760 |
| 50 | 5 | 0.1 | RBF | 0.0001 | 0.436 | 0.423 | 0.557 | 0.764 |
| 50 | 5 | 0.1 | RBF | 0.001 | 0.446 | 0.410 | 0.546 | 0.754 |
| 50 | 5 | 0.1 | RBF | 0.01 | 0.073 | 0.090 | 0.495 | 0.473 |
| 50 | 5 | 0.2 | LIN | - | 0.439 | 0.414 | 0.556 | 0.763 |
| 50 | 5 | 0.2 | RBF | 0.0001 | 0.436 | 0.423 | 0.557 | 0.764 |
| 50 | 5 | 0.2 | RBF | 0.001 | 0.446 | 0.410 | 0.546 | 0.754 |
| 50 | 5 | 0.2 | RBF | 0.01 | 0.072 | 0.093 | 0.495 | 0.471 |
| 50 | 5 | 0.4 | LIN | - | 0.445 | 0.399 | 0.559 | 0.770 |
| 50 | 5 | 0.4 | RBF | 0.0001 | 0.436 | 0.423 | 0.557 | 0.764 |
| 50 | 5 | 0.4 | RBF | 0.001 | 0.446 | 0.410 | 0.546 | 0.754 |
| 50 | 5 | 0.4 | RBF | 0.01 | 0.049 | 0.070 | 0.495 | 0.470 |
| 50 | 5 | 0.6 | LIN | - | 0.451 | 0.436 | 0.551 | 0.768 |
| 50 | 5 | 0.6 | RBF | 0.0001 | 0.436 | 0.423 | 0.557 | 0.764 |
| 50 | 5 | 0.6 | RBF | 0.001 | 0.446 | 0.410 | 0.546 | 0.754 |
| 50 | 5 | 0.6 | RBF | 0.01 | 0.049 | 0.070 | 0.496 | 0.469 |
| 50 | 5 | 0.8 | LIN | - | 0.433 | 0.413 | 0.553 | 0.771 |
| 50 | 5 | 0.8 | RBF | 0.0001 | 0.436 | 0.423 | 0.557 | 0.764 |
| 50 | 5 | 0.8 | RBF | 0.001 | 0.446 | 0.410 | 0.546 | 0.754 |
| 50 | 5 | 0.8 | RBF | 0.01 | 0.049 | 0.070 | 0.496 | 0.469 |
| 50 | 5 | 1.0 | LIN | - | 0.425 | 0.420 | 0.549 | 0.773 |
| 50 | 5 | 1.0 | RBF | 0.0001 | 0.436 | 0.423 | 0.557 | 0.764 |
| 50 | 5 | 1.0 | RBF | 0.001 | 0.446 | 0.410 | 0.546 | 0.754 |
| 50 | 5 | 1.0 | RBF | 0.01 | 0.029 | 0.050 | 0.496 | 0.469 |
| 50 | 5 | 10 | LIN | - | 0.442 | 0.416 | 0.555 | 0.759 |
| 50 | 5 | 10 | RBF | 0.0001 | 0.436 | 0.423 | 0.557 | 0.764 |
| 50 | 5 | 10 | RBF | 0.001 | 0.446 | 0.410 | 0.546 | 0.754 |
| 50 | 5 | 10 | RBF | 0.01 | 0.009 | 0.030 | 0.498 | 0.469 |
| 50 | 5 | 50 | LIN | - | 0.421 | 0.430 | 0.559 | 0.700 |
| 50 | 5 | 50 | RBF | 0.0001 | 0.436 | 0.423 | 0.557 | 0.764 |
| 50 | 5 | 50 | RBF | 0.001 | 0.446 | 0.410 | 0.546 | 0.754 |
| 50 | 5 | 50 | RBF | 0.01 | 0.009 | 0.030 | 0.498 | 0.468 |
| 50 | 5 | 100 | LIN | - | 0.421 | 0.430 | 0.559 | 0.700 |
| 50 | 5 | 100 | RBF | 0.0001 | 0.436 | 0.423 | 0.557 | 0.764 |
| 50 | 5 | 100 | RBF | 0.001 | 0.446 | 0.410 | 0.546 | 0.754 |
| 50 | 5 | 100 | RBF | 0.01 | 0.004 | 0.025 | 0.498 | 0.468 |
| 50 | 10 | 0.000001 | RBF | 0.0001 | 0.302 | 0.312 | 0.547 | 0.748 |
| 50 | 10 | 0.000001 | RBF | 0.01 | 0.126 | 0.158 | 0.541 | 0.598 |
| 50 | 10 | 0.001 | LIN | - | 0.186 | 0.221 | 0.523 | 0.689 |

Continued on next page

TABLE S16 – continued from previous page

| n | $k$ | $\lambda$ | usim | $\sigma$ | AP@5 | AP@10 | sCI | CI |
|---|---|---|---|---|---|---|---|---|
| 50 | 10 | 0.001 | RBF | 0.0001 | 0.437 | 0.427 | 0.558 | 0.765 |
| 50 | 10 | 0.001 | RBF | 0.001 | 0.449 | 0.419 | 0.548 | 0.747 |
| 50 | 10 | 0.001 | RBF | 0.01 | 0.106 | 0.163 | 0.546 | 0.527 |
| 50 | 10 | 0.01 | LIN | - | 0.205 | 0.226 | 0.520 | 0.722 |
| 50 | 10 | 0.01 | RBF | 0.0001 | 0.437 | 0.427 | 0.558 | 0.765 |
| 50 | 10 | 0.01 | RBF | 0.001 | 0.449 | 0.419 | 0.548 | 0.747 |
| 50 | 10 | 0.01 | RBF | 0.01 | 0.115 | 0.148 | 0.516 | 0.491 |
| 50 | 10 | 0.1 | LIN | - | 0.376 | 0.368 | 0.551 | 0.755 |
| 50 | 10 | 0.1 | RBF | 0.0001 | 0.437 | 0.427 | 0.558 | 0.765 |
| 50 | 10 | 0.1 | RBF | 0.001 | 0.449 | 0.419 | 0.548 | 0.747 |
| 50 | 10 | 0.1 | RBF | 0.01 | 0.070 | 0.081 | 0.493 | 0.474 |
| 50 | 10 | 0.2 | LIN | - | 0.445 | 0.409 | 0.551 | 0.756 |
| 50 | 10 | 0.2 | RBF | 0.0001 | 0.437 | 0.427 | 0.558 | 0.765 |
| 50 | 10 | 0.2 | RBF | 0.001 | 0.449 | 0.419 | 0.548 | 0.747 |
| 50 | 10 | 0.2 | RBF | 0.01 | 0.050 | 0.074 | 0.495 | 0.471 |
| 50 | 10 | 0.4 | LIN | - | 0.432 | 0.415 | 0.556 | 0.757 |
| 50 | 10 | 0.4 | RBF | 0.0001 | 0.437 | 0.427 | 0.558 | 0.765 |
| 50 | 10 | 0.4 | RBF | 0.001 | 0.449 | 0.419 | 0.548 | 0.747 |
| 50 | 10 | 0.4 | RBF | 0.01 | 0.059 | 0.080 | 0.494 | 0.470 |
| 50 | 10 | 0.6 | LIN | - | 0.425 | 0.403 | 0.555 | 0.761 |
| 50 | 10 | 0.6 | RBF | 0.0001 | 0.437 | 0.427 | 0.558 | 0.765 |
| 50 | 10 | 0.6 | RBF | 0.001 | 0.449 | 0.419 | 0.548 | 0.747 |
| 50 | 10 | 0.6 | RBF | 0.01 | 0.039 | 0.060 | 0.496 | 0.469 |
| 50 | 10 | 0.8 | LIN | - | 0.419 | 0.407 | 0.559 | 0.762 |
| 50 | 10 | 0.8 | RBF | 0.0001 | 0.437 | 0.427 | 0.558 | 0.765 |
| 50 | 10 | 0.8 | RBF | 0.001 | 0.449 | 0.419 | 0.548 | 0.747 |
| 50 | 10 | 0.8 | RBF | 0.01 | 0.049 | 0.070 | 0.496 | 0.469 |
| 50 | 10 | 1.0 | LIN | - | 0.409 | 0.401 | 0.553 | 0.762 |
| 50 | 10 | 1.0 | RBF | 0.0001 | 0.437 | 0.427 | 0.558 | 0.765 |
| 50 | 10 | 1.0 | RBF | 0.001 | 0.449 | 0.419 | 0.548 | 0.747 |
| 50 | 10 | 1.0 | RBF | 0.01 | 0.029 | 0.050 | 0.496 | 0.469 |
| 50 | 10 | 10 | LIN | - | 0.445 | 0.425 | 0.552 | 0.773 |
| 50 | 10 | 10 | RBF | 0.0001 | 0.437 | 0.427 | 0.558 | 0.765 |
| 50 | 10 | 10 | RBF | 0.001 | 0.449 | 0.419 | 0.548 | 0.747 |
| 50 | 10 | 10 | RBF | 0.01 | 0.009 | 0.030 | 0.498 | 0.469 |
| 50 | 10 | 50 | LIN | - | 0.440 | 0.436 | 0.548 | 0.771 |
| 50 | 10 | 50 | RBF | 0.0001 | 0.437 | 0.427 | 0.558 | 0.765 |
| 50 | 10 | 50 | RBF | 0.001 | 0.449 | 0.419 | 0.548 | 0.747 |
| 50 | 10 | 50 | RBF | 0.01 | 0.011 | 0.032 | 0.498 | 0.468 |
| 50 | 10 | 100 | LIN | - | 0.442 | 0.424 | 0.545 | 0.768 |
| 50 | 10 | 100 | RBF | 0.0001 | 0.437 | 0.427 | 0.558 | 0.765 |
| 50 | 10 | 100 | RBF | 0.001 | 0.449 | 0.419 | 0.548 | 0.747 |
| 50 | 10 | 100 | RBF | 0.01 | 0.004 | 0.025 | 0.498 | 0.468 |
| 50 | 15 | 0.001 | RBF | 0.0001 | 0.442 | 0.436 | 0.552 | 0.764 |
| 50 | 15 | 0.001 | RBF | 0.001 | 0.441 | 0.423 | 0.548 | 0.746 |
| 50 | 15 | 0.001 | RBF | 0.01 | 0.119 | 0.160 | 0.547 | 0.525 |
| 50 | 15 | 0.01 | LIN | - | 0.434 | 0.383 | 0.548 | 0.738 |
| 50 | 15 | 0.01 | RBF | 0.0001 | 0.442 | 0.436 | 0.552 | 0.764 |
| 50 | 15 | 0.01 | RBF | 0.001 | 0.441 | 0.423 | 0.548 | 0.746 |
| 50 | 15 | 0.01 | RBF | 0.01 | 0.100 | 0.131 | 0.518 | 0.490 |
| 50 | 15 | 0.1 | LIN | - | 0.404 | 0.386 | 0.543 | 0.738 |
| 50 | 15 | 0.1 | RBF | 0.0001 | 0.442 | 0.436 | 0.552 | 0.764 |
| 50 | 15 | 0.1 | RBF | 0.001 | 0.441 | 0.423 | 0.548 | 0.746 |
| 50 | 15 | 0.1 | RBF | 0.01 | 0.079 | 0.094 | 0.498 | 0.474 |
| 50 | 15 | 0.2 | LIN | - | 0.389 | 0.375 | 0.547 | 0.744 |
| 50 | 15 | 0.2 | RBF | 0.0001 | 0.442 | 0.436 | 0.552 | 0.764 |
| 50 | 15 | 0.2 | RBF | 0.001 | 0.441 | 0.423 | 0.548 | 0.746 |
| 50 | 15 | 0.2 | RBF | 0.01 | 0.051 | 0.075 | 0.498 | 0.471 |

Continued on next page

TABLE S16 – continued from previous page

| n | $k$ | $\lambda$ | usim | $\sigma$ | AP@5 | AP@10 | sCI | CI |
|---|---|---|---|---|---|---|---|---|
| 50 | 15 | 0.4 | LIN | - | 0.429 | 0.430 | 0.532 | 0.732 |
| 50 | 15 | 0.4 | RBF | 0.0001 | 0.442 | 0.436 | 0.552 | 0.764 |
| 50 | 15 | 0.4 | RBF | 0.001 | 0.441 | 0.423 | 0.548 | 0.746 |
| 50 | 15 | 0.4 | RBF | 0.01 | 0.056 | 0.077 | 0.496 | 0.470 |
| 50 | 15 | 0.6 | LIN | - | 0.377 | 0.369 | 0.539 | 0.741 |
| 50 | 15 | 0.6 | RBF | 0.0001 | 0.442 | 0.436 | 0.552 | 0.764 |
| 50 | 15 | 0.6 | RBF | 0.001 | 0.441 | 0.423 | 0.548 | 0.746 |
| 50 | 15 | 0.6 | RBF | 0.01 | 0.039 | 0.060 | 0.496 | 0.469 |
| 50 | 15 | 0.8 | LIN | - | 0.425 | 0.424 | 0.505 | 0.738 |
| 50 | 15 | 0.8 | RBF | 0.0001 | 0.442 | 0.436 | 0.552 | 0.764 |
| 50 | 15 | 0.8 | RBF | 0.001 | 0.441 | 0.423 | 0.548 | 0.746 |
| 50 | 15 | 0.8 | RBF | 0.01 | 0.039 | 0.060 | 0.496 | 0.469 |
| 50 | 15 | 1.0 | LIN | - | 0.434 | 0.431 | 0.528 | 0.741 |
| 50 | 15 | 1.0 | RBF | 0.0001 | 0.442 | 0.436 | 0.552 | 0.764 |
| 50 | 15 | 1.0 | RBF | 0.001 | 0.441 | 0.423 | 0.548 | 0.746 |
| 50 | 15 | 1.0 | RBF | 0.01 | 0.019 | 0.040 | 0.496 | 0.469 |
| 50 | 15 | 10 | LIN | - | 0.439 | 0.429 | 0.558 | 0.718 |
| 50 | 15 | 10 | RBF | 0.0001 | 0.442 | 0.436 | 0.552 | 0.764 |
| 50 | 15 | 10 | RBF | 0.001 | 0.441 | 0.423 | 0.548 | 0.746 |
| 50 | 15 | 10 | RBF | 0.01 | 0.009 | 0.030 | 0.498 | 0.469 |
| 50 | 15 | 50 | LIN | - | 0.440 | 0.423 | 0.545 | 0.756 |
| 50 | 15 | 50 | RBF | 0.0001 | 0.442 | 0.436 | 0.552 | 0.764 |
| 50 | 15 | 50 | RBF | 0.001 | 0.441 | 0.423 | 0.549 | 0.746 |
| 50 | 15 | 50 | RBF | 0.01 | 0.009 | 0.030 | 0.498 | 0.468 |
| 50 | 15 | 100 | LIN | - | 0.440 | 0.428 | 0.548 | 0.766 |
| 50 | 15 | 100 | RBF | 0.0001 | 0.442 | 0.436 | 0.552 | 0.764 |
| 50 | 15 | 100 | RBF | 0.001 | 0.441 | 0.423 | 0.549 | 0.746 |
| 50 | 15 | 100 | RBF | 0.01 | 0.004 | 0.025 | 0.498 | 0.468 |
| 100 | 5 | 0.000001 | RBF | 0.0001 | 0.353 | 0.353 | 0.512 | 0.718 |
| 100 | 5 | 0.000001 | RBF | 0.001 | 0.291 | 0.303 | 0.539 | 0.715 |
| 100 | 5 | 0.000001 | RBF | 0.01 | 0.133 | 0.162 | 0.522 | 0.585 |
| 100 | 5 | 0.00001 | LIN | - | 0.136 | 0.163 | 0.536 | 0.703 |
| 100 | 5 | 0.00001 | RBF | 0.001 | 0.365 | 0.347 | 0.551 | 0.748 |
| 100 | 5 | 0.00001 | RBF | 0.01 | 0.117 | 0.140 | 0.519 | 0.589 |
| 100 | 5 | 0.0001 | RBF | 0.0001 | 0.378 | 0.353 | 0.558 | 0.763 |
| 100 | 5 | 0.0001 | RBF | 0.001 | 0.365 | 0.347 | 0.551 | 0.748 |
| 100 | 5 | 0.0001 | RBF | 0.01 | 0.122 | 0.145 | 0.525 | 0.552 |
| 100 | 5 | 0.001 | LIN | - | 0.267 | 0.263 | 0.523 | 0.701 |
| 100 | 5 | 0.001 | RBF | 0.0001 | 0.378 | 0.353 | 0.558 | 0.763 |
| 100 | 5 | 0.001 | RBF | 0.001 | 0.365 | 0.347 | 0.551 | 0.748 |
| 100 | 5 | 0.001 | RBF | 0.01 | 0.111 | 0.138 | 0.521 | 0.518 |
| 100 | 5 | 0.01 | LIN | - | 0.312 | 0.305 | 0.516 | 0.712 |
| 100 | 5 | 0.01 | RBF | 0.0001 | 0.378 | 0.353 | 0.558 | 0.763 |
| 100 | 5 | 0.01 | RBF | 0.001 | 0.365 | 0.347 | 0.551 | 0.748 |
| 100 | 5 | 0.01 | RBF | 0.01 | 0.084 | 0.103 | 0.505 | 0.491 |
| 100 | 5 | 0.1 | LIN | - | 0.392 | 0.369 | 0.538 | 0.754 |
| 100 | 5 | 0.1 | RBF | 0.0001 | 0.378 | 0.353 | 0.558 | 0.763 |
| 100 | 5 | 0.1 | RBF | 0.001 | 0.365 | 0.347 | 0.551 | 0.748 |
| 100 | 5 | 0.1 | RBF | 0.01 | 0.063 | 0.080 | 0.505 | 0.475 |
| 100 | 5 | 0.2 | LIN | - | 0.343 | 0.334 | 0.547 | 0.759 |
| 100 | 5 | 0.2 | RBF | 0.0001 | 0.378 | 0.353 | 0.558 | 0.763 |
| 100 | 5 | 0.2 | RBF | 0.001 | 0.365 | 0.347 | 0.551 | 0.748 |
| 100 | 5 | 0.2 | RBF | 0.01 | 0.050 | 0.068 | 0.501 | 0.473 |
| 100 | 5 | 0.4 | LIN | - | 0.399 | 0.393 | 0.545 | 0.763 |
| 100 | 5 | 0.4 | RBF | 0.0001 | 0.378 | 0.353 | 0.558 | 0.763 |
| 100 | 5 | 0.4 | RBF | 0.001 | 0.365 | 0.347 | 0.551 | 0.748 |
| 100 | 5 | 0.4 | RBF | 0.01 | 0.040 | 0.058 | 0.501 | 0.471 |
| 100 | 5 | 0.6 | LIN | - | 0.369 | 0.355 | 0.544 | 0.763 |

Continued on next page

TABLE S16 – continued from previous page

| n | $k$ | $\lambda$ | usim | $\sigma$ | AP@5 | AP@10 | sCI | CI |
|---|---|---|---|---|---|---|---|---|
| 100 | 5 | 0.6 | RBF | 0.0001 | 0.378 | 0.353 | 0.558 | 0.763 |
| 100 | 5 | 0.6 | RBF | 0.001 | 0.365 | 0.347 | 0.551 | 0.748 |
| 100 | 5 | 0.6 | RBF | 0.01 | 0.034 | 0.052 | 0.502 | 0.470 |
| 100 | 5 | 0.8 | LIN | - | 0.400 | 0.394 | 0.546 | 0.763 |
| 100 | 5 | 0.8 | RBF | 0.0001 | 0.378 | 0.353 | 0.558 | 0.763 |
| 100 | 5 | 0.8 | RBF | 0.001 | 0.365 | 0.347 | 0.551 | 0.748 |
| 100 | 5 | 0.8 | RBF | 0.01 | 0.037 | 0.056 | 0.497 | 0.469 |
| 100 | 5 | 1.0 | LIN | - | 0.336 | 0.337 | 0.542 | 0.768 |
| 100 | 5 | 1.0 | RBF | 0.0001 | 0.378 | 0.353 | 0.558 | 0.763 |
| 100 | 5 | 1.0 | RBF | 0.001 | 0.365 | 0.347 | 0.551 | 0.748 |
| 100 | 5 | 1.0 | RBF | 0.01 | 0.021 | 0.039 | 0.497 | 0.469 |
| 100 | 5 | 10 | LIN | - | 0.368 | 0.359 | 0.544 | 0.759 |
| 100 | 5 | 10 | RBF | 0.0001 | 0.378 | 0.353 | 0.558 | 0.763 |
| 100 | 5 | 10 | RBF | 0.001 | 0.365 | 0.347 | 0.551 | 0.748 |
| 100 | 5 | 10 | RBF | 0.01 | 0.007 | 0.025 | 0.500 | 0.468 |
| 100 | 5 | 50 | LIN | - | 0.378 | 0.364 | 0.559 | 0.698 |
| 100 | 5 | 50 | RBF | 0.0001 | 0.378 | 0.353 | 0.558 | 0.763 |
| 100 | 5 | 50 | RBF | 0.001 | 0.365 | 0.347 | 0.551 | 0.748 |
| 100 | 5 | 50 | RBF | 0.01 | 0.005 | 0.023 | 0.499 | 0.467 |
| 100 | 5 | 100 | LIN | - | 0.378 | 0.364 | 0.559 | 0.698 |
| 100 | 5 | 100 | RBF | 0.0001 | 0.378 | 0.353 | 0.558 | 0.763 |
| 100 | 5 | 100 | RBF | 0.001 | 0.365 | 0.347 | 0.551 | 0.748 |
| 100 | 5 | 100 | RBF | 0.01 | 0.005 | 0.023 | 0.499 | 0.467 |
| 100 | 10 | 0.000001 | RBF | 0.01 | 0.134 | 0.159 | 0.522 | 0.581 |
| 100 | 10 | 0.001 | LIN | - | 0.187 | 0.199 | 0.527 | 0.709 |
| 100 | 10 | 0.001 | RBF | 0.0001 | 0.380 | 0.380 | 0.552 | 0.763 |
| 100 | 10 | 0.001 | RBF | 0.001 | 0.367 | 0.364 | 0.548 | 0.741 |
| 100 | 10 | 0.001 | RBF | 0.01 | 0.114 | 0.140 | 0.518 | 0.517 |
| 100 | 10 | 0.01 | LIN | - | 0.144 | 0.179 | 0.487 | 0.712 |
| 100 | 10 | 0.01 | RBF | 0.0001 | 0.380 | 0.380 | 0.552 | 0.763 |
| 100 | 10 | 0.01 | RBF | 0.001 | 0.367 | 0.364 | 0.548 | 0.741 |
| 100 | 10 | 0.01 | RBF | 0.01 | 0.117 | 0.133 | 0.502 | 0.491 |
| 100 | 10 | 0.1 | LIN | - | 0.206 | 0.246 | 0.535 | 0.731 |
| 100 | 10 | 0.1 | RBF | 0.0001 | 0.380 | 0.380 | 0.552 | 0.763 |
| 100 | 10 | 0.1 | RBF | 0.001 | 0.367 | 0.364 | 0.548 | 0.741 |
| 100 | 10 | 0.1 | RBF | 0.01 | 0.082 | 0.093 | 0.504 | 0.476 |
| 100 | 10 | 0.2 | LIN | - | 0.360 | 0.359 | 0.544 | 0.754 |
| 100 | 10 | 0.2 | RBF | 0.0001 | 0.380 | 0.380 | 0.552 | 0.763 |
| 100 | 10 | 0.2 | RBF | 0.001 | 0.367 | 0.364 | 0.548 | 0.741 |
| 100 | 10 | 0.2 | RBF | 0.01 | 0.064 | 0.080 | 0.503 | 0.473 |
| 100 | 10 | 0.4 | LIN | - | 0.408 | 0.398 | 0.543 | 0.758 |
| 100 | 10 | 0.4 | RBF | 0.0001 | 0.380 | 0.380 | 0.552 | 0.763 |
| 100 | 10 | 0.4 | RBF | 0.001 | 0.367 | 0.364 | 0.548 | 0.741 |
| 100 | 10 | 0.4 | RBF | 0.01 | 0.045 | 0.062 | 0.501 | 0.471 |
| 100 | 10 | 0.6 | LIN | - | 0.409 | 0.403 | 0.544 | 0.758 |
| 100 | 10 | 0.6 | RBF | 0.0001 | 0.380 | 0.380 | 0.552 | 0.763 |
| 100 | 10 | 0.6 | RBF | 0.001 | 0.367 | 0.364 | 0.548 | 0.741 |
| 100 | 10 | 0.6 | RBF | 0.01 | 0.040 | 0.057 | 0.501 | 0.470 |
| 100 | 10 | 0.8 | LIN | - | 0.393 | 0.376 | 0.548 | 0.759 |
| 100 | 10 | 0.8 | RBF | 0.0001 | 0.380 | 0.380 | 0.552 | 0.763 |
| 100 | 10 | 0.8 | RBF | 0.001 | 0.367 | 0.364 | 0.548 | 0.741 |
| 100 | 10 | 0.8 | RBF | 0.01 | 0.036 | 0.052 | 0.499 | 0.470 |
| 100 | 10 | 1.0 | LIN | - | 0.399 | 0.377 | 0.544 | 0.759 |
| 100 | 10 | 1.0 | RBF | 0.0001 | 0.380 | 0.380 | 0.552 | 0.763 |
| 100 | 10 | 1.0 | RBF | 0.001 | 0.367 | 0.364 | 0.548 | 0.741 |
| 100 | 10 | 1.0 | RBF | 0.01 | 0.027 | 0.042 | 0.499 | 0.469 |
| 100 | 10 | 10 | LIN | - | 0.339 | 0.334 | 0.545 | 0.768 |
| 100 | 10 | 10 | RBF | 0.0001 | 0.380 | 0.380 | 0.552 | 0.763 |

Continued on next page

TABLE S16 – continued from previous page

| n | $k$ | $\lambda$ | usim | $\sigma$ | AP@5 | AP@10 | sCI | CI |
|---|---|---|---|---|---|---|---|---|
| 100 | 10 | 10 | RBF | 0.001 | 0.367 | 0.364 | 0.548 | 0.741 |
| 100 | 10 | 10 | RBF | 0.01 | 0.007 | 0.027 | 0.501 | 0.468 |
| 100 | 10 | 50 | LIN | - | 0.369 | 0.380 | 0.541 | 0.770 |
| 100 | 10 | 50 | RBF | 0.0001 | 0.380 | 0.380 | 0.552 | 0.763 |
| 100 | 10 | 50 | RBF | 0.001 | 0.367 | 0.364 | 0.548 | 0.741 |
| 100 | 10 | 50 | RBF | 0.01 | 0.008 | 0.026 | 0.500 | 0.467 |
| 100 | 10 | 100 | LIN | - | 0.369 | 0.379 | 0.542 | 0.768 |
| 100 | 10 | 100 | RBF | 0.0001 | 0.380 | 0.380 | 0.552 | 0.763 |
| 100 | 10 | 100 | RBF | 0.001 | 0.367 | 0.364 | 0.548 | 0.741 |
| 100 | 10 | 100 | RBF | 0.01 | 0.005 | 0.023 | 0.499 | 0.467 |
| 100 | 15 | 0.001 | LIN | - | 0.179 | 0.208 | 0.536 | 0.714 |
| 100 | 15 | 0.001 | RBF | 0.0001 | 0.372 | 0.381 | 0.550 | 0.763 |
| 100 | 15 | 0.001 | RBF | 0.001 | 0.371 | 0.363 | 0.546 | 0.740 |
| 100 | 15 | 0.001 | RBF | 0.01 | 0.110 | 0.141 | 0.520 | 0.516 |
| 100 | 15 | 0.01 | LIN | - | 0.197 | 0.222 | 0.527 | 0.718 |
| 100 | 15 | 0.01 | RBF | 0.0001 | 0.372 | 0.381 | 0.550 | 0.763 |
| 100 | 15 | 0.01 | RBF | 0.001 | 0.371 | 0.363 | 0.546 | 0.740 |
| 100 | 15 | 0.01 | RBF | 0.01 | 0.100 | 0.124 | 0.508 | 0.490 |
| 100 | 15 | 0.1 | LIN | - | 0.217 | 0.232 | 0.544 | 0.731 |
| 100 | 15 | 0.1 | RBF | 0.0001 | 0.372 | 0.381 | 0.550 | 0.763 |
| 100 | 15 | 0.1 | RBF | 0.001 | 0.371 | 0.363 | 0.546 | 0.740 |
| 100 | 15 | 0.1 | RBF | 0.01 | 0.077 | 0.087 | 0.504 | 0.476 |
| 100 | 15 | 0.2 | LIN | - | 0.276 | 0.287 | 0.525 | 0.723 |
| 100 | 15 | 0.2 | RBF | 0.0001 | 0.372 | 0.381 | 0.550 | 0.763 |
| 100 | 15 | 0.2 | RBF | 0.001 | 0.371 | 0.363 | 0.546 | 0.740 |
| 100 | 15 | 0.2 | RBF | 0.01 | 0.066 | 0.081 | 0.504 | 0.473 |
| 100 | 15 | 0.4 | LIN | - | 0.346 | 0.343 | 0.534 | 0.731 |
| 100 | 15 | 0.4 | RBF | 0.0001 | 0.372 | 0.381 | 0.550 | 0.763 |
| 100 | 15 | 0.4 | RBF | 0.001 | 0.371 | 0.363 | 0.546 | 0.740 |
| 100 | 15 | 0.4 | RBF | 0.01 | 0.050 | 0.067 | 0.502 | 0.471 |
| 100 | 15 | 0.6 | LIN | - | 0.260 | 0.283 | 0.528 | 0.736 |
| 100 | 15 | 0.6 | RBF | 0.0001 | 0.372 | 0.381 | 0.550 | 0.763 |
| 100 | 15 | 0.6 | RBF | 0.001 | 0.371 | 0.363 | 0.546 | 0.740 |
| 100 | 15 | 0.6 | RBF | 0.01 | 0.042 | 0.058 | 0.501 | 0.470 |
| 100 | 15 | 0.8 | LIN | - | 0.301 | 0.282 | 0.524 | 0.734 |
| 100 | 15 | 0.8 | RBF | 0.0001 | 0.372 | 0.381 | 0.550 | 0.763 |
| 100 | 15 | 0.8 | RBF | 0.001 | 0.371 | 0.363 | 0.546 | 0.740 |
| 100 | 15 | 0.8 | RBF | 0.01 | 0.046 | 0.062 | 0.500 | 0.469 |
| 100 | 15 | 1.0 | LIN | - | 0.276 | 0.286 | 0.523 | 0.729 |
| 100 | 15 | 1.0 | RBF | 0.0001 | 0.372 | 0.381 | 0.550 | 0.763 |
| 100 | 15 | 1.0 | RBF | 0.001 | 0.371 | 0.363 | 0.546 | 0.740 |
| 100 | 15 | 1.0 | RBF | 0.01 | 0.030 | 0.045 | 0.499 | 0.469 |
| 100 | 15 | 10 | LIN | - | 0.381 | 0.378 | 0.557 | 0.703 |
| 100 | 15 | 10 | RBF | 0.0001 | 0.372 | 0.381 | 0.550 | 0.763 |
| 100 | 15 | 10 | RBF | 0.001 | 0.371 | 0.363 | 0.546 | 0.740 |
| 100 | 15 | 10 | RBF | 0.01 | 0.010 | 0.028 | 0.501 | 0.468 |
| 100 | 15 | 50 | LIN | - | 0.369 | 0.382 | 0.542 | 0.769 |
| 100 | 15 | 50 | RBF | 0.0001 | 0.372 | 0.381 | 0.550 | 0.763 |
| 100 | 15 | 50 | RBF | 0.001 | 0.371 | 0.363 | 0.546 | 0.740 |
| 100 | 15 | 50 | RBF | 0.01 | 0.010 | 0.028 | 0.500 | 0.467 |
| 100 | 15 | 100 | LIN | - | 0.369 | 0.379 | 0.544 | 0.768 |
| 100 | 15 | 100 | RBF | 0.0001 | 0.372 | 0.381 | 0.550 | 0.763 |
| 100 | 15 | 100 | RBF | 0.001 | 0.371 | 0.363 | 0.546 | 0.740 |
| 100 | 15 | 100 | RBF | 0.01 | 0.015 | 0.033 | 0.500 | 0.467 |
| 150 | 5 | 0.000001 | RBF | 0.0001 | 0.343 | 0.334 | 0.568 | 0.732 |
| 150 | 5 | 0.000001 | RBF | 0.001 | 0.267 | 0.278 | 0.558 | 0.703 |
| 150 | 5 | 0.000001 | RBF | 0.01 | 0.143 | 0.166 | 0.529 | 0.576 |
| 150 | 5 | 0.00001 | RBF | 0.001 | 0.382 | 0.367 | 0.563 | 0.740 |

Continued on next page

TABLE S16 – continued from previous page

| n | $k$ | $\lambda$ | usim | $\sigma$ | AP@5 | AP@10 | sCI | CI |
|---|---|---|---|---|---|---|---|---|
| 150 | 5 | 0.00001 | RBF | 0.01 | 0.135 | 0.164 | 0.517 | 0.579 |
| 150 | 5 | 0.0001 | RBF | 0.0001 | 0.395 | 0.381 | 0.567 | 0.757 |
| 150 | 5 | 0.0001 | RBF | 0.001 | 0.382 | 0.367 | 0.563 | 0.740 |
| 150 | 5 | 0.0001 | RBF | 0.01 | 0.141 | 0.156 | 0.525 | 0.544 |
| 150 | 5 | 0.001 | LIN | - | 0.212 | 0.235 | 0.561 | 0.707 |
| 150 | 5 | 0.001 | RBF | 0.0001 | 0.395 | 0.381 | 0.567 | 0.757 |
| 150 | 5 | 0.001 | RBF | 0.001 | 0.382 | 0.367 | 0.563 | 0.740 |
| 150 | 5 | 0.001 | RBF | 0.01 | 0.122 | 0.148 | 0.524 | 0.512 |
| 150 | 5 | 0.01 | LIN | - | 0.253 | 0.282 | 0.555 | 0.721 |
| 150 | 5 | 0.01 | RBF | 0.0001 | 0.395 | 0.381 | 0.567 | 0.757 |
| 150 | 5 | 0.01 | RBF | 0.001 | 0.382 | 0.367 | 0.563 | 0.740 |
| 150 | 5 | 0.01 | RBF | 0.01 | 0.107 | 0.124 | 0.511 | 0.488 |
| 150 | 5 | 0.1 | LIN | - | 0.294 | 0.294 | 0.567 | 0.750 |
| 150 | 5 | 0.1 | RBF | 0.0001 | 0.395 | 0.381 | 0.567 | 0.757 |
| 150 | 5 | 0.1 | RBF | 0.001 | 0.382 | 0.367 | 0.563 | 0.740 |
| 150 | 5 | 0.1 | RBF | 0.01 | 0.083 | 0.094 | 0.502 | 0.475 |
| 150 | 5 | 0.2 | LIN | - | 0.367 | 0.349 | 0.568 | 0.702 |
| 150 | 5 | 0.2 | RBF | 0.0001 | 0.395 | 0.381 | 0.567 | 0.757 |
| 150 | 5 | 0.2 | RBF | 0.001 | 0.382 | 0.367 | 0.563 | 0.740 |
| 150 | 5 | 0.2 | RBF | 0.01 | 0.076 | 0.090 | 0.497 | 0.473 |
| 150 | 5 | 0.4 | LIN | - | 0.391 | 0.377 | 0.566 | 0.757 |
| 150 | 5 | 0.4 | RBF | 0.0001 | 0.395 | 0.381 | 0.567 | 0.757 |
| 150 | 5 | 0.4 | RBF | 0.001 | 0.382 | 0.367 | 0.563 | 0.740 |
| 150 | 5 | 0.4 | RBF | 0.01 | 0.060 | 0.072 | 0.497 | 0.471 |
| 150 | 5 | 0.6 | LIN | - | 0.397 | 0.361 | 0.564 | 0.764 |
| 150 | 5 | 0.6 | RBF | 0.0001 | 0.395 | 0.381 | 0.567 | 0.757 |
| 150 | 5 | 0.6 | RBF | 0.001 | 0.382 | 0.367 | 0.563 | 0.740 |
| 150 | 5 | 0.6 | RBF | 0.01 | 0.050 | 0.066 | 0.496 | 0.470 |
| 150 | 5 | 0.8 | LIN | - | 0.350 | 0.324 | 0.564 | 0.757 |
| 150 | 5 | 0.8 | RBF | 0.0001 | 0.395 | 0.381 | 0.567 | 0.757 |
| 150 | 5 | 0.8 | RBF | 0.001 | 0.382 | 0.367 | 0.563 | 0.740 |
| 150 | 5 | 0.8 | RBF | 0.01 | 0.039 | 0.054 | 0.495 | 0.470 |
| 150 | 5 | 1.0 | LIN | - | 0.337 | 0.332 | 0.561 | 0.762 |
| 150 | 5 | 1.0 | RBF | 0.0001 | 0.395 | 0.381 | 0.567 | 0.757 |
| 150 | 5 | 1.0 | RBF | 0.001 | 0.382 | 0.367 | 0.563 | 0.740 |
| 150 | 5 | 1.0 | RBF | 0.01 | 0.039 | 0.054 | 0.495 | 0.469 |
| 150 | 5 | 10 | LIN | - | 0.369 | 0.358 | 0.561 | 0.755 |
| 150 | 5 | 10 | RBF | 0.0001 | 0.395 | 0.381 | 0.567 | 0.757 |
| 150 | 5 | 10 | RBF | 0.001 | 0.382 | 0.367 | 0.563 | 0.740 |
| 150 | 5 | 10 | RBF | 0.01 | 0.026 | 0.043 | 0.497 | 0.468 |
| 150 | 5 | 50 | LIN | - | 0.387 | 0.371 | 0.570 | 0.692 |
| 150 | 5 | 50 | RBF | 0.0001 | 0.395 | 0.381 | 0.567 | 0.757 |
| 150 | 5 | 50 | RBF | 0.001 | 0.382 | 0.367 | 0.563 | 0.740 |
| 150 | 5 | 50 | RBF | 0.01 | 0.025 | 0.040 | 0.496 | 0.467 |
| 150 | 5 | 100 | LIN | - | 0.387 | 0.371 | 0.570 | 0.692 |
| 150 | 5 | 100 | RBF | 0.0001 | 0.395 | 0.381 | 0.567 | 0.757 |
| 150 | 5 | 100 | RBF | 0.001 | 0.382 | 0.367 | 0.563 | 0.740 |
| 150 | 5 | 100 | RBF | 0.01 | 0.025 | 0.040 | 0.496 | 0.467 |
| 150 | 10 | 0.000001 | RBF | 0.01 | 0.153 | 0.177 | 0.528 | 0.570 |
| 150 | 10 | 0.001 | LIN | - | 0.208 | 0.221 | 0.553 | 0.715 |
| 150 | 10 | 0.001 | RBF | 0.0001 | 0.393 | 0.377 | 0.564 | 0.757 |
| 150 | 10 | 0.001 | RBF | 0.001 | 0.385 | 0.363 | 0.564 | 0.732 |
| 150 | 10 | 0.001 | RBF | 0.01 | 0.141 | 0.160 | 0.528 | 0.508 |
| 150 | 10 | 0.01 | LIN | - | 0.287 | 0.289 | 0.547 | 0.710 |
| 150 | 10 | 0.01 | RBF | 0.0001 | 0.393 | 0.377 | 0.564 | 0.757 |
| 150 | 10 | 0.01 | RBF | 0.001 | 0.385 | 0.363 | 0.564 | 0.732 |
| 150 | 10 | 0.01 | RBF | 0.01 | 0.120 | 0.135 | 0.509 | 0.488 |
| 150 | 10 | 0.1 | LIN | - | 0.357 | 0.347 | 0.516 | 0.707 |

Continued on next page

TABLE S16 – continued from previous page

| n | $k$ | $\lambda$ | usim | $\sigma$ | AP@5 | AP@10 | sCI | CI |
|---|---|---|---|---|---|---|---|---|
| 150 | 10 | 0.1 | RBF | 0.0001 | 0.393 | 0.377 | 0.564 | 0.757 |
| 150 | 10 | 0.1 | RBF | 0.001 | 0.385 | 0.363 | 0.564 | 0.732 |
| 150 | 10 | 0.1 | RBF | 0.01 | 0.085 | 0.096 | 0.500 | 0.475 |
| 150 | 10 | 0.2 | LIN | - | 0.245 | 0.257 | 0.553 | 0.658 |
| 150 | 10 | 0.2 | RBF | 0.0001 | 0.393 | 0.377 | 0.564 | 0.757 |
| 150 | 10 | 0.2 | RBF | 0.001 | 0.385 | 0.363 | 0.564 | 0.732 |
| 150 | 10 | 0.2 | RBF | 0.01 | 0.073 | 0.086 | 0.497 | 0.473 |
| 150 | 10 | 0.4 | LIN | - | 0.397 | 0.385 | 0.571 | 0.750 |
| 150 | 10 | 0.4 | RBF | 0.0001 | 0.393 | 0.377 | 0.564 | 0.757 |
| 150 | 10 | 0.4 | RBF | 0.001 | 0.385 | 0.363 | 0.564 | 0.732 |
| 150 | 10 | 0.4 | RBF | 0.01 | 0.059 | 0.072 | 0.496 | 0.471 |
| 150 | 10 | 0.6 | LIN | - | 0.399 | 0.390 | 0.568 | 0.751 |
| 150 | 10 | 0.6 | RBF | 0.0001 | 0.393 | 0.377 | 0.564 | 0.757 |
| 150 | 10 | 0.6 | RBF | 0.001 | 0.385 | 0.363 | 0.564 | 0.732 |
| 150 | 10 | 0.6 | RBF | 0.01 | 0.052 | 0.065 | 0.495 | 0.470 |
| 150 | 10 | 0.8 | LIN | - | 0.370 | 0.355 | 0.572 | 0.752 |
| 150 | 10 | 0.8 | RBF | 0.0001 | 0.393 | 0.377 | 0.564 | 0.757 |
| 150 | 10 | 0.8 | RBF | 0.001 | 0.385 | 0.363 | 0.564 | 0.732 |
| 150 | 10 | 0.8 | RBF | 0.01 | 0.045 | 0.057 | 0.494 | 0.470 |
| 150 | 10 | 1.0 | LIN | - | 0.386 | 0.357 | 0.568 | 0.753 |
| 150 | 10 | 1.0 | RBF | 0.0001 | 0.393 | 0.377 | 0.564 | 0.757 |
| 150 | 10 | 1.0 | RBF | 0.001 | 0.385 | 0.363 | 0.564 | 0.732 |
| 150 | 10 | 1.0 | RBF | 0.01 | 0.045 | 0.057 | 0.494 | 0.469 |
| 150 | 10 | 10 | LIN | - | 0.374 | 0.368 | 0.562 | 0.764 |
| 150 | 10 | 10 | RBF | 0.0001 | 0.393 | 0.377 | 0.564 | 0.757 |
| 150 | 10 | 10 | RBF | 0.001 | 0.385 | 0.363 | 0.564 | 0.732 |
| 150 | 10 | 10 | RBF | 0.01 | 0.028 | 0.043 | 0.497 | 0.468 |
| 150 | 10 | 50 | LIN | - | 0.386 | 0.389 | 0.557 | 0.756 |
| 150 | 10 | 50 | RBF | 0.0001 | 0.393 | 0.377 | 0.564 | 0.757 |
| 150 | 10 | 50 | RBF | 0.001 | 0.385 | 0.363 | 0.564 | 0.732 |
| 150 | 10 | 50 | RBF | 0.01 | 0.028 | 0.044 | 0.497 | 0.467 |
| 150 | 10 | 100 | LIN | - | 0.386 | 0.388 | 0.559 | 0.760 |
| 150 | 10 | 100 | RBF | 0.0001 | 0.393 | 0.377 | 0.564 | 0.757 |
| 150 | 10 | 100 | RBF | 0.001 | 0.385 | 0.363 | 0.564 | 0.732 |
| 150 | 10 | 100 | RBF | 0.01 | 0.025 | 0.040 | 0.496 | 0.467 |
| 150 | 15 | 0.001 | LIN | - | 0.141 | 0.173 | 0.510 | 0.717 |
| 150 | 15 | 0.001 | RBF | 0.0001 | 0.389 | 0.389 | 0.562 | 0.756 |
| 150 | 15 | 0.001 | RBF | 0.001 | 0.386 | 0.368 | 0.565 | 0.731 |
| 150 | 15 | 0.001 | RBF | 0.01 | 0.132 | 0.150 | 0.525 | 0.508 |
| 150 | 15 | 0.01 | LIN | - | 0.187 | 0.214 | 0.529 | 0.723 |
| 150 | 15 | 0.01 | RBF | 0.0001 | 0.389 | 0.389 | 0.562 | 0.756 |
| 150 | 15 | 0.01 | RBF | 0.001 | 0.386 | 0.368 | 0.565 | 0.731 |
| 150 | 15 | 0.01 | RBF | 0.01 | 0.108 | 0.124 | 0.512 | 0.488 |
| 150 | 15 | 0.1 | LIN | - | 0.366 | 0.359 | 0.540 | 0.733 |
| 150 | 15 | 0.1 | RBF | 0.0001 | 0.389 | 0.389 | 0.562 | 0.756 |
| 150 | 15 | 0.1 | RBF | 0.001 | 0.386 | 0.368 | 0.565 | 0.731 |
| 150 | 15 | 0.1 | RBF | 0.01 | 0.083 | 0.092 | 0.501 | 0.475 |
| 150 | 15 | 0.2 | LIN | - | 0.277 | 0.283 | 0.538 | 0.728 |
| 150 | 15 | 0.2 | RBF | 0.0001 | 0.389 | 0.389 | 0.562 | 0.756 |
| 150 | 15 | 0.2 | RBF | 0.001 | 0.386 | 0.368 | 0.565 | 0.731 |
| 150 | 15 | 0.2 | RBF | 0.01 | 0.067 | 0.083 | 0.499 | 0.473 |
| 150 | 15 | 0.4 | LIN | - | 0.392 | 0.369 | 0.572 | 0.735 |
| 150 | 15 | 0.4 | RBF | 0.0001 | 0.389 | 0.389 | 0.562 | 0.756 |
| 150 | 15 | 0.4 | RBF | 0.001 | 0.386 | 0.368 | 0.565 | 0.731 |
| 150 | 15 | 0.4 | RBF | 0.01 | 0.060 | 0.073 | 0.496 | 0.471 |
| 150 | 15 | 0.6 | LIN | - | 0.391 | 0.372 | 0.571 | 0.732 |
| 150 | 15 | 0.6 | RBF | 0.0001 | 0.389 | 0.389 | 0.562 | 0.756 |
| 150 | 15 | 0.6 | RBF | 0.001 | 0.386 | 0.368 | 0.565 | 0.731 |

Continued on next page

TABLE S16 – continued from previous page

| n | $k$ | $\lambda$ | usim | $\sigma$ | AP@5 | AP@10 | sCI | CI |
|---|---|---|---|---|---|---|---|---|
| 150 | 15 | 0.6 | RBF | 0.01 | 0.051 | 0.064 | 0.496 | 0.470 |
| 150 | 15 | 0.8 | LIN | - | 0.392 | 0.376 | 0.571 | 0.729 |
| 150 | 15 | 0.8 | RBF | 0.0001 | 0.389 | 0.389 | 0.562 | 0.756 |
| 150 | 15 | 0.8 | RBF | 0.001 | 0.386 | 0.368 | 0.565 | 0.731 |
| 150 | 15 | 0.8 | RBF | 0.01 | 0.052 | 0.066 | 0.494 | 0.469 |
| 150 | 15 | 1.0 | LIN | - | 0.393 | 0.382 | 0.573 | 0.725 |
| 150 | 15 | 1.0 | RBF | 0.0001 | 0.389 | 0.389 | 0.562 | 0.756 |
| 150 | 15 | 1.0 | RBF | 0.001 | 0.386 | 0.368 | 0.565 | 0.731 |
| 150 | 15 | 1.0 | RBF | 0.01 | 0.041 | 0.054 | 0.494 | 0.469 |
| 150 | 15 | 10 | LIN | - | 0.391 | 0.376 | 0.569 | 0.700 |
| 150 | 15 | 10 | RBF | 0.0001 | 0.389 | 0.389 | 0.562 | 0.756 |
| 150 | 15 | 10 | RBF | 0.001 | 0.386 | 0.368 | 0.565 | 0.731 |
| 150 | 15 | 10 | RBF | 0.01 | 0.029 | 0.044 | 0.497 | 0.468 |
| 150 | 15 | 50 | LIN | - | 0.387 | 0.388 | 0.557 | 0.756 |
| 150 | 15 | 50 | RBF | 0.0001 | 0.389 | 0.389 | 0.562 | 0.756 |
| 150 | 15 | 50 | RBF | 0.001 | 0.386 | 0.368 | 0.565 | 0.731 |
| 150 | 15 | 50 | RBF | 0.01 | 0.030 | 0.044 | 0.497 | 0.467 |
| 150 | 15 | 100 | LIN | - | 0.382 | 0.384 | 0.556 | 0.761 |
| 150 | 15 | 100 | RBF | 0.0001 | 0.389 | 0.389 | 0.563 | 0.756 |
| 150 | 15 | 100 | RBF | 0.001 | 0.386 | 0.368 | 0.565 | 0.731 |
| 150 | 15 | 100 | RBF | 0.01 | 0.032 | 0.046 | 0.497 | 0.467 |
| 200 | 5 | 0.000001 | RBF | 0.0001 | 0.293 | 0.290 | 0.551 | 0.724 |
| 200 | 5 | 0.000001 | RBF | 0.001 | 0.305 | 0.315 | 0.554 | 0.698 |
| 200 | 5 | 0.000001 | RBF | 0.01 | 0.156 | 0.171 | 0.524 | 0.564 |
| 200 | 5 | 0.00001 | LIN | - | 0.144 | 0.175 | 0.531 | 0.704 |
| 200 | 5 | 0.00001 | RBF | 0.001 | 0.373 | 0.358 | 0.554 | 0.734 |
| 200 | 5 | 0.00001 | RBF | 0.01 | 0.148 | 0.172 | 0.519 | 0.566 |
| 200 | 5 | 0.0001 | RBF | 0.0001 | 0.394 | 0.387 | 0.557 | 0.752 |
| 200 | 5 | 0.0001 | RBF | 0.001 | 0.373 | 0.358 | 0.554 | 0.734 |
| 200 | 5 | 0.0001 | RBF | 0.01 | 0.141 | 0.162 | 0.522 | 0.535 |
| 200 | 5 | 0.001 | LIN | - | 0.216 | 0.235 | 0.541 | 0.710 |
| 200 | 5 | 0.001 | RBF | 0.0001 | 0.394 | 0.387 | 0.557 | 0.752 |
| 200 | 5 | 0.001 | RBF | 0.001 | 0.373 | 0.358 | 0.554 | 0.734 |
| 200 | 5 | 0.001 | RBF | 0.01 | 0.117 | 0.135 | 0.528 | 0.508 |
| 200 | 5 | 0.01 | LIN | - | 0.312 | 0.310 | 0.504 | 0.697 |
| 200 | 5 | 0.01 | RBF | 0.0001 | 0.394 | 0.387 | 0.557 | 0.752 |
| 200 | 5 | 0.01 | RBF | 0.001 | 0.373 | 0.358 | 0.554 | 0.734 |
| 200 | 5 | 0.01 | RBF | 0.01 | 0.091 | 0.108 | 0.509 | 0.486 |
| 200 | 5 | 0.1 | LIN | - | 0.391 | 0.360 | 0.553 | 0.750 |
| 200 | 5 | 0.1 | RBF | 0.0001 | 0.394 | 0.387 | 0.557 | 0.752 |
| 200 | 5 | 0.1 | RBF | 0.001 | 0.373 | 0.358 | 0.554 | 0.734 |
| 200 | 5 | 0.1 | RBF | 0.01 | 0.063 | 0.076 | 0.501 | 0.475 |
| 200 | 5 | 0.2 | LIN | - | 0.400 | 0.374 | 0.553 | 0.753 |
| 200 | 5 | 0.2 | RBF | 0.0001 | 0.394 | 0.387 | 0.557 | 0.752 |
| 200 | 5 | 0.2 | RBF | 0.001 | 0.373 | 0.358 | 0.554 | 0.734 |
| 200 | 5 | 0.2 | RBF | 0.01 | 0.057 | 0.072 | 0.500 | 0.473 |
| 200 | 5 | 0.4 | LIN | - | 0.405 | 0.379 | 0.552 | 0.759 |
| 200 | 5 | 0.4 | RBF | 0.0001 | 0.394 | 0.387 | 0.557 | 0.752 |
| 200 | 5 | 0.4 | RBF | 0.001 | 0.373 | 0.358 | 0.554 | 0.734 |
| 200 | 5 | 0.4 | RBF | 0.01 | 0.044 | 0.060 | 0.498 | 0.472 |
| 200 | 5 | 0.6 | LIN | - | 0.347 | 0.318 | 0.552 | 0.754 |
| 200 | 5 | 0.6 | RBF | 0.0001 | 0.394 | 0.387 | 0.557 | 0.752 |
| 200 | 5 | 0.6 | RBF | 0.001 | 0.373 | 0.358 | 0.554 | 0.734 |
| 200 | 5 | 0.6 | RBF | 0.01 | 0.041 | 0.056 | 0.498 | 0.471 |
| 200 | 5 | 0.8 | LIN | - | 0.432 | 0.398 | 0.551 | 0.749 |
| 200 | 5 | 0.8 | RBF | 0.0001 | 0.394 | 0.387 | 0.557 | 0.752 |
| 200 | 5 | 0.8 | RBF | 0.001 | 0.373 | 0.358 | 0.554 | 0.734 |
| 200 | 5 | 0.8 | RBF | 0.01 | 0.039 | 0.053 | 0.497 | 0.470 |

Continued on next page

TABLE S16 – continued from previous page

| n | $k$ | $\lambda$ | usim | $\sigma$ | AP@5 | AP@10 | sCI | CI |
|---|---|---|---|---|---|---|---|---|
| 200 | 5 | 1.0 | LIN | - | 0.345 | 0.332 | 0.552 | 0.760 |
| 200 | 5 | 1.0 | RBF | 0.0001 | 0.394 | 0.387 | 0.557 | 0.752 |
| 200 | 5 | 1.0 | RBF | 0.001 | 0.373 | 0.358 | 0.554 | 0.734 |
| 200 | 5 | 1.0 | RBF | 0.01 | 0.036 | 0.050 | 0.498 | 0.470 |
| 200 | 5 | 10 | LIN | - | 0.393 | 0.382 | 0.552 | 0.750 |
| 200 | 5 | 10 | RBF | 0.0001 | 0.394 | 0.387 | 0.557 | 0.752 |
| 200 | 5 | 10 | RBF | 0.001 | 0.373 | 0.358 | 0.554 | 0.734 |
| 200 | 5 | 10 | RBF | 0.01 | 0.024 | 0.039 | 0.499 | 0.468 |
| 200 | 5 | 50 | LIN | - | 0.390 | 0.374 | 0.561 | 0.690 |
| 200 | 5 | 50 | RBF | 0.0001 | 0.394 | 0.387 | 0.557 | 0.752 |
| 200 | 5 | 50 | RBF | 0.001 | 0.376 | 0.359 | 0.554 | 0.734 |
| 200 | 5 | 50 | RBF | 0.01 | 0.018 | 0.033 | 0.498 | 0.468 |
| 200 | 5 | 100 | LIN | - | 0.390 | 0.374 | 0.561 | 0.690 |
| 200 | 5 | 100 | RBF | 0.0001 | 0.394 | 0.387 | 0.557 | 0.752 |
| 200 | 5 | 100 | RBF | 0.001 | 0.376 | 0.359 | 0.554 | 0.734 |
| 200 | 5 | 100 | RBF | 0.01 | 0.017 | 0.032 | 0.498 | 0.468 |
| 200 | 10 | 0.000001 | LIN | - | 0.101 | 0.122 | 0.527 | 0.703 |
| 200 | 10 | 0.000001 | RBF | 0.01 | 0.163 | 0.173 | 0.527 | 0.560 |
| 200 | 10 | 0.001 | LIN | - | 0.182 | 0.204 | 0.544 | 0.713 |
| 200 | 10 | 0.001 | RBF | 0.0001 | 0.392 | 0.388 | 0.556 | 0.751 |
| 200 | 10 | 0.001 | RBF | 0.001 | 0.373 | 0.365 | 0.558 | 0.725 |
| 200 | 10 | 0.001 | RBF | 0.01 | 0.123 | 0.134 | 0.527 | 0.505 |
| 200 | 10 | 0.01 | LIN | - | 0.273 | 0.281 | 0.530 | 0.718 |
| 200 | 10 | 0.01 | RBF | 0.0001 | 0.392 | 0.388 | 0.556 | 0.751 |
| 200 | 10 | 0.01 | RBF | 0.001 | 0.373 | 0.365 | 0.558 | 0.725 |
| 200 | 10 | 0.01 | RBF | 0.01 | 0.094 | 0.108 | 0.509 | 0.485 |
| 200 | 10 | 0.1 | LIN | - | 0.394 | 0.375 | 0.559 | 0.745 |
| 200 | 10 | 0.1 | RBF | 0.0001 | 0.392 | 0.388 | 0.556 | 0.751 |
| 200 | 10 | 0.1 | RBF | 0.001 | 0.373 | 0.365 | 0.558 | 0.725 |
| 200 | 10 | 0.1 | RBF | 0.01 | 0.065 | 0.075 | 0.502 | 0.475 |
| 200 | 10 | 0.2 | LIN | - | 0.407 | 0.382 | 0.556 | 0.747 |
| 200 | 10 | 0.2 | RBF | 0.0001 | 0.392 | 0.388 | 0.556 | 0.751 |
| 200 | 10 | 0.2 | RBF | 0.001 | 0.373 | 0.365 | 0.558 | 0.725 |
| 200 | 10 | 0.2 | RBF | 0.01 | 0.056 | 0.071 | 0.500 | 0.473 |
| 200 | 10 | 0.4 | LIN | - | 0.342 | 0.332 | 0.554 | 0.749 |
| 200 | 10 | 0.4 | RBF | 0.0001 | 0.392 | 0.388 | 0.556 | 0.751 |
| 200 | 10 | 0.4 | RBF | 0.001 | 0.373 | 0.365 | 0.558 | 0.725 |
| 200 | 10 | 0.4 | RBF | 0.01 | 0.043 | 0.057 | 0.497 | 0.471 |
| 200 | 10 | 0.6 | LIN | - | 0.324 | 0.321 | 0.556 | 0.751 |
| 200 | 10 | 0.6 | RBF | 0.0001 | 0.392 | 0.388 | 0.556 | 0.751 |
| 200 | 10 | 0.6 | RBF | 0.001 | 0.373 | 0.365 | 0.558 | 0.725 |
| 200 | 10 | 0.6 | RBF | 0.01 | 0.040 | 0.053 | 0.498 | 0.471 |
| 200 | 10 | 0.8 | LIN | - | 0.404 | 0.373 | 0.553 | 0.751 |
| 200 | 10 | 0.8 | RBF | 0.0001 | 0.392 | 0.388 | 0.556 | 0.751 |
| 200 | 10 | 0.8 | RBF | 0.001 | 0.373 | 0.365 | 0.558 | 0.725 |
| 200 | 10 | 0.8 | RBF | 0.01 | 0.035 | 0.049 | 0.497 | 0.470 |
| 200 | 10 | 1.0 | LIN | - | 0.358 | 0.360 | 0.550 | 0.751 |
| 200 | 10 | 1.0 | RBF | 0.0001 | 0.392 | 0.388 | 0.556 | 0.751 |
| 200 | 10 | 1.0 | RBF | 0.001 | 0.373 | 0.365 | 0.558 | 0.725 |
| 200 | 10 | 1.0 | RBF | 0.01 | 0.035 | 0.050 | 0.497 | 0.470 |
| 200 | 10 | 10 | LIN | - | 0.385 | 0.381 | 0.550 | 0.756 |
| 200 | 10 | 10 | RBF | 0.0001 | 0.392 | 0.388 | 0.556 | 0.751 |
| 200 | 10 | 10 | RBF | 0.001 | 0.373 | 0.365 | 0.558 | 0.725 |
| 200 | 10 | 10 | RBF | 0.01 | 0.022 | 0.038 | 0.499 | 0.468 |
| 200 | 10 | 50 | LIN | - | 0.392 | 0.383 | 0.550 | 0.755 |
| 200 | 10 | 50 | RBF | 0.0001 | 0.392 | 0.388 | 0.556 | 0.751 |
| 200 | 10 | 50 | RBF | 0.001 | 0.373 | 0.365 | 0.558 | 0.725 |
| 200 | 10 | 50 | RBF | 0.01 | 0.025 | 0.040 | 0.498 | 0.468 |

Continued on next page

TABLE S16 – continued from previous page

| n | $k$ | $\lambda$ | usim | $\sigma$ | AP@5 | AP@10 | sCI | CI |
|---|---|---|---|---|---|---|---|---|
| 200 | 10 | 100 | LIN | - | 0.390 | 0.390 | 0.552 | 0.756 |
| 200 | 10 | 100 | RBF | 0.0001 | 0.392 | 0.388 | 0.556 | 0.751 |
| 200 | 10 | 100 | RBF | 0.001 | 0.373 | 0.365 | 0.558 | 0.725 |
| 200 | 10 | 100 | RBF | 0.01 | 0.017 | 0.032 | 0.498 | 0.468 |
| 200 | 15 | 0.001 | LIN | - | 0.186 | 0.208 | 0.521 | 0.708 |
| 200 | 15 | 0.001 | RBF | 0.0001 | 0.396 | 0.388 | 0.555 | 0.750 |
| 200 | 15 | 0.001 | RBF | 0.001 | 0.371 | 0.365 | 0.556 | 0.724 |
| 200 | 15 | 0.001 | RBF | 0.01 | 0.118 | 0.131 | 0.529 | 0.504 |
| 200 | 15 | 0.01 | LIN | - | 0.239 | 0.254 | 0.531 | 0.721 |
| 200 | 15 | 0.01 | RBF | 0.0001 | 0.396 | 0.388 | 0.555 | 0.750 |
| 200 | 15 | 0.01 | RBF | 0.001 | 0.371 | 0.365 | 0.556 | 0.724 |
| 200 | 15 | 0.01 | RBF | 0.01 | 0.093 | 0.108 | 0.507 | 0.485 |
| 200 | 15 | 0.1 | LIN | - | 0.242 | 0.234 | 0.531 | 0.721 |
| 200 | 15 | 0.1 | RBF | 0.0001 | 0.396 | 0.388 | 0.555 | 0.750 |
| 200 | 15 | 0.1 | RBF | 0.001 | 0.371 | 0.365 | 0.556 | 0.724 |
| 200 | 15 | 0.1 | RBF | 0.01 | 0.065 | 0.075 | 0.503 | 0.475 |
| 200 | 15 | 0.2 | LIN | - | 0.314 | 0.308 | 0.509 | 0.721 |
| 200 | 15 | 0.2 | RBF | 0.0001 | 0.396 | 0.388 | 0.555 | 0.750 |
| 200 | 15 | 0.2 | RBF | 0.001 | 0.371 | 0.365 | 0.556 | 0.724 |
| 200 | 15 | 0.2 | RBF | 0.01 | 0.060 | 0.073 | 0.500 | 0.473 |
| 200 | 15 | 0.4 | LIN | - | 0.312 | 0.316 | 0.541 | 0.704 |
| 200 | 15 | 0.4 | RBF | 0.0001 | 0.396 | 0.388 | 0.555 | 0.750 |
| 200 | 15 | 0.4 | RBF | 0.001 | 0.371 | 0.365 | 0.556 | 0.724 |
| 200 | 15 | 0.4 | RBF | 0.01 | 0.049 | 0.062 | 0.498 | 0.471 |
| 200 | 15 | 0.6 | LIN | - | 0.344 | 0.322 | 0.550 | 0.706 |
| 200 | 15 | 0.6 | RBF | 0.0001 | 0.396 | 0.388 | 0.555 | 0.750 |
| 200 | 15 | 0.6 | RBF | 0.001 | 0.371 | 0.365 | 0.556 | 0.724 |
| 200 | 15 | 0.6 | RBF | 0.01 | 0.041 | 0.055 | 0.498 | 0.470 |
| 200 | 15 | 0.8 | LIN | - | 0.294 | 0.297 | 0.534 | 0.692 |
| 200 | 15 | 0.8 | RBF | 0.0001 | 0.396 | 0.388 | 0.555 | 0.750 |
| 200 | 15 | 0.8 | RBF | 0.001 | 0.371 | 0.365 | 0.556 | 0.724 |
| 200 | 15 | 0.8 | RBF | 0.01 | 0.042 | 0.054 | 0.497 | 0.470 |
| 200 | 15 | 1.0 | LIN | - | 0.289 | 0.305 | 0.553 | 0.698 |
| 200 | 15 | 1.0 | RBF | 0.0001 | 0.396 | 0.388 | 0.555 | 0.750 |
| 200 | 15 | 1.0 | RBF | 0.001 | 0.371 | 0.365 | 0.556 | 0.724 |
| 200 | 15 | 1.0 | RBF | 0.01 | 0.034 | 0.049 | 0.496 | 0.470 |
| 200 | 15 | 10 | LIN | - | 0.285 | 0.304 | 0.493 | 0.677 |
| 200 | 15 | 10 | RBF | 0.0001 | 0.396 | 0.388 | 0.555 | 0.750 |
| 200 | 15 | 10 | RBF | 0.001 | 0.371 | 0.365 | 0.556 | 0.724 |
| 200 | 15 | 10 | RBF | 0.01 | 0.023 | 0.038 | 0.498 | 0.468 |
| 200 | 15 | 50 | LIN | - | 0.389 | 0.379 | 0.548 | 0.751 |
| 200 | 15 | 50 | RBF | 0.0001 | 0.396 | 0.388 | 0.555 | 0.750 |
| 200 | 15 | 50 | RBF | 0.001 | 0.371 | 0.365 | 0.556 | 0.724 |
| 200 | 15 | 50 | RBF | 0.01 | 0.025 | 0.040 | 0.498 | 0.468 |
| 200 | 15 | 100 | LIN | - | 0.392 | 0.379 | 0.549 | 0.753 |
| 200 | 15 | 100 | RBF | 0.0001 | 0.396 | 0.388 | 0.555 | 0.750 |
| 200 | 15 | 100 | RBF | 0.001 | 0.371 | 0.365 | 0.556 | 0.724 |
| 200 | 15 | 100 | RBF | 0.01 | 0.025 | 0.040 | 0.498 | 0.468 |
| 250 | 5 | 0.000001 | LIN | - | 0.165 | 0.188 | 0.541 | 0.698 |
| 250 | 5 | 0.000001 | RBF | 0.0001 | 0.281 | 0.282 | 0.554 | 0.728 |
| 250 | 5 | 0.000001 | RBF | 0.001 | 0.320 | 0.315 | 0.555 | 0.699 |
| 250 | 5 | 0.000001 | RBF | 0.01 | 0.172 | 0.190 | 0.525 | 0.563 |
| 250 | 5 | 0.00001 | RBF | 0.0001 | 0.395 | 0.373 | 0.555 | 0.766 |
| 250 | 5 | 0.00001 | RBF | 0.001 | 0.395 | 0.375 | 0.561 | 0.736 |
| 250 | 5 | 0.00001 | RBF | 0.01 | 0.161 | 0.182 | 0.518 | 0.561 |
| 250 | 5 | 0.0001 | RBF | 0.0001 | 0.396 | 0.384 | 0.557 | 0.756 |
| 250 | 5 | 0.0001 | RBF | 0.001 | 0.395 | 0.375 | 0.561 | 0.736 |
| 250 | 5 | 0.0001 | RBF | 0.01 | 0.141 | 0.159 | 0.524 | 0.531 |

Continued on next page

TABLE S16 – continued from previous page

| n | $k$ | $\lambda$ | usim | $\sigma$ | AP@5 | AP@10 | sCI | CI |
|---|---|---|---|---|---|---|---|---|
| 250 | 5 | 0.001 | LIN | - | 0.200 | 0.223 | 0.535 | 0.711 |
| 250 | 5 | 0.001 | RBF | 0.0001 | 0.396 | 0.384 | 0.557 | 0.756 |
| 250 | 5 | 0.001 | RBF | 0.001 | 0.395 | 0.375 | 0.561 | 0.736 |
| 250 | 5 | 0.001 | RBF | 0.01 | 0.123 | 0.140 | 0.520 | 0.506 |
| 250 | 5 | 0.01 | LIN | - | 0.317 | 0.325 | 0.537 | 0.703 |
| 250 | 5 | 0.01 | RBF | 0.0001 | 0.396 | 0.384 | 0.557 | 0.756 |
| 250 | 5 | 0.01 | RBF | 0.001 | 0.395 | 0.375 | 0.561 | 0.736 |
| 250 | 5 | 0.01 | RBF | 0.01 | 0.094 | 0.108 | 0.504 | 0.487 |
| 250 | 5 | 0.1 | LIN | - | 0.381 | 0.373 | 0.544 | 0.728 |
| 250 | 5 | 0.1 | RBF | 0.0001 | 0.396 | 0.384 | 0.557 | 0.756 |
| 250 | 5 | 0.1 | RBF | 0.001 | 0.395 | 0.375 | 0.561 | 0.736 |
| 250 | 5 | 0.1 | RBF | 0.01 | 0.065 | 0.074 | 0.503 | 0.476 |
| 250 | 5 | 0.2 | LIN | - | 0.381 | 0.365 | 0.558 | 0.752 |
| 250 | 5 | 0.2 | RBF | 0.0001 | 0.396 | 0.384 | 0.557 | 0.756 |
| 250 | 5 | 0.2 | RBF | 0.001 | 0.395 | 0.375 | 0.561 | 0.736 |
| 250 | 5 | 0.2 | RBF | 0.01 | 0.050 | 0.064 | 0.502 | 0.474 |
| 250 | 5 | 0.4 | LIN | - | 0.393 | 0.377 | 0.554 | 0.757 |
| 250 | 5 | 0.4 | RBF | 0.0001 | 0.396 | 0.384 | 0.557 | 0.756 |
| 250 | 5 | 0.4 | RBF | 0.001 | 0.395 | 0.375 | 0.561 | 0.736 |
| 250 | 5 | 0.4 | RBF | 0.01 | 0.041 | 0.057 | 0.500 | 0.473 |
| 250 | 5 | 0.6 | LIN | - | 0.394 | 0.384 | 0.550 | 0.761 |
| 250 | 5 | 0.6 | usim | 0.0001 | 0.396 | 0.384 | 0.557 | 0.756 |
| 250 | 5 | 0.6 | RBF | 0.001 | 0.395 | 0.375 | 0.561 | 0.736 |
| 250 | 5 | 0.6 | RBF | 0.01 | 0.043 | 0.058 | 0.500 | 0.472 |
| 250 | 5 | 0.8 | LIN | - | 0.398 | 0.374 | 0.551 | 0.759 |
| 250 | 5 | 0.8 | RBF | 0.0001 | 0.396 | 0.384 | 0.557 | 0.756 |
| 250 | 5 | 0.8 | RBF | 0.001 | 0.395 | 0.375 | 0.561 | 0.736 |
| 250 | 5 | 0.8 | RBF | 0.01 | 0.038 | 0.052 | 0.499 | 0.471 |
| 250 | 5 | 1.0 | LIN | - | 0.430 | 0.404 | 0.551 | 0.758 |
| 250 | 5 | 1.0 | RBF | 0.0001 | 0.396 | 0.384 | 0.557 | 0.756 |
| 250 | 5 | 1.0 | RBF | 0.001 | 0.395 | 0.375 | 0.561 | 0.736 |
| 250 | 5 | 1.0 | RBF | 0.01 | 0.032 | 0.047 | 0.499 | 0.471 |
| 250 | 5 | 10 | LIN | - | 0.381 | 0.374 | 0.553 | 0.752 |
| 250 | 5 | 10 | RBF | 0.0001 | 0.396 | 0.384 | 0.557 | 0.756 |
| 250 | 5 | 10 | RBF | 0.001 | 0.395 | 0.375 | 0.561 | 0.736 |
| 250 | 5 | 10 | usim | 0.01 | 0.019 | 0.035 | 0.502 | 0.469 |
| 250 | 5 | 50 | LIN | - | 0.391 | 0.383 | 0.556 | 0.699 |
| 250 | 5 | 50 | RBF | 0.0001 | 0.396 | 0.384 | 0.557 | 0.756 |
| 250 | 5 | 50 | RBF | 0.001 | 0.395 | 0.375 | 0.562 | 0.736 |
| 250 | 5 | 50 | RBF | 0.01 | 0.018 | 0.033 | 0.502 | 0.469 |
| 250 | 5 | 100 | LIN | - | 0.391 | 0.383 | 0.556 | 0.699 |
| 250 | 5 | 100 | RBF | 0.0001 | 0.396 | 0.384 | 0.557 | 0.756 |
| 250 | 5 | 100 | RBF | 0.001 | 0.395 | 0.375 | 0.561 | 0.736 |
| 250 | 5 | 100 | RBF | 0.01 | 0.016 | 0.030 | 0.502 | 0.468 |
| 250 | 10 | 0.000001 | LIN | - | 0.142 | 0.171 | 0.529 | 0.701 |
| 250 | 10 | 0.000001 | RBF | 0.01 | 0.175 | 0.186 | 0.526 | 0.560 |
| 250 | 10 | 0.001 | LIN | - | 0.277 | 0.269 | 0.533 | 0.693 |
| 250 | 10 | 0.001 | RBF | 0.0001 | 0.397 | 0.385 | 0.555 | 0.755 |
| 250 | 10 | 0.001 | RBF | 0.001 | 0.376 | 0.362 | 0.557 | 0.729 |
| 250 | 10 | 0.001 | RBF | 0.01 | 0.129 | 0.144 | 0.527 | 0.504 |
| 250 | 10 | 0.01 | LIN | - | 0.178 | 0.199 | 0.542 | 0.724 |
| 250 | 10 | 0.01 | RBF | 0.0001 | 0.397 | 0.385 | 0.555 | 0.755 |
| 250 | 10 | 0.01 | RBF | 0.001 | 0.376 | 0.362 | 0.557 | 0.729 |
| 250 | 10 | 0.01 | RBF | 0.01 | 0.092 | 0.107 | 0.506 | 0.486 |
| 250 | 10 | 0.1 | LIN | - | 0.229 | 0.260 | 0.537 | 0.730 |
| 250 | 10 | 0.1 | RBF | 0.0001 | 0.397 | 0.385 | 0.555 | 0.755 |
| 250 | 10 | 0.1 | RBF | 0.001 | 0.376 | 0.362 | 0.557 | 0.729 |
| 250 | 10 | 0.1 | RBF | 0.01 | 0.065 | 0.077 | 0.502 | 0.476 |

Continued on next page

TABLE S16 – continued from previous page

| n | $k$ | $\lambda$ | usim | $\sigma$ | AP@5 | AP@10 | sCI | CI |
|---|---|---|---|---|---|---|---|---|
| 250 | 10 | 0.2 | LIN | - | 0.420 | 0.388 | 0.558 | 0.749 |
| 250 | 10 | 0.2 | RBF | 0.0001 | 0.397 | 0.385 | 0.555 | 0.755 |
| 250 | 10 | 0.2 | RBF | 0.001 | 0.376 | 0.362 | 0.557 | 0.729 |
| 250 | 10 | 0.2 | RBF | 0.01 | 0.058 | 0.074 | 0.502 | 0.474 |
| 250 | 10 | 0.4 | LIN | - | 0.419 | 0.386 | 0.558 | 0.749 |
| 250 | 10 | 0.4 | RBF | 0.0001 | 0.397 | 0.385 | 0.555 | 0.755 |
| 250 | 10 | 0.4 | RBF | 0.001 | 0.376 | 0.362 | 0.557 | 0.729 |
| 250 | 10 | 0.4 | RBF | 0.01 | 0.044 | 0.060 | 0.500 | 0.472 |
| 250 | 10 | 0.6 | LIN | - | 0.422 | 0.387 | 0.558 | 0.750 |
| 250 | 10 | 0.6 | RBF | 0.0001 | 0.397 | 0.385 | 0.555 | 0.755 |
| 250 | 10 | 0.6 | RBF | 0.001 | 0.376 | 0.362 | 0.557 | 0.729 |
| 250 | 10 | 0.6 | RBF | 0.01 | 0.043 | 0.058 | 0.499 | 0.472 |
| 250 | 10 | 0.8 | LIN | - | 0.376 | 0.361 | 0.554 | 0.751 |
| 250 | 10 | 0.8 | RBF | 0.0001 | 0.397 | 0.385 | 0.555 | 0.755 |
| 250 | 10 | 0.8 | RBF | 0.001 | 0.376 | 0.362 | 0.557 | 0.729 |
| 250 | 10 | 0.8 | RBF | 0.01 | 0.040 | 0.054 | 0.499 | 0.471 |
| 250 | 10 | 1.0 | LIN | - | 0.384 | 0.373 | 0.555 | 0.750 |
| 250 | 10 | 1.0 | RBF | 0.0001 | 0.397 | 0.385 | 0.555 | 0.755 |
| 250 | 10 | 1.0 | RBF | 0.001 | 0.376 | 0.362 | 0.557 | 0.729 |
| 250 | 10 | 1.0 | RBF | 0.01 | 0.036 | 0.051 | 0.500 | 0.471 |
| 250 | 10 | 10 | LIN | - | 0.392 | 0.383 | 0.553 | 0.761 |
| 250 | 10 | 10 | RBF | 0.0001 | 0.397 | 0.385 | 0.555 | 0.755 |
| 250 | 10 | 10 | RBF | 0.001 | 0.376 | 0.362 | 0.557 | 0.729 |
| 250 | 10 | 10 | RBF | 0.01 | 0.022 | 0.038 | 0.501 | 0.469 |
| 250 | 10 | 50 | LIN | - | 0.392 | 0.383 | 0.551 | 0.758 |
| 250 | 10 | 50 | RBF | 0.0001 | 0.397 | 0.385 | 0.555 | 0.755 |
| 250 | 10 | 50 | RBF | 0.001 | 0.376 | 0.362 | 0.557 | 0.729 |
| 250 | 10 | 50 | RBF | 0.01 | 0.019 | 0.035 | 0.502 | 0.469 |
| 250 | 10 | 100 | LIN | - | 0.393 | 0.386 | 0.551 | 0.759 |
| 250 | 10 | 100 | RBF | 0.0001 | 0.397 | 0.385 | 0.555 | 0.755 |
| 250 | 10 | 100 | RBF | 0.001 | 0.376 | 0.362 | 0.557 | 0.729 |
| 250 | 10 | 100 | RBF | 0.01 | 0.018 | 0.034 | 0.502 | 0.468 |
| 250 | 15 | 0.001 | LIN | - | 0.236 | 0.252 | 0.533 | 0.724 |
| 250 | 15 | 0.001 | RBF | 0.0001 | 0.399 | 0.385 | 0.553 | 0.755 |
| 250 | 15 | 0.001 | RBF | 0.001 | 0.374 | 0.362 | 0.557 | 0.728 |
| 250 | 15 | 0.001 | RBF | 0.01 | 0.137 | 0.148 | 0.527 | 0.503 |
| 250 | 15 | 0.01 | LIN | - | 0.238 | 0.252 | 0.512 | 0.721 |
| 250 | 15 | 0.01 | RBF | 0.0001 | 0.399 | 0.385 | 0.553 | 0.755 |
| 250 | 15 | 0.01 | RBF | 0.001 | 0.374 | 0.362 | 0.557 | 0.728 |
| 250 | 15 | 0.01 | RBF | 0.01 | 0.099 | 0.114 | 0.509 | 0.486 |
| 250 | 15 | 0.1 | LIN | - | 0.293 | 0.294 | 0.522 | 0.726 |
| 250 | 15 | 0.1 | RBF | 0.0001 | 0.399 | 0.385 | 0.553 | 0.755 |
| 250 | 15 | 0.1 | RBF | 0.001 | 0.374 | 0.362 | 0.557 | 0.728 |
| 250 | 15 | 0.1 | RBF | 0.01 | 0.071 | 0.083 | 0.503 | 0.476 |
| 250 | 15 | 0.2 | LIN | - | 0.339 | 0.315 | 0.498 | 0.722 |
| 250 | 15 | 0.2 | RBF | 0.0001 | 0.399 | 0.385 | 0.553 | 0.755 |
| 250 | 15 | 0.2 | RBF | 0.001 | 0.374 | 0.362 | 0.557 | 0.728 |
| 250 | 15 | 0.2 | RBF | 0.01 | 0.060 | 0.075 | 0.503 | 0.474 |
| 250 | 15 | 0.4 | LIN | - | 0.354 | 0.357 | 0.510 | 0.711 |
| 250 | 15 | 0.4 | RBF | 0.0001 | 0.399 | 0.385 | 0.553 | 0.755 |
| 250 | 15 | 0.4 | RBF | 0.001 | 0.374 | 0.362 | 0.557 | 0.728 |
| 250 | 15 | 0.4 | RBF | 0.01 | 0.046 | 0.061 | 0.499 | 0.472 |
| 250 | 15 | 0.6 | LIN | - | 0.390 | 0.383 | 0.558 | 0.732 |
| 250 | 15 | 0.6 | RBF | 0.0001 | 0.399 | 0.385 | 0.553 | 0.755 |
| 250 | 15 | 0.6 | RBF | 0.001 | 0.374 | 0.362 | 0.557 | 0.728 |
| 250 | 15 | 0.6 | RBF | 0.01 | 0.044 | 0.059 | 0.500 | 0.472 |
| 250 | 15 | 0.8 | LIN | - | 0.390 | 0.380 | 0.558 | 0.729 |
| 250 | 15 | 0.8 | RBF | 0.0001 | 0.399 | 0.385 | 0.553 | 0.755 |

Continued on next page

TABLE S16 – continued from previous page

| n | $k$ | $\lambda$ | usim | $\sigma$ | AP@5 | AP@10 | sCI | CI |
|---|---|---|---|---|---|---|---|---|
| 250 | 15 | 0.8 | RBF | 0.001 | 0.374 | 0.362 | 0.557 | 0.728 |
| 250 | 15 | 0.8 | RBF | 0.01 | 0.041 | 0.054 | 0.501 | 0.471 |
| 250 | 15 | 1.0 | LIN | - | 0.385 | 0.371 | 0.559 | 0.726 |
| 250 | 15 | 1.0 | RBF | 0.0001 | 0.399 | 0.385 | 0.553 | 0.755 |
| 250 | 15 | 1.0 | RBF | 0.001 | 0.374 | 0.362 | 0.557 | 0.728 |
| 250 | 15 | 1.0 | RBF | 0.01 | 0.037 | 0.051 | 0.500 | 0.471 |
| 250 | 15 | 10 | LIN | - | 0.374 | 0.354 | 0.554 | 0.747 |
| 250 | 15 | 10 | RBF | 0.0001 | 0.399 | 0.385 | 0.553 | 0.755 |
| 250 | 15 | 10 | RBF | 0.001 | 0.374 | 0.362 | 0.557 | 0.728 |
| 250 | 15 | 10 | RBF | 0.01 | 0.024 | 0.039 | 0.502 | 0.469 |
| 250 | 15 | 50 | LIN | - | 0.392 | 0.385 | 0.551 | 0.757 |
| 250 | 15 | 50 | RBF | 0.0001 | 0.399 | 0.385 | 0.553 | 0.755 |
| 250 | 15 | 50 | RBF | 0.001 | 0.374 | 0.362 | 0.557 | 0.728 |
| 250 | 15 | 50 | RBF | 0.01 | 0.019 | 0.035 | 0.501 | 0.469 |
| 250 | 15 | 100 | LIN | - | 0.393 | 0.386 | 0.551 | 0.757 |
| 250 | 15 | 100 | RBF | 0.0001 | 0.399 | 0.385 | 0.553 | 0.755 |
| 250 | 15 | 100 | RBF | 0.001 | 0.374 | 0.362 | 0.557 | 0.728 |
| 250 | 15 | 100 | RBF | 0.01 | 0.019 | 0.035 | 0.501 | 0.468 |
| 300 | 5 | 0.000001 | RBF | 0.0001 | 0.306 | 0.313 | 0.550 | 0.735 |
| 300 | 5 | 0.000001 | RBF | 0.001 | 0.320 | 0.322 | 0.551 | 0.692 |
| 300 | 5 | 0.000001 | RBF | 0.01 | 0.179 | 0.190 | 0.525 | 0.553 |
| 300 | 5 | 0.00001 | RBF | 0.0001 | 0.365 | 0.351 | 0.552 | 0.753 |
| 300 | 5 | 0.00001 | RBF | 0.001 | 0.357 | 0.353 | 0.552 | 0.729 |
| 300 | 5 | 0.00001 | RBF | 0.01 | 0.168 | 0.185 | 0.528 | 0.550 |
| 300 | 5 | 0.0001 | RBF | 0.0001 | 0.384 | 0.375 | 0.557 | 0.752 |
| 300 | 5 | 0.0001 | RBF | 0.001 | 0.357 | 0.353 | 0.552 | 0.729 |
| 300 | 5 | 0.0001 | RBF | 0.01 | 0.147 | 0.162 | 0.530 | 0.524 |
| 300 | 5 | 0.001 | LIN | - | 0.222 | 0.231 | 0.537 | 0.702 |
| 300 | 5 | 0.001 | RBF | 0.0001 | 0.384 | 0.375 | 0.557 | 0.752 |
| 300 | 5 | 0.001 | RBF | 0.001 | 0.357 | 0.353 | 0.552 | 0.729 |
| 300 | 5 | 0.001 | RBF | 0.01 | 0.126 | 0.139 | 0.526 | 0.502 |
| 300 | 5 | 0.01 | LIN | - | 0.243 | 0.253 | 0.520 | 0.674 |
| 300 | 5 | 0.01 | RBF | 0.0001 | 0.384 | 0.375 | 0.557 | 0.752 |
| 300 | 5 | 0.01 | RBF | 0.001 | 0.357 | 0.353 | 0.552 | 0.729 |
| 300 | 5 | 0.01 | RBF | 0.01 | 0.100 | 0.108 | 0.511 | 0.486 |
| 300 | 5 | 0.1 | LIN | - | 0.296 | 0.299 | 0.552 | 0.747 |
| 300 | 5 | 0.1 | RBF | 0.0001 | 0.384 | 0.375 | 0.557 | 0.752 |
| 300 | 5 | 0.1 | RBF | 0.001 | 0.357 | 0.353 | 0.552 | 0.729 |
| 300 | 5 | 0.1 | RBF | 0.01 | 0.067 | 0.081 | 0.507 | 0.476 |
| 300 | 5 | 0.2 | LIN | - | 0.364 | 0.360 | 0.549 | 0.750 |
| 300 | 5 | 0.2 | RBF | 0.0001 | 0.384 | 0.375 | 0.557 | 0.752 |
| 300 | 5 | 0.2 | RBF | 0.001 | 0.357 | 0.353 | 0.552 | 0.729 |
| 300 | 5 | 0.2 | RBF | 0.01 | 0.061 | 0.073 | 0.505 | 0.474 |
| 300 | 5 | 0.4 | LIN | - | 0.365 | 0.341 | 0.552 | 0.755 |
| 300 | 5 | 0.4 | RBF | 0.0001 | 0.384 | 0.375 | 0.557 | 0.752 |
| 300 | 5 | 0.4 | RBF | 0.001 | 0.357 | 0.353 | 0.552 | 0.729 |
| 300 | 5 | 0.4 | RBF | 0.01 | 0.049 | 0.063 | 0.505 | 0.472 |
| 300 | 5 | 0.6 | LIN | - | 0.336 | 0.329 | 0.551 | 0.760 |
| 300 | 5 | 0.6 | RBF | 0.0001 | 0.384 | 0.375 | 0.557 | 0.752 |
| 300 | 5 | 0.6 | RBF | 0.001 | 0.357 | 0.353 | 0.552 | 0.729 |
| 300 | 5 | 0.6 | RBF | 0.01 | 0.041 | 0.056 | 0.504 | 0.471 |
| 300 | 5 | 0.8 | LIN | - | 0.381 | 0.373 | 0.553 | 0.759 |
| 300 | 5 | 0.8 | RBF | 0.0001 | 0.384 | 0.375 | 0.557 | 0.752 |
| 300 | 5 | 0.8 | RBF | 0.001 | 0.357 | 0.353 | 0.552 | 0.729 |
| 300 | 5 | 0.8 | RBF | 0.01 | 0.042 | 0.056 | 0.504 | 0.471 |
| 300 | 5 | 1.0 | LIN | - | 0.354 | 0.346 | 0.552 | 0.761 |
| 300 | 5 | 1.0 | RBF | 0.0001 | 0.384 | 0.375 | 0.557 | 0.752 |
| 300 | 5 | 1.0 | RBF | 0.001 | 0.357 | 0.353 | 0.552 | 0.729 |

Continued on next page

TABLE S16 – continued from previous page

| n | $k$ | $\lambda$ | usim | $\sigma$ | AP@5 | AP@10 | sCI | CI |
|---|---|---|---|---|---|---|---|---|
| 300 | 5 | 1.0 | RBF | 0.01 | 0.036 | 0.049 | 0.505 | 0.470 |
| 300 | 5 | 10 | LIN | - | 0.366 | 0.349 | 0.552 | 0.750 |
| 300 | 5 | 10 | RBF | 0.0001 | 0.384 | 0.375 | 0.557 | 0.752 |
| 300 | 5 | 10 | RBF | 0.001 | 0.357 | 0.353 | 0.552 | 0.729 |
| 300 | 5 | 10 | RBF | 0.01 | 0.020 | 0.036 | 0.505 | 0.469 |
| 300 | 5 | 50 | LIN | - | 0.376 | 0.368 | 0.558 | 0.701 |
| 300 | 5 | 50 | RBF | 0.0001 | 0.384 | 0.375 | 0.557 | 0.752 |
| 300 | 5 | 50 | RBF | 0.001 | 0.357 | 0.353 | 0.552 | 0.729 |
| 300 | 5 | 50 | RBF | 0.01 | 0.018 | 0.034 | 0.505 | 0.468 |
| 300 | 5 | 100 | LIN | - | 0.376 | 0.368 | 0.558 | 0.701 |
| 300 | 5 | 100 | RBF | 0.0001 | 0.384 | 0.375 | 0.557 | 0.752 |
| 300 | 5 | 100 | RBF | 0.001 | 0.357 | 0.353 | 0.552 | 0.729 |
| 300 | 5 | 100 | RBF | 0.01 | 0.016 | 0.032 | 0.505 | 0.468 |
| 300 | 10 | 0.000001 | LIN | - | 0.129 | 0.157 | 0.534 | 0.710 |
| 300 | 10 | 0.000001 | RBF | 0.01 | 0.180 | 0.185 | 0.524 | 0.548 |
| 300 | 10 | 0.001 | LIN | - | 0.170 | 0.195 | 0.511 | 0.711 |
| 300 | 10 | 0.001 | RBF | 0.0001 | 0.387 | 0.371 | 0.556 | 0.750 |
| 300 | 10 | 0.001 | RBF | 0.001 | 0.360 | 0.354 | 0.554 | 0.722 |
| 300 | 10 | 0.001 | RBF | 0.01 | 0.129 | 0.141 | 0.525 | 0.500 |
| 300 | 10 | 0.01 | LIN | - | 0.255 | 0.264 | 0.509 | 0.660 |
| 300 | 10 | 0.01 | RBF | 0.0001 | 0.387 | 0.371 | 0.556 | 0.750 |
| 300 | 10 | 0.01 | RBF | 0.001 | 0.360 | 0.354 | 0.554 | 0.722 |
| 300 | 10 | 0.01 | RBF | 0.01 | 0.107 | 0.116 | 0.511 | 0.485 |
| 300 | 10 | 0.1 | LIN | - | 0.373 | 0.352 | 0.554 | 0.740 |
| 300 | 10 | 0.1 | RBF | 0.0001 | 0.387 | 0.371 | 0.556 | 0.750 |
| 300 | 10 | 0.1 | RBF | 0.001 | 0.360 | 0.354 | 0.554 | 0.722 |
| 300 | 10 | 0.1 | RBF | 0.01 | 0.073 | 0.086 | 0.508 | 0.476 |
| 300 | 10 | 0.2 | LIN | - | 0.381 | 0.378 | 0.553 | 0.744 |
| 300 | 10 | 0.2 | RBF | 0.0001 | 0.387 | 0.371 | 0.556 | 0.750 |
| 300 | 10 | 0.2 | RBF | 0.001 | 0.360 | 0.354 | 0.554 | 0.722 |
| 300 | 10 | 0.2 | RBF | 0.01 | 0.064 | 0.077 | 0.506 | 0.474 |
| 300 | 10 | 0.4 | LIN | - | 0.363 | 0.360 | 0.556 | 0.748 |
| 300 | 10 | 0.4 | RBF | 0.0001 | 0.387 | 0.371 | 0.556 | 0.750 |
| 300 | 10 | 0.4 | RBF | 0.001 | 0.360 | 0.354 | 0.554 | 0.722 |
| 300 | 10 | 0.4 | RBF | 0.01 | 0.047 | 0.062 | 0.504 | 0.472 |
| 300 | 10 | 0.6 | LIN | - | 0.368 | 0.358 | 0.554 | 0.750 |
| 300 | 10 | 0.6 | RBF | 0.0001 | 0.387 | 0.371 | 0.556 | 0.750 |
| 300 | 10 | 0.6 | RBF | 0.001 | 0.360 | 0.354 | 0.554 | 0.722 |
| 300 | 10 | 0.6 | RBF | 0.01 | 0.044 | 0.059 | 0.504 | 0.471 |
| 300 | 10 | 0.8 | LIN | - | 0.370 | 0.370 | 0.552 | 0.749 |
| 300 | 10 | 0.8 | RBF | 0.0001 | 0.387 | 0.371 | 0.556 | 0.750 |
| 300 | 10 | 0.8 | RBF | 0.001 | 0.360 | 0.354 | 0.554 | 0.722 |
| 300 | 10 | 0.8 | RBF | 0.01 | 0.043 | 0.057 | 0.504 | 0.471 |
| 300 | 10 | 1.0 | LIN | - | 0.378 | 0.373 | 0.552 | 0.749 |
| 300 | 10 | 1.0 | RBF | 0.0001 | 0.387 | 0.371 | 0.556 | 0.750 |
| 300 | 10 | 1.0 | RBF | 0.001 | 0.360 | 0.354 | 0.554 | 0.722 |
| 300 | 10 | 1.0 | RBF | 0.01 | 0.036 | 0.050 | 0.504 | 0.470 |
| 300 | 10 | 10 | LIN | - | 0.374 | 0.362 | 0.550 | 0.756 |
| 300 | 10 | 10 | RBF | 0.0001 | 0.387 | 0.371 | 0.556 | 0.750 |
| 300 | 10 | 10 | RBF | 0.001 | 0.360 | 0.354 | 0.554 | 0.722 |
| 300 | 10 | 10 | RBF | 0.01 | 0.022 | 0.038 | 0.506 | 0.469 |
| 300 | 10 | 50 | LIN | - | 0.385 | 0.375 | 0.551 | 0.756 |
| 300 | 10 | 50 | RBF | 0.0001 | 0.387 | 0.371 | 0.556 | 0.750 |
| 300 | 10 | 50 | RBF | 0.001 | 0.360 | 0.354 | 0.554 | 0.722 |
| 300 | 10 | 50 | RBF | 0.01 | 0.020 | 0.036 | 0.505 | 0.468 |
| 300 | 10 | 100 | LIN | - | 0.385 | 0.376 | 0.552 | 0.755 |
| 300 | 10 | 100 | RBF | 0.0001 | 0.387 | 0.371 | 0.556 | 0.750 |
| 300 | 10 | 100 | RBF | 0.001 | 0.360 | 0.354 | 0.555 | 0.722 |

Continued on next page

TABLE S16 – continued from previous page

| n | $k$ | $\lambda$ | usim | $\sigma$ | AP@5 | AP@10 | sCI | CI |
|---|---|---|---|---|---|---|---|---|
| 300 | 10 | 100 | RBF | 0.01 | 0.016 | 0.032 | 0.505 | 0.468 |
| 300 | 15 | 0.001 | LIN | - | 0.206 | 0.227 | 0.535 | 0.712 |
| 300 | 15 | 0.001 | RBF | 0.0001 | 0.388 | 0.379 | 0.555 | 0.750 |
| 300 | 15 | 0.001 | RBF | 0.001 | 0.359 | 0.352 | 0.552 | 0.721 |
| 300 | 15 | 0.001 | RBF | 0.01 | 0.127 | 0.138 | 0.528 | 0.499 |
| 300 | 15 | 0.01 | LIN | - | 0.276 | 0.281 | 0.547 | 0.724 |
| 300 | 15 | 0.01 | RBF | 0.0001 | 0.388 | 0.379 | 0.555 | 0.750 |
| 300 | 15 | 0.01 | RBF | 0.001 | 0.359 | 0.352 | 0.552 | 0.721 |
| 300 | 15 | 0.01 | RBF | 0.01 | 0.099 | 0.111 | 0.511 | 0.484 |
| 300 | 15 | 0.1 | LIN | - | 0.382 | 0.372 | 0.556 | 0.737 |
| 300 | 15 | 0.1 | RBF | 0.0001 | 0.388 | 0.379 | 0.555 | 0.750 |
| 300 | 15 | 0.1 | RBF | 0.001 | 0.359 | 0.352 | 0.552 | 0.721 |
| 300 | 15 | 0.1 | RBF | 0.01 | 0.074 | 0.086 | 0.510 | 0.476 |
| 300 | 15 | 0.2 | LIN | - | 0.378 | 0.358 | 0.552 | 0.734 |
| 300 | 15 | 0.2 | RBF | 0.0001 | 0.388 | 0.379 | 0.555 | 0.750 |
| 300 | 15 | 0.2 | RBF | 0.001 | 0.359 | 0.352 | 0.552 | 0.721 |
| 300 | 15 | 0.2 | RBF | 0.01 | 0.066 | 0.078 | 0.507 | 0.474 |
| 300 | 15 | 0.4 | LIN | - | 0.366 | 0.358 | 0.558 | 0.729 |
| 300 | 15 | 0.4 | RBF | 0.0001 | 0.388 | 0.379 | 0.555 | 0.750 |
| 300 | 15 | 0.4 | RBF | 0.001 | 0.359 | 0.352 | 0.552 | 0.721 |
| 300 | 15 | 0.4 | RBF | 0.01 | 0.053 | 0.068 | 0.505 | 0.472 |
| 300 | 15 | 0.6 | LIN | - | 0.367 | 0.367 | 0.559 | 0.726 |
| 300 | 15 | 0.6 | RBF | 0.0001 | 0.388 | 0.379 | 0.555 | 0.750 |
| 300 | 15 | 0.6 | RBF | 0.001 | 0.359 | 0.352 | 0.552 | 0.721 |
| 300 | 15 | 0.6 | RBF | 0.01 | 0.043 | 0.058 | 0.504 | 0.471 |
| 300 | 15 | 0.8 | LIN | - | 0.365 | 0.356 | 0.559 | 0.723 |
| 300 | 15 | 0.8 | RBF | 0.0001 | 0.388 | 0.379 | 0.555 | 0.750 |
| 300 | 15 | 0.8 | RBF | 0.001 | 0.359 | 0.352 | 0.552 | 0.721 |
| 300 | 15 | 0.8 | RBF | 0.01 | 0.037 | 0.052 | 0.504 | 0.471 |
| 300 | 15 | 1.0 | LIN | - | 0.382 | 0.365 | 0.559 | 0.721 |
| 300 | 15 | 1.0 | RBF | 0.0001 | 0.388 | 0.379 | 0.555 | 0.750 |
| 300 | 15 | 1.0 | RBF | 0.001 | 0.359 | 0.352 | 0.552 | 0.721 |
| 300 | 15 | 1.0 | RBF | 0.01 | 0.037 | 0.052 | 0.505 | 0.470 |
| 300 | 15 | 10 | LIN | - | 0.385 | 0.370 | 0.557 | 0.704 |
| 300 | 15 | 10 | RBF | 0.0001 | 0.388 | 0.379 | 0.555 | 0.750 |
| 300 | 15 | 10 | RBF | 0.001 | 0.359 | 0.352 | 0.552 | 0.721 |
| 300 | 15 | 10 | RBF | 0.01 | 0.022 | 0.038 | 0.506 | 0.469 |
| 300 | 15 | 50 | LIN | - | 0.381 | 0.371 | 0.547 | 0.751 |
| 300 | 15 | 50 | RBF | 0.0001 | 0.388 | 0.379 | 0.555 | 0.750 |
| 300 | 15 | 50 | RBF | 0.001 | 0.359 | 0.353 | 0.552 | 0.721 |
| 300 | 15 | 50 | RBF | 0.01 | 0.020 | 0.036 | 0.505 | 0.468 |
| 300 | 15 | 100 | LIN | - | 0.381 | 0.370 | 0.550 | 0.752 |
| 300 | 15 | 100 | RBF | 0.0001 | 0.388 | 0.379 | 0.555 | 0.750 |
| 300 | 15 | 100 | RBF | 0.001 | 0.358 | 0.352 | 0.552 | 0.721 |
| 300 | 15 | 100 | RBF | 0.01 | 0.021 | 0.036 | 0.505 | 0.468 |
| 350 | 5 | 0.000001 | LIN | - | 0.134 | 0.155 | 0.548 | 0.712 |
| 350 | 5 | 0.000001 | RBF | 0.0001 | 0.306 | 0.310 | 0.556 | 0.737 |
| 350 | 5 | 0.000001 | RBF | 0.001 | 0.311 | 0.310 | 0.554 | 0.694 |
| 350 | 5 | 0.000001 | RBF | 0.01 | 0.181 | 0.190 | 0.525 | 0.549 |
| 350 | 5 | 0.00001 | LIN | - | 0.209 | 0.221 | 0.532 | 0.720 |
| 350 | 5 | 0.00001 | RBF | 0.0001 | 0.358 | 0.348 | 0.555 | 0.757 |
| 350 | 5 | 0.00001 | RBF | 0.001 | 0.348 | 0.341 | 0.555 | 0.728 |
| 350 | 5 | 0.00001 | RBF | 0.01 | 0.167 | 0.180 | 0.524 | 0.547 |
| 350 | 5 | 0.0001 | RBF | 0.0001 | 0.373 | 0.365 | 0.555 | 0.748 |
| 350 | 5 | 0.0001 | RBF | 0.001 | 0.348 | 0.341 | 0.555 | 0.728 |
| 350 | 5 | 0.0001 | RBF | 0.01 | 0.146 | 0.156 | 0.525 | 0.522 |
| 350 | 5 | 0.001 | LIN | - | 0.188 | 0.210 | 0.533 | 0.713 |
| 350 | 5 | 0.001 | RBF | 0.0001 | 0.373 | 0.365 | 0.555 | 0.748 |

Continued on next page

TABLE S16 – continued from previous page

| n | $k$ | $\lambda$ | usim | $\sigma$ | AP@5 | AP@10 | sCI | CI |
|---|---|---|---|---|---|---|---|---|
| 350 | 5 | 0.001 | RBF | 0.001 | 0.348 | 0.341 | 0.555 | 0.728 |
| 350 | 5 | 0.001 | RBF | 0.01 | 0.127 | 0.139 | 0.519 | 0.502 |
| 350 | 5 | 0.01 | LIN | - | 0.281 | 0.286 | 0.554 | 0.741 |
| 350 | 5 | 0.01 | RBF | 0.0001 | 0.373 | 0.365 | 0.555 | 0.748 |
| 350 | 5 | 0.01 | RBF | 0.001 | 0.348 | 0.341 | 0.555 | 0.728 |
| 350 | 5 | 0.01 | RBF | 0.01 | 0.097 | 0.109 | 0.508 | 0.486 |
| 350 | 5 | 0.1 | LIN | - | 0.287 | 0.290 | 0.543 | 0.726 |
| 350 | 5 | 0.1 | RBF | 0.0001 | 0.373 | 0.365 | 0.555 | 0.748 |
| 350 | 5 | 0.1 | RBF | 0.001 | 0.348 | 0.341 | 0.555 | 0.728 |
| 350 | 5 | 0.1 | RBF | 0.01 | 0.071 | 0.081 | 0.504 | 0.476 |
| 350 | 5 | 0.2 | LIN | - | 0.377 | 0.352 | 0.553 | 0.747 |
| 350 | 5 | 0.2 | RBF | 0.0001 | 0.373 | 0.365 | 0.555 | 0.748 |
| 350 | 5 | 0.2 | RBF | 0.001 | 0.348 | 0.341 | 0.555 | 0.728 |
| 350 | 5 | 0.2 | RBF | 0.01 | 0.063 | 0.076 | 0.503 | 0.474 |
| 350 | 5 | 0.4 | LIN | - | 0.368 | 0.355 | 0.552 | 0.750 |
| 350 | 5 | 0.4 | RBF | 0.0001 | 0.373 | 0.365 | 0.555 | 0.748 |
| 350 | 5 | 0.4 | RBF | 0.001 | 0.348 | 0.341 | 0.555 | 0.728 |
| 350 | 5 | 0.4 | RBF | 0.01 | 0.055 | 0.068 | 0.501 | 0.472 |
| 350 | 5 | 0.6 | LIN | - | 0.356 | 0.340 | 0.555 | 0.743 |
| 350 | 5 | 0.6 | RBF | 0.0001 | 0.373 | 0.365 | 0.555 | 0.748 |
| 350 | 5 | 0.6 | RBF | 0.001 | 0.348 | 0.341 | 0.555 | 0.728 |
| 350 | 5 | 0.6 | RBF | 0.01 | 0.046 | 0.061 | 0.502 | 0.472 |
| 350 | 5 | 0.8 | LIN | - | 0.367 | 0.343 | 0.550 | 0.749 |
| 350 | 5 | 0.8 | RBF | 0.0001 | 0.373 | 0.365 | 0.555 | 0.748 |
| 350 | 5 | 0.8 | RBF | 0.001 | 0.348 | 0.341 | 0.555 | 0.728 |
| 350 | 5 | 0.8 | RBF | 0.01 | 0.043 | 0.057 | 0.502 | 0.471 |
| 350 | 5 | 1.0 | LIN | - | 0.374 | 0.354 | 0.551 | 0.756 |
| 350 | 5 | 1.0 | RBF | 0.0001 | 0.373 | 0.365 | 0.555 | 0.748 |
| 350 | 5 | 1.0 | RBF | 0.001 | 0.348 | 0.341 | 0.555 | 0.728 |
| 350 | 5 | 1.0 | RBF | 0.01 | 0.039 | 0.053 | 0.500 | 0.471 |
| 350 | 5 | 10 | LIN | - | 0.362 | 0.354 | 0.553 | 0.738 |
| 350 | 5 | 10 | RBF | 0.0001 | 0.373 | 0.365 | 0.555 | 0.748 |
| 350 | 5 | 10 | RBF | 0.001 | 0.348 | 0.341 | 0.555 | 0.728 |
| 350 | 5 | 10 | RBF | 0.01 | 0.026 | 0.042 | 0.501 | 0.469 |
| 350 | 5 | 50 | LIN | - | 0.369 | 0.364 | 0.559 | 0.697 |
| 350 | 5 | 50 | RBF | 0.0001 | 0.373 | 0.365 | 0.555 | 0.748 |
| 350 | 5 | 50 | RBF | 0.001 | 0.348 | 0.340 | 0.555 | 0.728 |
| 350 | 5 | 50 | RBF | 0.01 | 0.021 | 0.037 | 0.501 | 0.469 |
| 350 | 5 | 100 | LIN | - | 0.369 | 0.364 | 0.559 | 0.697 |
| 350 | 5 | 100 | RBF | 0.0001 | 0.373 | 0.365 | 0.555 | 0.748 |
| 350 | 5 | 100 | RBF | 0.001 | 0.348 | 0.340 | 0.555 | 0.728 |
| 350 | 5 | 100 | RBF | 0.01 | 0.019 | 0.035 | 0.501 | 0.469 |
| 350 | 10 | 0.000001 | LIN | - | 0.206 | 0.219 | 0.546 | 0.714 |
| 350 | 10 | 0.000001 | RBF | 0.01 | 0.186 | 0.191 | 0.527 | 0.546 |
| 350 | 10 | 0.001 | LIN | - | 0.193 | 0.214 | 0.531 | 0.704 |
| 350 | 10 | 0.001 | RBF | 0.0001 | 0.380 | 0.367 | 0.553 | 0.748 |
| 350 | 10 | 0.001 | RBF | 0.001 | 0.351 | 0.344 | 0.556 | 0.721 |
| 350 | 10 | 0.001 | RBF | 0.01 | 0.132 | 0.143 | 0.519 | 0.499 |
| 350 | 10 | 0.01 | LIN | - | 0.262 | 0.266 | 0.547 | 0.720 |
| 350 | 10 | 0.01 | RBF | 0.0001 | 0.380 | 0.367 | 0.553 | 0.748 |
| 350 | 10 | 0.01 | RBF | 0.001 | 0.351 | 0.344 | 0.556 | 0.721 |
| 350 | 10 | 0.01 | RBF | 0.01 | 0.102 | 0.113 | 0.507 | 0.486 |
| 350 | 10 | 0.1 | LIN | - | 0.276 | 0.285 | 0.551 | 0.711 |
| 350 | 10 | 0.1 | RBF | 0.0001 | 0.380 | 0.367 | 0.553 | 0.748 |
| 350 | 10 | 0.1 | RBF | 0.001 | 0.351 | 0.344 | 0.556 | 0.721 |
| 350 | 10 | 0.1 | RBF | 0.01 | 0.074 | 0.084 | 0.503 | 0.476 |
| 350 | 10 | 0.2 | LIN | - | 0.396 | 0.368 | 0.560 | 0.742 |
| 350 | 10 | 0.2 | RBF | 0.0001 | 0.380 | 0.367 | 0.553 | 0.748 |

Continued on next page

TABLE S16 – continued from previous page

| n | $k$ | $\lambda$ | usim | $\sigma$ | AP@5 | AP@10 | sCI | CI |
|---|---|---|---|---|---|---|---|---|
| 350 | 10 | 0.2 | RBF | 0.001 | 0.351 | 0.344 | 0.556 | 0.721 |
| 350 | 10 | 0.2 | RBF | 0.01 | 0.070 | 0.083 | 0.502 | 0.474 |
| 350 | 10 | 0.4 | LIN | - | 0.397 | 0.377 | 0.554 | 0.743 |
| 350 | 10 | 0.4 | RBF | 0.0001 | 0.380 | 0.367 | 0.553 | 0.748 |
| 350 | 10 | 0.4 | RBF | 0.001 | 0.351 | 0.344 | 0.556 | 0.721 |
| 350 | 10 | 0.4 | RBF | 0.01 | 0.053 | 0.068 | 0.502 | 0.472 |
| 350 | 10 | 0.6 | LIN | - | 0.369 | 0.358 | 0.556 | 0.743 |
| 350 | 10 | 0.6 | RBF | 0.0001 | 0.380 | 0.367 | 0.553 | 0.748 |
| 350 | 10 | 0.6 | RBF | 0.001 | 0.351 | 0.344 | 0.556 | 0.721 |
| 350 | 10 | 0.6 | RBF | 0.01 | 0.049 | 0.063 | 0.500 | 0.472 |
| 350 | 10 | 0.8 | LIN | - | 0.386 | 0.352 | 0.555 | 0.745 |
| 350 | 10 | 0.8 | RBF | 0.0001 | 0.380 | 0.367 | 0.553 | 0.748 |
| 350 | 10 | 0.8 | RBF | 0.001 | 0.351 | 0.344 | 0.556 | 0.721 |
| 350 | 10 | 0.8 | RBF | 0.01 | 0.040 | 0.053 | 0.501 | 0.471 |
| 350 | 10 | 1.0 | LIN | - | 0.393 | 0.365 | 0.552 | 0.743 |
| 350 | 10 | 1.0 | RBF | 0.0001 | 0.380 | 0.367 | 0.553 | 0.748 |
| 350 | 10 | 1.0 | RBF | 0.001 | 0.351 | 0.344 | 0.556 | 0.721 |
| 350 | 10 | 1.0 | RBF | 0.01 | 0.038 | 0.053 | 0.501 | 0.471 |
| 350 | 10 | 10 | LIN | - | 0.349 | 0.349 | 0.547 | 0.757 |
| 350 | 10 | 10 | RBF | 0.0001 | 0.380 | 0.367 | 0.553 | 0.748 |
| 350 | 10 | 10 | RBF | 0.001 | 0.351 | 0.344 | 0.556 | 0.721 |
| 350 | 10 | 10 | RBF | 0.01 | 0.026 | 0.042 | 0.501 | 0.469 |
| 350 | 10 | 50 | LIN | - | 0.374 | 0.371 | 0.547 | 0.754 |
| 350 | 10 | 50 | RBF | 0.0001 | 0.380 | 0.367 | 0.553 | 0.748 |
| 350 | 10 | 50 | RBF | 0.001 | 0.351 | 0.345 | 0.556 | 0.721 |
| 350 | 10 | 50 | RBF | 0.01 | 0.021 | 0.037 | 0.501 | 0.469 |
| 350 | 10 | 100 | LIN | - | 0.382 | 0.376 | 0.548 | 0.752 |
| 350 | 10 | 100 | RBF | 0.0001 | 0.380 | 0.367 | 0.553 | 0.748 |
| 350 | 10 | 100 | RBF | 0.001 | 0.351 | 0.345 | 0.556 | 0.721 |
| 350 | 10 | 100 | RBF | 0.01 | 0.022 | 0.038 | 0.502 | 0.469 |
| 350 | 15 | 0.001 | LIN | - | 0.180 | 0.201 | 0.524 | 0.712 |
| 350 | 15 | 0.001 | RBF | 0.0001 | 0.381 | 0.370 | 0.550 | 0.747 |
| 350 | 15 | 0.001 | RBF | 0.001 | 0.353 | 0.348 | 0.555 | 0.721 |
| 350 | 15 | 0.001 | RBF | 0.01 | 0.125 | 0.137 | 0.518 | 0.499 |
| 350 | 15 | 0.01 | LIN | - | 0.179 | 0.190 | 0.515 | 0.707 |
| 350 | 15 | 0.01 | RBF | 0.0001 | 0.381 | 0.370 | 0.550 | 0.747 |
| 350 | 15 | 0.01 | RBF | 0.001 | 0.353 | 0.348 | 0.555 | 0.721 |
| 350 | 15 | 0.01 | RBF | 0.01 | 0.096 | 0.110 | 0.509 | 0.485 |
| 350 | 15 | 0.1 | LIN | - | 0.301 | 0.303 | 0.530 | 0.719 |
| 350 | 15 | 0.1 | RBF | 0.0001 | 0.381 | 0.370 | 0.550 | 0.747 |
| 350 | 15 | 0.1 | RBF | 0.001 | 0.353 | 0.348 | 0.555 | 0.721 |
| 350 | 15 | 0.1 | RBF | 0.01 | 0.073 | 0.084 | 0.504 | 0.476 |
| 350 | 15 | 0.2 | LIN | - | 0.143 | 0.173 | 0.526 | 0.712 |
| 350 | 15 | 0.2 | RBF | 0.0001 | 0.381 | 0.370 | 0.550 | 0.747 |
| 350 | 15 | 0.2 | RBF | 0.001 | 0.353 | 0.348 | 0.555 | 0.721 |
| 350 | 15 | 0.2 | RBF | 0.01 | 0.066 | 0.079 | 0.503 | 0.474 |
| 350 | 15 | 0.4 | LIN | - | 0.257 | 0.262 | 0.515 | 0.729 |
| 350 | 15 | 0.4 | RBF | 0.0001 | 0.381 | 0.370 | 0.550 | 0.747 |
| 350 | 15 | 0.4 | RBF | 0.001 | 0.353 | 0.348 | 0.555 | 0.721 |
| 350 | 15 | 0.4 | RBF | 0.01 | 0.057 | 0.071 | 0.502 | 0.472 |
| 350 | 15 | 0.6 | LIN | - | 0.320 | 0.321 | 0.529 | 0.717 |
| 350 | 15 | 0.6 | RBF | 0.0001 | 0.381 | 0.370 | 0.550 | 0.747 |
| 350 | 15 | 0.6 | RBF | 0.001 | 0.353 | 0.348 | 0.555 | 0.721 |
| 350 | 15 | 0.6 | RBF | 0.01 | 0.050 | 0.062 | 0.500 | 0.472 |
| 350 | 15 | 0.8 | LIN | - | 0.382 | 0.351 | 0.555 | 0.739 |
| 350 | 15 | 0.8 | RBF | 0.0001 | 0.381 | 0.370 | 0.550 | 0.747 |
| 350 | 15 | 0.8 | RBF | 0.001 | 0.353 | 0.348 | 0.555 | 0.721 |
| 350 | 15 | 0.8 | RBF | 0.01 | 0.043 | 0.057 | 0.500 | 0.471 |

Continued on next page

TABLE S16 – continued from previous page

| n | $k$ | $\lambda$ | usim | $\sigma$ | AP@5 | AP@10 | sCI | CI |
|---|---|---|---|---|---|---|---|---|
| 350 | 15 | 1.0 | LIN | - | 0.380 | 0.361 | 0.554 | 0.740 |
| 350 | 15 | 1.0 | RBF | 0.0001 | 0.381 | 0.370 | 0.550 | 0.747 |
| 350 | 15 | 1.0 | RBF | 0.001 | 0.353 | 0.348 | 0.555 | 0.721 |
| 350 | 15 | 1.0 | RBF | 0.01 | 0.040 | 0.055 | 0.500 | 0.471 |
| 350 | 15 | 10 | LIN | - | 0.349 | 0.352 | 0.549 | 0.736 |
| 350 | 15 | 10 | RBF | 0.0001 | 0.381 | 0.370 | 0.550 | 0.747 |
| 350 | 15 | 10 | RBF | 0.001 | 0.353 | 0.348 | 0.555 | 0.721 |
| 350 | 15 | 10 | RBF | 0.01 | 0.025 | 0.041 | 0.501 | 0.469 |
| 350 | 15 | 50 | LIN | - | 0.374 | 0.367 | 0.546 | 0.751 |
| 350 | 15 | 50 | RBF | 0.0001 | 0.381 | 0.370 | 0.550 | 0.747 |
| 350 | 15 | 50 | RBF | 0.001 | 0.353 | 0.348 | 0.555 | 0.721 |
| 350 | 15 | 50 | RBF | 0.01 | 0.021 | 0.037 | 0.501 | 0.469 |
| 350 | 15 | 100 | LIN | - | 0.377 | 0.370 | 0.546 | 0.749 |
| 350 | 15 | 100 | RBF | 0.0001 | 0.381 | 0.370 | 0.550 | 0.747 |
| 350 | 15 | 100 | RBF | 0.001 | 0.352 | 0.348 | 0.555 | 0.721 |
| 350 | 15 | 100 | RBF | 0.01 | 0.022 | 0.038 | 0.502 | 0.469 |
| 400 | 5 | 0.000001 | LIN | - | 0.234 | 0.249 | 0.538 | 0.711 |
| 400 | 5 | 0.000001 | RBF | 0.0001 | 0.328 | 0.320 | 0.555 | 0.727 |
| 400 | 5 | 0.000001 | RBF | 0.001 | 0.316 | 0.314 | 0.556 | 0.680 |
| 400 | 5 | 0.000001 | RBF | 0.01 | 0.183 | 0.195 | 0.523 | 0.540 |
| 400 | 5 | 0.00001 | LIN | - | 0.123 | 0.155 | 0.528 | 0.705 |
| 400 | 5 | 0.00001 | RBF | 0.0001 | 0.357 | 0.347 | 0.551 | 0.757 |
| 400 | 5 | 0.00001 | RBF | 0.001 | 0.355 | 0.358 | 0.552 | 0.720 |
| 400 | 5 | 0.00001 | RBF | 0.01 | 0.178 | 0.186 | 0.527 | 0.538 |
| 400 | 5 | 0.0001 | LIN | - | 0.204 | 0.222 | 0.516 | 0.709 |
| 400 | 5 | 0.0001 | RBF | 0.0001 | 0.370 | 0.366 | 0.552 | 0.746 |
| 400 | 5 | 0.0001 | RBF | 0.001 | 0.355 | 0.358 | 0.552 | 0.720 |
| 400 | 5 | 0.0001 | RBF | 0.01 | 0.150 | 0.158 | 0.525 | 0.517 |
| 400 | 5 | 0.001 | LIN | - | 0.109 | 0.141 | 0.524 | 0.634 |
| 400 | 5 | 0.001 | RBF | 0.0001 | 0.370 | 0.366 | 0.552 | 0.746 |
| 400 | 5 | 0.001 | RBF | 0.001 | 0.355 | 0.358 | 0.552 | 0.720 |
| 400 | 5 | 0.001 | RBF | 0.01 | 0.134 | 0.148 | 0.519 | 0.498 |
| 400 | 5 | 0.01 | LIN | - | 0.286 | 0.292 | 0.511 | 0.660 |
| 400 | 5 | 0.01 | RBF | 0.0001 | 0.370 | 0.366 | 0.552 | 0.746 |
| 400 | 5 | 0.01 | RBF | 0.001 | 0.355 | 0.358 | 0.552 | 0.720 |
| 400 | 5 | 0.01 | RBF | 0.01 | 0.100 | 0.111 | 0.506 | 0.484 |
| 400 | 5 | 0.1 | LIN | - | 0.328 | 0.318 | 0.555 | 0.742 |
| 400 | 5 | 0.1 | RBF | 0.0001 | 0.370 | 0.366 | 0.552 | 0.746 |
| 400 | 5 | 0.1 | RBF | 0.001 | 0.355 | 0.358 | 0.552 | 0.720 |
| 400 | 5 | 0.1 | RBF | 0.01 | 0.074 | 0.087 | 0.502 | 0.476 |
| 400 | 5 | 0.2 | LIN | - | 0.359 | 0.353 | 0.555 | 0.746 |
| 400 | 5 | 0.2 | RBF | 0.0001 | 0.370 | 0.366 | 0.552 | 0.746 |
| 400 | 5 | 0.2 | RBF | 0.001 | 0.355 | 0.358 | 0.552 | 0.720 |
| 400 | 5 | 0.2 | RBF | 0.01 | 0.068 | 0.080 | 0.503 | 0.474 |
| 400 | 5 | 0.4 | LIN | - | 0.374 | 0.362 | 0.555 | 0.752 |
| 400 | 5 | 0.4 | RBF | 0.0001 | 0.370 | 0.366 | 0.552 | 0.746 |
| 400 | 5 | 0.4 | RBF | 0.001 | 0.355 | 0.358 | 0.552 | 0.720 |
| 400 | 5 | 0.4 | RBF | 0.01 | 0.058 | 0.071 | 0.500 | 0.472 |
| 400 | 5 | 0.6 | LIN | - | 0.324 | 0.329 | 0.554 | 0.749 |
| 400 | 5 | 0.6 | RBF | 0.0001 | 0.370 | 0.366 | 0.552 | 0.746 |
| 400 | 5 | 0.6 | RBF | 0.001 | 0.355 | 0.358 | 0.552 | 0.720 |
| 400 | 5 | 0.6 | RBF | 0.01 | 0.050 | 0.065 | 0.501 | 0.471 |
| 400 | 5 | 0.8 | LIN | - | 0.359 | 0.342 | 0.554 | 0.750 |
| 400 | 5 | 0.8 | RBF | 0.0001 | 0.370 | 0.366 | 0.552 | 0.746 |
| 400 | 5 | 0.8 | RBF | 0.001 | 0.355 | 0.358 | 0.552 | 0.720 |
| 400 | 5 | 0.8 | RBF | 0.01 | 0.046 | 0.060 | 0.501 | 0.471 |
| 400 | 5 | 1.0 | LIN | - | 0.381 | 0.364 | 0.550 | 0.754 |
| 400 | 5 | 1.0 | RBF | 0.0001 | 0.370 | 0.366 | 0.552 | 0.746 |

Continued on next page

TABLE S16 – continued from previous page

| n | $k$ | $\lambda$ | usim | $\sigma$ | AP@5 | AP@10 | sCI | CI |
|---|---|---|---|---|---|---|---|---|
| 400 | 5 | 1.0 | RBF | 0.001 | 0.355 | 0.358 | 0.552 | 0.720 |
| 400 | 5 | 1.0 | RBF | 0.01 | 0.042 | 0.056 | 0.501 | 0.471 |
| 400 | 5 | 10 | LIN | - | 0.367 | 0.361 | 0.553 | 0.724 |
| 400 | 5 | 10 | RBF | 0.0001 | 0.370 | 0.366 | 0.552 | 0.746 |
| 400 | 5 | 10 | RBF | 0.001 | 0.355 | 0.358 | 0.551 | 0.720 |
| 400 | 5 | 10 | RBF | 0.01 | 0.026 | 0.043 | 0.501 | 0.469 |
| 400 | 5 | 50 | LIN | - | 0.366 | 0.362 | 0.554 | 0.695 |
| 400 | 5 | 50 | RBF | 0.0001 | 0.370 | 0.366 | 0.552 | 0.746 |
| 400 | 5 | 50 | RBF | 0.001 | 0.355 | 0.358 | 0.552 | 0.720 |
| 400 | 5 | 50 | RBF | 0.01 | 0.019 | 0.036 | 0.500 | 0.469 |
| 400 | 5 | 100 | LIN | - | 0.366 | 0.362 | 0.554 | 0.695 |
| 400 | 5 | 100 | RBF | 0.0001 | 0.370 | 0.366 | 0.552 | 0.746 |
| 400 | 5 | 100 | RBF | 0.001 | 0.355 | 0.358 | 0.552 | 0.720 |
| 400 | 5 | 100 | RBF | 0.01 | 0.020 | 0.037 | 0.501 | 0.469 |
| 400 | 10 | 0.000001 | LIN | - | 0.165 | 0.187 | 0.535 | 0.722 |
| 400 | 10 | 0.000001 | RBF | 0.001 | 0.331 | 0.334 | 0.557 | 0.664 |
| 400 | 10 | 0.000001 | RBF | 0.01 | 0.183 | 0.191 | 0.521 | 0.536 |
| 400 | 10 | 0.001 | LIN | - | 0.206 | 0.228 | 0.515 | 0.708 |
| 400 | 10 | 0.001 | RBF | 0.0001 | 0.374 | 0.370 | 0.552 | 0.743 |
| 400 | 10 | 0.001 | RBF | 0.001 | 0.354 | 0.350 | 0.552 | 0.710 |
| 400 | 10 | 0.001 | RBF | 0.01 | 0.138 | 0.153 | 0.519 | 0.497 |
| 400 | 10 | 0.01 | LIN | - | 0.228 | 0.233 | 0.525 | 0.687 |
| 400 | 10 | 0.01 | RBF | 0.0001 | 0.374 | 0.370 | 0.552 | 0.743 |
| 400 | 10 | 0.01 | RBF | 0.001 | 0.354 | 0.350 | 0.552 | 0.710 |
| 400 | 10 | 0.01 | RBF | 0.01 | 0.093 | 0.108 | 0.509 | 0.484 |
| 400 | 10 | 0.1 | LIN | - | 0.319 | 0.313 | 0.559 | 0.738 |
| 400 | 10 | 0.1 | RBF | 0.0001 | 0.374 | 0.370 | 0.552 | 0.743 |
| 400 | 10 | 0.1 | RBF | 0.001 | 0.354 | 0.350 | 0.552 | 0.710 |
| 400 | 10 | 0.1 | RBF | 0.01 | 0.076 | 0.089 | 0.503 | 0.476 |
| 400 | 10 | 0.2 | LIN | - | 0.332 | 0.327 | 0.557 | 0.739 |
| 400 | 10 | 0.2 | RBF | 0.0001 | 0.374 | 0.370 | 0.552 | 0.743 |
| 400 | 10 | 0.2 | RBF | 0.001 | 0.354 | 0.350 | 0.552 | 0.710 |
| 400 | 10 | 0.2 | RBF | 0.01 | 0.071 | 0.085 | 0.503 | 0.474 |
| 400 | 10 | 0.4 | LIN | - | 0.335 | 0.326 | 0.556 | 0.739 |
| 400 | 10 | 0.4 | RBF | 0.0001 | 0.374 | 0.370 | 0.552 | 0.743 |
| 400 | 10 | 0.4 | RBF | 0.001 | 0.354 | 0.350 | 0.552 | 0.710 |
| 400 | 10 | 0.4 | RBF | 0.01 | 0.059 | 0.074 | 0.501 | 0.472 |
| 400 | 10 | 0.6 | LIN | - | 0.381 | 0.357 | 0.560 | 0.739 |
| 400 | 10 | 0.6 | RBF | 0.0001 | 0.374 | 0.370 | 0.552 | 0.743 |
| 400 | 10 | 0.6 | RBF | 0.001 | 0.354 | 0.350 | 0.552 | 0.710 |
| 400 | 10 | 0.6 | RBF | 0.01 | 0.050 | 0.064 | 0.500 | 0.471 |
| 400 | 10 | 0.8 | LIN | - | 0.382 | 0.356 | 0.559 | 0.739 |
| 400 | 10 | 0.8 | RBF | 0.0001 | 0.374 | 0.370 | 0.552 | 0.743 |
| 400 | 10 | 0.8 | RBF | 0.001 | 0.354 | 0.350 | 0.552 | 0.710 |
| 400 | 10 | 0.8 | RBF | 0.01 | 0.047 | 0.062 | 0.501 | 0.471 |
| 400 | 10 | 1.0 | LIN | - | 0.338 | 0.310 | 0.558 | 0.738 |
| 400 | 10 | 1.0 | RBF | 0.0001 | 0.374 | 0.370 | 0.552 | 0.743 |
| 400 | 10 | 1.0 | RBF | 0.001 | 0.354 | 0.350 | 0.552 | 0.710 |
| 400 | 10 | 1.0 | RBF | 0.01 | 0.044 | 0.058 | 0.501 | 0.471 |
| 400 | 10 | 10 | LIN | - | 0.376 | 0.366 | 0.548 | 0.754 |
| 400 | 10 | 10 | RBF | 0.0001 | 0.374 | 0.370 | 0.552 | 0.743 |
| 400 | 10 | 10 | RBF | 0.001 | 0.354 | 0.350 | 0.552 | 0.710 |
| 400 | 10 | 10 | RBF | 0.01 | 0.029 | 0.045 | 0.502 | 0.469 |
| 400 | 10 | 50 | LIN | - | 0.379 | 0.370 | 0.549 | 0.745 |
| 400 | 10 | 50 | RBF | 0.0001 | 0.374 | 0.370 | 0.552 | 0.743 |
| 400 | 10 | 50 | RBF | 0.001 | 0.354 | 0.350 | 0.552 | 0.710 |
| 400 | 10 | 50 | RBF | 0.01 | 0.023 | 0.039 | 0.501 | 0.469 |
| 400 | 10 | 100 | LIN | - | 0.382 | 0.373 | 0.550 | 0.746 |

Continued on next page

TABLE S16 – continued from previous page

| n | $k$ | $\lambda$ | usim | $\sigma$ | AP@5 | AP@10 | sCI | CI |
|---|---|---|---|---|---|---|---|---|
| 400 | 10 | 100 | RBF | 0.0001 | 0.374 | 0.370 | 0.552 | 0.743 |
| 400 | 10 | 100 | RBF | 0.001 | 0.354 | 0.350 | 0.552 | 0.710 |
| 400 | 10 | 100 | RBF | 0.01 | 0.019 | 0.036 | 0.501 | 0.469 |
| 400 | 15 | 0.001 | LIN | - | 0.154 | 0.178 | 0.515 | 0.694 |
| 400 | 15 | 0.001 | RBF | 0.0001 | 0.378 | 0.370 | 0.552 | 0.742 |
| 400 | 15 | 0.001 | RBF | 0.001 | 0.351 | 0.346 | 0.552 | 0.710 |
| 400 | 15 | 0.001 | RBF | 0.01 | 0.136 | 0.147 | 0.518 | 0.496 |
| 400 | 15 | 0.01 | LIN | - | 0.282 | 0.285 | 0.556 | 0.732 |
| 400 | 15 | 0.01 | RBF | 0.0001 | 0.378 | 0.370 | 0.552 | 0.742 |
| 400 | 15 | 0.01 | RBF | 0.001 | 0.351 | 0.346 | 0.552 | 0.710 |
| 400 | 15 | 0.01 | RBF | 0.01 | 0.097 | 0.112 | 0.509 | 0.484 |
| 400 | 15 | 0.1 | LIN | - | 0.339 | 0.341 | 0.558 | 0.730 |
| 400 | 15 | 0.1 | RBF | 0.0001 | 0.378 | 0.370 | 0.552 | 0.742 |
| 400 | 15 | 0.1 | RBF | 0.001 | 0.351 | 0.346 | 0.552 | 0.710 |
| 400 | 15 | 0.1 | RBF | 0.01 | 0.077 | 0.089 | 0.504 | 0.476 |
| 400 | 15 | 0.2 | LIN | - | 0.301 | 0.298 | 0.560 | 0.724 |
| 400 | 15 | 0.2 | RBF | 0.0001 | 0.378 | 0.370 | 0.552 | 0.742 |
| 400 | 15 | 0.2 | RBF | 0.001 | 0.351 | 0.346 | 0.552 | 0.710 |
| 400 | 15 | 0.2 | RBF | 0.01 | 0.068 | 0.082 | 0.503 | 0.474 |
| 400 | 15 | 0.4 | LIN | - | 0.359 | 0.344 | 0.554 | 0.719 |
| 400 | 15 | 0.4 | RBF | 0.0001 | 0.378 | 0.370 | 0.552 | 0.742 |
| 400 | 15 | 0.4 | RBF | 0.001 | 0.351 | 0.346 | 0.552 | 0.710 |
| 400 | 15 | 0.4 | RBF | 0.01 | 0.060 | 0.074 | 0.501 | 0.472 |
| 400 | 15 | 0.6 | LIN | - | 0.381 | 0.370 | 0.557 | 0.716 |
| 400 | 15 | 0.6 | RBF | 0.0001 | 0.378 | 0.370 | 0.552 | 0.742 |
| 400 | 15 | 0.6 | RBF | 0.001 | 0.351 | 0.346 | 0.552 | 0.710 |
| 400 | 15 | 0.6 | RBF | 0.01 | 0.051 | 0.065 | 0.500 | 0.471 |
| 400 | 15 | 0.8 | LIN | - | 0.358 | 0.354 | 0.558 | 0.712 |
| 400 | 15 | 0.8 | RBF | 0.0001 | 0.378 | 0.370 | 0.552 | 0.742 |
| 400 | 15 | 0.8 | RBF | 0.001 | 0.351 | 0.346 | 0.552 | 0.710 |
| 400 | 15 | 0.8 | RBF | 0.01 | 0.047 | 0.061 | 0.501 | 0.471 |
| 400 | 15 | 1.0 | LIN | - | 0.361 | 0.358 | 0.557 | 0.709 |
| 400 | 15 | 1.0 | RBF | 0.0001 | 0.378 | 0.370 | 0.552 | 0.742 |
| 400 | 15 | 1.0 | RBF | 0.001 | 0.351 | 0.346 | 0.552 | 0.710 |
| 400 | 15 | 1.0 | RBF | 0.01 | 0.044 | 0.058 | 0.501 | 0.471 |
| 400 | 15 | 10 | LIN | - | 0.362 | 0.361 | 0.551 | 0.732 |
| 400 | 15 | 10 | RBF | 0.0001 | 0.378 | 0.370 | 0.552 | 0.742 |
| 400 | 15 | 10 | RBF | 0.001 | 0.351 | 0.346 | 0.552 | 0.710 |
| 400 | 15 | 10 | RBF | 0.01 | 0.028 | 0.045 | 0.502 | 0.469 |
| 400 | 15 | 50 | LIN | - | 0.380 | 0.372 | 0.550 | 0.744 |
| 400 | 15 | 50 | RBF | 0.0001 | 0.378 | 0.370 | 0.552 | 0.742 |
| 400 | 15 | 50 | RBF | 0.001 | 0.351 | 0.346 | 0.552 | 0.710 |
| 400 | 15 | 50 | RBF | 0.01 | 0.021 | 0.038 | 0.501 | 0.469 |
| 400 | 15 | 100 | LIN | - | 0.380 | 0.372 | 0.550 | 0.744 |
| 400 | 15 | 100 | RBF | 0.0001 | 0.378 | 0.370 | 0.552 | 0.742 |
| 400 | 15 | 100 | RBF | 0.001 | 0.351 | 0.346 | 0.551 | 0.710 |
| 400 | 15 | 100 | RBF | 0.01 | 0.022 | 0.038 | 0.501 | 0.469 |

The columns corresponding to "$k$", "$\lambda$", "usim", and "$\sigma$" have the two hyperparameters, cell line similarity function, and parameter for RBF cell line similarity, respectively, for KRL.

**TABLE S17:** KRL Performance on New Cell Lines ($\theta$ = 5)

| n | $k$ | $\lambda$ | usim | $\sigma$ | AP@5 | AP@10 | sCI | CI |
|---|---|---|---|---|---|---|---|---|
| 50 | 5 | 0.000001 | RBF | 0.0001 | 0.511 | 0.463 | 0.538 | 0.729 |
| 50 | 5 | 0.000001 | RBF | 0.001 | 0.474 | 0.438 | 0.570 | 0.736 |
| 50 | 5 | 0.000001 | RBF | 0.01 | 0.261 | 0.267 | 0.550 | 0.620 |
| 50 | 5 | 0.00001 | RBF | 0.01 | 0.275 | 0.306 | 0.533 | 0.635 |
| 50 | 5 | 0.0001 | RBF | 0.0001 | 0.478 | 0.450 | 0.552 | 0.783 |
| 50 | 5 | 0.0001 | RBF | 0.001 | 0.602 | 0.530 | 0.560 | 0.764 |
| 50 | 5 | 0.0001 | RBF | 0.01 | 0.295 | 0.319 | 0.527 | 0.604 |
| 50 | 5 | 0.001 | LIN | - | 0.422 | 0.400 | 0.551 | 0.723 |
| 50 | 5 | 0.001 | RBF | 0.0001 | 0.571 | 0.529 | 0.559 | 0.734 |
| 50 | 5 | 0.001 | RBF | 0.001 | 0.602 | 0.530 | 0.560 | 0.764 |
| 50 | 5 | 0.001 | RBF | 0.01 | 0.288 | 0.304 | 0.528 | 0.558 |
| 50 | 5 | 0.01 | LIN | - | 0.499 | 0.438 | 0.545 | 0.738 |
| 50 | 5 | 0.01 | RBF | 0.0001 | 0.571 | 0.529 | 0.559 | 0.734 |
| 50 | 5 | 0.01 | RBF | 0.001 | 0.602 | 0.530 | 0.560 | 0.764 |
| 50 | 5 | 0.01 | RBF | 0.01 | 0.204 | 0.249 | 0.512 | 0.506 |
| 50 | 5 | 0.1 | LIN | - | 0.570 | 0.506 | 0.535 | 0.767 |
| 50 | 5 | 0.1 | RBF | 0.0001 | 0.571 | 0.529 | 0.559 | 0.734 |
| 50 | 5 | 0.1 | RBF | 0.001 | 0.602 | 0.530 | 0.560 | 0.764 |
| 50 | 5 | 0.1 | RBF | 0.01 | 0.144 | 0.173 | 0.508 | 0.477 |
| 50 | 5 | 0.2 | LIN | - | 0.516 | 0.483 | 0.553 | 0.766 |
| 50 | 5 | 0.2 | RBF | 0.0001 | 0.571 | 0.529 | 0.559 | 0.734 |
| 50 | 5 | 0.2 | RBF | 0.001 | 0.602 | 0.530 | 0.560 | 0.764 |
| 50 | 5 | 0.2 | RBF | 0.01 | 0.071 | 0.099 | 0.512 | 0.473 |
| 50 | 5 | 0.4 | LIN | - | 0.454 | 0.430 | 0.535 | 0.780 |
| 50 | 5 | 0.4 | RBF | 0.0001 | 0.571 | 0.529 | 0.559 | 0.734 |
| 50 | 5 | 0.4 | RBF | 0.001 | 0.602 | 0.530 | 0.560 | 0.764 |
| 50 | 5 | 0.4 | RBF | 0.01 | 0.067 | 0.093 | 0.509 | 0.471 |
| 50 | 5 | 0.6 | LIN | - | 0.438 | 0.417 | 0.548 | 0.761 |
| 50 | 5 | 0.6 | RBF | 0.0001 | 0.571 | 0.529 | 0.559 | 0.734 |
| 50 | 5 | 0.6 | RBF | 0.001 | 0.602 | 0.530 | 0.560 | 0.764 |
| 50 | 5 | 0.6 | RBF | 0.01 | 0.037 | 0.069 | 0.508 | 0.470 |
| 50 | 5 | 0.8 | LIN | - | 0.594 | 0.559 | 0.548 | 0.760 |
| 50 | 5 | 0.8 | RBF | 0.0001 | 0.571 | 0.529 | 0.559 | 0.734 |
| 50 | 5 | 0.8 | RBF | 0.001 | 0.602 | 0.530 | 0.560 | 0.764 |
| 50 | 5 | 0.8 | RBF | 0.01 | 0.046 | 0.077 | 0.508 | 0.469 |
| 50 | 5 | 1.0 | LIN | - | 0.573 | 0.536 | 0.547 | 0.774 |
| 50 | 5 | 1.0 | RBF | 0.0001 | 0.571 | 0.529 | 0.559 | 0.734 |
| 50 | 5 | 1.0 | RBF | 0.001 | 0.602 | 0.530 | 0.560 | 0.764 |
| 50 | 5 | 1.0 | RBF | 0.01 | 0.046 | 0.077 | 0.508 | 0.469 |
| 50 | 5 | 10 | LIN | - | 0.567 | 0.520 | 0.531 | 0.789 |
| 50 | 5 | 10 | RBF | 0.0001 | 0.571 | 0.529 | 0.559 | 0.734 |
| 50 | 5 | 10 | RBF | 0.001 | 0.602 | 0.530 | 0.560 | 0.764 |
| 50 | 5 | 10 | RBF | 0.01 | 0.021 | 0.051 | 0.510 | 0.469 |
| 50 | 5 | 50 | LIN | - | 0.586 | 0.560 | 0.561 | 0.752 |
| 50 | 5 | 50 | RBF | 0.0001 | 0.571 | 0.529 | 0.559 | 0.734 |
| 50 | 5 | 50 | RBF | 0.001 | 0.602 | 0.530 | 0.560 | 0.764 |
| 50 | 5 | 50 | RBF | 0.01 | 0.018 | 0.050 | 0.509 | 0.468 |
| 50 | 5 | 100 | LIN | - | 0.590 | 0.530 | 0.561 | 0.707 |
| 50 | 5 | 100 | RBF | 0.0001 | 0.571 | 0.529 | 0.559 | 0.734 |
| 50 | 5 | 100 | RBF | 0.001 | 0.602 | 0.530 | 0.560 | 0.764 |
| 50 | 5 | 100 | RBF | 0.01 | 0.021 | 0.053 | 0.509 | 0.468 |
| 50 | 10 | 0.000001 | LIN | - | 0.347 | 0.355 | 0.534 | 0.700 |
| 50 | 10 | 0.000001 | RBF | 0.01 | 0.288 | 0.281 | 0.548 | 0.610 |
| 50 | 10 | 0.001 | LIN | - | 0.401 | 0.352 | 0.535 | 0.700 |
| 50 | 10 | 0.001 | RBF | 0.0001 | 0.571 | 0.534 | 0.563 | 0.774 |
| 50 | 10 | 0.001 | RBF | 0.001 | 0.609 | 0.535 | 0.564 | 0.777 |
| 50 | 10 | 0.001 | RBF | 0.01 | 0.260 | 0.287 | 0.535 | 0.570 |

Continued on next page

TABLE S17 – continued from previous page

| n | $k$ | $\lambda$ | usim | $\sigma$ | AP@5 | AP@10 | sCI | CI |
|---|---|---|---|---|---|---|---|---|
| 50 | 10 | 0.01 | LIN | - | 0.461 | 0.450 | 0.551 | 0.768 |
| 50 | 10 | 0.01 | RBF | 0.0001 | 0.571 | 0.534 | 0.563 | 0.774 |
| 50 | 10 | 0.01 | RBF | 0.001 | 0.609 | 0.535 | 0.564 | 0.777 |
| 50 | 10 | 0.01 | RBF | 0.01 | 0.215 | 0.251 | 0.516 | 0.512 |
| 50 | 10 | 0.1 | LIN | - | 0.583 | 0.526 | 0.545 | 0.783 |
| 50 | 10 | 0.1 | RBF | 0.0001 | 0.571 | 0.534 | 0.563 | 0.774 |
| 50 | 10 | 0.1 | RBF | 0.001 | 0.609 | 0.535 | 0.564 | 0.777 |
| 50 | 10 | 0.1 | RBF | 0.01 | 0.145 | 0.174 | 0.509 | 0.479 |
| 50 | 10 | 0.2 | LIN | - | 0.528 | 0.479 | 0.550 | 0.782 |
| 50 | 10 | 0.2 | RBF | 0.0001 | 0.571 | 0.534 | 0.563 | 0.774 |
| 50 | 10 | 0.2 | RBF | 0.001 | 0.609 | 0.535 | 0.564 | 0.777 |
| 50 | 10 | 0.2 | RBF | 0.01 | 0.069 | 0.098 | 0.512 | 0.474 |
| 50 | 10 | 0.4 | LIN | - | 0.600 | 0.546 | 0.551 | 0.786 |
| 50 | 10 | 0.4 | RBF | 0.0001 | 0.571 | 0.534 | 0.563 | 0.774 |
| 50 | 10 | 0.4 | RBF | 0.001 | 0.609 | 0.535 | 0.564 | 0.777 |
| 50 | 10 | 0.4 | RBF | 0.01 | 0.077 | 0.104 | 0.510 | 0.472 |
| 50 | 10 | 0.6 | LIN | - | 0.597 | 0.556 | 0.549 | 0.783 |
| 50 | 10 | 0.6 | RBF | 0.0001 | 0.571 | 0.534 | 0.563 | 0.774 |
| 50 | 10 | 0.6 | RBF | 0.001 | 0.609 | 0.535 | 0.564 | 0.777 |
| 50 | 10 | 0.6 | RBF | 0.01 | 0.049 | 0.081 | 0.509 | 0.470 |
| 50 | 10 | 0.8 | LIN | - | 0.587 | 0.559 | 0.545 | 0.785 |
| 50 | 10 | 0.8 | RBF | 0.0001 | 0.571 | 0.534 | 0.563 | 0.774 |
| 50 | 10 | 0.8 | RBF | 0.001 | 0.609 | 0.535 | 0.564 | 0.777 |
| 50 | 10 | 0.8 | RBF | 0.01 | 0.046 | 0.078 | 0.510 | 0.470 |
| 50 | 10 | 1.0 | LIN | - | 0.594 | 0.539 | 0.545 | 0.785 |
| 50 | 10 | 1.0 | RBF | 0.0001 | 0.571 | 0.534 | 0.563 | 0.774 |
| 50 | 10 | 1.0 | RBF | 0.001 | 0.609 | 0.535 | 0.564 | 0.777 |
| 50 | 10 | 1.0 | RBF | 0.01 | 0.049 | 0.081 | 0.510 | 0.470 |
| 50 | 10 | 10 | LIN | - | 0.582 | 0.545 | 0.547 | 0.791 |
| 50 | 10 | 10 | RBF | 0.0001 | 0.571 | 0.534 | 0.563 | 0.774 |
| 50 | 10 | 10 | RBF | 0.001 | 0.609 | 0.535 | 0.564 | 0.777 |
| 50 | 10 | 10 | RBF | 0.01 | 0.019 | 0.051 | 0.510 | 0.469 |
| 50 | 10 | 50 | LIN | - | 0.586 | 0.555 | 0.553 | 0.768 |
| 50 | 10 | 50 | RBF | 0.0001 | 0.571 | 0.534 | 0.563 | 0.774 |
| 50 | 10 | 50 | RBF | 0.001 | 0.609 | 0.535 | 0.564 | 0.777 |
| 50 | 10 | 50 | RBF | 0.01 | 0.024 | 0.054 | 0.510 | 0.469 |
| 50 | 10 | 100 | LIN | - | 0.572 | 0.535 | 0.561 | 0.720 |
| 50 | 10 | 100 | RBF | 0.0001 | 0.571 | 0.534 | 0.563 | 0.774 |
| 50 | 10 | 100 | RBF | 0.001 | 0.609 | 0.535 | 0.564 | 0.777 |
| 50 | 10 | 100 | RBF | 0.01 | 0.021 | 0.053 | 0.509 | 0.468 |
| 50 | 15 | 0.001 | LIN | - | 0.374 | 0.362 | 0.534 | 0.717 |
| 50 | 15 | 0.001 | RBF | 0.0001 | 0.577 | 0.522 | 0.562 | 0.781 |
| 50 | 15 | 0.001 | RBF | 0.001 | 0.608 | 0.538 | 0.566 | 0.776 |
| 50 | 15 | 0.001 | RBF | 0.01 | 0.277 | 0.303 | 0.538 | 0.574 |
| 50 | 15 | 0.01 | LIN | - | 0.473 | 0.436 | 0.555 | 0.768 |
| 50 | 15 | 0.01 | RBF | 0.0001 | 0.577 | 0.522 | 0.562 | 0.781 |
| 50 | 15 | 0.01 | RBF | 0.001 | 0.608 | 0.538 | 0.566 | 0.776 |
| 50 | 15 | 0.01 | RBF | 0.01 | 0.228 | 0.260 | 0.518 | 0.515 |
| 50 | 15 | 0.1 | LIN | - | 0.347 | 0.339 | 0.515 | 0.743 |
| 50 | 15 | 0.1 | RBF | 0.0001 | 0.577 | 0.522 | 0.562 | 0.781 |
| 50 | 15 | 0.1 | RBF | 0.001 | 0.608 | 0.538 | 0.566 | 0.776 |
| 50 | 15 | 0.1 | RBF | 0.01 | 0.141 | 0.171 | 0.513 | 0.480 |
| 50 | 15 | 0.2 | LIN | - | 0.621 | 0.573 | 0.548 | 0.780 |
| 50 | 15 | 0.2 | RBF | 0.0001 | 0.577 | 0.522 | 0.562 | 0.781 |
| 50 | 15 | 0.2 | RBF | 0.001 | 0.608 | 0.538 | 0.566 | 0.776 |
| 50 | 15 | 0.2 | RBF | 0.01 | 0.076 | 0.106 | 0.513 | 0.474 |
| 50 | 15 | 0.4 | LIN | - | 0.605 | 0.555 | 0.551 | 0.783 |
| 50 | 15 | 0.4 | RBF | 0.0001 | 0.577 | 0.522 | 0.562 | 0.781 |

Continued on next page

TABLE S17 – continued from previous page

| n | $k$ | $\lambda$ | usim | $\sigma$ | AP@5 | AP@10 | sCI | CI |
|---|---|---|---|---|---|---|---|---|
| 50 | 15 | 0.4 | RBF | 0.001 | 0.608 | 0.538 | 0.566 | 0.776 |
| 50 | 15 | 0.4 | RBF | 0.01 | 0.081 | 0.108 | 0.512 | 0.471 |
| 50 | 15 | 0.6 | LIN | - | 0.602 | 0.563 | 0.550 | 0.783 |
| 50 | 15 | 0.6 | RBF | 0.0001 | 0.577 | 0.522 | 0.562 | 0.781 |
| 50 | 15 | 0.6 | RBF | 0.001 | 0.608 | 0.538 | 0.566 | 0.776 |
| 50 | 15 | 0.6 | RBF | 0.01 | 0.049 | 0.082 | 0.510 | 0.470 |
| 50 | 15 | 0.8 | LIN | - | 0.303 | 0.332 | 0.510 | 0.758 |
| 50 | 15 | 0.8 | RBF | 0.0001 | 0.577 | 0.522 | 0.562 | 0.781 |
| 50 | 15 | 0.8 | RBF | 0.001 | 0.608 | 0.538 | 0.566 | 0.776 |
| 50 | 15 | 0.8 | RBF | 0.01 | 0.046 | 0.078 | 0.511 | 0.470 |
| 50 | 15 | 1.0 | LIN | - | 0.466 | 0.445 | 0.532 | 0.757 |
| 50 | 15 | 1.0 | RBF | 0.0001 | 0.577 | 0.522 | 0.562 | 0.781 |
| 50 | 15 | 1.0 | RBF | 0.001 | 0.608 | 0.538 | 0.566 | 0.776 |
| 50 | 15 | 1.0 | RBF | 0.01 | 0.046 | 0.078 | 0.512 | 0.470 |
| 50 | 15 | 10 | LIN | - | 0.547 | 0.529 | 0.551 | 0.786 |
| 50 | 15 | 10 | RBF | 0.0001 | 0.577 | 0.522 | 0.562 | 0.781 |
| 50 | 15 | 10 | RBF | 0.001 | 0.608 | 0.538 | 0.566 | 0.776 |
| 50 | 15 | 10 | RBF | 0.01 | 0.019 | 0.051 | 0.511 | 0.469 |
| 50 | 15 | 50 | LIN | - | 0.593 | 0.560 | 0.546 | 0.785 |
| 50 | 15 | 50 | RBF | 0.0001 | 0.577 | 0.522 | 0.562 | 0.781 |
| 50 | 15 | 50 | RBF | 0.001 | 0.608 | 0.538 | 0.566 | 0.776 |
| 50 | 15 | 50 | RBF | 0.01 | 0.024 | 0.054 | 0.510 | 0.469 |
| 50 | 15 | 100 | LIN | - | 0.567 | 0.520 | 0.557 | 0.748 |
| 50 | 15 | 100 | RBF | 0.0001 | 0.577 | 0.522 | 0.562 | 0.781 |
| 50 | 15 | 100 | RBF | 0.001 | 0.608 | 0.538 | 0.566 | 0.776 |
| 50 | 15 | 100 | RBF | 0.01 | 0.019 | 0.051 | 0.509 | 0.469 |
| 100 | 5 | 0.000001 | RBF | 0.0001 | 0.503 | 0.474 | 0.541 | 0.726 |
| 100 | 5 | 0.000001 | RBF | 0.001 | 0.562 | 0.481 | 0.550 | 0.732 |
| 100 | 5 | 0.000001 | RBF | 0.01 | 0.278 | 0.272 | 0.526 | 0.614 |
| 100 | 5 | 0.00001 | LIN | - | 0.350 | 0.333 | 0.521 | 0.692 |
| 100 | 5 | 0.00001 | RBF | 0.01 | 0.264 | 0.277 | 0.517 | 0.618 |
| 100 | 5 | 0.0001 | RBF | 0.0001 | 0.495 | 0.439 | 0.545 | 0.779 |
| 100 | 5 | 0.0001 | RBF | 0.001 | 0.568 | 0.497 | 0.568 | 0.761 |
| 100 | 5 | 0.0001 | RBF | 0.01 | 0.238 | 0.259 | 0.520 | 0.586 |
| 100 | 5 | 0.001 | LIN | - | 0.417 | 0.408 | 0.539 | 0.721 |
| 100 | 5 | 0.001 | RBF | 0.0001 | 0.512 | 0.470 | 0.557 | 0.733 |
| 100 | 5 | 0.001 | RBF | 0.001 | 0.568 | 0.497 | 0.568 | 0.761 |
| 100 | 5 | 0.001 | RBF | 0.01 | 0.227 | 0.248 | 0.512 | 0.546 |
| 100 | 5 | 0.01 | LIN | - | 0.463 | 0.446 | 0.534 | 0.743 |
| 100 | 5 | 0.01 | RBF | 0.0001 | 0.512 | 0.470 | 0.557 | 0.733 |
| 100 | 5 | 0.01 | RBF | 0.001 | 0.568 | 0.497 | 0.568 | 0.761 |
| 100 | 5 | 0.01 | RBF | 0.01 | 0.182 | 0.209 | 0.509 | 0.508 |
| 100 | 5 | 0.1 | LIN | - | 0.479 | 0.444 | 0.543 | 0.768 |
| 100 | 5 | 0.1 | RBF | 0.0001 | 0.512 | 0.470 | 0.557 | 0.733 |
| 100 | 5 | 0.1 | RBF | 0.001 | 0.568 | 0.497 | 0.568 | 0.761 |
| 100 | 5 | 0.1 | RBF | 0.01 | 0.140 | 0.164 | 0.510 | 0.483 |
| 100 | 5 | 0.2 | LIN | - | 0.458 | 0.429 | 0.544 | 0.763 |
| 100 | 5 | 0.2 | RBF | 0.0001 | 0.512 | 0.470 | 0.557 | 0.733 |
| 100 | 5 | 0.2 | RBF | 0.001 | 0.568 | 0.497 | 0.568 | 0.761 |
| 100 | 5 | 0.2 | RBF | 0.01 | 0.074 | 0.102 | 0.512 | 0.478 |
| 100 | 5 | 0.4 | LIN | - | 0.495 | 0.485 | 0.546 | 0.769 |
| 100 | 5 | 0.4 | RBF | 0.0001 | 0.512 | 0.470 | 0.557 | 0.733 |
| 100 | 5 | 0.4 | RBF | 0.001 | 0.568 | 0.497 | 0.568 | 0.761 |
| 100 | 5 | 0.4 | RBF | 0.01 | 0.075 | 0.106 | 0.509 | 0.475 |
| 100 | 5 | 0.6 | LIN | - | 0.524 | 0.493 | 0.551 | 0.762 |
| 100 | 5 | 0.6 | RBF | 0.0001 | 0.512 | 0.470 | 0.557 | 0.733 |
| 100 | 5 | 0.6 | RBF | 0.001 | 0.568 | 0.497 | 0.568 | 0.761 |
| 100 | 5 | 0.6 | RBF | 0.01 | 0.064 | 0.099 | 0.509 | 0.473 |

Continued on next page

TABLE S17 – continued from previous page

| n | $k$ | $\lambda$ | usim | $\sigma$ | AP@5 | AP@10 | sCI | CI |
|---|---|---|---|---|---|---|---|---|
| 100 | 5 | 0.8 | LIN | - | 0.524 | 0.488 | 0.549 | 0.761 |
| 100 | 5 | 0.8 | RBF | 0.0001 | 0.512 | 0.470 | 0.557 | 0.733 |
| 100 | 5 | 0.8 | RBF | 0.001 | 0.568 | 0.497 | 0.568 | 0.761 |
| 100 | 5 | 0.8 | RBF | 0.01 | 0.053 | 0.089 | 0.509 | 0.472 |
| 100 | 5 | 1.0 | LIN | - | 0.555 | 0.503 | 0.549 | 0.775 |
| 100 | 5 | 1.0 | RBF | 0.0001 | 0.512 | 0.470 | 0.557 | 0.733 |
| 100 | 5 | 1.0 | RBF | 0.001 | 0.568 | 0.497 | 0.568 | 0.761 |
| 100 | 5 | 1.0 | RBF | 0.01 | 0.043 | 0.077 | 0.508 | 0.472 |
| 100 | 5 | 10 | LIN | - | 0.504 | 0.477 | 0.535 | 0.782 |
| 100 | 5 | 10 | RBF | 0.0001 | 0.512 | 0.470 | 0.557 | 0.733 |
| 100 | 5 | 10 | RBF | 0.001 | 0.568 | 0.497 | 0.568 | 0.761 |
| 100 | 5 | 10 | RBF | 0.01 | 0.026 | 0.064 | 0.506 | 0.469 |
| 100 | 5 | 50 | LIN | - | 0.515 | 0.500 | 0.558 | 0.752 |
| 100 | 5 | 50 | RBF | 0.0001 | 0.512 | 0.470 | 0.557 | 0.733 |
| 100 | 5 | 50 | RBF | 0.001 | 0.568 | 0.497 | 0.568 | 0.761 |
| 100 | 5 | 50 | RBF | 0.01 | 0.026 | 0.066 | 0.505 | 0.468 |
| 100 | 5 | 100 | LIN | - | 0.508 | 0.469 | 0.557 | 0.699 |
| 100 | 5 | 100 | RBF | 0.0001 | 0.512 | 0.470 | 0.557 | 0.733 |
| 100 | 5 | 100 | RBF | 0.001 | 0.568 | 0.497 | 0.568 | 0.761 |
| 100 | 5 | 100 | RBF | 0.01 | 0.026 | 0.067 | 0.505 | 0.468 |
| 100 | 10 | 0.000001 | LIN | - | 0.160 | 0.203 | 0.520 | 0.694 |
| 100 | 10 | 0.000001 | RBF | 0.01 | 0.280 | 0.284 | 0.531 | 0.605 |
| 100 | 10 | 0.001 | RBF | 0.0001 | 0.523 | 0.485 | 0.559 | 0.773 |
| 100 | 10 | 0.001 | RBF | 0.001 | 0.560 | 0.496 | 0.566 | 0.774 |
| 100 | 10 | 0.001 | RBF | 0.01 | 0.210 | 0.247 | 0.512 | 0.557 |
| 100 | 10 | 0.01 | LIN | - | 0.484 | 0.454 | 0.547 | 0.765 |
| 100 | 10 | 0.01 | RBF | 0.0001 | 0.523 | 0.485 | 0.559 | 0.773 |
| 100 | 10 | 0.01 | RBF | 0.001 | 0.560 | 0.496 | 0.566 | 0.774 |
| 100 | 10 | 0.01 | RBF | 0.01 | 0.188 | 0.218 | 0.509 | 0.514 |
| 100 | 10 | 0.1 | LIN | - | 0.513 | 0.458 | 0.553 | 0.781 |
| 100 | 10 | 0.1 | RBF | 0.0001 | 0.523 | 0.485 | 0.559 | 0.773 |
| 100 | 10 | 0.1 | RBF | 0.001 | 0.560 | 0.496 | 0.566 | 0.774 |
| 100 | 10 | 0.1 | RBF | 0.01 | 0.138 | 0.165 | 0.511 | 0.485 |
| 100 | 10 | 0.2 | LIN | - | 0.525 | 0.480 | 0.550 | 0.774 |
| 100 | 10 | 0.2 | RBF | 0.0001 | 0.523 | 0.485 | 0.559 | 0.773 |
| 100 | 10 | 0.2 | RBF | 0.001 | 0.560 | 0.496 | 0.566 | 0.774 |
| 100 | 10 | 0.2 | RBF | 0.01 | 0.087 | 0.115 | 0.513 | 0.479 |
| 100 | 10 | 0.4 | LIN | - | 0.538 | 0.496 | 0.547 | 0.781 |
| 100 | 10 | 0.4 | RBF | 0.0001 | 0.523 | 0.485 | 0.559 | 0.773 |
| 100 | 10 | 0.4 | RBF | 0.001 | 0.560 | 0.496 | 0.566 | 0.774 |
| 100 | 10 | 0.4 | RBF | 0.01 | 0.077 | 0.108 | 0.510 | 0.475 |
| 100 | 10 | 0.6 | LIN | - | 0.547 | 0.488 | 0.547 | 0.784 |
| 100 | 10 | 0.6 | RBF | 0.0001 | 0.523 | 0.485 | 0.559 | 0.773 |
| 100 | 10 | 0.6 | RBF | 0.001 | 0.560 | 0.496 | 0.566 | 0.774 |
| 100 | 10 | 0.6 | RBF | 0.01 | 0.068 | 0.105 | 0.509 | 0.473 |
| 100 | 10 | 0.8 | LIN | - | 0.481 | 0.466 | 0.552 | 0.781 |
| 100 | 10 | 0.8 | RBF | 0.0001 | 0.523 | 0.485 | 0.559 | 0.773 |
| 100 | 10 | 0.8 | RBF | 0.001 | 0.560 | 0.496 | 0.566 | 0.774 |
| 100 | 10 | 0.8 | RBF | 0.01 | 0.057 | 0.094 | 0.509 | 0.472 |
| 100 | 10 | 1.0 | LIN | - | 0.542 | 0.498 | 0.545 | 0.784 |
| 100 | 10 | 1.0 | RBF | 0.0001 | 0.523 | 0.485 | 0.559 | 0.773 |
| 100 | 10 | 1.0 | RBF | 0.001 | 0.560 | 0.496 | 0.566 | 0.774 |
| 100 | 10 | 1.0 | RBF | 0.01 | 0.056 | 0.092 | 0.509 | 0.472 |
| 100 | 10 | 10 | LIN | - | 0.493 | 0.466 | 0.543 | 0.774 |
| 100 | 10 | 10 | RBF | 0.0001 | 0.523 | 0.485 | 0.559 | 0.773 |
| 100 | 10 | 10 | RBF | 0.001 | 0.560 | 0.496 | 0.566 | 0.774 |
| 100 | 10 | 10 | RBF | 0.01 | 0.028 | 0.067 | 0.506 | 0.469 |
| 100 | 10 | 50 | LIN | - | 0.525 | 0.499 | 0.550 | 0.771 |

Continued on next page

TABLE S17 – continued from previous page

| n | $k$ | $\lambda$ | usim | $\sigma$ | AP@5 | AP@10 | sCI | CI |
|---|---|---|---|---|---|---|---|---|
| 100 | 10 | 50 | RBF | 0.0001 | 0.523 | 0.485 | 0.559 | 0.773 |
| 100 | 10 | 50 | RBF | 0.001 | 0.560 | 0.496 | 0.566 | 0.774 |
| 100 | 10 | 50 | RBF | 0.01 | 0.032 | 0.071 | 0.506 | 0.468 |
| 100 | 10 | 100 | LIN | - | 0.510 | 0.481 | 0.558 | 0.723 |
| 100 | 10 | 100 | RBF | 0.0001 | 0.523 | 0.485 | 0.559 | 0.773 |
| 100 | 10 | 100 | RBF | 0.001 | 0.560 | 0.496 | 0.566 | 0.774 |
| 100 | 10 | 100 | RBF | 0.01 | 0.029 | 0.067 | 0.505 | 0.468 |
| 100 | 15 | 0.001 | LIN | - | 0.353 | 0.335 | 0.535 | 0.703 |
| 100 | 15 | 0.001 | RBF | 0.0001 | 0.528 | 0.490 | 0.559 | 0.781 |
| 100 | 15 | 0.001 | RBF | 0.001 | 0.554 | 0.494 | 0.562 | 0.773 |
| 100 | 15 | 0.001 | RBF | 0.01 | 0.212 | 0.249 | 0.514 | 0.561 |
| 100 | 15 | 0.01 | RBF | 0.0001 | 0.528 | 0.490 | 0.559 | 0.781 |
| 100 | 15 | 0.01 | RBF | 0.001 | 0.554 | 0.494 | 0.562 | 0.773 |
| 100 | 15 | 0.01 | RBF | 0.01 | 0.188 | 0.220 | 0.512 | 0.517 |
| 100 | 15 | 0.1 | LIN | - | 0.507 | 0.460 | 0.555 | 0.777 |
| 100 | 15 | 0.1 | RBF | 0.0001 | 0.528 | 0.490 | 0.559 | 0.781 |
| 100 | 15 | 0.1 | RBF | 0.001 | 0.554 | 0.494 | 0.562 | 0.773 |
| 100 | 15 | 0.1 | RBF | 0.01 | 0.142 | 0.167 | 0.511 | 0.486 |
| 100 | 15 | 0.2 | LIN | - | 0.539 | 0.503 | 0.554 | 0.779 |
| 100 | 15 | 0.2 | RBF | 0.0001 | 0.528 | 0.490 | 0.559 | 0.781 |
| 100 | 15 | 0.2 | RBF | 0.001 | 0.554 | 0.494 | 0.562 | 0.773 |
| 100 | 15 | 0.2 | RBF | 0.01 | 0.092 | 0.119 | 0.515 | 0.480 |
| 100 | 15 | 0.4 | LIN | - | 0.538 | 0.503 | 0.554 | 0.781 |
| 100 | 15 | 0.4 | RBF | 0.0001 | 0.528 | 0.490 | 0.559 | 0.781 |
| 100 | 15 | 0.4 | RBF | 0.001 | 0.554 | 0.494 | 0.562 | 0.773 |
| 100 | 15 | 0.4 | RBF | 0.01 | 0.080 | 0.112 | 0.510 | 0.476 |
| 100 | 15 | 0.6 | LIN | - | 0.535 | 0.497 | 0.554 | 0.782 |
| 100 | 15 | 0.6 | RBF | 0.0001 | 0.528 | 0.490 | 0.559 | 0.781 |
| 100 | 15 | 0.6 | RBF | 0.001 | 0.554 | 0.494 | 0.562 | 0.773 |
| 100 | 15 | 0.6 | RBF | 0.01 | 0.067 | 0.104 | 0.509 | 0.473 |
| 100 | 15 | 0.8 | LIN | - | 0.533 | 0.504 | 0.551 | 0.782 |
| 100 | 15 | 0.8 | RBF | 0.0001 | 0.528 | 0.490 | 0.559 | 0.781 |
| 100 | 15 | 0.8 | RBF | 0.001 | 0.554 | 0.494 | 0.562 | 0.773 |
| 100 | 15 | 0.8 | RBF | 0.01 | 0.058 | 0.096 | 0.509 | 0.473 |
| 100 | 15 | 1.0 | LIN | - | 0.511 | 0.494 | 0.553 | 0.783 |
| 100 | 15 | 1.0 | RBF | 0.0001 | 0.528 | 0.490 | 0.559 | 0.781 |
| 100 | 15 | 1.0 | RBF | 0.001 | 0.554 | 0.494 | 0.562 | 0.773 |
| 100 | 15 | 1.0 | RBF | 0.01 | 0.044 | 0.079 | 0.507 | 0.472 |
| 100 | 15 | 10 | LIN | - | 0.508 | 0.494 | 0.547 | 0.784 |
| 100 | 15 | 10 | RBF | 0.0001 | 0.528 | 0.490 | 0.559 | 0.781 |
| 100 | 15 | 10 | RBF | 0.001 | 0.554 | 0.494 | 0.562 | 0.773 |
| 100 | 15 | 10 | RBF | 0.01 | 0.030 | 0.068 | 0.506 | 0.469 |
| 100 | 15 | 50 | LIN | - | 0.528 | 0.498 | 0.547 | 0.786 |
| 100 | 15 | 50 | RBF | 0.0001 | 0.528 | 0.490 | 0.559 | 0.781 |
| 100 | 15 | 50 | RBF | 0.001 | 0.554 | 0.494 | 0.562 | 0.773 |
| 100 | 15 | 50 | RBF | 0.01 | 0.031 | 0.069 | 0.506 | 0.468 |
| 100 | 15 | 100 | LIN | - | 0.511 | 0.486 | 0.555 | 0.749 |
| 100 | 15 | 100 | RBF | 0.0001 | 0.528 | 0.490 | 0.559 | 0.781 |
| 100 | 15 | 100 | RBF | 0.001 | 0.554 | 0.494 | 0.562 | 0.773 |
| 100 | 15 | 100 | RBF | 0.01 | 0.034 | 0.072 | 0.505 | 0.468 |
| 150 | 5 | 0.000001 | LIN | - | 0.330 | 0.312 | 0.534 | 0.688 |
| 150 | 5 | 0.000001 | RBF | 0.0001 | 0.460 | 0.444 | 0.543 | 0.728 |
| 150 | 5 | 0.000001 | RBF | 0.001 | 0.481 | 0.431 | 0.548 | 0.729 |
| 150 | 5 | 0.000001 | RBF | 0.01 | 0.277 | 0.280 | 0.529 | 0.605 |
| 150 | 5 | 0.00001 | RBF | 0.001 | 0.534 | 0.496 | 0.565 | 0.758 |
| 150 | 5 | 0.00001 | RBF | 0.01 | 0.249 | 0.273 | 0.524 | 0.608 |
| 150 | 5 | 0.0001 | RBF | 0.0001 | 0.459 | 0.429 | 0.551 | 0.773 |
| 150 | 5 | 0.0001 | RBF | 0.001 | 0.534 | 0.496 | 0.565 | 0.758 |

Continued on next page

TABLE S17 – continued from previous page

| n | $k$ | $\lambda$ | usim | $\sigma$ | AP@5 | AP@10 | sCI | CI |
|---|---|---|---|---|---|---|---|---|
| 150 | 5 | 0.0001 | RBF | 0.01 | 0.250 | 0.272 | 0.522 | 0.573 |
| 150 | 5 | 0.001 | LIN | - | 0.407 | 0.393 | 0.535 | 0.727 |
| 150 | 5 | 0.001 | RBF | 0.0001 | 0.543 | 0.496 | 0.556 | 0.727 |
| 150 | 5 | 0.001 | RBF | 0.001 | 0.534 | 0.496 | 0.565 | 0.758 |
| 150 | 5 | 0.001 | RBF | 0.01 | 0.240 | 0.261 | 0.525 | 0.535 |
| 150 | 5 | 0.01 | LIN | - | 0.484 | 0.458 | 0.548 | 0.750 |
| 150 | 5 | 0.01 | RBF | 0.0001 | 0.543 | 0.496 | 0.556 | 0.727 |
| 150 | 5 | 0.01 | RBF | 0.001 | 0.534 | 0.496 | 0.565 | 0.758 |
| 150 | 5 | 0.01 | RBF | 0.01 | 0.200 | 0.223 | 0.524 | 0.503 |
| 150 | 5 | 0.1 | LIN | - | 0.488 | 0.432 | 0.543 | 0.749 |
| 150 | 5 | 0.1 | RBF | 0.0001 | 0.543 | 0.496 | 0.556 | 0.727 |
| 150 | 5 | 0.1 | RBF | 0.001 | 0.534 | 0.496 | 0.565 | 0.758 |
| 150 | 5 | 0.1 | RBF | 0.01 | 0.135 | 0.158 | 0.519 | 0.482 |
| 150 | 5 | 0.2 | LIN | - | 0.510 | 0.473 | 0.547 | 0.761 |
| 150 | 5 | 0.2 | RBF | 0.0001 | 0.543 | 0.496 | 0.556 | 0.727 |
| 150 | 5 | 0.2 | RBF | 0.001 | 0.534 | 0.496 | 0.565 | 0.758 |
| 150 | 5 | 0.2 | RBF | 0.01 | 0.110 | 0.134 | 0.520 | 0.478 |
| 150 | 5 | 0.4 | LIN | - | 0.519 | 0.466 | 0.546 | 0.759 |
| 150 | 5 | 0.4 | RBF | 0.0001 | 0.543 | 0.496 | 0.556 | 0.727 |
| 150 | 5 | 0.4 | RBF | 0.001 | 0.534 | 0.496 | 0.565 | 0.758 |
| 150 | 5 | 0.4 | RBF | 0.01 | 0.095 | 0.126 | 0.516 | 0.475 |
| 150 | 5 | 0.6 | LIN | - | 0.434 | 0.405 | 0.549 | 0.777 |
| 150 | 5 | 0.6 | RBF | 0.0001 | 0.543 | 0.496 | 0.556 | 0.727 |
| 150 | 5 | 0.6 | RBF | 0.001 | 0.534 | 0.496 | 0.565 | 0.758 |
| 150 | 5 | 0.6 | RBF | 0.01 | 0.088 | 0.119 | 0.516 | 0.473 |
| 150 | 5 | 0.8 | LIN | - | 0.526 | 0.474 | 0.549 | 0.772 |
| 150 | 5 | 0.8 | RBF | 0.0001 | 0.543 | 0.496 | 0.556 | 0.727 |
| 150 | 5 | 0.8 | RBF | 0.001 | 0.534 | 0.496 | 0.565 | 0.758 |
| 150 | 5 | 0.8 | RBF | 0.01 | 0.072 | 0.100 | 0.514 | 0.472 |
| 150 | 5 | 1.0 | LIN | - | 0.523 | 0.475 | 0.550 | 0.776 |
| 150 | 5 | 1.0 | RBF | 0.0001 | 0.543 | 0.496 | 0.556 | 0.727 |
| 150 | 5 | 1.0 | RBF | 0.001 | 0.534 | 0.496 | 0.565 | 0.758 |
| 150 | 5 | 1.0 | RBF | 0.01 | 0.079 | 0.107 | 0.514 | 0.472 |
| 150 | 5 | 10 | LIN | - | 0.537 | 0.504 | 0.543 | 0.779 |
| 150 | 5 | 10 | RBF | 0.0001 | 0.543 | 0.496 | 0.556 | 0.727 |
| 150 | 5 | 10 | RBF | 0.001 | 0.534 | 0.496 | 0.565 | 0.758 |
| 150 | 5 | 10 | RBF | 0.01 | 0.055 | 0.087 | 0.513 | 0.469 |
| 150 | 5 | 50 | LIN | - | 0.521 | 0.497 | 0.558 | 0.748 |
| 150 | 5 | 50 | RBF | 0.0001 | 0.543 | 0.496 | 0.556 | 0.727 |
| 150 | 5 | 50 | RBF | 0.001 | 0.534 | 0.496 | 0.565 | 0.758 |
| 150 | 5 | 50 | RBF | 0.01 | 0.056 | 0.088 | 0.512 | 0.468 |
| 150 | 5 | 100 | LIN | - | 0.513 | 0.478 | 0.555 | 0.683 |
| 150 | 5 | 100 | RBF | 0.0001 | 0.543 | 0.496 | 0.556 | 0.727 |
| 150 | 5 | 100 | RBF | 0.001 | 0.534 | 0.496 | 0.565 | 0.758 |
| 150 | 5 | 100 | RBF | 0.01 | 0.055 | 0.087 | 0.512 | 0.467 |
| 150 | 10 | 0.000001 | LIN | - | 0.367 | 0.341 | 0.526 | 0.700 |
| 150 | 10 | 0.000001 | RBF | 0.01 | 0.292 | 0.285 | 0.526 | 0.598 |
| 150 | 10 | 0.001 | RBF | 0.0001 | 0.542 | 0.500 | 0.557 | 0.771 |
| 150 | 10 | 0.001 | RBF | 0.001 | 0.537 | 0.495 | 0.564 | 0.773 |
| 150 | 10 | 0.001 | RBF | 0.01 | 0.234 | 0.262 | 0.523 | 0.546 |
| 150 | 10 | 0.01 | LIN | - | 0.454 | 0.428 | 0.548 | 0.760 |
| 150 | 10 | 0.01 | RBF | 0.0001 | 0.542 | 0.500 | 0.557 | 0.771 |
| 150 | 10 | 0.01 | RBF | 0.001 | 0.537 | 0.495 | 0.564 | 0.773 |
| 150 | 10 | 0.01 | RBF | 0.01 | 0.195 | 0.217 | 0.522 | 0.508 |
| 150 | 10 | 0.1 | LIN | - | 0.512 | 0.462 | 0.557 | 0.777 |
| 150 | 10 | 0.1 | RBF | 0.0001 | 0.542 | 0.500 | 0.557 | 0.771 |
| 150 | 10 | 0.1 | RBF | 0.001 | 0.537 | 0.495 | 0.564 | 0.773 |
| 150 | 10 | 0.1 | RBF | 0.01 | 0.146 | 0.166 | 0.518 | 0.484 |

Continued on next page

TABLE S17 – continued from previous page

| n | $k$ | $\lambda$ | usim | $\sigma$ | AP@5 | AP@10 | sCI | CI |
|---|---|---|---|---|---|---|---|---|
| 150 | 10 | 0.2 | LIN | - | 0.553 | 0.498 | 0.558 | 0.773 |
| 150 | 10 | 0.2 | RBF | 0.0001 | 0.542 | 0.500 | 0.557 | 0.771 |
| 150 | 10 | 0.2 | RBF | 0.001 | 0.537 | 0.495 | 0.564 | 0.773 |
| 150 | 10 | 0.2 | RBF | 0.01 | 0.109 | 0.129 | 0.519 | 0.480 |
| 150 | 10 | 0.4 | LIN | - | 0.516 | 0.468 | 0.551 | 0.777 |
| 150 | 10 | 0.4 | RBF | 0.0001 | 0.542 | 0.500 | 0.557 | 0.771 |
| 150 | 10 | 0.4 | RBF | 0.001 | 0.537 | 0.495 | 0.564 | 0.773 |
| 150 | 10 | 0.4 | RBF | 0.01 | 0.102 | 0.131 | 0.517 | 0.476 |
| 150 | 10 | 0.6 | LIN | - | 0.518 | 0.485 | 0.553 | 0.777 |
| 150 | 10 | 0.6 | RBF | 0.0001 | 0.542 | 0.500 | 0.557 | 0.771 |
| 150 | 10 | 0.6 | RBF | 0.001 | 0.537 | 0.495 | 0.564 | 0.773 |
| 150 | 10 | 0.6 | RBF | 0.01 | 0.085 | 0.116 | 0.516 | 0.474 |
| 150 | 10 | 0.8 | LIN | - | 0.529 | 0.508 | 0.549 | 0.778 |
| 150 | 10 | 0.8 | RBF | 0.0001 | 0.542 | 0.500 | 0.557 | 0.771 |
| 150 | 10 | 0.8 | RBF | 0.001 | 0.537 | 0.495 | 0.564 | 0.773 |
| 150 | 10 | 0.8 | RBF | 0.01 | 0.070 | 0.102 | 0.515 | 0.473 |
| 150 | 10 | 1.0 | LIN | - | 0.565 | 0.524 | 0.550 | 0.782 |
| 150 | 10 | 1.0 | RBF | 0.0001 | 0.542 | 0.500 | 0.557 | 0.771 |
| 150 | 10 | 1.0 | RBF | 0.001 | 0.537 | 0.495 | 0.564 | 0.773 |
| 150 | 10 | 1.0 | RBF | 0.01 | 0.071 | 0.101 | 0.513 | 0.472 |
| 150 | 10 | 10 | LIN | - | 0.527 | 0.501 | 0.546 | 0.779 |
| 150 | 10 | 10 | RBF | 0.0001 | 0.542 | 0.500 | 0.557 | 0.771 |
| 150 | 10 | 10 | RBF | 0.001 | 0.537 | 0.495 | 0.564 | 0.773 |
| 150 | 10 | 10 | RBF | 0.01 | 0.058 | 0.091 | 0.513 | 0.469 |
| 150 | 10 | 50 | LIN | - | 0.511 | 0.493 | 0.555 | 0.764 |
| 150 | 10 | 50 | RBF | 0.0001 | 0.542 | 0.500 | 0.557 | 0.771 |
| 150 | 10 | 50 | RBF | 0.001 | 0.537 | 0.495 | 0.564 | 0.773 |
| 150 | 10 | 50 | RBF | 0.01 | 0.057 | 0.089 | 0.512 | 0.468 |
| 150 | 10 | 100 | LIN | - | 0.529 | 0.487 | 0.555 | 0.695 |
| 150 | 10 | 100 | RBF | 0.0001 | 0.542 | 0.500 | 0.557 | 0.771 |
| 150 | 10 | 100 | RBF | 0.001 | 0.537 | 0.495 | 0.564 | 0.773 |
| 150 | 10 | 100 | RBF | 0.01 | 0.056 | 0.088 | 0.512 | 0.467 |
| 150 | 15 | 0.001 | LIN | - | 0.398 | 0.407 | 0.547 | 0.719 |
| 150 | 15 | 0.001 | RBF | 0.0001 | 0.538 | 0.492 | 0.557 | 0.779 |
| 150 | 15 | 0.001 | RBF | 0.001 | 0.539 | 0.493 | 0.561 | 0.772 |
| 150 | 15 | 0.001 | RBF | 0.01 | 0.259 | 0.278 | 0.522 | 0.549 |
| 150 | 15 | 0.01 | LIN | - | 0.444 | 0.416 | 0.556 | 0.764 |
| 150 | 15 | 0.01 | RBF | 0.0001 | 0.538 | 0.492 | 0.557 | 0.779 |
| 150 | 15 | 0.01 | RBF | 0.001 | 0.539 | 0.493 | 0.561 | 0.772 |
| 150 | 15 | 0.01 | RBF | 0.01 | 0.201 | 0.218 | 0.521 | 0.510 |
| 150 | 15 | 0.1 | LIN | - | 0.550 | 0.498 | 0.559 | 0.776 |
| 150 | 15 | 0.1 | RBF | 0.0001 | 0.538 | 0.492 | 0.557 | 0.779 |
| 150 | 15 | 0.1 | RBF | 0.001 | 0.539 | 0.493 | 0.561 | 0.772 |
| 150 | 15 | 0.1 | RBF | 0.01 | 0.147 | 0.164 | 0.518 | 0.485 |
| 150 | 15 | 0.2 | LIN | - | 0.540 | 0.505 | 0.556 | 0.777 |
| 150 | 15 | 0.2 | RBF | 0.0001 | 0.538 | 0.492 | 0.557 | 0.779 |
| 150 | 15 | 0.2 | RBF | 0.001 | 0.539 | 0.493 | 0.561 | 0.772 |
| 150 | 15 | 0.2 | RBF | 0.01 | 0.116 | 0.139 | 0.519 | 0.480 |
| 150 | 15 | 0.4 | LIN | - | 0.540 | 0.509 | 0.556 | 0.777 |
| 150 | 15 | 0.4 | RBF | 0.0001 | 0.538 | 0.492 | 0.557 | 0.779 |
| 150 | 15 | 0.4 | RBF | 0.001 | 0.539 | 0.493 | 0.561 | 0.772 |
| 150 | 15 | 0.4 | RBF | 0.01 | 0.108 | 0.134 | 0.516 | 0.476 |
| 150 | 15 | 0.6 | LIN | - | 0.544 | 0.508 | 0.554 | 0.780 |
| 150 | 15 | 0.6 | RBF | 0.0001 | 0.538 | 0.492 | 0.557 | 0.779 |
| 150 | 15 | 0.6 | RBF | 0.001 | 0.539 | 0.493 | 0.561 | 0.772 |
| 150 | 15 | 0.6 | RBF | 0.01 | 0.087 | 0.119 | 0.516 | 0.474 |
| 150 | 15 | 0.8 | LIN | - | 0.558 | 0.522 | 0.553 | 0.781 |
| 150 | 15 | 0.8 | RBF | 0.0001 | 0.538 | 0.492 | 0.557 | 0.779 |

Continued on next page

TABLE S17 – continued from previous page

| n | $k$ | $\lambda$ | usim | $\sigma$ | AP@5 | AP@10 | sCI | CI |
|---|---|---|---|---|---|---|---|---|
| 150 | 15 | 0.8 | RBF | 0.001 | 0.539 | 0.493 | 0.561 | 0.772 |
| 150 | 15 | 0.8 | RBF | 0.01 | 0.078 | 0.108 | 0.515 | 0.473 |
| 150 | 15 | 1.0 | LIN | - | 0.544 | 0.506 | 0.555 | 0.782 |
| 150 | 15 | 1.0 | RBF | 0.0001 | 0.538 | 0.492 | 0.557 | 0.779 |
| 150 | 15 | 1.0 | RBF | 0.001 | 0.539 | 0.493 | 0.561 | 0.772 |
| 150 | 15 | 1.0 | RBF | 0.01 | 0.073 | 0.101 | 0.514 | 0.473 |
| 150 | 15 | 10 | LIN | - | 0.530 | 0.485 | 0.549 | 0.783 |
| 150 | 15 | 10 | RBF | 0.0001 | 0.538 | 0.492 | 0.557 | 0.779 |
| 150 | 15 | 10 | RBF | 0.001 | 0.539 | 0.493 | 0.561 | 0.772 |
| 150 | 15 | 10 | RBF | 0.01 | 0.058 | 0.091 | 0.513 | 0.469 |
| 150 | 15 | 50 | LIN | - | 0.521 | 0.494 | 0.553 | 0.770 |
| 150 | 15 | 50 | RBF | 0.0001 | 0.538 | 0.492 | 0.557 | 0.779 |
| 150 | 15 | 50 | RBF | 0.001 | 0.539 | 0.493 | 0.561 | 0.772 |
| 150 | 15 | 50 | RBF | 0.01 | 0.055 | 0.087 | 0.512 | 0.468 |
| 150 | 15 | 100 | LIN | - | 0.525 | 0.486 | 0.553 | 0.730 |
| 150 | 15 | 100 | RBF | 0.0001 | 0.538 | 0.492 | 0.557 | 0.779 |
| 150 | 15 | 100 | RBF | 0.001 | 0.539 | 0.493 | 0.561 | 0.772 |
| 150 | 15 | 100 | RBF | 0.01 | 0.058 | 0.089 | 0.512 | 0.468 |
| 200 | 5 | 0.000001 | LIN | - | 0.322 | 0.328 | 0.521 | 0.703 |
| 200 | 5 | 0.000001 | RBF | 0.0001 | 0.490 | 0.458 | 0.532 | 0.729 |
| 200 | 5 | 0.000001 | RBF | 0.001 | 0.464 | 0.445 | 0.546 | 0.728 |
| 200 | 5 | 0.000001 | RBF | 0.01 | 0.299 | 0.300 | 0.528 | 0.597 |
| 200 | 5 | 0.00001 | RBF | 0.001 | 0.520 | 0.488 | 0.557 | 0.756 |
| 200 | 5 | 0.00001 | RBF | 0.01 | 0.271 | 0.295 | 0.524 | 0.596 |
| 200 | 5 | 0.0001 | RBF | 0.0001 | 0.515 | 0.475 | 0.550 | 0.774 |
| 200 | 5 | 0.0001 | RBF | 0.001 | 0.520 | 0.488 | 0.557 | 0.756 |
| 200 | 5 | 0.0001 | RBF | 0.01 | 0.262 | 0.284 | 0.526 | 0.564 |
| 200 | 5 | 0.001 | LIN | - | 0.440 | 0.420 | 0.535 | 0.722 |
| 200 | 5 | 0.001 | RBF | 0.0001 | 0.528 | 0.495 | 0.551 | 0.729 |
| 200 | 5 | 0.001 | RBF | 0.001 | 0.520 | 0.488 | 0.557 | 0.756 |
| 200 | 5 | 0.001 | RBF | 0.01 | 0.241 | 0.261 | 0.527 | 0.530 |
| 200 | 5 | 0.01 | LIN | - | 0.469 | 0.457 | 0.542 | 0.746 |
| 200 | 5 | 0.01 | RBF | 0.0001 | 0.528 | 0.495 | 0.551 | 0.729 |
| 200 | 5 | 0.01 | RBF | 0.001 | 0.520 | 0.488 | 0.557 | 0.756 |
| 200 | 5 | 0.01 | RBF | 0.01 | 0.185 | 0.206 | 0.522 | 0.500 |
| 200 | 5 | 0.1 | LIN | - | 0.487 | 0.466 | 0.544 | 0.756 |
| 200 | 5 | 0.1 | RBF | 0.0001 | 0.528 | 0.495 | 0.551 | 0.729 |
| 200 | 5 | 0.1 | RBF | 0.001 | 0.520 | 0.488 | 0.557 | 0.756 |
| 200 | 5 | 0.1 | RBF | 0.01 | 0.124 | 0.149 | 0.521 | 0.481 |
| 200 | 5 | 0.2 | LIN | - | 0.520 | 0.463 | 0.543 | 0.769 |
| 200 | 5 | 0.2 | RBF | 0.0001 | 0.528 | 0.495 | 0.551 | 0.729 |
| 200 | 5 | 0.2 | RBF | 0.001 | 0.520 | 0.488 | 0.557 | 0.756 |
| 200 | 5 | 0.2 | RBF | 0.01 | 0.106 | 0.135 | 0.518 | 0.477 |
| 200 | 5 | 0.4 | LIN | - | 0.499 | 0.475 | 0.546 | 0.767 |
| 200 | 5 | 0.4 | RBF | 0.0001 | 0.528 | 0.495 | 0.551 | 0.729 |
| 200 | 5 | 0.4 | RBF | 0.001 | 0.520 | 0.488 | 0.557 | 0.756 |
| 200 | 5 | 0.4 | RBF | 0.01 | 0.094 | 0.126 | 0.516 | 0.475 |
| 200 | 5 | 0.6 | LIN | - | 0.530 | 0.487 | 0.544 | 0.754 |
| 200 | 5 | 0.6 | RBF | 0.0001 | 0.528 | 0.495 | 0.551 | 0.729 |
| 200 | 5 | 0.6 | RBF | 0.001 | 0.520 | 0.488 | 0.557 | 0.756 |
| 200 | 5 | 0.6 | RBF | 0.01 | 0.075 | 0.108 | 0.516 | 0.473 |
| 200 | 5 | 0.8 | LIN | - | 0.497 | 0.460 | 0.547 | 0.761 |
| 200 | 5 | 0.8 | RBF | 0.0001 | 0.528 | 0.495 | 0.551 | 0.729 |
| 200 | 5 | 0.8 | RBF | 0.001 | 0.520 | 0.488 | 0.557 | 0.756 |
| 200 | 5 | 0.8 | RBF | 0.01 | 0.079 | 0.110 | 0.514 | 0.472 |
| 200 | 5 | 1.0 | LIN | - | 0.518 | 0.472 | 0.543 | 0.757 |
| 200 | 5 | 1.0 | RBF | 0.0001 | 0.528 | 0.495 | 0.551 | 0.729 |
| 200 | 5 | 1.0 | RBF | 0.001 | 0.520 | 0.488 | 0.557 | 0.756 |

Continued on next page

TABLE S17 – continued from previous page

| n | $k$ | $\lambda$ | usim | $\sigma$ | AP@5 | AP@10 | sCI | CI |
|---|---|---|---|---|---|---|---|---|
| 200 | 5 | 1.0 | RBF | 0.01 | 0.068 | 0.100 | 0.514 | 0.472 |
| 200 | 5 | 10 | LIN | - | 0.533 | 0.500 | 0.543 | 0.779 |
| 200 | 5 | 10 | RBF | 0.0001 | 0.528 | 0.495 | 0.551 | 0.729 |
| 200 | 5 | 10 | RBF | 0.001 | 0.520 | 0.488 | 0.557 | 0.756 |
| 200 | 5 | 10 | RBF | 0.01 | 0.055 | 0.088 | 0.514 | 0.469 |
| 200 | 5 | 50 | LIN | - | 0.533 | 0.505 | 0.554 | 0.744 |
| 200 | 5 | 50 | RBF | 0.0001 | 0.528 | 0.495 | 0.551 | 0.729 |
| 200 | 5 | 50 | RBF | 0.001 | 0.520 | 0.487 | 0.557 | 0.756 |
| 200 | 5 | 50 | RBF | 0.01 | 0.051 | 0.084 | 0.513 | 0.468 |
| 200 | 5 | 100 | LIN | - | 0.529 | 0.491 | 0.550 | 0.668 |
| 200 | 5 | 100 | RBF | 0.0001 | 0.528 | 0.495 | 0.551 | 0.729 |
| 200 | 5 | 100 | RBF | 0.001 | 0.520 | 0.487 | 0.557 | 0.756 |
| 200 | 5 | 100 | RBF | 0.01 | 0.055 | 0.088 | 0.513 | 0.468 |
| 200 | 10 | 0.000001 | LIN | - | 0.233 | 0.249 | 0.518 | 0.703 |
| 200 | 10 | 0.000001 | RBF | 0.01 | 0.297 | 0.299 | 0.526 | 0.590 |
| 200 | 10 | 0.001 | RBF | 0.0001 | 0.533 | 0.495 | 0.552 | 0.769 |
| 200 | 10 | 0.001 | RBF | 0.001 | 0.522 | 0.493 | 0.556 | 0.770 |
| 200 | 10 | 0.001 | RBF | 0.01 | 0.233 | 0.254 | 0.522 | 0.539 |
| 200 | 10 | 0.01 | LIN | - | 0.439 | 0.418 | 0.543 | 0.764 |
| 200 | 10 | 0.01 | RBF | 0.0001 | 0.533 | 0.495 | 0.552 | 0.769 |
| 200 | 10 | 0.01 | RBF | 0.001 | 0.522 | 0.493 | 0.556 | 0.770 |
| 200 | 10 | 0.01 | RBF | 0.01 | 0.194 | 0.211 | 0.521 | 0.506 |
| 200 | 10 | 0.1 | LIN | - | 0.500 | 0.471 | 0.548 | 0.773 |
| 200 | 10 | 0.1 | RBF | 0.0001 | 0.533 | 0.495 | 0.552 | 0.769 |
| 200 | 10 | 0.1 | RBF | 0.001 | 0.522 | 0.493 | 0.556 | 0.770 |
| 200 | 10 | 0.1 | RBF | 0.01 | 0.127 | 0.151 | 0.519 | 0.483 |
| 200 | 10 | 0.2 | LIN | - | 0.523 | 0.486 | 0.554 | 0.773 |
| 200 | 10 | 0.2 | RBF | 0.0001 | 0.533 | 0.495 | 0.552 | 0.769 |
| 200 | 10 | 0.2 | RBF | 0.001 | 0.522 | 0.493 | 0.556 | 0.770 |
| 200 | 10 | 0.2 | RBF | 0.01 | 0.115 | 0.141 | 0.518 | 0.479 |
| 200 | 10 | 0.4 | LIN | - | 0.502 | 0.473 | 0.548 | 0.782 |
| 200 | 10 | 0.4 | RBF | 0.0001 | 0.533 | 0.495 | 0.552 | 0.769 |
| 200 | 10 | 0.4 | RBF | 0.001 | 0.522 | 0.493 | 0.556 | 0.770 |
| 200 | 10 | 0.4 | RBF | 0.01 | 0.095 | 0.127 | 0.516 | 0.476 |
| 200 | 10 | 0.6 | LIN | - | 0.484 | 0.458 | 0.547 | 0.779 |
| 200 | 10 | 0.6 | RBF | 0.0001 | 0.533 | 0.495 | 0.552 | 0.769 |
| 200 | 10 | 0.6 | RBF | 0.001 | 0.522 | 0.493 | 0.556 | 0.770 |
| 200 | 10 | 0.6 | RBF | 0.01 | 0.079 | 0.109 | 0.515 | 0.474 |
| 200 | 10 | 0.8 | LIN | - | 0.495 | 0.474 | 0.548 | 0.783 |
| 200 | 10 | 0.8 | RBF | 0.0001 | 0.533 | 0.495 | 0.552 | 0.769 |
| 200 | 10 | 0.8 | RBF | 0.001 | 0.522 | 0.493 | 0.556 | 0.770 |
| 200 | 10 | 0.8 | RBF | 0.01 | 0.078 | 0.110 | 0.515 | 0.473 |
| 200 | 10 | 1.0 | LIN | - | 0.514 | 0.488 | 0.547 | 0.781 |
| 200 | 10 | 1.0 | RBF | 0.0001 | 0.533 | 0.495 | 0.552 | 0.769 |
| 200 | 10 | 1.0 | RBF | 0.001 | 0.522 | 0.493 | 0.556 | 0.770 |
| 200 | 10 | 1.0 | RBF | 0.01 | 0.070 | 0.099 | 0.515 | 0.473 |
| 200 | 10 | 10 | LIN | - | 0.536 | 0.503 | 0.546 | 0.762 |
| 200 | 10 | 10 | RBF | 0.0001 | 0.533 | 0.495 | 0.552 | 0.769 |
| 200 | 10 | 10 | RBF | 0.001 | 0.522 | 0.493 | 0.556 | 0.770 |
| 200 | 10 | 10 | RBF | 0.01 | 0.055 | 0.088 | 0.514 | 0.469 |
| 200 | 10 | 50 | LIN | - | 0.542 | 0.511 | 0.551 | 0.760 |
| 200 | 10 | 50 | RBF | 0.0001 | 0.533 | 0.495 | 0.552 | 0.769 |
| 200 | 10 | 50 | RBF | 0.001 | 0.522 | 0.493 | 0.556 | 0.770 |
| 200 | 10 | 50 | RBF | 0.01 | 0.052 | 0.086 | 0.513 | 0.468 |
| 200 | 10 | 100 | LIN | - | 0.529 | 0.491 | 0.550 | 0.686 |
| 200 | 10 | 100 | RBF | 0.0001 | 0.533 | 0.495 | 0.552 | 0.769 |
| 200 | 10 | 100 | RBF | 0.001 | 0.522 | 0.493 | 0.556 | 0.770 |
| 200 | 10 | 100 | RBF | 0.01 | 0.056 | 0.088 | 0.513 | 0.468 |

Continued on next page

TABLE S17 – continued from previous page

| n | $k$ | $\lambda$ | usim | $\sigma$ | AP@5 | AP@10 | sCI | CI |
|---|---|---|---|---|---|---|---|---|
| 200 | 15 | 0.001 | LIN | - | 0.373 | 0.361 | 0.532 | 0.703 |
| 200 | 15 | 0.001 | RBF | 0.0001 | 0.537 | 0.496 | 0.552 | 0.777 |
| 200 | 15 | 0.001 | RBF | 0.001 | 0.540 | 0.506 | 0.554 | 0.770 |
| 200 | 15 | 0.001 | RBF | 0.01 | 0.240 | 0.259 | 0.522 | 0.543 |
| 200 | 15 | 0.01 | RBF | 0.0001 | 0.537 | 0.496 | 0.552 | 0.777 |
| 200 | 15 | 0.01 | RBF | 0.001 | 0.540 | 0.506 | 0.554 | 0.770 |
| 200 | 15 | 0.01 | RBF | 0.01 | 0.188 | 0.206 | 0.520 | 0.508 |
| 200 | 15 | 0.1 | LIN | - | 0.505 | 0.478 | 0.553 | 0.775 |
| 200 | 15 | 0.1 | RBF | 0.0001 | 0.537 | 0.496 | 0.552 | 0.777 |
| 200 | 15 | 0.1 | RBF | 0.001 | 0.540 | 0.506 | 0.554 | 0.770 |
| 200 | 15 | 0.1 | RBF | 0.01 | 0.129 | 0.157 | 0.518 | 0.485 |
| 200 | 15 | 0.2 | LIN | - | 0.534 | 0.503 | 0.553 | 0.775 |
| 200 | 15 | 0.2 | RBF | 0.0001 | 0.537 | 0.496 | 0.552 | 0.777 |
| 200 | 15 | 0.2 | RBF | 0.001 | 0.540 | 0.506 | 0.554 | 0.770 |
| 200 | 15 | 0.2 | RBF | 0.01 | 0.115 | 0.140 | 0.519 | 0.480 |
| 200 | 15 | 0.4 | LIN | - | 0.515 | 0.494 | 0.553 | 0.777 |
| 200 | 15 | 0.4 | RBF | 0.0001 | 0.537 | 0.496 | 0.552 | 0.777 |
| 200 | 15 | 0.4 | RBF | 0.001 | 0.540 | 0.506 | 0.554 | 0.770 |
| 200 | 15 | 0.4 | RBF | 0.01 | 0.103 | 0.130 | 0.516 | 0.477 |
| 200 | 15 | 0.6 | LIN | - | 0.527 | 0.507 | 0.553 | 0.779 |
| 200 | 15 | 0.6 | RBF | 0.0001 | 0.537 | 0.496 | 0.552 | 0.777 |
| 200 | 15 | 0.6 | RBF | 0.001 | 0.540 | 0.506 | 0.554 | 0.770 |
| 200 | 15 | 0.6 | RBF | 0.01 | 0.084 | 0.113 | 0.515 | 0.475 |
| 200 | 15 | 0.8 | LIN | - | 0.511 | 0.489 | 0.552 | 0.780 |
| 200 | 15 | 0.8 | RBF | 0.0001 | 0.537 | 0.496 | 0.552 | 0.777 |
| 200 | 15 | 0.8 | RBF | 0.001 | 0.540 | 0.506 | 0.554 | 0.770 |
| 200 | 15 | 0.8 | RBF | 0.01 | 0.079 | 0.110 | 0.515 | 0.474 |
| 200 | 15 | 1.0 | LIN | - | 0.545 | 0.501 | 0.553 | 0.780 |
| 200 | 15 | 1.0 | RBF | 0.0001 | 0.537 | 0.496 | 0.552 | 0.777 |
| 200 | 15 | 1.0 | RBF | 0.001 | 0.540 | 0.506 | 0.554 | 0.770 |
| 200 | 15 | 1.0 | RBF | 0.01 | 0.074 | 0.102 | 0.514 | 0.473 |
| 200 | 15 | 10 | LIN | - | 0.536 | 0.514 | 0.548 | 0.785 |
| 200 | 15 | 10 | RBF | 0.0001 | 0.537 | 0.496 | 0.552 | 0.777 |
| 200 | 15 | 10 | RBF | 0.001 | 0.540 | 0.506 | 0.554 | 0.770 |
| 200 | 15 | 10 | RBF | 0.01 | 0.057 | 0.089 | 0.514 | 0.470 |
| 200 | 15 | 50 | LIN | - | 0.535 | 0.514 | 0.550 | 0.768 |
| 200 | 15 | 50 | RBF | 0.0001 | 0.537 | 0.496 | 0.552 | 0.777 |
| 200 | 15 | 50 | RBF | 0.001 | 0.540 | 0.506 | 0.554 | 0.770 |
| 200 | 15 | 50 | RBF | 0.01 | 0.052 | 0.086 | 0.513 | 0.468 |
| 200 | 15 | 100 | LIN | - | 0.528 | 0.492 | 0.550 | 0.724 |
| 200 | 15 | 100 | RBF | 0.0001 | 0.537 | 0.496 | 0.552 | 0.777 |
| 200 | 15 | 100 | RBF | 0.001 | 0.540 | 0.506 | 0.554 | 0.770 |
| 200 | 15 | 100 | RBF | 0.01 | 0.062 | 0.093 | 0.513 | 0.468 |
| 250 | 5 | 0.000001 | RBF | 0.0001 | 0.473 | 0.442 | 0.538 | 0.728 |
| 250 | 5 | 0.000001 | RBF | 0.001 | 0.499 | 0.467 | 0.549 | 0.722 |
| 250 | 5 | 0.000001 | RBF | 0.01 | 0.317 | 0.320 | 0.525 | 0.590 |
| 250 | 5 | 0.00001 | LIN | - | 0.195 | 0.231 | 0.538 | 0.671 |
| 250 | 5 | 0.00001 | RBF | 0.0001 | 0.523 | 0.489 | 0.535 | 0.757 |
| 250 | 5 | 0.00001 | RBF | 0.001 | 0.553 | 0.516 | 0.560 | 0.758 |
| 250 | 5 | 0.00001 | RBF | 0.01 | 0.294 | 0.302 | 0.527 | 0.587 |
| 250 | 5 | 0.0001 | RBF | 0.0001 | 0.513 | 0.467 | 0.550 | 0.775 |
| 250 | 5 | 0.0001 | RBF | 0.001 | 0.553 | 0.516 | 0.560 | 0.758 |
| 250 | 5 | 0.0001 | RBF | 0.01 | 0.269 | 0.277 | 0.523 | 0.556 |
| 250 | 5 | 0.001 | LIN | - | 0.393 | 0.380 | 0.542 | 0.723 |
| 250 | 5 | 0.001 | RBF | 0.0001 | 0.536 | 0.501 | 0.552 | 0.730 |
| 250 | 5 | 0.001 | RBF | 0.001 | 0.553 | 0.516 | 0.560 | 0.758 |
| 250 | 5 | 0.001 | RBF | 0.01 | 0.241 | 0.254 | 0.520 | 0.525 |
| 250 | 5 | 0.01 | LIN | - | 0.493 | 0.466 | 0.549 | 0.749 |

Continued on next page

TABLE S17 – continued from previous page

| n | $k$ | $\lambda$ | usim | $\sigma$ | AP@5 | AP@10 | sCI | CI |
|---|---|---|---|---|---|---|---|---|
| 250 | 5 | 0.01 | RBF | 0.0001 | 0.536 | 0.501 | 0.552 | 0.730 |
| 250 | 5 | 0.01 | RBF | 0.001 | 0.553 | 0.516 | 0.560 | 0.758 |
| 250 | 5 | 0.01 | RBF | 0.01 | 0.180 | 0.201 | 0.517 | 0.498 |
| 250 | 5 | 0.1 | LIN | - | 0.475 | 0.447 | 0.541 | 0.764 |
| 250 | 5 | 0.1 | RBF | 0.0001 | 0.536 | 0.501 | 0.552 | 0.730 |
| 250 | 5 | 0.1 | RBF | 0.001 | 0.553 | 0.516 | 0.560 | 0.758 |
| 250 | 5 | 0.1 | RBF | 0.01 | 0.138 | 0.163 | 0.516 | 0.482 |
| 250 | 5 | 0.2 | LIN | - | 0.460 | 0.431 | 0.546 | 0.771 |
| 250 | 5 | 0.2 | RBF | 0.0001 | 0.536 | 0.501 | 0.552 | 0.730 |
| 250 | 5 | 0.2 | RBF | 0.001 | 0.553 | 0.516 | 0.560 | 0.758 |
| 250 | 5 | 0.2 | RBF | 0.01 | 0.114 | 0.140 | 0.514 | 0.479 |
| 250 | 5 | 0.4 | LIN | - | 0.512 | 0.472 | 0.545 | 0.772 |
| 250 | 5 | 0.4 | RBF | 0.0001 | 0.536 | 0.501 | 0.552 | 0.730 |
| 250 | 5 | 0.4 | RBF | 0.001 | 0.553 | 0.516 | 0.560 | 0.758 |
| 250 | 5 | 0.4 | RBF | 0.01 | 0.106 | 0.134 | 0.513 | 0.475 |
| 250 | 5 | 0.6 | LIN | - | 0.518 | 0.484 | 0.543 | 0.767 |
| 250 | 5 | 0.6 | RBF | 0.0001 | 0.536 | 0.501 | 0.552 | 0.730 |
| 250 | 5 | 0.6 | RBF | 0.001 | 0.553 | 0.516 | 0.560 | 0.758 |
| 250 | 5 | 0.6 | RBF | 0.01 | 0.092 | 0.122 | 0.512 | 0.474 |
| 250 | 5 | 0.8 | LIN | - | 0.514 | 0.472 | 0.549 | 0.766 |
| 250 | 5 | 0.8 | RBF | 0.0001 | 0.536 | 0.501 | 0.552 | 0.730 |
| 250 | 5 | 0.8 | RBF | 0.001 | 0.553 | 0.516 | 0.560 | 0.758 |
| 250 | 5 | 0.8 | RBF | 0.01 | 0.078 | 0.111 | 0.512 | 0.473 |
| 250 | 5 | 1.0 | LIN | - | 0.506 | 0.475 | 0.547 | 0.760 |
| 250 | 5 | 1.0 | RBF | 0.0001 | 0.536 | 0.501 | 0.552 | 0.730 |
| 250 | 5 | 1.0 | RBF | 0.001 | 0.553 | 0.516 | 0.560 | 0.758 |
| 250 | 5 | 1.0 | RBF | 0.01 | 0.080 | 0.110 | 0.511 | 0.473 |
| 250 | 5 | 10 | LIN | - | 0.561 | 0.520 | 0.547 | 0.777 |
| 250 | 5 | 10 | RBF | 0.0001 | 0.536 | 0.501 | 0.552 | 0.730 |
| 250 | 5 | 10 | RBF | 0.001 | 0.553 | 0.516 | 0.560 | 0.758 |
| 250 | 5 | 10 | RBF | 0.01 | 0.058 | 0.092 | 0.510 | 0.470 |
| 250 | 5 | 50 | LIN | - | 0.534 | 0.502 | 0.554 | 0.737 |
| 250 | 5 | 50 | RBF | 0.0001 | 0.536 | 0.501 | 0.552 | 0.730 |
| 250 | 5 | 50 | RBF | 0.001 | 0.553 | 0.516 | 0.560 | 0.758 |
| 250 | 5 | 50 | RBF | 0.01 | 0.051 | 0.086 | 0.509 | 0.469 |
| 250 | 5 | 100 | LIN | - | 0.527 | 0.493 | 0.552 | 0.656 |
| 250 | 5 | 100 | RBF | 0.0001 | 0.536 | 0.501 | 0.552 | 0.730 |
| 250 | 5 | 100 | RBF | 0.001 | 0.553 | 0.516 | 0.560 | 0.758 |
| 250 | 5 | 100 | RBF | 0.01 | 0.045 | 0.079 | 0.510 | 0.469 |
| 250 | 10 | 0.000001 | LIN | - | 0.334 | 0.325 | 0.516 | 0.685 |
| 250 | 10 | 0.000001 | RBF | 0.01 | 0.311 | 0.317 | 0.525 | 0.583 |
| 250 | 10 | 0.001 | LIN | - | 0.371 | 0.365 | 0.544 | 0.719 |
| 250 | 10 | 0.001 | RBF | 0.0001 | 0.537 | 0.506 | 0.554 | 0.769 |
| 250 | 10 | 0.001 | RBF | 0.001 | 0.554 | 0.514 | 0.557 | 0.770 |
| 250 | 10 | 0.001 | RBF | 0.01 | 0.238 | 0.253 | 0.521 | 0.533 |
| 250 | 10 | 0.01 | LIN | - | 0.419 | 0.397 | 0.546 | 0.762 |
| 250 | 10 | 0.01 | RBF | 0.0001 | 0.537 | 0.506 | 0.554 | 0.769 |
| 250 | 10 | 0.01 | RBF | 0.001 | 0.554 | 0.514 | 0.557 | 0.770 |
| 250 | 10 | 0.01 | RBF | 0.01 | 0.177 | 0.197 | 0.518 | 0.503 |
| 250 | 10 | 0.1 | LIN | - | 0.519 | 0.474 | 0.551 | 0.777 |
| 250 | 10 | 0.1 | RBF | 0.0001 | 0.537 | 0.506 | 0.554 | 0.769 |
| 250 | 10 | 0.1 | RBF | 0.001 | 0.554 | 0.514 | 0.557 | 0.770 |
| 250 | 10 | 0.1 | RBF | 0.01 | 0.148 | 0.170 | 0.515 | 0.485 |
| 250 | 10 | 0.2 | LIN | - | 0.481 | 0.442 | 0.553 | 0.778 |
| 250 | 10 | 0.2 | RBF | 0.0001 | 0.537 | 0.506 | 0.554 | 0.769 |
| 250 | 10 | 0.2 | RBF | 0.001 | 0.554 | 0.514 | 0.557 | 0.770 |
| 250 | 10 | 0.2 | RBF | 0.01 | 0.122 | 0.149 | 0.515 | 0.481 |
| 250 | 10 | 0.4 | LIN | - | 0.562 | 0.505 | 0.552 | 0.778 |

Continued on next page

TABLE S17 – continued from previous page

| n | $k$ | $\lambda$ | usim | $\sigma$ | AP@5 | AP@10 | sCI | CI |
|---|---|---|---|---|---|---|---|---|
| 250 | 10 | 0.4 | RBF | 0.0001 | 0.537 | 0.506 | 0.554 | 0.769 |
| 250 | 10 | 0.4 | RBF | 0.001 | 0.554 | 0.514 | 0.557 | 0.770 |
| 250 | 10 | 0.4 | RBF | 0.01 | 0.104 | 0.133 | 0.513 | 0.477 |
| 250 | 10 | 0.6 | LIN | - | 0.497 | 0.456 | 0.554 | 0.780 |
| 250 | 10 | 0.6 | RBF | 0.0001 | 0.537 | 0.506 | 0.554 | 0.769 |
| 250 | 10 | 0.6 | RBF | 0.001 | 0.554 | 0.514 | 0.557 | 0.770 |
| 250 | 10 | 0.6 | RBF | 0.01 | 0.095 | 0.122 | 0.512 | 0.475 |
| 250 | 10 | 0.8 | LIN | - | 0.511 | 0.486 | 0.553 | 0.782 |
| 250 | 10 | 0.8 | RBF | 0.0001 | 0.537 | 0.506 | 0.554 | 0.769 |
| 250 | 10 | 0.8 | RBF | 0.001 | 0.554 | 0.514 | 0.557 | 0.770 |
| 250 | 10 | 0.8 | RBF | 0.01 | 0.091 | 0.119 | 0.512 | 0.474 |
| 250 | 10 | 1.0 | LIN | - | 0.547 | 0.484 | 0.550 | 0.779 |
| 250 | 10 | 1.0 | RBF | 0.0001 | 0.537 | 0.506 | 0.554 | 0.769 |
| 250 | 10 | 1.0 | RBF | 0.001 | 0.554 | 0.514 | 0.557 | 0.770 |
| 250 | 10 | 1.0 | RBF | 0.01 | 0.075 | 0.108 | 0.512 | 0.474 |
| 250 | 10 | 10 | LIN | - | 0.560 | 0.537 | 0.548 | 0.784 |
| 250 | 10 | 10 | RBF | 0.0001 | 0.537 | 0.506 | 0.554 | 0.769 |
| 250 | 10 | 10 | RBF | 0.001 | 0.554 | 0.514 | 0.557 | 0.770 |
| 250 | 10 | 10 | RBF | 0.01 | 0.058 | 0.092 | 0.510 | 0.470 |
| 250 | 10 | 50 | LIN | - | 0.537 | 0.508 | 0.552 | 0.753 |
| 250 | 10 | 50 | RBF | 0.0001 | 0.537 | 0.506 | 0.554 | 0.769 |
| 250 | 10 | 50 | RBF | 0.001 | 0.554 | 0.514 | 0.557 | 0.770 |
| 250 | 10 | 50 | RBF | 0.01 | 0.051 | 0.085 | 0.510 | 0.469 |
| 250 | 10 | 100 | LIN | - | 0.532 | 0.496 | 0.555 | 0.687 |
| 250 | 10 | 100 | RBF | 0.0001 | 0.537 | 0.506 | 0.554 | 0.769 |
| 250 | 10 | 100 | RBF | 0.001 | 0.554 | 0.514 | 0.557 | 0.770 |
| 250 | 10 | 100 | RBF | 0.01 | 0.045 | 0.078 | 0.510 | 0.469 |
| 250 | 15 | 0.001 | LIN | - | 0.358 | 0.353 | 0.534 | 0.702 |
| 250 | 15 | 0.001 | RBF | 0.0001 | 0.546 | 0.509 | 0.553 | 0.776 |
| 250 | 15 | 0.001 | RBF | 0.001 | 0.551 | 0.512 | 0.555 | 0.769 |
| 250 | 15 | 0.001 | RBF | 0.01 | 0.234 | 0.250 | 0.519 | 0.536 |
| 250 | 15 | 0.01 | LIN | - | 0.382 | 0.374 | 0.519 | 0.675 |
| 250 | 15 | 0.01 | RBF | 0.0001 | 0.546 | 0.509 | 0.553 | 0.776 |
| 250 | 15 | 0.01 | RBF | 0.001 | 0.551 | 0.512 | 0.555 | 0.769 |
| 250 | 15 | 0.01 | RBF | 0.01 | 0.183 | 0.203 | 0.515 | 0.505 |
| 250 | 15 | 0.1 | LIN | - | 0.516 | 0.470 | 0.556 | 0.774 |
| 250 | 15 | 0.1 | RBF | 0.0001 | 0.546 | 0.509 | 0.553 | 0.776 |
| 250 | 15 | 0.1 | RBF | 0.001 | 0.551 | 0.512 | 0.555 | 0.769 |
| 250 | 15 | 0.1 | RBF | 0.01 | 0.139 | 0.163 | 0.515 | 0.485 |
| 250 | 15 | 0.2 | LIN | - | 0.538 | 0.501 | 0.559 | 0.775 |
| 250 | 15 | 0.2 | RBF | 0.0001 | 0.546 | 0.509 | 0.553 | 0.776 |
| 250 | 15 | 0.2 | RBF | 0.001 | 0.551 | 0.512 | 0.555 | 0.769 |
| 250 | 15 | 0.2 | RBF | 0.01 | 0.118 | 0.148 | 0.516 | 0.481 |
| 250 | 15 | 0.4 | LIN | - | 0.551 | 0.514 | 0.558 | 0.776 |
| 250 | 15 | 0.4 | RBF | 0.0001 | 0.546 | 0.509 | 0.553 | 0.776 |
| 250 | 15 | 0.4 | RBF | 0.001 | 0.551 | 0.512 | 0.555 | 0.769 |
| 250 | 15 | 0.4 | RBF | 0.01 | 0.100 | 0.130 | 0.513 | 0.477 |
| 250 | 15 | 0.6 | LIN | - | 0.522 | 0.483 | 0.559 | 0.776 |
| 250 | 15 | 0.6 | RBF | 0.0001 | 0.546 | 0.509 | 0.553 | 0.776 |
| 250 | 15 | 0.6 | RBF | 0.001 | 0.551 | 0.512 | 0.555 | 0.769 |
| 250 | 15 | 0.6 | RBF | 0.01 | 0.095 | 0.123 | 0.513 | 0.476 |
| 250 | 15 | 0.8 | LIN | - | 0.554 | 0.508 | 0.556 | 0.777 |
| 250 | 15 | 0.8 | RBF | 0.0001 | 0.546 | 0.509 | 0.553 | 0.776 |
| 250 | 15 | 0.8 | RBF | 0.001 | 0.551 | 0.512 | 0.555 | 0.769 |
| 250 | 15 | 0.8 | RBF | 0.01 | 0.089 | 0.120 | 0.512 | 0.475 |
| 250 | 15 | 1.0 | LIN | - | 0.525 | 0.490 | 0.556 | 0.778 |
| 250 | 15 | 1.0 | RBF | 0.0001 | 0.546 | 0.509 | 0.553 | 0.776 |
| 250 | 15 | 1.0 | RBF | 0.001 | 0.551 | 0.512 | 0.555 | 0.769 |

Continued on next page

TABLE S17 – continued from previous page

| n | $k$ | $\lambda$ | usim | $\sigma$ | AP@5 | AP@10 | sCI | CI |
|---|---|---|---|---|---|---|---|---|
| 250 | 15 | 1.0 | RBF | 0.01 | 0.077 | 0.108 | 0.512 | 0.474 |
| 250 | 15 | 10 | LIN | - | 0.565 | 0.520 | 0.552 | 0.778 |
| 250 | 15 | 10 | RBF | 0.0001 | 0.546 | 0.509 | 0.553 | 0.776 |
| 250 | 15 | 10 | RBF | 0.001 | 0.551 | 0.512 | 0.555 | 0.769 |
| 250 | 15 | 10 | RBF | 0.01 | 0.059 | 0.092 | 0.510 | 0.470 |
| 250 | 15 | 50 | LIN | - | 0.543 | 0.520 | 0.553 | 0.766 |
| 250 | 15 | 50 | RBF | 0.0001 | 0.546 | 0.509 | 0.553 | 0.776 |
| 250 | 15 | 50 | RBF | 0.001 | 0.551 | 0.512 | 0.555 | 0.769 |
| 250 | 15 | 50 | RBF | 0.01 | 0.051 | 0.085 | 0.510 | 0.469 |
| 250 | 15 | 100 | LIN | - | 0.537 | 0.501 | 0.554 | 0.712 |
| 250 | 15 | 100 | RBF | 0.0001 | 0.546 | 0.509 | 0.553 | 0.776 |
| 250 | 15 | 100 | RBF | 0.001 | 0.551 | 0.512 | 0.555 | 0.769 |
| 250 | 15 | 100 | RBF | 0.01 | 0.047 | 0.079 | 0.509 | 0.469 |
| 300 | 5 | 0.000001 | LIN | - | 0.291 | 0.309 | 0.527 | 0.693 |
| 300 | 5 | 0.000001 | RBF | 0.0001 | 0.414 | 0.409 | 0.539 | 0.718 |
| 300 | 5 | 0.000001 | RBF | 0.001 | 0.453 | 0.429 | 0.553 | 0.719 |
| 300 | 5 | 0.000001 | RBF | 0.01 | 0.311 | 0.315 | 0.528 | 0.580 |
| 300 | 5 | 0.00001 | RBF | 0.0001 | 0.512 | 0.479 | 0.539 | 0.751 |
| 300 | 5 | 0.00001 | RBF | 0.001 | 0.519 | 0.487 | 0.561 | 0.754 |
| 300 | 5 | 0.00001 | RBF | 0.01 | 0.309 | 0.315 | 0.524 | 0.579 |
| 300 | 5 | 0.0001 | RBF | 0.0001 | 0.482 | 0.459 | 0.559 | 0.776 |
| 300 | 5 | 0.0001 | RBF | 0.001 | 0.519 | 0.487 | 0.561 | 0.754 |
| 300 | 5 | 0.0001 | RBF | 0.01 | 0.277 | 0.287 | 0.520 | 0.551 |
| 300 | 5 | 0.001 | LIN | - | 0.385 | 0.361 | 0.545 | 0.725 |
| 300 | 5 | 0.001 | RBF | 0.0001 | 0.534 | 0.497 | 0.550 | 0.729 |
| 300 | 5 | 0.001 | RBF | 0.001 | 0.519 | 0.487 | 0.561 | 0.754 |
| 300 | 5 | 0.001 | RBF | 0.01 | 0.247 | 0.263 | 0.520 | 0.522 |
| 300 | 5 | 0.01 | LIN | - | 0.469 | 0.449 | 0.549 | 0.747 |
| 300 | 5 | 0.01 | RBF | 0.0001 | 0.534 | 0.497 | 0.550 | 0.729 |
| 300 | 5 | 0.01 | RBF | 0.001 | 0.519 | 0.487 | 0.561 | 0.754 |
| 300 | 5 | 0.01 | RBF | 0.01 | 0.182 | 0.198 | 0.514 | 0.497 |
| 300 | 5 | 0.1 | LIN | - | 0.483 | 0.460 | 0.543 | 0.755 |
| 300 | 5 | 0.1 | RBF | 0.0001 | 0.534 | 0.497 | 0.550 | 0.729 |
| 300 | 5 | 0.1 | RBF | 0.001 | 0.519 | 0.487 | 0.561 | 0.754 |
| 300 | 5 | 0.1 | RBF | 0.01 | 0.133 | 0.159 | 0.515 | 0.482 |
| 300 | 5 | 0.2 | LIN | - | 0.533 | 0.486 | 0.550 | 0.762 |
| 300 | 5 | 0.2 | RBF | 0.0001 | 0.534 | 0.497 | 0.550 | 0.729 |
| 300 | 5 | 0.2 | RBF | 0.001 | 0.519 | 0.487 | 0.561 | 0.754 |
| 300 | 5 | 0.2 | RBF | 0.01 | 0.124 | 0.151 | 0.511 | 0.478 |
| 300 | 5 | 0.4 | LIN | - | 0.427 | 0.426 | 0.551 | 0.772 |
| 300 | 5 | 0.4 | RBF | 0.0001 | 0.534 | 0.497 | 0.550 | 0.729 |
| 300 | 5 | 0.4 | RBF | 0.001 | 0.519 | 0.487 | 0.561 | 0.754 |
| 300 | 5 | 0.4 | RBF | 0.01 | 0.102 | 0.129 | 0.510 | 0.475 |
| 300 | 5 | 0.6 | LIN | - | 0.545 | 0.488 | 0.551 | 0.765 |
| 300 | 5 | 0.6 | RBF | 0.0001 | 0.534 | 0.497 | 0.550 | 0.729 |
| 300 | 5 | 0.6 | RBF | 0.001 | 0.519 | 0.487 | 0.561 | 0.754 |
| 300 | 5 | 0.6 | RBF | 0.01 | 0.088 | 0.117 | 0.510 | 0.474 |
| 300 | 5 | 0.8 | LIN | - | 0.507 | 0.477 | 0.550 | 0.770 |
| 300 | 5 | 0.8 | RBF | 0.0001 | 0.534 | 0.497 | 0.550 | 0.729 |
| 300 | 5 | 0.8 | RBF | 0.001 | 0.519 | 0.487 | 0.561 | 0.754 |
| 300 | 5 | 0.8 | RBF | 0.01 | 0.077 | 0.107 | 0.509 | 0.473 |
| 300 | 5 | 1.0 | LIN | - | 0.519 | 0.490 | 0.553 | 0.770 |
| 300 | 5 | 1.0 | RBF | 0.0001 | 0.534 | 0.497 | 0.550 | 0.729 |
| 300 | 5 | 1.0 | RBF | 0.001 | 0.519 | 0.487 | 0.561 | 0.754 |
| 300 | 5 | 1.0 | RBF | 0.01 | 0.078 | 0.105 | 0.509 | 0.472 |
| 300 | 5 | 10 | LIN | - | 0.570 | 0.503 | 0.549 | 0.773 |
| 300 | 5 | 10 | RBF | 0.0001 | 0.534 | 0.497 | 0.550 | 0.729 |
| 300 | 5 | 10 | RBF | 0.001 | 0.519 | 0.487 | 0.561 | 0.754 |

Continued on next page

TABLE S17 – continued from previous page

| n | $k$ | $\lambda$ | usim | $\sigma$ | AP@5 | AP@10 | sCI | CI |
|---|---|---|---|---|---|---|---|---|
| 300 | 5 | 10 | RBF | 0.01 | 0.052 | 0.086 | 0.508 | 0.470 |
| 300 | 5 | 50 | LIN | - | 0.540 | 0.502 | 0.555 | 0.742 |
| 300 | 5 | 50 | RBF | 0.0001 | 0.534 | 0.497 | 0.550 | 0.729 |
| 300 | 5 | 50 | RBF | 0.001 | 0.519 | 0.487 | 0.561 | 0.754 |
| 300 | 5 | 50 | RBF | 0.01 | 0.044 | 0.079 | 0.508 | 0.469 |
| 300 | 5 | 100 | LIN | - | 0.532 | 0.495 | 0.550 | 0.664 |
| 300 | 5 | 100 | RBF | 0.0001 | 0.534 | 0.497 | 0.550 | 0.729 |
| 300 | 5 | 100 | RBF | 0.001 | 0.519 | 0.487 | 0.561 | 0.754 |
| 300 | 5 | 100 | RBF | 0.01 | 0.044 | 0.077 | 0.508 | 0.468 |
| 300 | 10 | 0.000001 | LIN | - | 0.252 | 0.267 | 0.516 | 0.693 |
| 300 | 10 | 0.000001 | RBF | 0.01 | 0.318 | 0.320 | 0.527 | 0.572 |
| 300 | 10 | 0.001 | LIN | - | 0.376 | 0.367 | 0.536 | 0.708 |
| 300 | 10 | 0.001 | RBF | 0.0001 | 0.534 | 0.499 | 0.552 | 0.770 |
| 300 | 10 | 0.001 | RBF | 0.001 | 0.525 | 0.491 | 0.560 | 0.767 |
| 300 | 10 | 0.001 | RBF | 0.01 | 0.250 | 0.265 | 0.520 | 0.530 |
| 300 | 10 | 0.01 | LIN | - | 0.438 | 0.417 | 0.550 | 0.757 |
| 300 | 10 | 0.01 | RBF | 0.0001 | 0.534 | 0.499 | 0.552 | 0.770 |
| 300 | 10 | 0.01 | RBF | 0.001 | 0.525 | 0.491 | 0.560 | 0.767 |
| 300 | 10 | 0.01 | RBF | 0.01 | 0.188 | 0.203 | 0.514 | 0.502 |
| 300 | 10 | 0.1 | LIN | - | 0.482 | 0.459 | 0.552 | 0.776 |
| 300 | 10 | 0.1 | RBF | 0.0001 | 0.534 | 0.499 | 0.552 | 0.770 |
| 300 | 10 | 0.1 | RBF | 0.001 | 0.525 | 0.491 | 0.560 | 0.767 |
| 300 | 10 | 0.1 | RBF | 0.01 | 0.138 | 0.163 | 0.513 | 0.484 |
| 300 | 10 | 0.2 | LIN | - | 0.489 | 0.463 | 0.552 | 0.776 |
| 300 | 10 | 0.2 | RBF | 0.0001 | 0.534 | 0.499 | 0.552 | 0.770 |
| 300 | 10 | 0.2 | RBF | 0.001 | 0.525 | 0.491 | 0.560 | 0.767 |
| 300 | 10 | 0.2 | RBF | 0.01 | 0.130 | 0.154 | 0.511 | 0.480 |
| 300 | 10 | 0.4 | LIN | - | 0.518 | 0.470 | 0.551 | 0.776 |
| 300 | 10 | 0.4 | RBF | 0.0001 | 0.534 | 0.499 | 0.552 | 0.770 |
| 300 | 10 | 0.4 | RBF | 0.001 | 0.525 | 0.491 | 0.560 | 0.767 |
| 300 | 10 | 0.4 | RBF | 0.01 | 0.113 | 0.137 | 0.511 | 0.476 |
| 300 | 10 | 0.6 | LIN | - | 0.519 | 0.476 | 0.554 | 0.779 |
| 300 | 10 | 0.6 | RBF | 0.0001 | 0.534 | 0.499 | 0.552 | 0.770 |
| 300 | 10 | 0.6 | RBF | 0.001 | 0.525 | 0.491 | 0.560 | 0.767 |
| 300 | 10 | 0.6 | RBF | 0.01 | 0.091 | 0.119 | 0.509 | 0.475 |
| 300 | 10 | 0.8 | LIN | - | 0.549 | 0.499 | 0.552 | 0.780 |
| 300 | 10 | 0.8 | RBF | 0.0001 | 0.534 | 0.499 | 0.552 | 0.770 |
| 300 | 10 | 0.8 | RBF | 0.001 | 0.525 | 0.491 | 0.560 | 0.767 |
| 300 | 10 | 0.8 | RBF | 0.01 | 0.081 | 0.112 | 0.509 | 0.474 |
| 300 | 10 | 1.0 | LIN | - | 0.561 | 0.508 | 0.548 | 0.775 |
| 300 | 10 | 1.0 | RBF | 0.0001 | 0.534 | 0.499 | 0.552 | 0.770 |
| 300 | 10 | 1.0 | RBF | 0.001 | 0.525 | 0.491 | 0.560 | 0.767 |
| 300 | 10 | 1.0 | RBF | 0.01 | 0.080 | 0.108 | 0.509 | 0.473 |
| 300 | 10 | 10 | LIN | - | 0.546 | 0.517 | 0.549 | 0.788 |
| 300 | 10 | 10 | RBF | 0.0001 | 0.534 | 0.499 | 0.552 | 0.770 |
| 300 | 10 | 10 | RBF | 0.001 | 0.525 | 0.491 | 0.560 | 0.767 |
| 300 | 10 | 10 | RBF | 0.01 | 0.053 | 0.088 | 0.508 | 0.470 |
| 300 | 10 | 50 | LIN | - | 0.536 | 0.500 | 0.554 | 0.754 |
| 300 | 10 | 50 | RBF | 0.0001 | 0.534 | 0.499 | 0.552 | 0.770 |
| 300 | 10 | 50 | RBF | 0.001 | 0.525 | 0.491 | 0.560 | 0.767 |
| 300 | 10 | 50 | RBF | 0.01 | 0.046 | 0.081 | 0.508 | 0.469 |
| 300 | 10 | 100 | LIN | - | 0.533 | 0.495 | 0.551 | 0.691 |
| 300 | 10 | 100 | RBF | 0.0001 | 0.534 | 0.499 | 0.552 | 0.770 |
| 300 | 10 | 100 | RBF | 0.001 | 0.525 | 0.491 | 0.560 | 0.767 |
| 300 | 10 | 100 | RBF | 0.01 | 0.046 | 0.081 | 0.508 | 0.469 |
| 300 | 15 | 0.001 | LIN | - | 0.298 | 0.301 | 0.534 | 0.691 |
| 300 | 15 | 0.001 | RBF | 0.0001 | 0.538 | 0.504 | 0.556 | 0.776 |
| 300 | 15 | 0.001 | RBF | 0.001 | 0.527 | 0.497 | 0.558 | 0.765 |

Continued on next page

TABLE S17 – continued from previous page

| n | $k$ | $\lambda$ | usim | $\sigma$ | AP@5 | AP@10 | sCI | CI |
|---|---|---|---|---|---|---|---|---|
| 300 | 15 | 0.001 | RBF | 0.01 | 0.252 | 0.266 | 0.520 | 0.532 |
| 300 | 15 | 0.01 | LIN | - | 0.359 | 0.353 | 0.535 | 0.699 |
| 300 | 15 | 0.01 | RBF | 0.0001 | 0.538 | 0.504 | 0.556 | 0.776 |
| 300 | 15 | 0.01 | RBF | 0.001 | 0.527 | 0.497 | 0.558 | 0.765 |
| 300 | 15 | 0.01 | RBF | 0.01 | 0.192 | 0.208 | 0.515 | 0.503 |
| 300 | 15 | 0.1 | LIN | - | 0.480 | 0.458 | 0.558 | 0.774 |
| 300 | 15 | 0.1 | RBF | 0.0001 | 0.538 | 0.504 | 0.556 | 0.776 |
| 300 | 15 | 0.1 | RBF | 0.001 | 0.527 | 0.497 | 0.558 | 0.765 |
| 300 | 15 | 0.1 | RBF | 0.01 | 0.136 | 0.162 | 0.513 | 0.485 |
| 300 | 15 | 0.2 | LIN | - | 0.525 | 0.485 | 0.557 | 0.774 |
| 300 | 15 | 0.2 | RBF | 0.0001 | 0.538 | 0.504 | 0.556 | 0.776 |
| 300 | 15 | 0.2 | RBF | 0.001 | 0.527 | 0.497 | 0.558 | 0.765 |
| 300 | 15 | 0.2 | RBF | 0.01 | 0.132 | 0.155 | 0.511 | 0.480 |
| 300 | 15 | 0.4 | LIN | - | 0.522 | 0.484 | 0.557 | 0.776 |
| 300 | 15 | 0.4 | RBF | 0.0001 | 0.538 | 0.504 | 0.556 | 0.776 |
| 300 | 15 | 0.4 | RBF | 0.001 | 0.527 | 0.497 | 0.558 | 0.765 |
| 300 | 15 | 0.4 | RBF | 0.01 | 0.118 | 0.143 | 0.509 | 0.477 |
| 300 | 15 | 0.6 | LIN | - | 0.542 | 0.496 | 0.555 | 0.775 |
| 300 | 15 | 0.6 | RBF | 0.0001 | 0.538 | 0.504 | 0.556 | 0.776 |
| 300 | 15 | 0.6 | RBF | 0.001 | 0.527 | 0.497 | 0.558 | 0.765 |
| 300 | 15 | 0.6 | RBF | 0.01 | 0.093 | 0.119 | 0.508 | 0.475 |
| 300 | 15 | 0.8 | LIN | - | 0.536 | 0.506 | 0.556 | 0.779 |
| 300 | 15 | 0.8 | RBF | 0.0001 | 0.538 | 0.504 | 0.556 | 0.776 |
| 300 | 15 | 0.8 | RBF | 0.001 | 0.527 | 0.497 | 0.558 | 0.765 |
| 300 | 15 | 0.8 | RBF | 0.01 | 0.081 | 0.113 | 0.509 | 0.474 |
| 300 | 15 | 1.0 | LIN | - | 0.560 | 0.514 | 0.556 | 0.779 |
| 300 | 15 | 1.0 | RBF | 0.0001 | 0.538 | 0.504 | 0.556 | 0.776 |
| 300 | 15 | 1.0 | RBF | 0.001 | 0.527 | 0.497 | 0.558 | 0.765 |
| 300 | 15 | 1.0 | RBF | 0.01 | 0.075 | 0.105 | 0.508 | 0.473 |
| 300 | 15 | 10 | LIN | - | 0.555 | 0.515 | 0.551 | 0.780 |
| 300 | 15 | 10 | RBF | 0.0001 | 0.538 | 0.504 | 0.556 | 0.776 |
| 300 | 15 | 10 | RBF | 0.001 | 0.527 | 0.497 | 0.558 | 0.765 |
| 300 | 15 | 10 | RBF | 0.01 | 0.054 | 0.088 | 0.508 | 0.470 |
| 300 | 15 | 50 | LIN | - | 0.534 | 0.506 | 0.555 | 0.764 |
| 300 | 15 | 50 | RBF | 0.0001 | 0.538 | 0.504 | 0.556 | 0.776 |
| 300 | 15 | 50 | RBF | 0.001 | 0.527 | 0.498 | 0.558 | 0.765 |
| 300 | 15 | 50 | RBF | 0.01 | 0.045 | 0.081 | 0.508 | 0.469 |
| 300 | 15 | 100 | LIN | - | 0.536 | 0.500 | 0.553 | 0.705 |
| 300 | 15 | 100 | RBF | 0.0001 | 0.538 | 0.504 | 0.556 | 0.776 |
| 300 | 15 | 100 | RBF | 0.001 | 0.527 | 0.498 | 0.558 | 0.765 |
| 300 | 15 | 100 | RBF | 0.01 | 0.047 | 0.081 | 0.508 | 0.469 |
| 350 | 5 | 0.000001 | LIN | - | 0.247 | 0.264 | 0.534 | 0.691 |
| 350 | 5 | 0.000001 | RBF | 0.0001 | 0.426 | 0.406 | 0.533 | 0.730 |
| 350 | 5 | 0.000001 | RBF | 0.001 | 0.463 | 0.431 | 0.549 | 0.714 |
| 350 | 5 | 0.000001 | RBF | 0.01 | 0.314 | 0.314 | 0.524 | 0.574 |
| 350 | 5 | 0.00001 | RBF | 0.0001 | 0.476 | 0.442 | 0.539 | 0.758 |
| 350 | 5 | 0.00001 | RBF | 0.001 | 0.513 | 0.482 | 0.555 | 0.748 |
| 350 | 5 | 0.00001 | RBF | 0.01 | 0.295 | 0.303 | 0.520 | 0.570 |
| 350 | 5 | 0.0001 | RBF | 0.0001 | 0.527 | 0.493 | 0.553 | 0.774 |
| 350 | 5 | 0.0001 | RBF | 0.001 | 0.513 | 0.482 | 0.555 | 0.748 |
| 350 | 5 | 0.0001 | RBF | 0.01 | 0.262 | 0.276 | 0.517 | 0.543 |
| 350 | 5 | 0.001 | LIN | - | 0.329 | 0.324 | 0.523 | 0.684 |
| 350 | 5 | 0.001 | RBF | 0.0001 | 0.528 | 0.488 | 0.551 | 0.724 |
| 350 | 5 | 0.001 | RBF | 0.001 | 0.513 | 0.482 | 0.555 | 0.748 |
| 350 | 5 | 0.001 | RBF | 0.01 | 0.236 | 0.252 | 0.515 | 0.518 |
| 350 | 5 | 0.01 | LIN | - | 0.461 | 0.432 | 0.545 | 0.744 |
| 350 | 5 | 0.01 | RBF | 0.0001 | 0.528 | 0.488 | 0.551 | 0.724 |
| 350 | 5 | 0.01 | RBF | 0.001 | 0.513 | 0.482 | 0.555 | 0.748 |

Continued on next page

TABLE S17 – continued from previous page

| n | $k$ | $\lambda$ | usim | $\sigma$ | AP@5 | AP@10 | sCI | CI |
|---|---|---|---|---|---|---|---|---|
| 350 | 5 | 0.01 | RBF | 0.01 | 0.178 | 0.197 | 0.513 | 0.496 |
| 350 | 5 | 0.1 | LIN | - | 0.465 | 0.440 | 0.546 | 0.763 |
| 350 | 5 | 0.1 | RBF | 0.0001 | 0.528 | 0.488 | 0.551 | 0.724 |
| 350 | 5 | 0.1 | RBF | 0.001 | 0.513 | 0.482 | 0.555 | 0.748 |
| 350 | 5 | 0.1 | RBF | 0.01 | 0.138 | 0.164 | 0.510 | 0.482 |
| 350 | 5 | 0.2 | LIN | - | 0.460 | 0.438 | 0.545 | 0.761 |
| 350 | 5 | 0.2 | RBF | 0.0001 | 0.528 | 0.488 | 0.551 | 0.724 |
| 350 | 5 | 0.2 | RBF | 0.001 | 0.513 | 0.482 | 0.555 | 0.748 |
| 350 | 5 | 0.2 | RBF | 0.01 | 0.121 | 0.144 | 0.510 | 0.479 |
| 350 | 5 | 0.4 | LIN | - | 0.488 | 0.452 | 0.549 | 0.769 |
| 350 | 5 | 0.4 | RBF | 0.0001 | 0.528 | 0.488 | 0.551 | 0.724 |
| 350 | 5 | 0.4 | RBF | 0.001 | 0.513 | 0.482 | 0.555 | 0.748 |
| 350 | 5 | 0.4 | RBF | 0.01 | 0.102 | 0.129 | 0.510 | 0.476 |
| 350 | 5 | 0.6 | LIN | - | 0.518 | 0.464 | 0.548 | 0.767 |
| 350 | 5 | 0.6 | RBF | 0.0001 | 0.528 | 0.488 | 0.551 | 0.724 |
| 350 | 5 | 0.6 | RBF | 0.001 | 0.513 | 0.482 | 0.555 | 0.748 |
| 350 | 5 | 0.6 | RBF | 0.01 | 0.094 | 0.120 | 0.509 | 0.474 |
| 350 | 5 | 0.8 | LIN | - | 0.493 | 0.459 | 0.550 | 0.774 |
| 350 | 5 | 0.8 | RBF | 0.0001 | 0.528 | 0.488 | 0.551 | 0.724 |
| 350 | 5 | 0.8 | RBF | 0.001 | 0.513 | 0.482 | 0.555 | 0.748 |
| 350 | 5 | 0.8 | RBF | 0.01 | 0.092 | 0.119 | 0.508 | 0.474 |
| 350 | 5 | 1.0 | LIN | - | 0.488 | 0.457 | 0.548 | 0.770 |
| 350 | 5 | 1.0 | RBF | 0.0001 | 0.528 | 0.488 | 0.551 | 0.724 |
| 350 | 5 | 1.0 | RBF | 0.001 | 0.513 | 0.482 | 0.555 | 0.748 |
| 350 | 5 | 1.0 | RBF | 0.01 | 0.085 | 0.112 | 0.508 | 0.473 |
| 350 | 5 | 10 | LIN | - | 0.541 | 0.491 | 0.542 | 0.762 |
| 350 | 5 | 10 | RBF | 0.0001 | 0.528 | 0.488 | 0.551 | 0.724 |
| 350 | 5 | 10 | RBF | 0.001 | 0.513 | 0.482 | 0.555 | 0.748 |
| 350 | 5 | 10 | RBF | 0.01 | 0.057 | 0.090 | 0.508 | 0.470 |
| 350 | 5 | 50 | LIN | - | 0.520 | 0.491 | 0.553 | 0.719 |
| 350 | 5 | 50 | RBF | 0.0001 | 0.528 | 0.488 | 0.551 | 0.724 |
| 350 | 5 | 50 | RBF | 0.001 | 0.513 | 0.482 | 0.555 | 0.748 |
| 350 | 5 | 50 | RBF | 0.01 | 0.053 | 0.088 | 0.507 | 0.469 |
| 350 | 5 | 100 | LIN | - | 0.509 | 0.473 | 0.549 | 0.647 |
| 350 | 5 | 100 | RBF | 0.0001 | 0.528 | 0.488 | 0.551 | 0.724 |
| 350 | 5 | 100 | RBF | 0.001 | 0.513 | 0.482 | 0.555 | 0.748 |
| 350 | 5 | 100 | RBF | 0.01 | 0.050 | 0.084 | 0.507 | 0.469 |
| 350 | 10 | 0.000001 | LIN | - | 0.291 | 0.304 | 0.517 | 0.706 |
| 350 | 10 | 0.000001 | RBF | 0.01 | 0.314 | 0.315 | 0.524 | 0.566 |
| 350 | 10 | 0.001 | LIN | - | 0.365 | 0.366 | 0.535 | 0.696 |
| 350 | 10 | 0.001 | RBF | 0.0001 | 0.528 | 0.498 | 0.552 | 0.765 |
| 350 | 10 | 0.001 | RBF | 0.001 | 0.515 | 0.484 | 0.554 | 0.762 |
| 350 | 10 | 0.001 | RBF | 0.01 | 0.247 | 0.258 | 0.515 | 0.526 |
| 350 | 10 | 0.01 | LIN | - | 0.367 | 0.367 | 0.529 | 0.704 |
| 350 | 10 | 0.01 | RBF | 0.0001 | 0.528 | 0.498 | 0.552 | 0.765 |
| 350 | 10 | 0.01 | RBF | 0.001 | 0.515 | 0.484 | 0.554 | 0.762 |
| 350 | 10 | 0.01 | RBF | 0.01 | 0.180 | 0.200 | 0.513 | 0.501 |
| 350 | 10 | 0.1 | LIN | - | 0.472 | 0.440 | 0.547 | 0.774 |
| 350 | 10 | 0.1 | RBF | 0.0001 | 0.528 | 0.498 | 0.552 | 0.765 |
| 350 | 10 | 0.1 | RBF | 0.001 | 0.515 | 0.484 | 0.554 | 0.762 |
| 350 | 10 | 0.1 | RBF | 0.01 | 0.141 | 0.166 | 0.509 | 0.485 |
| 350 | 10 | 0.2 | LIN | - | 0.518 | 0.481 | 0.546 | 0.773 |
| 350 | 10 | 0.2 | RBF | 0.0001 | 0.528 | 0.498 | 0.552 | 0.765 |
| 350 | 10 | 0.2 | RBF | 0.001 | 0.515 | 0.484 | 0.554 | 0.762 |
| 350 | 10 | 0.2 | RBF | 0.01 | 0.123 | 0.149 | 0.510 | 0.481 |
| 350 | 10 | 0.4 | LIN | - | 0.523 | 0.486 | 0.546 | 0.776 |
| 350 | 10 | 0.4 | RBF | 0.0001 | 0.528 | 0.498 | 0.552 | 0.765 |
| 350 | 10 | 0.4 | RBF | 0.001 | 0.515 | 0.484 | 0.554 | 0.762 |

Continued on next page

TABLE S17 – continued from previous page

| n | $k$ | $\lambda$ | usim | $\sigma$ | AP@5 | AP@10 | sCI | CI |
|---|---|---|---|---|---|---|---|---|
| 350 | 10 | 0.4 | RBF | 0.01 | 0.102 | 0.129 | 0.510 | 0.477 |
| 350 | 10 | 0.6 | LIN | - | 0.523 | 0.477 | 0.544 | 0.773 |
| 350 | 10 | 0.6 | RBF | 0.0001 | 0.528 | 0.498 | 0.552 | 0.765 |
| 350 | 10 | 0.6 | RBF | 0.001 | 0.515 | 0.484 | 0.554 | 0.762 |
| 350 | 10 | 0.6 | RBF | 0.01 | 0.092 | 0.120 | 0.509 | 0.476 |
| 350 | 10 | 0.8 | LIN | - | 0.533 | 0.502 | 0.547 | 0.778 |
| 350 | 10 | 0.8 | RBF | 0.0001 | 0.528 | 0.498 | 0.552 | 0.765 |
| 350 | 10 | 0.8 | RBF | 0.001 | 0.515 | 0.484 | 0.554 | 0.762 |
| 350 | 10 | 0.8 | RBF | 0.01 | 0.100 | 0.125 | 0.508 | 0.475 |
| 350 | 10 | 1.0 | LIN | - | 0.526 | 0.489 | 0.547 | 0.774 |
| 350 | 10 | 1.0 | RBF | 0.0001 | 0.528 | 0.498 | 0.552 | 0.765 |
| 350 | 10 | 1.0 | RBF | 0.001 | 0.515 | 0.484 | 0.554 | 0.762 |
| 350 | 10 | 1.0 | RBF | 0.01 | 0.080 | 0.108 | 0.508 | 0.474 |
| 350 | 10 | 10 | LIN | - | 0.549 | 0.515 | 0.544 | 0.782 |
| 350 | 10 | 10 | RBF | 0.0001 | 0.528 | 0.498 | 0.552 | 0.765 |
| 350 | 10 | 10 | RBF | 0.001 | 0.515 | 0.484 | 0.554 | 0.762 |
| 350 | 10 | 10 | RBF | 0.01 | 0.056 | 0.089 | 0.508 | 0.471 |
| 350 | 10 | 50 | LIN | - | 0.532 | 0.509 | 0.553 | 0.737 |
| 350 | 10 | 50 | RBF | 0.0001 | 0.528 | 0.498 | 0.552 | 0.765 |
| 350 | 10 | 50 | RBF | 0.001 | 0.515 | 0.484 | 0.554 | 0.762 |
| 350 | 10 | 50 | RBF | 0.01 | 0.055 | 0.089 | 0.507 | 0.470 |
| 350 | 10 | 100 | LIN | - | 0.513 | 0.481 | 0.552 | 0.686 |
| 350 | 10 | 100 | RBF | 0.0001 | 0.528 | 0.498 | 0.552 | 0.765 |
| 350 | 10 | 100 | RBF | 0.001 | 0.515 | 0.484 | 0.554 | 0.762 |
| 350 | 10 | 100 | RBF | 0.01 | 0.050 | 0.084 | 0.507 | 0.469 |
| 350 | 15 | 0.001 | LIN | - | 0.361 | 0.350 | 0.517 | 0.704 |
| 350 | 15 | 0.001 | RBF | 0.0001 | 0.531 | 0.506 | 0.554 | 0.772 |
| 350 | 15 | 0.001 | RBF | 0.001 | 0.511 | 0.485 | 0.553 | 0.760 |
| 350 | 15 | 0.001 | RBF | 0.01 | 0.250 | 0.259 | 0.515 | 0.528 |
| 350 | 15 | 0.01 | LIN | - | 0.351 | 0.351 | 0.528 | 0.723 |
| 350 | 15 | 0.01 | RBF | 0.0001 | 0.531 | 0.506 | 0.554 | 0.772 |
| 350 | 15 | 0.01 | RBF | 0.001 | 0.511 | 0.485 | 0.553 | 0.760 |
| 350 | 15 | 0.01 | RBF | 0.01 | 0.182 | 0.200 | 0.513 | 0.502 |
| 350 | 15 | 0.1 | LIN | - | 0.447 | 0.431 | 0.513 | 0.709 |
| 350 | 15 | 0.1 | RBF | 0.0001 | 0.531 | 0.506 | 0.554 | 0.772 |
| 350 | 15 | 0.1 | RBF | 0.001 | 0.511 | 0.485 | 0.553 | 0.760 |
| 350 | 15 | 0.1 | RBF | 0.01 | 0.143 | 0.163 | 0.510 | 0.485 |
| 350 | 15 | 0.2 | LIN | - | 0.505 | 0.475 | 0.551 | 0.771 |
| 350 | 15 | 0.2 | RBF | 0.0001 | 0.531 | 0.506 | 0.554 | 0.772 |
| 350 | 15 | 0.2 | RBF | 0.001 | 0.511 | 0.485 | 0.553 | 0.760 |
| 350 | 15 | 0.2 | RBF | 0.01 | 0.127 | 0.151 | 0.510 | 0.482 |
| 350 | 15 | 0.4 | LIN | - | 0.477 | 0.448 | 0.551 | 0.771 |
| 350 | 15 | 0.4 | RBF | 0.0001 | 0.531 | 0.506 | 0.554 | 0.772 |
| 350 | 15 | 0.4 | RBF | 0.001 | 0.511 | 0.485 | 0.553 | 0.760 |
| 350 | 15 | 0.4 | RBF | 0.01 | 0.107 | 0.130 | 0.510 | 0.478 |
| 350 | 15 | 0.6 | LIN | - | 0.510 | 0.484 | 0.550 | 0.773 |
| 350 | 15 | 0.6 | RBF | 0.0001 | 0.531 | 0.506 | 0.554 | 0.772 |
| 350 | 15 | 0.6 | RBF | 0.001 | 0.511 | 0.485 | 0.553 | 0.760 |
| 350 | 15 | 0.6 | RBF | 0.01 | 0.094 | 0.122 | 0.509 | 0.476 |
| 350 | 15 | 0.8 | LIN | - | 0.532 | 0.498 | 0.552 | 0.774 |
| 350 | 15 | 0.8 | RBF | 0.0001 | 0.531 | 0.506 | 0.554 | 0.772 |
| 350 | 15 | 0.8 | RBF | 0.001 | 0.511 | 0.485 | 0.553 | 0.760 |
| 350 | 15 | 0.8 | RBF | 0.01 | 0.099 | 0.125 | 0.509 | 0.475 |
| 350 | 15 | 1.0 | LIN | - | 0.479 | 0.461 | 0.551 | 0.775 |
| 350 | 15 | 1.0 | RBF | 0.0001 | 0.531 | 0.506 | 0.554 | 0.772 |
| 350 | 15 | 1.0 | RBF | 0.001 | 0.511 | 0.485 | 0.553 | 0.760 |
| 350 | 15 | 1.0 | RBF | 0.01 | 0.086 | 0.112 | 0.508 | 0.474 |
| 350 | 15 | 10 | LIN | - | 0.536 | 0.502 | 0.547 | 0.776 |

Continued on next page

TABLE S17 – continued from previous page

| n | $k$ | $\lambda$ | usim | $\sigma$ | AP@5 | AP@10 | sCI | CI |
|---|---|---|---|---|---|---|---|---|
| 350 | 15 | 10 | RBF | 0.0001 | 0.531 | 0.506 | 0.554 | 0.772 |
| 350 | 15 | 10 | RBF | 0.001 | 0.511 | 0.485 | 0.553 | 0.760 |
| 350 | 15 | 10 | RBF | 0.01 | 0.057 | 0.089 | 0.508 | 0.471 |
| 350 | 15 | 50 | LIN | - | 0.537 | 0.512 | 0.551 | 0.751 |
| 350 | 15 | 50 | RBF | 0.0001 | 0.531 | 0.506 | 0.554 | 0.772 |
| 350 | 15 | 50 | RBF | 0.001 | 0.511 | 0.485 | 0.553 | 0.760 |
| 350 | 15 | 50 | RBF | 0.01 | 0.052 | 0.087 | 0.507 | 0.470 |
| 350 | 15 | 100 | LIN | - | 0.533 | 0.490 | 0.553 | 0.698 |
| 350 | 15 | 100 | RBF | 0.0001 | 0.531 | 0.506 | 0.554 | 0.772 |
| 350 | 15 | 100 | RBF | 0.001 | 0.510 | 0.484 | 0.553 | 0.760 |
| 350 | 15 | 100 | RBF | 0.01 | 0.051 | 0.085 | 0.507 | 0.469 |
| 400 | 5 | 0.000001 | LIN | - | 0.238 | 0.251 | 0.528 | 0.699 |
| 400 | 5 | 0.000001 | RBF | 0.0001 | 0.433 | 0.413 | 0.539 | 0.714 |
| 400 | 5 | 0.000001 | RBF | 0.001 | 0.456 | 0.434 | 0.551 | 0.712 |
| 400 | 5 | 0.000001 | RBF | 0.01 | 0.314 | 0.317 | 0.521 | 0.571 |
| 400 | 5 | 0.00001 | RBF | 0.0001 | 0.472 | 0.446 | 0.543 | 0.766 |
| 400 | 5 | 0.00001 | RBF | 0.001 | 0.530 | 0.491 | 0.556 | 0.747 |
| 400 | 5 | 0.00001 | RBF | 0.01 | 0.314 | 0.316 | 0.521 | 0.566 |
| 400 | 5 | 0.0001 | LIN | - | 0.376 | 0.359 | 0.523 | 0.680 |
| 400 | 5 | 0.0001 | RBF | 0.0001 | 0.535 | 0.497 | 0.555 | 0.770 |
| 400 | 5 | 0.0001 | RBF | 0.001 | 0.530 | 0.491 | 0.556 | 0.747 |
| 400 | 5 | 0.0001 | RBF | 0.01 | 0.279 | 0.286 | 0.515 | 0.541 |
| 400 | 5 | 0.001 | LIN | - | 0.371 | 0.366 | 0.544 | 0.723 |
| 400 | 5 | 0.001 | RBF | 0.0001 | 0.515 | 0.479 | 0.550 | 0.724 |
| 400 | 5 | 0.001 | RBF | 0.001 | 0.530 | 0.491 | 0.556 | 0.747 |
| 400 | 5 | 0.001 | RBF | 0.01 | 0.229 | 0.244 | 0.514 | 0.517 |
| 400 | 5 | 0.01 | LIN | - | 0.444 | 0.429 | 0.549 | 0.746 |
| 400 | 5 | 0.01 | RBF | 0.0001 | 0.515 | 0.479 | 0.550 | 0.724 |
| 400 | 5 | 0.01 | RBF | 0.001 | 0.530 | 0.491 | 0.556 | 0.747 |
| 400 | 5 | 0.01 | RBF | 0.01 | 0.175 | 0.194 | 0.511 | 0.496 |
| 400 | 5 | 0.1 | LIN | - | 0.441 | 0.417 | 0.535 | 0.766 |
| 400 | 5 | 0.1 | RBF | 0.0001 | 0.515 | 0.479 | 0.550 | 0.724 |
| 400 | 5 | 0.1 | RBF | 0.001 | 0.530 | 0.491 | 0.556 | 0.747 |
| 400 | 5 | 0.1 | RBF | 0.01 | 0.134 | 0.160 | 0.509 | 0.482 |
| 400 | 5 | 0.2 | LIN | - | 0.479 | 0.436 | 0.548 | 0.766 |
| 400 | 5 | 0.2 | RBF | 0.0001 | 0.515 | 0.479 | 0.550 | 0.724 |
| 400 | 5 | 0.2 | RBF | 0.001 | 0.530 | 0.491 | 0.556 | 0.747 |
| 400 | 5 | 0.2 | RBF | 0.01 | 0.126 | 0.149 | 0.508 | 0.479 |
| 400 | 5 | 0.4 | LIN | - | 0.451 | 0.442 | 0.548 | 0.768 |
| 400 | 5 | 0.4 | RBF | 0.0001 | 0.515 | 0.479 | 0.550 | 0.724 |
| 400 | 5 | 0.4 | RBF | 0.001 | 0.530 | 0.491 | 0.556 | 0.747 |
| 400 | 5 | 0.4 | RBF | 0.01 | 0.106 | 0.130 | 0.507 | 0.476 |
| 400 | 5 | 0.6 | LIN | - | 0.498 | 0.463 | 0.546 | 0.768 |
| 400 | 5 | 0.6 | RBF | 0.0001 | 0.515 | 0.479 | 0.550 | 0.724 |
| 400 | 5 | 0.6 | RBF | 0.001 | 0.530 | 0.491 | 0.556 | 0.747 |
| 400 | 5 | 0.6 | RBF | 0.01 | 0.098 | 0.125 | 0.508 | 0.474 |
| 400 | 5 | 0.8 | LIN | - | 0.443 | 0.436 | 0.549 | 0.763 |
| 400 | 5 | 0.8 | RBF | 0.0001 | 0.515 | 0.479 | 0.550 | 0.724 |
| 400 | 5 | 0.8 | RBF | 0.001 | 0.530 | 0.491 | 0.556 | 0.747 |
| 400 | 5 | 0.8 | RBF | 0.01 | 0.089 | 0.115 | 0.507 | 0.474 |
| 400 | 5 | 1.0 | LIN | - | 0.532 | 0.499 | 0.550 | 0.774 |
| 400 | 5 | 1.0 | RBF | 0.0001 | 0.515 | 0.479 | 0.550 | 0.724 |
| 400 | 5 | 1.0 | RBF | 0.001 | 0.530 | 0.491 | 0.556 | 0.747 |
| 400 | 5 | 1.0 | RBF | 0.01 | 0.084 | 0.109 | 0.507 | 0.473 |
| 400 | 5 | 10 | LIN | - | 0.474 | 0.444 | 0.548 | 0.762 |
| 400 | 5 | 10 | RBF | 0.0001 | 0.515 | 0.479 | 0.550 | 0.724 |
| 400 | 5 | 10 | RBF | 0.001 | 0.530 | 0.491 | 0.556 | 0.747 |
| 400 | 5 | 10 | RBF | 0.01 | 0.058 | 0.091 | 0.507 | 0.470 |

Continued on next page

TABLE S17 – continued from previous page

| n | $k$ | $\lambda$ | usim | $\sigma$ | AP@5 | AP@10 | sCI | CI |
|---|---|---|---|---|---|---|---|---|
| 400 | 5 | 50 | LIN | - | 0.505 | 0.474 | 0.553 | 0.705 |
| 400 | 5 | 50 | RBF | 0.0001 | 0.515 | 0.479 | 0.550 | 0.724 |
| 400 | 5 | 50 | RBF | 0.001 | 0.530 | 0.491 | 0.556 | 0.747 |
| 400 | 5 | 50 | RBF | 0.01 | 0.049 | 0.084 | 0.505 | 0.469 |
| 400 | 5 | 100 | LIN | - | 0.510 | 0.476 | 0.549 | 0.649 |
| 400 | 5 | 100 | RBF | 0.0001 | 0.515 | 0.479 | 0.550 | 0.724 |
| 400 | 5 | 100 | RBF | 0.001 | 0.529 | 0.491 | 0.556 | 0.747 |
| 400 | 5 | 100 | RBF | 0.01 | 0.049 | 0.083 | 0.505 | 0.469 |
| 400 | 10 | 0.000001 | LIN | - | 0.281 | 0.284 | 0.534 | 0.691 |
| 400 | 10 | 0.000001 | RBF | 0.001 | 0.454 | 0.428 | 0.553 | 0.701 |
| 400 | 10 | 0.000001 | RBF | 0.01 | 0.312 | 0.318 | 0.520 | 0.564 |
| 400 | 10 | 0.001 | LIN | - | 0.381 | 0.372 | 0.520 | 0.706 |
| 400 | 10 | 0.001 | RBF | 0.0001 | 0.516 | 0.487 | 0.551 | 0.764 |
| 400 | 10 | 0.001 | RBF | 0.001 | 0.530 | 0.491 | 0.555 | 0.762 |
| 400 | 10 | 0.001 | RBF | 0.01 | 0.230 | 0.247 | 0.515 | 0.525 |
| 400 | 10 | 0.01 | LIN | - | 0.405 | 0.394 | 0.549 | 0.762 |
| 400 | 10 | 0.01 | RBF | 0.0001 | 0.516 | 0.487 | 0.551 | 0.764 |
| 400 | 10 | 0.01 | RBF | 0.001 | 0.530 | 0.491 | 0.555 | 0.762 |
| 400 | 10 | 0.01 | RBF | 0.01 | 0.181 | 0.197 | 0.511 | 0.501 |
| 400 | 10 | 0.1 | LIN | - | 0.459 | 0.435 | 0.551 | 0.769 |
| 400 | 10 | 0.1 | RBF | 0.0001 | 0.516 | 0.487 | 0.551 | 0.764 |
| 400 | 10 | 0.1 | RBF | 0.001 | 0.530 | 0.491 | 0.555 | 0.762 |
| 400 | 10 | 0.1 | RBF | 0.01 | 0.136 | 0.158 | 0.509 | 0.484 |
| 400 | 10 | 0.2 | LIN | - | 0.503 | 0.469 | 0.552 | 0.775 |
| 400 | 10 | 0.2 | RBF | 0.0001 | 0.516 | 0.487 | 0.551 | 0.764 |
| 400 | 10 | 0.2 | RBF | 0.001 | 0.530 | 0.491 | 0.555 | 0.762 |
| 400 | 10 | 0.2 | RBF | 0.01 | 0.129 | 0.149 | 0.508 | 0.481 |
| 400 | 10 | 0.4 | LIN | - | 0.506 | 0.471 | 0.551 | 0.776 |
| 400 | 10 | 0.4 | RBF | 0.0001 | 0.516 | 0.487 | 0.551 | 0.764 |
| 400 | 10 | 0.4 | RBF | 0.001 | 0.530 | 0.491 | 0.555 | 0.762 |
| 400 | 10 | 0.4 | RBF | 0.01 | 0.109 | 0.131 | 0.508 | 0.477 |
| 400 | 10 | 0.6 | LIN | - | 0.525 | 0.473 | 0.550 | 0.779 |
| 400 | 10 | 0.6 | RBF | 0.0001 | 0.516 | 0.487 | 0.551 | 0.764 |
| 400 | 10 | 0.6 | RBF | 0.001 | 0.530 | 0.491 | 0.555 | 0.762 |
| 400 | 10 | 0.6 | RBF | 0.01 | 0.096 | 0.121 | 0.508 | 0.476 |
| 400 | 10 | 0.8 | LIN | - | 0.543 | 0.502 | 0.549 | 0.778 |
| 400 | 10 | 0.8 | RBF | 0.0001 | 0.516 | 0.487 | 0.551 | 0.764 |
| 400 | 10 | 0.8 | RBF | 0.001 | 0.530 | 0.491 | 0.555 | 0.762 |
| 400 | 10 | 0.8 | RBF | 0.01 | 0.095 | 0.121 | 0.508 | 0.475 |
| 400 | 10 | 1.0 | LIN | - | 0.515 | 0.477 | 0.545 | 0.777 |
| 400 | 10 | 1.0 | RBF | 0.0001 | 0.516 | 0.487 | 0.551 | 0.764 |
| 400 | 10 | 1.0 | RBF | 0.001 | 0.530 | 0.491 | 0.555 | 0.762 |
| 400 | 10 | 1.0 | RBF | 0.01 | 0.084 | 0.111 | 0.507 | 0.474 |
| 400 | 10 | 10 | LIN | - | 0.528 | 0.500 | 0.547 | 0.785 |
| 400 | 10 | 10 | RBF | 0.0001 | 0.516 | 0.487 | 0.551 | 0.764 |
| 400 | 10 | 10 | RBF | 0.001 | 0.530 | 0.491 | 0.555 | 0.762 |
| 400 | 10 | 10 | RBF | 0.01 | 0.058 | 0.091 | 0.507 | 0.471 |
| 400 | 10 | 50 | LIN | - | 0.509 | 0.482 | 0.552 | 0.721 |
| 400 | 10 | 50 | RBF | 0.0001 | 0.516 | 0.487 | 0.551 | 0.764 |
| 400 | 10 | 50 | RBF | 0.001 | 0.530 | 0.491 | 0.555 | 0.762 |
| 400 | 10 | 50 | RBF | 0.01 | 0.049 | 0.084 | 0.505 | 0.469 |
| 400 | 10 | 100 | LIN | - | 0.509 | 0.475 | 0.552 | 0.688 |
| 400 | 10 | 100 | RBF | 0.0001 | 0.516 | 0.487 | 0.551 | 0.764 |
| 400 | 10 | 100 | RBF | 0.001 | 0.530 | 0.491 | 0.555 | 0.762 |
| 400 | 10 | 100 | RBF | 0.01 | 0.047 | 0.083 | 0.505 | 0.469 |
| 400 | 15 | 0.001 | LIN | - | 0.336 | 0.333 | 0.531 | 0.706 |
| 400 | 15 | 0.001 | RBF | 0.0001 | 0.520 | 0.491 | 0.552 | 0.771 |
| 400 | 15 | 0.001 | RBF | 0.001 | 0.527 | 0.490 | 0.554 | 0.760 |

Continued on next page

TABLE S17 – continued from previous page

| n | $k$ | $\lambda$ | usim | $\sigma$ | AP@5 | AP@10 | sCI | CI |
|---|---|---|---|---|---|---|---|---|
| 400 | 15 | 0.001 | RBF | 0.01 | 0.235 | 0.249 | 0.512 | 0.528 |
| 400 | 15 | 0.01 | LIN | - | 0.421 | 0.409 | 0.550 | 0.762 |
| 400 | 15 | 0.01 | RBF | 0.0001 | 0.520 | 0.491 | 0.552 | 0.771 |
| 400 | 15 | 0.01 | RBF | 0.001 | 0.527 | 0.490 | 0.554 | 0.760 |
| 400 | 15 | 0.01 | RBF | 0.01 | 0.183 | 0.201 | 0.509 | 0.503 |
| 400 | 15 | 0.1 | LIN | - | 0.510 | 0.472 | 0.558 | 0.769 |
| 400 | 15 | 0.1 | RBF | 0.0001 | 0.520 | 0.491 | 0.552 | 0.771 |
| 400 | 15 | 0.1 | RBF | 0.001 | 0.527 | 0.490 | 0.554 | 0.760 |
| 400 | 15 | 0.1 | RBF | 0.01 | 0.135 | 0.158 | 0.509 | 0.485 |
| 400 | 15 | 0.2 | LIN | - | 0.497 | 0.464 | 0.555 | 0.769 |
| 400 | 15 | 0.2 | RBF | 0.0001 | 0.520 | 0.491 | 0.552 | 0.771 |
| 400 | 15 | 0.2 | RBF | 0.001 | 0.527 | 0.490 | 0.554 | 0.760 |
| 400 | 15 | 0.2 | RBF | 0.01 | 0.122 | 0.147 | 0.509 | 0.481 |
| 400 | 15 | 0.4 | LIN | - | 0.519 | 0.483 | 0.557 | 0.772 |
| 400 | 15 | 0.4 | RBF | 0.0001 | 0.520 | 0.491 | 0.552 | 0.771 |
| 400 | 15 | 0.4 | RBF | 0.001 | 0.527 | 0.490 | 0.554 | 0.760 |
| 400 | 15 | 0.4 | RBF | 0.01 | 0.108 | 0.133 | 0.508 | 0.478 |
| 400 | 15 | 0.6 | LIN | - | 0.491 | 0.469 | 0.557 | 0.773 |
| 400 | 15 | 0.6 | RBF | 0.0001 | 0.520 | 0.491 | 0.552 | 0.771 |
| 400 | 15 | 0.6 | RBF | 0.001 | 0.527 | 0.490 | 0.554 | 0.760 |
| 400 | 15 | 0.6 | RBF | 0.01 | 0.095 | 0.123 | 0.507 | 0.476 |
| 400 | 15 | 0.8 | LIN | - | 0.534 | 0.494 | 0.555 | 0.775 |
| 400 | 15 | 0.8 | RBF | 0.0001 | 0.520 | 0.491 | 0.552 | 0.771 |
| 400 | 15 | 0.8 | RBF | 0.001 | 0.527 | 0.490 | 0.554 | 0.760 |
| 400 | 15 | 0.8 | RBF | 0.01 | 0.093 | 0.120 | 0.508 | 0.475 |
| 400 | 15 | 1.0 | LIN | - | 0.512 | 0.472 | 0.555 | 0.774 |
| 400 | 15 | 1.0 | RBF | 0.0001 | 0.520 | 0.491 | 0.552 | 0.771 |
| 400 | 15 | 1.0 | RBF | 0.001 | 0.527 | 0.490 | 0.554 | 0.760 |
| 400 | 15 | 1.0 | RBF | 0.01 | 0.083 | 0.110 | 0.507 | 0.474 |
| 400 | 15 | 10 | LIN | - | 0.523 | 0.482 | 0.547 | 0.778 |
| 400 | 15 | 10 | RBF | 0.0001 | 0.520 | 0.491 | 0.552 | 0.771 |
| 400 | 15 | 10 | RBF | 0.001 | 0.527 | 0.490 | 0.554 | 0.760 |
| 400 | 15 | 10 | RBF | 0.01 | 0.057 | 0.091 | 0.506 | 0.471 |
| 400 | 15 | 50 | LIN | - | 0.532 | 0.501 | 0.552 | 0.743 |
| 400 | 15 | 50 | RBF | 0.0001 | 0.520 | 0.491 | 0.552 | 0.771 |
| 400 | 15 | 50 | RBF | 0.001 | 0.527 | 0.490 | 0.554 | 0.760 |
| 400 | 15 | 50 | RBF | 0.01 | 0.050 | 0.085 | 0.505 | 0.470 |
| 400 | 15 | 100 | LIN | - | 0.515 | 0.485 | 0.552 | 0.702 |
| 400 | 15 | 100 | RBF | 0.0001 | 0.520 | 0.491 | 0.552 | 0.771 |
| 400 | 15 | 100 | RBF | 0.001 | 0.527 | 0.490 | 0.554 | 0.760 |
| 400 | 15 | 100 | RBF | 0.01 | 0.049 | 0.084 | 0.504 | 0.469 |

The columns corresponding to “$k$”, “$\lambda$”, “usim”, and “$\sigma$” have the two hyperparameters, cell line similarity function, and parameter for RBF cell line similarity, respectively, for KRL.

**TABLE S18:** pLETORg Performance on New Cell Lines ($\theta$ = 2)

| n | $l$ | $\alpha$ | $\beta$ | $\gamma$ | usim | $\sigma$ | AP@5 | AP@10 | sCI | CI |
|---|---|---|---|---|---|---|---|---|---|---|
| 50 | 5 | 0.00 | 0.1 | 10.0 | RBF | 10.0 | 0.866 | 0.776 | 0.628 | 0.740 |
| 50 | 5 | 0.00 | 0.1 | 100.0 | RBF | 10.0 | 0.866 | 0.776 | 0.628 | 0.740 |
| 50 | 5 | 0.05 | 0.1 | 10.0 | RBF | 10.0 | 0.868 | 0.807 | 0.619 | 0.630 |
| 50 | 5 | 0.05 | 0.1 | 100.0 | RBF | 10.0 | 0.865 | 0.777 | 0.627 | 0.742 |
| 50 | 5 | 0.10 | 0.1 | 10.0 | RBF | 10.0 | 0.865 | 0.804 | 0.618 | 0.634 |
| 50 | 5 | 0.10 | 0.1 | 100.0 | RBF | 10.0 | 0.876 | 0.800 | 0.615 | 0.628 |
| 50 | 5 | 0.50 | 0.1 | 10.0 | RBF | 10.0 | 0.864 | 0.776 | 0.632 | 0.761 |
| 50 | 5 | 0.50 | 0.1 | 100.0 | RBF | 10.0 | 0.864 | 0.776 | 0.631 | 0.761 |
| 50 | 5 | 1.00 | 0.1 | 10.0 | RBF | 10.0 | 0.857 | 0.783 | 0.638 | 0.791 |
| 50 | 5 | 1.00 | 0.1 | 100.0 | RBF | 10.0 | 0.863 | 0.780 | 0.638 | 0.792 |
| 50 | 10 | 0.00 | 0.1 | 10.0 | RBF | 10.0 | 0.865 | 0.796 | 0.626 | 0.669 |
| 50 | 10 | 0.00 | 0.1 | 100.0 | RBF | 10.0 | 0.866 | 0.800 | 0.625 | 0.667 |
| 50 | 10 | 0.05 | 0.1 | 10.0 | RBF | 10.0 | 0.864 | 0.796 | 0.623 | 0.674 |
| 50 | 10 | 0.05 | 0.1 | 100.0 | RBF | 10.0 | 0.863 | 0.796 | 0.619 | 0.672 |
| 50 | 10 | 0.10 | 0.1 | 10.0 | RBF | 10.0 | 0.861 | 0.804 | 0.613 | 0.788 |
| 50 | 10 | 0.10 | 0.1 | 100.0 | RBF | 10.0 | 0.861 | 0.804 | 0.613 | 0.788 |
| 50 | 10 | 0.50 | 0.1 | 10.0 | RBF | 10.0 | 0.859 | 0.780 | 0.617 | 0.769 |
| 50 | 10 | 0.50 | 0.1 | 100.0 | RBF | 10.0 | 0.866 | 0.776 | 0.625 | 0.677 |
| 50 | 10 | 1.00 | 0.1 | 10.0 | RBF | 10.0 | 0.853 | 0.791 | 0.611 | 0.792 |
| 50 | 10 | 1.00 | 0.1 | 100.0 | RBF | 10.0 | 0.853 | 0.794 | 0.611 | 0.792 |
| 50 | 15 | 0.00 | 0.1 | 10.0 | RBF | 10.0 | 0.863 | 0.785 | 0.618 | 0.755 |
| 50 | 15 | 0.00 | 0.1 | 100.0 | RBF | 10.0 | 0.864 | 0.784 | 0.621 | 0.745 |
| 50 | 15 | 0.05 | 0.1 | 10.0 | RBF | 10.0 | 0.869 | 0.802 | 0.623 | 0.682 |
| 50 | 15 | 0.05 | 0.1 | 100.0 | RBF | 10.0 | 0.866 | 0.802 | 0.622 | 0.680 |
| 50 | 15 | 0.10 | 0.1 | 10.0 | RBF | 10.0 | 0.865 | 0.800 | 0.618 | 0.628 |
| 50 | 15 | 0.10 | 0.1 | 100.0 | RBF | 10.0 | 0.863 | 0.784 | 0.615 | 0.759 |
| 50 | 15 | 0.50 | 0.1 | 10.0 | RBF | 10.0 | 0.858 | 0.796 | 0.618 | 0.640 |
| 50 | 15 | 0.50 | 0.1 | 100.0 | RBF | 10.0 | 0.859 | 0.798 | 0.620 | 0.649 |
| 50 | 15 | 1.00 | 0.1 | 10.0 | RBF | 10.0 | 0.847 | 0.780 | 0.613 | 0.792 |
| 50 | 15 | 1.00 | 0.1 | 100.0 | RBF | 10.0 | 0.846 | 0.779 | 0.610 | 0.792 |
| 100 | 5 | 0.00 | 0.1 | 10.0 | RBF | 10.0 | 0.853 | 0.770 | 0.615 | 0.772 |
| 100 | 5 | 0.00 | 0.1 | 100.0 | RBF | 10.0 | 0.853 | 0.772 | 0.612 | 0.782 |
| 100 | 5 | 0.05 | 0.1 | 10.0 | RBF | 10.0 | 0.856 | 0.763 | 0.622 | 0.741 |
| 100 | 5 | 0.05 | 0.1 | 100.0 | RBF | 10.0 | 0.855 | 0.765 | 0.622 | 0.741 |
| 100 | 5 | 0.10 | 0.1 | 10.0 | RBF | 10.0 | 0.858 | 0.764 | 0.623 | 0.743 |
| 100 | 5 | 0.10 | 0.1 | 100.0 | RBF | 10.0 | 0.863 | 0.785 | 0.626 | 0.626 |
| 100 | 5 | 0.50 | 0.1 | 10.0 | RBF | 10.0 | 0.855 | 0.764 | 0.628 | 0.760 |
| 100 | 5 | 0.50 | 0.1 | 100.0 | RBF | 10.0 | 0.856 | 0.765 | 0.627 | 0.760 |
| 100 | 5 | 1.00 | 0.1 | 10.0 | RBF | 10.0 | 0.846 | 0.764 | 0.626 | 0.788 |
| 100 | 5 | 1.00 | 0.1 | 100.0 | RBF | 10.0 | 0.848 | 0.765 | 0.623 | 0.788 |
| 100 | 10 | 0.00 | 0.1 | 10.0 | RBF | 10.0 | 0.853 | 0.768 | 0.621 | 0.746 |
| 100 | 10 | 0.00 | 0.1 | 100.0 | RBF | 10.0 | 0.856 | 0.772 | 0.611 | 0.784 |
| 100 | 10 | 0.05 | 0.1 | 10.0 | RBF | 10.0 | 0.856 | 0.769 | 0.619 | 0.750 |
| 100 | 10 | 0.05 | 0.1 | 100.0 | RBF | 10.0 | 0.855 | 0.768 | 0.618 | 0.750 |
| 100 | 10 | 0.10 | 0.1 | 10.0 | RBF | 10.0 | 0.857 | 0.770 | 0.618 | 0.752 |
| 100 | 10 | 0.10 | 0.1 | 100.0 | RBF | 10.0 | 0.857 | 0.769 | 0.617 | 0.752 |
| 100 | 10 | 0.50 | 0.1 | 10.0 | RBF | 10.0 | 0.858 | 0.783 | 0.623 | 0.645 |
| 100 | 10 | 0.50 | 0.1 | 100.0 | RBF | 10.0 | 0.870 | 0.770 | 0.630 | 0.678 |
| 100 | 10 | 1.00 | 0.1 | 10.0 | RBF | 10.0 | 0.851 | 0.763 | 0.610 | 0.788 |
| 100 | 10 | 1.00 | 0.1 | 100.0 | RBF | 10.0 | 0.853 | 0.767 | 0.609 | 0.788 |
| 100 | 15 | 0.00 | 0.1 | 10.0 | RBF | 10.0 | 0.853 | 0.765 | 0.621 | 0.754 |
| 100 | 15 | 0.00 | 0.1 | 100.0 | RBF | 10.0 | 0.855 | 0.770 | 0.625 | 0.738 |
| 100 | 15 | 0.05 | 0.1 | 10.0 | RBF | 10.0 | 0.854 | 0.764 | 0.620 | 0.755 |
| 100 | 15 | 0.05 | 0.1 | 100.0 | RBF | 10.0 | 0.853 | 0.764 | 0.620 | 0.755 |
| 100 | 15 | 0.10 | 0.1 | 10.0 | RBF | 10.0 | 0.856 | 0.766 | 0.620 | 0.756 |
| 100 | 15 | 0.10 | 0.1 | 100.0 | RBF | 10.0 | 0.860 | 0.777 | 0.622 | 0.616 |
| 100 | 15 | 0.50 | 0.1 | 10.0 | RBF | 10.0 | 0.856 | 0.779 | 0.628 | 0.647 |

Continued on next page

TABLE S18 – continued from previous page

| n | $l$ | $\alpha$ | $\beta$ | $\gamma$ | usim | $\sigma$ | AP@5 | AP@10 | sCI | CI |
|---|---|---|---|---|---|---|---|---|---|---|
| 100 | 15 | 0.50 | 0.1 | 100.0 | RBF | 10.0 | 0.855 | 0.761 | 0.632 | 0.684 |
| 100 | 15 | 1.00 | 0.1 | 10.0 | RBF | 10.0 | 0.848 | 0.741 | 0.632 | 0.763 |
| 100 | 15 | 1.00 | 0.1 | 100.0 | RBF | 10.0 | 0.842 | 0.752 | 0.620 | 0.785 |
| 150 | 5 | 0.00 | 0.1 | 10.0 | RBF | 10.0 | 0.860 | 0.785 | 0.619 | 0.774 |
| 150 | 5 | 0.00 | 0.1 | 100.0 | RBF | 10.0 | 0.859 | 0.789 | 0.616 | 0.784 |
| 150 | 5 | 0.05 | 0.1 | 10.0 | RBF | 10.0 | 0.858 | 0.789 | 0.617 | 0.784 |
| 150 | 5 | 0.05 | 0.1 | 100.0 | RBF | 10.0 | 0.858 | 0.789 | 0.617 | 0.784 |
| 150 | 5 | 0.10 | 0.1 | 10.0 | RBF | 10.0 | 0.860 | 0.794 | 0.637 | 0.639 |
| 150 | 5 | 0.10 | 0.1 | 100.0 | RBF | 10.0 | 0.860 | 0.798 | 0.636 | 0.629 |
| 150 | 5 | 0.50 | 0.1 | 10.0 | RBF | 10.0 | 0.869 | 0.789 | 0.647 | 0.666 |
| 150 | 5 | 0.50 | 0.1 | 100.0 | RBF | 10.0 | 0.863 | 0.782 | 0.632 | 0.763 |
| 150 | 5 | 1.00 | 0.1 | 10.0 | RBF | 10.0 | 0.859 | 0.775 | 0.633 | 0.789 |
| 150 | 5 | 1.00 | 0.1 | 100.0 | RBF | 10.0 | 0.863 | 0.780 | 0.629 | 0.789 |
| 150 | 10 | 0.00 | 0.1 | 10.0 | RBF | 10.0 | 0.860 | 0.780 | 0.624 | 0.750 |
| 150 | 10 | 0.00 | 0.1 | 100.0 | RBF | 10.0 | 0.858 | 0.776 | 0.627 | 0.744 |
| 150 | 10 | 0.05 | 0.1 | 10.0 | RBF | 10.0 | 0.860 | 0.780 | 0.623 | 0.754 |
| 150 | 10 | 0.05 | 0.1 | 100.0 | RBF | 10.0 | 0.860 | 0.780 | 0.623 | 0.754 |
| 150 | 10 | 0.10 | 0.1 | 10.0 | RBF | 10.0 | 0.860 | 0.781 | 0.623 | 0.755 |
| 150 | 10 | 0.10 | 0.1 | 100.0 | RBF | 10.0 | 0.860 | 0.780 | 0.624 | 0.755 |
| 150 | 10 | 0.50 | 0.1 | 10.0 | RBF | 10.0 | 0.867 | 0.788 | 0.633 | 0.645 |
| 150 | 10 | 0.50 | 0.1 | 100.0 | RBF | 10.0 | 0.870 | 0.789 | 0.642 | 0.680 |
| 150 | 10 | 1.00 | 0.1 | 10.0 | RBF | 10.0 | 0.852 | 0.771 | 0.620 | 0.789 |
| 150 | 10 | 1.00 | 0.1 | 100.0 | RBF | 10.0 | 0.853 | 0.775 | 0.615 | 0.789 |
| 150 | 15 | 0.00 | 0.1 | 10.0 | RBF | 10.0 | 0.865 | 0.784 | 0.619 | 0.780 |
| 150 | 15 | 0.00 | 0.1 | 100.0 | RBF | 10.0 | 0.858 | 0.778 | 0.617 | 0.786 |
| 150 | 15 | 0.05 | 0.1 | 10.0 | RBF | 10.0 | 0.860 | 0.782 | 0.625 | 0.758 |
| 150 | 15 | 0.05 | 0.1 | 100.0 | RBF | 10.0 | 0.861 | 0.783 | 0.625 | 0.758 |
| 150 | 15 | 0.10 | 0.1 | 10.0 | RBF | 10.0 | 0.861 | 0.782 | 0.625 | 0.760 |
| 150 | 15 | 0.10 | 0.1 | 100.0 | RBF | 10.0 | 0.864 | 0.788 | 0.633 | 0.614 |
| 150 | 15 | 0.50 | 0.1 | 10.0 | RBF | 10.0 | 0.857 | 0.789 | 0.637 | 0.633 |
| 150 | 15 | 0.50 | 0.1 | 100.0 | RBF | 10.0 | 0.856 | 0.783 | 0.645 | 0.687 |
| 150 | 15 | 1.00 | 0.1 | 10.0 | RBF | 10.0 | 0.851 | 0.779 | 0.618 | 0.788 |
| 150 | 15 | 1.00 | 0.1 | 100.0 | RBF | 10.0 | 0.849 | 0.783 | 0.616 | 0.789 |
| 200 | 5 | 0.00 | 0.1 | 10.0 | RBF | 10.0 | 0.845 | 0.778 | 0.623 | 0.777 |
| 200 | 5 | 0.00 | 0.1 | 100.0 | RBF | 10.0 | 0.842 | 0.780 | 0.618 | 0.786 |
| 200 | 5 | 0.05 | 0.1 | 10.0 | RBF | 10.0 | 0.843 | 0.789 | 0.643 | 0.665 |
| 200 | 5 | 0.05 | 0.1 | 100.0 | RBF | 10.0 | 0.844 | 0.786 | 0.641 | 0.614 |
| 200 | 5 | 0.10 | 0.1 | 10.0 | RBF | 10.0 | 0.847 | 0.772 | 0.633 | 0.750 |
| 200 | 5 | 0.10 | 0.1 | 100.0 | RBF | 10.0 | 0.845 | 0.771 | 0.632 | 0.750 |
| 200 | 5 | 0.50 | 0.1 | 10.0 | RBF | 10.0 | 0.848 | 0.780 | 0.645 | 0.659 |
| 200 | 5 | 0.50 | 0.1 | 100.0 | RBF | 10.0 | 0.849 | 0.779 | 0.645 | 0.650 |
| 200 | 5 | 1.00 | 0.1 | 10.0 | RBF | 10.0 | 0.848 | 0.776 | 0.630 | 0.790 |
| 200 | 5 | 1.00 | 0.1 | 100.0 | RBF | 10.0 | 0.849 | 0.777 | 0.630 | 0.790 |
| 200 | 10 | 0.00 | 0.1 | 10.0 | RBF | 10.0 | 0.846 | 0.770 | 0.629 | 0.753 |
| 200 | 10 | 0.00 | 0.1 | 100.0 | RBF | 10.0 | 0.846 | 0.770 | 0.632 | 0.740 |
| 200 | 10 | 0.05 | 0.1 | 10.0 | RBF | 10.0 | 0.847 | 0.771 | 0.629 | 0.757 |
| 200 | 10 | 0.05 | 0.1 | 100.0 | RBF | 10.0 | 0.847 | 0.771 | 0.629 | 0.757 |
| 200 | 10 | 0.10 | 0.1 | 10.0 | RBF | 10.0 | 0.849 | 0.771 | 0.629 | 0.758 |
| 200 | 10 | 0.10 | 0.1 | 100.0 | RBF | 10.0 | 0.849 | 0.770 | 0.629 | 0.759 |
| 200 | 10 | 0.50 | 0.1 | 10.0 | RBF | 10.0 | 0.847 | 0.776 | 0.637 | 0.651 |
| 200 | 10 | 0.50 | 0.1 | 100.0 | RBF | 10.0 | 0.847 | 0.777 | 0.644 | 0.683 |
| 200 | 10 | 1.00 | 0.1 | 10.0 | RBF | 10.0 | 0.841 | 0.768 | 0.622 | 0.790 |
| 200 | 10 | 1.00 | 0.1 | 100.0 | RBF | 10.0 | 0.837 | 0.769 | 0.621 | 0.790 |
| 200 | 15 | 0.00 | 0.1 | 10.0 | RBF | 10.0 | 0.852 | 0.777 | 0.624 | 0.784 |
| 200 | 15 | 0.00 | 0.1 | 100.0 | RBF | 10.0 | 0.848 | 0.771 | 0.632 | 0.728 |
| 200 | 15 | 0.05 | 0.1 | 10.0 | RBF | 10.0 | 0.851 | 0.776 | 0.628 | 0.762 |
| 200 | 15 | 0.05 | 0.1 | 100.0 | RBF | 10.0 | 0.851 | 0.776 | 0.628 | 0.762 |
| 200 | 15 | 0.10 | 0.1 | 10.0 | RBF | 10.0 | 0.852 | 0.776 | 0.629 | 0.763 |

Continued on next page

TABLE S18 – continued from previous page

| n | $l$ | $\alpha$ | $\beta$ | $\gamma$ | usim | $\sigma$ | AP@5 | AP@10 | sCI | CI |
|---|---|---|---|---|---|---|---|---|---|---|
| 200 | 15 | 0.10 | 0.1 | 100.0 | RBF | 10.0 | 0.851 | 0.776 | 0.629 | 0.763 |
| 200 | 15 | 0.50 | 0.1 | 10.0 | RBF | 10.0 | 0.846 | 0.771 | 0.621 | 0.788 |
| 200 | 15 | 0.50 | 0.1 | 100.0 | RBF | 10.0 | 0.849 | 0.782 | 0.641 | 0.652 |
| 200 | 15 | 1.00 | 0.1 | 10.0 | RBF | 10.0 | 0.839 | 0.772 | 0.621 | 0.790 |
| 200 | 15 | 1.00 | 0.1 | 100.0 | RBF | 10.0 | 0.837 | 0.769 | 0.619 | 0.790 |
| 250 | 5 | 0.00 | 0.1 | 10.0 | RBF | 10.0 | 0.847 | 0.781 | 0.622 | 0.778 |
| 250 | 5 | 0.00 | 0.1 | 100.0 | RBF | 10.0 | 0.847 | 0.783 | 0.616 | 0.787 |
| 250 | 5 | 0.05 | 0.1 | 10.0 | RBF | 10.0 | 0.847 | 0.783 | 0.616 | 0.787 |
| 250 | 5 | 0.05 | 0.1 | 100.0 | RBF | 10.0 | 0.847 | 0.783 | 0.616 | 0.787 |
| 250 | 5 | 0.10 | 0.1 | 10.0 | RBF | 10.0 | 0.847 | 0.784 | 0.615 | 0.788 |
| 250 | 5 | 0.10 | 0.1 | 100.0 | RBF | 10.0 | 0.848 | 0.795 | 0.640 | 0.612 |
| 250 | 5 | 0.50 | 0.1 | 10.0 | RBF | 10.0 | 0.861 | 0.798 | 0.644 | 0.661 |
| 250 | 5 | 0.50 | 0.1 | 100.0 | RBF | 10.0 | 0.853 | 0.779 | 0.635 | 0.768 |
| 250 | 5 | 1.00 | 0.1 | 10.0 | RBF | 10.0 | 0.853 | 0.777 | 0.628 | 0.791 |
| 250 | 5 | 1.00 | 0.1 | 100.0 | RBF | 10.0 | 0.852 | 0.777 | 0.627 | 0.791 |
| 250 | 10 | 0.00 | 0.1 | 10.0 | RBF | 10.0 | 0.855 | 0.782 | 0.618 | 0.784 |
| 250 | 10 | 0.00 | 0.1 | 100.0 | RBF | 10.0 | 0.852 | 0.782 | 0.618 | 0.788 |
| 250 | 10 | 0.05 | 0.1 | 10.0 | RBF | 10.0 | 0.853 | 0.777 | 0.627 | 0.760 |
| 250 | 10 | 0.05 | 0.1 | 100.0 | RBF | 10.0 | 0.852 | 0.783 | 0.618 | 0.789 |
| 250 | 10 | 0.10 | 0.1 | 10.0 | RBF | 10.0 | 0.853 | 0.778 | 0.627 | 0.761 |
| 250 | 10 | 0.10 | 0.1 | 100.0 | RBF | 10.0 | 0.853 | 0.778 | 0.627 | 0.761 |
| 250 | 10 | 0.50 | 0.1 | 10.0 | RBF | 10.0 | 0.853 | 0.782 | 0.618 | 0.790 |
| 250 | 10 | 0.50 | 0.1 | 100.0 | RBF | 10.0 | 0.853 | 0.782 | 0.618 | 0.790 |
| 250 | 10 | 1.00 | 0.1 | 10.0 | RBF | 10.0 | 0.850 | 0.773 | 0.622 | 0.791 |
| 250 | 10 | 1.00 | 0.1 | 100.0 | RBF | 10.0 | 0.850 | 0.776 | 0.620 | 0.792 |
| 250 | 15 | 0.00 | 0.1 | 10.0 | RBF | 10.0 | 0.856 | 0.781 | 0.621 | 0.785 |
| 250 | 15 | 0.00 | 0.1 | 100.0 | RBF | 10.0 | 0.852 | 0.780 | 0.618 | 0.789 |
| 250 | 15 | 0.05 | 0.1 | 10.0 | RBF | 10.0 | 0.852 | 0.781 | 0.627 | 0.765 |
| 250 | 15 | 0.05 | 0.1 | 100.0 | RBF | 10.0 | 0.853 | 0.781 | 0.628 | 0.756 |
| 250 | 15 | 0.10 | 0.1 | 10.0 | RBF | 10.0 | 0.853 | 0.781 | 0.627 | 0.766 |
| 250 | 15 | 0.10 | 0.1 | 100.0 | RBF | 10.0 | 0.858 | 0.794 | 0.632 | 0.616 |
| 250 | 15 | 0.50 | 0.1 | 10.0 | RBF | 10.0 | 0.849 | 0.787 | 0.638 | 0.639 |
| 250 | 15 | 0.50 | 0.1 | 100.0 | RBF | 10.0 | 0.853 | 0.783 | 0.641 | 0.633 |
| 250 | 15 | 1.00 | 0.1 | 10.0 | RBF | 10.0 | 0.847 | 0.775 | 0.620 | 0.791 |
| 250 | 15 | 1.00 | 0.1 | 100.0 | RBF | 10.0 | 0.846 | 0.776 | 0.618 | 0.791 |
| 300 | 5 | 0.00 | 0.1 | 10.0 | RBF | 10.0 | 0.845 | 0.778 | 0.623 | 0.780 |
| 300 | 5 | 0.00 | 0.1 | 100.0 | RBF | 10.0 | 0.847 | 0.780 | 0.618 | 0.788 |
| 300 | 5 | 0.05 | 0.1 | 10.0 | RBF | 10.0 | 0.848 | 0.780 | 0.619 | 0.788 |
| 300 | 5 | 0.05 | 0.1 | 100.0 | RBF | 10.0 | 0.848 | 0.780 | 0.619 | 0.788 |
| 300 | 5 | 0.10 | 0.1 | 10.0 | RBF | 10.0 | 0.848 | 0.780 | 0.618 | 0.788 |
| 300 | 5 | 0.10 | 0.1 | 100.0 | RBF | 10.0 | 0.852 | 0.787 | 0.638 | 0.613 |
| 300 | 5 | 0.50 | 0.1 | 10.0 | RBF | 10.0 | 0.855 | 0.787 | 0.643 | 0.659 |
| 300 | 5 | 0.50 | 0.1 | 100.0 | RBF | 10.0 | 0.852 | 0.785 | 0.645 | 0.650 |
| 300 | 5 | 1.00 | 0.1 | 10.0 | RBF | 10.0 | 0.851 | 0.772 | 0.631 | 0.791 |
| 300 | 5 | 1.00 | 0.1 | 100.0 | RBF | 10.0 | 0.852 | 0.773 | 0.629 | 0.792 |
| 300 | 10 | 0.00 | 0.1 | 10.0 | RBF | 10.0 | 0.851 | 0.778 | 0.621 | 0.786 |
| 300 | 10 | 0.00 | 0.1 | 100.0 | RBF | 10.0 | 0.851 | 0.779 | 0.621 | 0.789 |
| 300 | 10 | 0.05 | 0.1 | 10.0 | RBF | 10.0 | 0.852 | 0.780 | 0.621 | 0.789 |
| 300 | 10 | 0.05 | 0.1 | 100.0 | RBF | 10.0 | 0.851 | 0.779 | 0.621 | 0.789 |
| 300 | 10 | 0.10 | 0.1 | 10.0 | RBF | 10.0 | 0.853 | 0.780 | 0.621 | 0.789 |
| 300 | 10 | 0.10 | 0.1 | 100.0 | RBF | 10.0 | 0.853 | 0.780 | 0.621 | 0.789 |
| 300 | 10 | 0.50 | 0.1 | 10.0 | RBF | 10.0 | 0.856 | 0.774 | 0.627 | 0.776 |
| 300 | 10 | 0.50 | 0.1 | 100.0 | RBF | 10.0 | 0.852 | 0.779 | 0.622 | 0.791 |
| 300 | 10 | 1.00 | 0.1 | 10.0 | RBF | 10.0 | 0.849 | 0.770 | 0.627 | 0.792 |
| 300 | 10 | 1.00 | 0.1 | 100.0 | RBF | 10.0 | 0.846 | 0.773 | 0.625 | 0.792 |
| 300 | 15 | 0.00 | 0.1 | 10.0 | RBF | 10.0 | 0.853 | 0.780 | 0.621 | 0.788 |
| 300 | 15 | 0.00 | 0.1 | 100.0 | RBF | 10.0 | 0.853 | 0.780 | 0.622 | 0.789 |
| 300 | 15 | 0.05 | 0.1 | 10.0 | RBF | 10.0 | 0.856 | 0.780 | 0.628 | 0.767 |

Continued on next page

TABLE S18 – continued from previous page

| n | $l$ | $\alpha$ | $\beta$ | $\gamma$ | usim | $\sigma$ | AP@5 | AP@10 | sCI | CI |
|---|---|---|---|---|---|---|---|---|---|---|
| 300 | 15 | 0.05 | 0.1 | 100.0 | RBF | 10.0 | 0.853 | 0.780 | 0.622 | 0.790 |
| 300 | 15 | 0.10 | 0.1 | 10.0 | RBF | 10.0 | 0.855 | 0.782 | 0.627 | 0.768 |
| 300 | 15 | 0.10 | 0.1 | 100.0 | RBF | 10.0 | 0.856 | 0.779 | 0.629 | 0.761 |
| 300 | 15 | 0.50 | 0.1 | 10.0 | RBF | 10.0 | 0.849 | 0.781 | 0.621 | 0.791 |
| 300 | 15 | 0.50 | 0.1 | 100.0 | RBF | 10.0 | 0.850 | 0.781 | 0.621 | 0.791 |
| 300 | 15 | 1.00 | 0.1 | 10.0 | RBF | 10.0 | 0.849 | 0.769 | 0.624 | 0.792 |
| 300 | 15 | 1.00 | 0.1 | 100.0 | RBF | 10.0 | 0.847 | 0.776 | 0.623 | 0.792 |
| 350 | 5 | 0.00 | 0.1 | 10.0 | RBF | 10.0 | 0.838 | 0.771 | 0.621 | 0.781 |
| 350 | 5 | 0.00 | 0.1 | 100.0 | RBF | 10.0 | 0.839 | 0.771 | 0.620 | 0.786 |
| 350 | 5 | 0.05 | 0.1 | 10.0 | RBF | 10.0 | 0.840 | 0.771 | 0.619 | 0.786 |
| 350 | 5 | 0.05 | 0.1 | 100.0 | RBF | 10.0 | 0.840 | 0.771 | 0.620 | 0.786 |
| 350 | 5 | 0.10 | 0.1 | 10.0 | RBF | 10.0 | 0.841 | 0.781 | 0.644 | 0.673 |
| 350 | 5 | 0.10 | 0.1 | 100.0 | RBF | 10.0 | 0.840 | 0.771 | 0.619 | 0.786 |
| 350 | 5 | 0.50 | 0.1 | 10.0 | RBF | 10.0 | 0.846 | 0.770 | 0.635 | 0.769 |
| 350 | 5 | 0.50 | 0.1 | 100.0 | RBF | 10.0 | 0.845 | 0.771 | 0.635 | 0.769 |
| 350 | 5 | 1.00 | 0.1 | 10.0 | RBF | 10.0 | 0.840 | 0.765 | 0.630 | 0.790 |
| 350 | 5 | 1.00 | 0.1 | 100.0 | RBF | 10.0 | 0.841 | 0.764 | 0.628 | 0.790 |
| 350 | 10 | 0.00 | 0.1 | 10.0 | RBF | 10.0 | 0.842 | 0.771 | 0.621 | 0.786 |
| 350 | 10 | 0.00 | 0.1 | 100.0 | RBF | 10.0 | 0.843 | 0.771 | 0.620 | 0.788 |
| 350 | 10 | 0.05 | 0.1 | 10.0 | RBF | 10.0 | 0.845 | 0.767 | 0.628 | 0.762 |
| 350 | 10 | 0.05 | 0.1 | 100.0 | RBF | 10.0 | 0.843 | 0.771 | 0.620 | 0.788 |
| 350 | 10 | 0.10 | 0.1 | 10.0 | RBF | 10.0 | 0.845 | 0.770 | 0.620 | 0.788 |
| 350 | 10 | 0.10 | 0.1 | 100.0 | RBF | 10.0 | 0.845 | 0.770 | 0.620 | 0.788 |
| 350 | 10 | 0.50 | 0.1 | 10.0 | RBF | 10.0 | 0.844 | 0.769 | 0.621 | 0.789 |
| 350 | 10 | 0.50 | 0.1 | 100.0 | RBF | 10.0 | 0.844 | 0.769 | 0.621 | 0.789 |
| 350 | 10 | 1.00 | 0.1 | 10.0 | RBF | 10.0 | 0.842 | 0.763 | 0.626 | 0.790 |
| 350 | 10 | 1.00 | 0.1 | 100.0 | RBF | 10.0 | 0.841 | 0.766 | 0.625 | 0.791 |
| 350 | 15 | 0.00 | 0.1 | 10.0 | RBF | 10.0 | 0.848 | 0.771 | 0.629 | 0.764 |
| 350 | 15 | 0.00 | 0.1 | 100.0 | RBF | 10.0 | 0.845 | 0.770 | 0.624 | 0.788 |
| 350 | 15 | 0.05 | 0.1 | 10.0 | RBF | 10.0 | 0.846 | 0.771 | 0.629 | 0.767 |
| 350 | 15 | 0.05 | 0.1 | 100.0 | RBF | 10.0 | 0.844 | 0.785 | 0.640 | 0.617 |
| 350 | 15 | 0.10 | 0.1 | 10.0 | RBF | 10.0 | 0.844 | 0.771 | 0.629 | 0.769 |
| 350 | 15 | 0.10 | 0.1 | 100.0 | RBF | 10.0 | 0.844 | 0.769 | 0.623 | 0.788 |
| 350 | 15 | 0.50 | 0.1 | 10.0 | RBF | 10.0 | 0.844 | 0.770 | 0.623 | 0.789 |
| 350 | 15 | 0.50 | 0.1 | 100.0 | RBF | 10.0 | 0.843 | 0.770 | 0.623 | 0.789 |
| 350 | 15 | 1.00 | 0.1 | 10.0 | RBF | 10.0 | 0.842 | 0.768 | 0.627 | 0.790 |
| 350 | 15 | 1.00 | 0.1 | 100.0 | RBF | 10.0 | 0.842 | 0.767 | 0.626 | 0.790 |
| 400 | 5 | 0.00 | 0.1 | 10.0 | RBF | 10.0 | 0.845 | 0.773 | 0.635 | 0.754 |
| 400 | 5 | 0.00 | 0.1 | 100.0 | RBF | 10.0 | 0.843 | 0.777 | 0.621 | 0.787 |
| 400 | 5 | 0.05 | 0.1 | 10.0 | RBF | 10.0 | 0.846 | 0.773 | 0.635 | 0.756 |
| 400 | 5 | 0.05 | 0.1 | 100.0 | RBF | 10.0 | 0.845 | 0.773 | 0.635 | 0.756 |
| 400 | 5 | 0.10 | 0.1 | 10.0 | RBF | 10.0 | 0.846 | 0.788 | 0.650 | 0.674 |
| 400 | 5 | 0.10 | 0.1 | 100.0 | RBF | 10.0 | 0.846 | 0.772 | 0.635 | 0.757 |
| 400 | 5 | 0.50 | 0.1 | 10.0 | RBF | 10.0 | 0.850 | 0.780 | 0.651 | 0.659 |
| 400 | 5 | 0.50 | 0.1 | 100.0 | RBF | 10.0 | 0.844 | 0.777 | 0.650 | 0.644 |
| 400 | 5 | 1.00 | 0.1 | 10.0 | RBF | 10.0 | 0.843 | 0.763 | 0.631 | 0.791 |
| 400 | 5 | 1.00 | 0.1 | 100.0 | RBF | 10.0 | 0.844 | 0.770 | 0.628 | 0.791 |
| 400 | 10 | 0.00 | 0.1 | 10.0 | RBF | 10.0 | 0.847 | 0.773 | 0.623 | 0.789 |
| 400 | 10 | 0.00 | 0.1 | 100.0 | RBF | 10.0 | 0.846 | 0.772 | 0.623 | 0.789 |
| 400 | 10 | 0.05 | 0.1 | 10.0 | RBF | 10.0 | 0.847 | 0.773 | 0.631 | 0.765 |
| 400 | 10 | 0.05 | 0.1 | 100.0 | RBF | 10.0 | 0.847 | 0.775 | 0.640 | 0.734 |
| 400 | 10 | 0.10 | 0.1 | 10.0 | RBF | 10.0 | 0.847 | 0.774 | 0.631 | 0.766 |
| 400 | 10 | 0.10 | 0.1 | 100.0 | RBF | 10.0 | 0.849 | 0.787 | 0.646 | 0.618 |
| 400 | 10 | 0.50 | 0.1 | 10.0 | RBF | 10.0 | 0.849 | 0.773 | 0.629 | 0.777 |
| 400 | 10 | 0.50 | 0.1 | 100.0 | RBF | 10.0 | 0.846 | 0.779 | 0.653 | 0.688 |
| 400 | 10 | 1.00 | 0.1 | 10.0 | RBF | 10.0 | 0.844 | 0.767 | 0.626 | 0.792 |
| 400 | 10 | 1.00 | 0.1 | 100.0 | RBF | 10.0 | 0.845 | 0.770 | 0.623 | 0.792 |
| 400 | 15 | 0.00 | 0.1 | 10.0 | RBF | 10.0 | 0.847 | 0.773 | 0.625 | 0.790 |

Continued on next page

TABLE S18 – continued from previous page

| n | $l$ | $\alpha$ | $\beta$ | $\gamma$ | usim | $\sigma$ | AP@5 | AP@10 | sCI | CI |
|---|---|---|---|---|---|---|---|---|---|---|
| 400 | 15 | 0.00 | 0.1 | 100.0 | RBF | 10.0 | 0.847 | 0.772 | 0.625 | 0.790 |
| 400 | 15 | 0.05 | 0.1 | 10.0 | RBF | 10.0 | 0.848 | 0.776 | 0.632 | 0.770 |
| 400 | 15 | 0.05 | 0.1 | 100.0 | RBF | 10.0 | 0.853 | 0.792 | 0.643 | 0.605 |
| 400 | 15 | 0.10 | 0.1 | 10.0 | RBF | 10.0 | 0.849 | 0.776 | 0.630 | 0.771 |
| 400 | 15 | 0.10 | 0.1 | 100.0 | RBF | 10.0 | 0.848 | 0.789 | 0.645 | 0.617 |
| 400 | 15 | 0.50 | 0.1 | 10.0 | RBF | 10.0 | 0.850 | 0.780 | 0.649 | 0.644 |
| 400 | 15 | 0.50 | 0.1 | 100.0 | RBF | 10.0 | 0.847 | 0.781 | 0.650 | 0.638 |
| 400 | 15 | 1.00 | 0.1 | 10.0 | RBF | 10.0 | 0.843 | 0.768 | 0.628 | 0.792 |
| 400 | 15 | 1.00 | 0.1 | 100.0 | RBF | 10.0 | 0.843 | 0.768 | 0.625 | 0.792 |

The columns corresponding to "$l$", "$\alpha$", "$\beta$", "$\gamma$", "usim", and "$\sigma$" have the latent dimension, weighting factor, latent vector regularization parameter, cell line similarity regularization parameter, cell line similarity function, and parameter for rbf cell line similarity, respectively, for pLETORg.

**TABLE S19:** pLETORg Performance on New Cell Lines ($\theta$ = 5)

| n | d | $\alpha$ | $\beta$ | $\gamma$ | usim | $\sigma$ | AP@5 | AP@10 | sCI | CI |
|---|---|---|---|---|---|---|---|---|---|---|
| 50 | 5 | 0.00 | 0.1 | 10.0 | RBF | 10.0 | 0.963 | 0.910 | 0.639 | 0.674 |
| 50 | 5 | 0.00 | 0.1 | 100.0 | RBF | 10.0 | 0.961 | 0.907 | 0.643 | 0.645 |
| 50 | 5 | 0.05 | 0.1 | 10.0 | RBF | 10.0 | 0.955 | 0.901 | 0.643 | 0.741 |
| 50 | 5 | 0.05 | 0.1 | 100.0 | RBF | 10.0 | 0.955 | 0.902 | 0.644 | 0.741 |
| 50 | 5 | 0.10 | 0.1 | 10.0 | RBF | 10.0 | 0.963 | 0.900 | 0.635 | 0.678 |
| 50 | 5 | 0.10 | 0.1 | 100.0 | RBF | 10.0 | 0.955 | 0.902 | 0.644 | 0.742 |
| 50 | 5 | 0.50 | 0.1 | 10.0 | RBF | 10.0 | 0.955 | 0.901 | 0.647 | 0.758 |
| 50 | 5 | 0.50 | 0.1 | 100.0 | RBF | 10.0 | 0.955 | 0.901 | 0.647 | 0.758 |
| 50 | 5 | 1.00 | 0.1 | 10.0 | RBF | 10.0 | 0.955 | 0.895 | 0.640 | 0.792 |
| 50 | 5 | 1.00 | 0.1 | 100.0 | RBF | 10.0 | 0.952 | 0.894 | 0.637 | 0.792 |
| 50 | 10 | 0.00 | 0.1 | 10.0 | RBF | 10.0 | 0.962 | 0.905 | 0.638 | 0.680 |
| 50 | 10 | 0.00 | 0.1 | 100.0 | RBF | 10.0 | 0.960 | 0.901 | 0.638 | 0.747 |
| 50 | 10 | 0.05 | 0.1 | 10.0 | RBF | 10.0 | 0.965 | 0.902 | 0.638 | 0.681 |
| 50 | 10 | 0.05 | 0.1 | 100.0 | RBF | 10.0 | 0.962 | 0.892 | 0.633 | 0.666 |
| 50 | 10 | 0.10 | 0.1 | 10.0 | RBF | 10.0 | 0.964 | 0.898 | 0.632 | 0.679 |
| 50 | 10 | 0.10 | 0.1 | 100.0 | RBF | 10.0 | 0.960 | 0.902 | 0.639 | 0.750 |
| 50 | 10 | 0.50 | 0.1 | 10.0 | RBF | 10.0 | 0.961 | 0.900 | 0.633 | 0.693 |
| 50 | 10 | 0.50 | 0.1 | 100.0 | RBF | 10.0 | 0.964 | 0.905 | 0.640 | 0.677 |
| 50 | 10 | 1.00 | 0.1 | 10.0 | RBF | 10.0 | 0.953 | 0.900 | 0.625 | 0.792 |
| 50 | 10 | 1.00 | 0.1 | 100.0 | RBF | 10.0 | 0.953 | 0.899 | 0.626 | 0.792 |
| 50 | 15 | 0.00 | 0.1 | 10.0 | RBF | 10.0 | 0.964 | 0.907 | 0.641 | 0.685 |
| 50 | 15 | 0.00 | 0.1 | 100.0 | RBF | 10.0 | 0.964 | 0.907 | 0.641 | 0.683 |
| 50 | 15 | 0.05 | 0.1 | 10.0 | RBF | 10.0 | 0.965 | 0.908 | 0.641 | 0.689 |
| 50 | 15 | 0.05 | 0.1 | 100.0 | RBF | 10.0 | 0.965 | 0.902 | 0.640 | 0.662 |
| 50 | 15 | 0.10 | 0.1 | 10.0 | RBF | 10.0 | 0.959 | 0.905 | 0.642 | 0.754 |
| 50 | 15 | 0.10 | 0.1 | 100.0 | RBF | 10.0 | 0.959 | 0.904 | 0.641 | 0.754 |
| 50 | 15 | 0.50 | 0.1 | 10.0 | RBF | 10.0 | 0.960 | 0.897 | 0.641 | 0.693 |
| 50 | 15 | 0.50 | 0.1 | 100.0 | RBF | 10.0 | 0.964 | 0.904 | 0.644 | 0.686 |
| 50 | 15 | 1.00 | 0.1 | 10.0 | RBF | 10.0 | 0.955 | 0.901 | 0.633 | 0.792 |
| 50 | 15 | 1.00 | 0.1 | 100.0 | RBF | 10.0 | 0.955 | 0.901 | 0.633 | 0.792 |
| 100 | 5 | 0.00 | 0.1 | 10.0 | RBF | 10.0 | 0.952 | 0.910 | 0.651 | 0.671 |
| 100 | 5 | 0.00 | 0.1 | 100.0 | RBF | 10.0 | 0.953 | 0.909 | 0.652 | 0.654 |
| 100 | 5 | 0.05 | 0.1 | 10.0 | RBF | 10.0 | 0.950 | 0.904 | 0.651 | 0.740 |
| 100 | 5 | 0.05 | 0.1 | 100.0 | RBF | 10.0 | 0.950 | 0.904 | 0.651 | 0.740 |
| 100 | 5 | 0.10 | 0.1 | 10.0 | RBF | 10.0 | 0.950 | 0.905 | 0.651 | 0.742 |
| 100 | 5 | 0.10 | 0.1 | 100.0 | RBF | 10.0 | 0.950 | 0.905 | 0.651 | 0.742 |
| 100 | 5 | 0.50 | 0.1 | 10.0 | RBF | 10.0 | 0.949 | 0.905 | 0.652 | 0.757 |
| 100 | 5 | 0.50 | 0.1 | 100.0 | RBF | 10.0 | 0.951 | 0.901 | 0.657 | 0.669 |
| 100 | 5 | 1.00 | 0.1 | 10.0 | RBF | 10.0 | 0.946 | 0.895 | 0.643 | 0.788 |
| 100 | 5 | 1.00 | 0.1 | 100.0 | RBF | 10.0 | 0.944 | 0.899 | 0.640 | 0.788 |
| 100 | 10 | 0.00 | 0.1 | 10.0 | RBF | 10.0 | 0.956 | 0.909 | 0.652 | 0.678 |
| 100 | 10 | 0.00 | 0.1 | 100.0 | RBF | 10.0 | 0.957 | 0.910 | 0.651 | 0.656 |
| 100 | 10 | 0.05 | 0.1 | 10.0 | RBF | 10.0 | 0.957 | 0.907 | 0.651 | 0.677 |
| 100 | 10 | 0.05 | 0.1 | 100.0 | RBF | 10.0 | 0.957 | 0.907 | 0.650 | 0.747 |
| 100 | 10 | 0.10 | 0.1 | 10.0 | RBF | 10.0 | 0.957 | 0.906 | 0.650 | 0.749 |
| 100 | 10 | 0.10 | 0.1 | 100.0 | RBF | 10.0 | 0.957 | 0.907 | 0.650 | 0.749 |
| 100 | 10 | 0.50 | 0.1 | 10.0 | RBF | 10.0 | 0.954 | 0.907 | 0.649 | 0.763 |
| 100 | 10 | 0.50 | 0.1 | 100.0 | RBF | 10.0 | 0.954 | 0.907 | 0.649 | 0.763 |
| 100 | 10 | 1.00 | 0.1 | 10.0 | RBF | 10.0 | 0.954 | 0.902 | 0.639 | 0.788 |
| 100 | 10 | 1.00 | 0.1 | 100.0 | RBF | 10.0 | 0.954 | 0.902 | 0.639 | 0.788 |
| 100 | 15 | 0.00 | 0.1 | 10.0 | RBF | 10.0 | 0.958 | 0.908 | 0.651 | 0.750 |
| 100 | 15 | 0.00 | 0.1 | 100.0 | RBF | 10.0 | 0.958 | 0.908 | 0.651 | 0.750 |
| 100 | 15 | 0.05 | 0.1 | 10.0 | RBF | 10.0 | 0.958 | 0.908 | 0.651 | 0.751 |
| 100 | 15 | 0.05 | 0.1 | 100.0 | RBF | 10.0 | 0.958 | 0.908 | 0.651 | 0.751 |
| 100 | 15 | 0.10 | 0.1 | 10.0 | RBF | 10.0 | 0.958 | 0.908 | 0.654 | 0.690 |
| 100 | 15 | 0.10 | 0.1 | 100.0 | RBF | 10.0 | 0.958 | 0.908 | 0.651 | 0.753 |
| 100 | 15 | 0.50 | 0.1 | 10.0 | RBF | 10.0 | 0.952 | 0.907 | 0.651 | 0.766 |

Continued on next page

TABLE S19 – continued from previous page

| n | d | $\alpha$ | $\beta$ | $\gamma$ | usim | $\sigma$ | AP@5 | AP@10 | sCI | CI |
|---|---|---|---|---|---|---|---|---|---|---|
| 100 | 15 | 0.50 | 0.1 | 100.0 | RBF | 10.0 | 0.952 | 0.906 | 0.650 | 0.766 |
| 100 | 15 | 1.00 | 0.1 | 10.0 | RBF | 10.0 | 0.947 | 0.896 | 0.640 | 0.787 |
| 100 | 15 | 1.00 | 0.1 | 100.0 | RBF | 10.0 | 0.947 | 0.896 | 0.640 | 0.787 |
| 150 | 5 | 0.00 | 0.1 | 10.0 | RBF | 10.0 | 0.951 | 0.910 | 0.655 | 0.671 |
| 150 | 5 | 0.00 | 0.1 | 100.0 | RBF | 10.0 | 0.950 | 0.911 | 0.656 | 0.670 |
| 150 | 5 | 0.05 | 0.1 | 10.0 | RBF | 10.0 | 0.950 | 0.908 | 0.656 | 0.675 |
| 150 | 5 | 0.05 | 0.1 | 100.0 | RBF | 10.0 | 0.948 | 0.905 | 0.654 | 0.743 |
| 150 | 5 | 0.10 | 0.1 | 10.0 | RBF | 10.0 | 0.947 | 0.905 | 0.654 | 0.745 |
| 150 | 5 | 0.10 | 0.1 | 100.0 | RBF | 10.0 | 0.950 | 0.906 | 0.659 | 0.644 |
| 150 | 5 | 0.50 | 0.1 | 10.0 | RBF | 10.0 | 0.948 | 0.900 | 0.661 | 0.665 |
| 150 | 5 | 0.50 | 0.1 | 100.0 | RBF | 10.0 | 0.947 | 0.896 | 0.664 | 0.670 |
| 150 | 5 | 1.00 | 0.1 | 10.0 | RBF | 10.0 | 0.946 | 0.895 | 0.642 | 0.789 |
| 150 | 5 | 1.00 | 0.1 | 100.0 | RBF | 10.0 | 0.947 | 0.900 | 0.640 | 0.789 |
| 150 | 10 | 0.00 | 0.1 | 10.0 | RBF | 10.0 | 0.952 | 0.908 | 0.655 | 0.679 |
| 150 | 10 | 0.00 | 0.1 | 100.0 | RBF | 10.0 | 0.951 | 0.909 | 0.655 | 0.677 |
| 150 | 10 | 0.05 | 0.1 | 10.0 | RBF | 10.0 | 0.951 | 0.907 | 0.656 | 0.683 |
| 150 | 10 | 0.05 | 0.1 | 100.0 | RBF | 10.0 | 0.953 | 0.903 | 0.657 | 0.659 |
| 150 | 10 | 0.10 | 0.1 | 10.0 | RBF | 10.0 | 0.950 | 0.905 | 0.652 | 0.752 |
| 150 | 10 | 0.10 | 0.1 | 100.0 | RBF | 10.0 | 0.950 | 0.905 | 0.653 | 0.752 |
| 150 | 10 | 0.50 | 0.1 | 10.0 | RBF | 10.0 | 0.952 | 0.907 | 0.651 | 0.766 |
| 150 | 10 | 0.50 | 0.1 | 100.0 | RBF | 10.0 | 0.952 | 0.907 | 0.651 | 0.766 |
| 150 | 10 | 1.00 | 0.1 | 10.0 | RBF | 10.0 | 0.949 | 0.903 | 0.641 | 0.789 |
| 150 | 10 | 1.00 | 0.1 | 100.0 | RBF | 10.0 | 0.949 | 0.903 | 0.641 | 0.789 |
| 150 | 15 | 0.00 | 0.1 | 10.0 | RBF | 10.0 | 0.955 | 0.908 | 0.654 | 0.753 |
| 150 | 15 | 0.00 | 0.1 | 100.0 | RBF | 10.0 | 0.954 | 0.907 | 0.653 | 0.753 |
| 150 | 15 | 0.05 | 0.1 | 10.0 | RBF | 10.0 | 0.954 | 0.908 | 0.654 | 0.755 |
| 150 | 15 | 0.05 | 0.1 | 100.0 | RBF | 10.0 | 0.953 | 0.908 | 0.654 | 0.755 |
| 150 | 15 | 0.10 | 0.1 | 10.0 | RBF | 10.0 | 0.953 | 0.908 | 0.654 | 0.756 |
| 150 | 15 | 0.10 | 0.1 | 100.0 | RBF | 10.0 | 0.954 | 0.908 | 0.654 | 0.756 |
| 150 | 15 | 0.50 | 0.1 | 10.0 | RBF | 10.0 | 0.951 | 0.907 | 0.653 | 0.769 |
| 150 | 15 | 0.50 | 0.1 | 100.0 | RBF | 10.0 | 0.951 | 0.907 | 0.652 | 0.769 |
| 150 | 15 | 1.00 | 0.1 | 10.0 | RBF | 10.0 | 0.945 | 0.900 | 0.643 | 0.789 |
| 150 | 15 | 1.00 | 0.1 | 100.0 | RBF | 10.0 | 0.945 | 0.900 | 0.643 | 0.789 |
| 200 | 5 | 0.00 | 0.1 | 10.0 | RBF | 10.0 | 0.943 | 0.907 | 0.656 | 0.671 |
| 200 | 5 | 0.00 | 0.1 | 100.0 | RBF | 10.0 | 0.942 | 0.904 | 0.657 | 0.648 |
| 200 | 5 | 0.05 | 0.1 | 10.0 | RBF | 10.0 | 0.940 | 0.902 | 0.656 | 0.746 |
| 200 | 5 | 0.05 | 0.1 | 100.0 | RBF | 10.0 | 0.940 | 0.902 | 0.656 | 0.746 |
| 200 | 5 | 0.10 | 0.1 | 10.0 | RBF | 10.0 | 0.943 | 0.900 | 0.658 | 0.665 |
| 200 | 5 | 0.10 | 0.1 | 100.0 | RBF | 10.0 | 0.940 | 0.902 | 0.656 | 0.748 |
| 200 | 5 | 0.50 | 0.1 | 10.0 | RBF | 10.0 | 0.940 | 0.902 | 0.657 | 0.763 |
| 200 | 5 | 0.50 | 0.1 | 100.0 | RBF | 10.0 | 0.942 | 0.896 | 0.668 | 0.668 |
| 200 | 5 | 1.00 | 0.1 | 10.0 | RBF | 10.0 | 0.937 | 0.897 | 0.646 | 0.790 |
| 200 | 5 | 1.00 | 0.1 | 100.0 | RBF | 10.0 | 0.937 | 0.898 | 0.644 | 0.790 |
| 200 | 10 | 0.00 | 0.1 | 10.0 | RBF | 10.0 | 0.946 | 0.906 | 0.656 | 0.680 |
| 200 | 10 | 0.00 | 0.1 | 100.0 | RBF | 10.0 | 0.946 | 0.905 | 0.656 | 0.678 |
| 200 | 10 | 0.05 | 0.1 | 10.0 | RBF | 10.0 | 0.947 | 0.906 | 0.657 | 0.684 |
| 200 | 10 | 0.05 | 0.1 | 100.0 | RBF | 10.0 | 0.945 | 0.906 | 0.657 | 0.683 |
| 200 | 10 | 0.10 | 0.1 | 10.0 | RBF | 10.0 | 0.944 | 0.903 | 0.654 | 0.755 |
| 200 | 10 | 0.10 | 0.1 | 100.0 | RBF | 10.0 | 0.944 | 0.903 | 0.654 | 0.755 |
| 200 | 10 | 0.50 | 0.1 | 10.0 | RBF | 10.0 | 0.944 | 0.901 | 0.653 | 0.768 |
| 200 | 10 | 0.50 | 0.1 | 100.0 | RBF | 10.0 | 0.944 | 0.901 | 0.653 | 0.769 |
| 200 | 10 | 1.00 | 0.1 | 10.0 | RBF | 10.0 | 0.937 | 0.893 | 0.644 | 0.790 |
| 200 | 10 | 1.00 | 0.1 | 100.0 | RBF | 10.0 | 0.937 | 0.893 | 0.644 | 0.790 |
| 200 | 15 | 0.00 | 0.1 | 10.0 | RBF | 10.0 | 0.948 | 0.907 | 0.657 | 0.685 |
| 200 | 15 | 0.00 | 0.1 | 100.0 | RBF | 10.0 | 0.949 | 0.906 | 0.657 | 0.683 |
| 200 | 15 | 0.05 | 0.1 | 10.0 | RBF | 10.0 | 0.947 | 0.906 | 0.659 | 0.690 |
| 200 | 15 | 0.05 | 0.1 | 100.0 | RBF | 10.0 | 0.947 | 0.906 | 0.658 | 0.688 |
| 200 | 15 | 0.10 | 0.1 | 10.0 | RBF | 10.0 | 0.946 | 0.905 | 0.659 | 0.693 |

Continued on next page

TABLE S19 – continued from previous page

| n | d | $\alpha$ | $\beta$ | $\gamma$ | usim | $\sigma$ | AP@5 | AP@10 | sCI | CI |
|---|---|---|---|---|---|---|---|---|---|---|
| 200 | 15 | 0.10 | 0.1 | 100.0 | RBF | 10.0 | 0.946 | 0.902 | 0.655 | 0.759 |
| 200 | 15 | 0.50 | 0.1 | 10.0 | RBF | 10.0 | 0.944 | 0.900 | 0.653 | 0.771 |
| 200 | 15 | 0.50 | 0.1 | 100.0 | RBF | 10.0 | 0.944 | 0.900 | 0.653 | 0.772 |
| 200 | 15 | 1.00 | 0.1 | 10.0 | RBF | 10.0 | 0.935 | 0.891 | 0.644 | 0.790 |
| 200 | 15 | 1.00 | 0.1 | 100.0 | RBF | 10.0 | 0.935 | 0.890 | 0.644 | 0.790 |
| 250 | 5 | 0.00 | 0.1 | 10.0 | RBF | 10.0 | 0.945 | 0.908 | 0.659 | 0.671 |
| 250 | 5 | 0.00 | 0.1 | 100.0 | RBF | 10.0 | 0.945 | 0.909 | 0.659 | 0.670 |
| 250 | 5 | 0.05 | 0.1 | 10.0 | RBF | 10.0 | 0.944 | 0.906 | 0.660 | 0.675 |
| 250 | 5 | 0.05 | 0.1 | 100.0 | RBF | 10.0 | 0.941 | 0.904 | 0.658 | 0.749 |
| 250 | 5 | 0.10 | 0.1 | 10.0 | RBF | 10.0 | 0.944 | 0.906 | 0.662 | 0.676 |
| 250 | 5 | 0.10 | 0.1 | 100.0 | RBF | 10.0 | 0.944 | 0.902 | 0.662 | 0.660 |
| 250 | 5 | 0.50 | 0.1 | 10.0 | RBF | 10.0 | 0.943 | 0.899 | 0.663 | 0.682 |
| 250 | 5 | 0.50 | 0.1 | 100.0 | RBF | 10.0 | 0.942 | 0.903 | 0.660 | 0.765 |
| 250 | 5 | 1.00 | 0.1 | 10.0 | RBF | 10.0 | 0.940 | 0.900 | 0.649 | 0.792 |
| 250 | 5 | 1.00 | 0.1 | 100.0 | RBF | 10.0 | 0.940 | 0.898 | 0.646 | 0.792 |
| 250 | 10 | 0.00 | 0.1 | 10.0 | RBF | 10.0 | 0.947 | 0.900 | 0.651 | 0.783 |
| 250 | 10 | 0.00 | 0.1 | 100.0 | RBF | 10.0 | 0.946 | 0.901 | 0.648 | 0.788 |
| 250 | 10 | 0.05 | 0.1 | 10.0 | RBF | 10.0 | 0.946 | 0.900 | 0.648 | 0.788 |
| 250 | 10 | 0.05 | 0.1 | 100.0 | RBF | 10.0 | 0.946 | 0.900 | 0.648 | 0.788 |
| 250 | 10 | 0.10 | 0.1 | 10.0 | RBF | 10.0 | 0.946 | 0.900 | 0.648 | 0.788 |
| 250 | 10 | 0.10 | 0.1 | 100.0 | RBF | 10.0 | 0.946 | 0.900 | 0.648 | 0.788 |
| 250 | 10 | 0.50 | 0.1 | 10.0 | RBF | 10.0 | 0.947 | 0.903 | 0.656 | 0.771 |
| 250 | 10 | 0.50 | 0.1 | 100.0 | RBF | 10.0 | 0.947 | 0.903 | 0.656 | 0.771 |
| 250 | 10 | 1.00 | 0.1 | 10.0 | RBF | 10.0 | 0.944 | 0.899 | 0.646 | 0.792 |
| 250 | 10 | 1.00 | 0.1 | 100.0 | RBF | 10.0 | 0.944 | 0.899 | 0.646 | 0.792 |
| 250 | 15 | 0.00 | 0.1 | 10.0 | RBF | 10.0 | 0.949 | 0.904 | 0.657 | 0.759 |
| 250 | 15 | 0.00 | 0.1 | 100.0 | RBF | 10.0 | 0.948 | 0.905 | 0.657 | 0.752 |
| 250 | 15 | 0.05 | 0.1 | 10.0 | RBF | 10.0 | 0.949 | 0.904 | 0.656 | 0.761 |
| 250 | 15 | 0.05 | 0.1 | 100.0 | RBF | 10.0 | 0.949 | 0.904 | 0.656 | 0.761 |
| 250 | 15 | 0.10 | 0.1 | 10.0 | RBF | 10.0 | 0.949 | 0.904 | 0.656 | 0.762 |
| 250 | 15 | 0.10 | 0.1 | 100.0 | RBF | 10.0 | 0.949 | 0.904 | 0.656 | 0.762 |
| 250 | 15 | 0.50 | 0.1 | 10.0 | RBF | 10.0 | 0.946 | 0.903 | 0.656 | 0.774 |
| 250 | 15 | 0.50 | 0.1 | 100.0 | RBF | 10.0 | 0.947 | 0.903 | 0.656 | 0.774 |
| 250 | 15 | 1.00 | 0.1 | 10.0 | RBF | 10.0 | 0.937 | 0.895 | 0.647 | 0.791 |
| 250 | 15 | 1.00 | 0.1 | 100.0 | RBF | 10.0 | 0.937 | 0.895 | 0.647 | 0.791 |
| 300 | 5 | 0.00 | 0.1 | 10.0 | RBF | 10.0 | 0.944 | 0.908 | 0.658 | 0.673 |
| 300 | 5 | 0.00 | 0.1 | 100.0 | RBF | 10.0 | 0.944 | 0.908 | 0.658 | 0.672 |
| 300 | 5 | 0.05 | 0.1 | 10.0 | RBF | 10.0 | 0.940 | 0.905 | 0.656 | 0.751 |
| 300 | 5 | 0.05 | 0.1 | 100.0 | RBF | 10.0 | 0.940 | 0.905 | 0.656 | 0.751 |
| 300 | 5 | 0.10 | 0.1 | 10.0 | RBF | 10.0 | 0.940 | 0.904 | 0.657 | 0.753 |
| 300 | 5 | 0.10 | 0.1 | 100.0 | RBF | 10.0 | 0.940 | 0.904 | 0.657 | 0.753 |
| 300 | 5 | 0.50 | 0.1 | 10.0 | RBF | 10.0 | 0.939 | 0.903 | 0.658 | 0.767 |
| 300 | 5 | 0.50 | 0.1 | 100.0 | RBF | 10.0 | 0.940 | 0.903 | 0.658 | 0.767 |
| 300 | 5 | 1.00 | 0.1 | 10.0 | RBF | 10.0 | 0.939 | 0.899 | 0.647 | 0.792 |
| 300 | 5 | 1.00 | 0.1 | 100.0 | RBF | 10.0 | 0.939 | 0.898 | 0.645 | 0.792 |
| 300 | 10 | 0.00 | 0.1 | 10.0 | RBF | 10.0 | 0.946 | 0.907 | 0.658 | 0.683 |
| 300 | 10 | 0.00 | 0.1 | 100.0 | RBF | 10.0 | 0.945 | 0.902 | 0.647 | 0.788 |
| 300 | 10 | 0.05 | 0.1 | 10.0 | RBF | 10.0 | 0.945 | 0.908 | 0.659 | 0.687 |
| 300 | 10 | 0.05 | 0.1 | 100.0 | RBF | 10.0 | 0.946 | 0.907 | 0.656 | 0.759 |
| 300 | 10 | 0.10 | 0.1 | 10.0 | RBF | 10.0 | 0.947 | 0.907 | 0.655 | 0.760 |
| 300 | 10 | 0.10 | 0.1 | 100.0 | RBF | 10.0 | 0.946 | 0.907 | 0.655 | 0.760 |
| 300 | 10 | 0.50 | 0.1 | 10.0 | RBF | 10.0 | 0.946 | 0.904 | 0.654 | 0.773 |
| 300 | 10 | 0.50 | 0.1 | 100.0 | RBF | 10.0 | 0.946 | 0.905 | 0.654 | 0.773 |
| 300 | 10 | 1.00 | 0.1 | 10.0 | RBF | 10.0 | 0.941 | 0.900 | 0.644 | 0.792 |
| 300 | 10 | 1.00 | 0.1 | 100.0 | RBF | 10.0 | 0.941 | 0.900 | 0.644 | 0.792 |
| 300 | 15 | 0.00 | 0.1 | 10.0 | RBF | 10.0 | 0.948 | 0.906 | 0.656 | 0.762 |
| 300 | 15 | 0.00 | 0.1 | 100.0 | RBF | 10.0 | 0.944 | 0.905 | 0.657 | 0.741 |
| 300 | 15 | 0.05 | 0.1 | 10.0 | RBF | 10.0 | 0.947 | 0.905 | 0.656 | 0.763 |

Continued on next page

TABLE S19 – continued from previous page

| n | d | $\alpha$ | $\beta$ | $\gamma$ | usim | $\sigma$ | AP@5 | AP@10 | sCI | CI |
|---|---|---|---|---|---|---|---|---|---|---|
| 300 | 15 | 0.05 | 0.1 | 100.0 | RBF | 10.0 | 0.947 | 0.906 | 0.656 | 0.763 |
| 300 | 15 | 0.10 | 0.1 | 10.0 | RBF | 10.0 | 0.948 | 0.908 | 0.660 | 0.697 |
| 300 | 15 | 0.10 | 0.1 | 100.0 | RBF | 10.0 | 0.947 | 0.905 | 0.656 | 0.765 |
| 300 | 15 | 0.50 | 0.1 | 10.0 | RBF | 10.0 | 0.948 | 0.907 | 0.655 | 0.776 |
| 300 | 15 | 0.50 | 0.1 | 100.0 | RBF | 10.0 | 0.949 | 0.906 | 0.655 | 0.776 |
| 300 | 15 | 1.00 | 0.1 | 10.0 | RBF | 10.0 | 0.938 | 0.897 | 0.647 | 0.792 |
| 300 | 15 | 1.00 | 0.1 | 100.0 | RBF | 10.0 | 0.938 | 0.897 | 0.647 | 0.792 |
| 350 | 5 | 0.00 | 0.1 | 10.0 | RBF | 10.0 | 0.941 | 0.902 | 0.655 | 0.675 |
| 350 | 5 | 0.00 | 0.1 | 100.0 | RBF | 10.0 | 0.940 | 0.902 | 0.654 | 0.674 |
| 350 | 5 | 0.05 | 0.1 | 10.0 | RBF | 10.0 | 0.941 | 0.902 | 0.656 | 0.679 |
| 350 | 5 | 0.05 | 0.1 | 100.0 | RBF | 10.0 | 0.941 | 0.903 | 0.656 | 0.673 |
| 350 | 5 | 0.10 | 0.1 | 10.0 | RBF | 10.0 | 0.940 | 0.901 | 0.657 | 0.682 |
| 350 | 5 | 0.10 | 0.1 | 100.0 | RBF | 10.0 | 0.938 | 0.899 | 0.653 | 0.753 |
| 350 | 5 | 0.50 | 0.1 | 10.0 | RBF | 10.0 | 0.937 | 0.900 | 0.654 | 0.767 |
| 350 | 5 | 0.50 | 0.1 | 100.0 | RBF | 10.0 | 0.938 | 0.895 | 0.664 | 0.661 |
| 350 | 5 | 1.00 | 0.1 | 10.0 | RBF | 10.0 | 0.934 | 0.893 | 0.644 | 0.790 |
| 350 | 5 | 1.00 | 0.1 | 100.0 | RBF | 10.0 | 0.934 | 0.892 | 0.644 | 0.790 |
| 350 | 10 | 0.00 | 0.1 | 10.0 | RBF | 10.0 | 0.942 | 0.902 | 0.655 | 0.685 |
| 350 | 10 | 0.00 | 0.1 | 100.0 | RBF | 10.0 | 0.943 | 0.901 | 0.653 | 0.746 |
| 350 | 10 | 0.05 | 0.1 | 10.0 | RBF | 10.0 | 0.943 | 0.903 | 0.656 | 0.689 |
| 350 | 10 | 0.05 | 0.1 | 100.0 | RBF | 10.0 | 0.943 | 0.903 | 0.656 | 0.687 |
| 350 | 10 | 0.10 | 0.1 | 10.0 | RBF | 10.0 | 0.942 | 0.902 | 0.658 | 0.692 |
| 350 | 10 | 0.10 | 0.1 | 100.0 | RBF | 10.0 | 0.942 | 0.901 | 0.653 | 0.760 |
| 350 | 10 | 0.50 | 0.1 | 10.0 | RBF | 10.0 | 0.943 | 0.900 | 0.652 | 0.773 |
| 350 | 10 | 0.50 | 0.1 | 100.0 | RBF | 10.0 | 0.943 | 0.900 | 0.652 | 0.773 |
| 350 | 10 | 1.00 | 0.1 | 10.0 | RBF | 10.0 | 0.939 | 0.895 | 0.643 | 0.791 |
| 350 | 10 | 1.00 | 0.1 | 100.0 | RBF | 10.0 | 0.939 | 0.895 | 0.643 | 0.791 |
| 350 | 15 | 0.00 | 0.1 | 10.0 | RBF | 10.0 | 0.946 | 0.900 | 0.653 | 0.763 |
| 350 | 15 | 0.00 | 0.1 | 100.0 | RBF | 10.0 | 0.944 | 0.902 | 0.654 | 0.730 |
| 350 | 15 | 0.05 | 0.1 | 10.0 | RBF | 10.0 | 0.945 | 0.904 | 0.656 | 0.695 |
| 350 | 15 | 0.05 | 0.1 | 100.0 | RBF | 10.0 | 0.947 | 0.901 | 0.654 | 0.757 |
| 350 | 15 | 0.10 | 0.1 | 10.0 | RBF | 10.0 | 0.945 | 0.903 | 0.657 | 0.699 |
| 350 | 15 | 0.10 | 0.1 | 100.0 | RBF | 10.0 | 0.944 | 0.900 | 0.653 | 0.765 |
| 350 | 15 | 0.50 | 0.1 | 10.0 | RBF | 10.0 | 0.942 | 0.900 | 0.654 | 0.776 |
| 350 | 15 | 0.50 | 0.1 | 100.0 | RBF | 10.0 | 0.942 | 0.900 | 0.654 | 0.776 |
| 350 | 15 | 1.00 | 0.1 | 10.0 | RBF | 10.0 | 0.936 | 0.892 | 0.646 | 0.790 |
| 350 | 15 | 1.00 | 0.1 | 100.0 | RBF | 10.0 | 0.936 | 0.892 | 0.646 | 0.791 |
| 400 | 5 | 0.00 | 0.1 | 10.0 | RBF | 10.0 | 0.943 | 0.904 | 0.658 | 0.676 |
| 400 | 5 | 0.00 | 0.1 | 100.0 | RBF | 10.0 | 0.940 | 0.902 | 0.658 | 0.675 |
| 400 | 5 | 0.05 | 0.1 | 10.0 | RBF | 10.0 | 0.943 | 0.904 | 0.660 | 0.680 |
| 400 | 5 | 0.05 | 0.1 | 100.0 | RBF | 10.0 | 0.944 | 0.904 | 0.659 | 0.679 |
| 400 | 5 | 0.10 | 0.1 | 10.0 | RBF | 10.0 | 0.942 | 0.904 | 0.661 | 0.681 |
| 400 | 5 | 0.10 | 0.1 | 100.0 | RBF | 10.0 | 0.940 | 0.902 | 0.656 | 0.755 |
| 400 | 5 | 0.50 | 0.1 | 10.0 | RBF | 10.0 | 0.938 | 0.898 | 0.649 | 0.789 |
| 400 | 5 | 0.50 | 0.1 | 100.0 | RBF | 10.0 | 0.938 | 0.900 | 0.657 | 0.769 |
| 400 | 5 | 1.00 | 0.1 | 10.0 | RBF | 10.0 | 0.938 | 0.897 | 0.647 | 0.791 |
| 400 | 5 | 1.00 | 0.1 | 100.0 | RBF | 10.0 | 0.938 | 0.897 | 0.647 | 0.791 |
| 400 | 10 | 0.00 | 0.1 | 10.0 | RBF | 10.0 | 0.944 | 0.904 | 0.655 | 0.760 |
| 400 | 10 | 0.00 | 0.1 | 100.0 | RBF | 10.0 | 0.946 | 0.905 | 0.656 | 0.736 |
| 400 | 10 | 0.05 | 0.1 | 10.0 | RBF | 10.0 | 0.944 | 0.905 | 0.660 | 0.690 |
| 400 | 10 | 0.05 | 0.1 | 100.0 | RBF | 10.0 | 0.944 | 0.904 | 0.655 | 0.762 |
| 400 | 10 | 0.10 | 0.1 | 10.0 | RBF | 10.0 | 0.945 | 0.905 | 0.655 | 0.763 |
| 400 | 10 | 0.10 | 0.1 | 100.0 | RBF | 10.0 | 0.945 | 0.904 | 0.655 | 0.763 |
| 400 | 10 | 0.50 | 0.1 | 10.0 | RBF | 10.0 | 0.945 | 0.902 | 0.655 | 0.775 |
| 400 | 10 | 0.50 | 0.1 | 100.0 | RBF | 10.0 | 0.945 | 0.903 | 0.655 | 0.775 |
| 400 | 10 | 1.00 | 0.1 | 10.0 | RBF | 10.0 | 0.941 | 0.898 | 0.647 | 0.792 |
| 400 | 10 | 1.00 | 0.1 | 100.0 | RBF | 10.0 | 0.941 | 0.898 | 0.647 | 0.792 |
| 400 | 15 | 0.00 | 0.1 | 10.0 | RBF | 10.0 | 0.944 | 0.905 | 0.659 | 0.694 |

Continued on next page

TABLE S19 – continued from previous page

| n | d | $\alpha$ | $\beta$ | $\gamma$ | usim | $\sigma$ | AP@5 | AP@10 | sCI | CI |
|---|---|---|---|---|---|---|---|---|---|---|
| 400 | 15 | 0.00 | 0.1 | 100.0 | RBF | 10.0 | 0.946 | 0.907 | 0.661 | 0.657 |
| 400 | 15 | 0.05 | 0.1 | 10.0 | RBF | 10.0 | 0.946 | 0.906 | 0.660 | 0.697 |
| 400 | 15 | 0.05 | 0.1 | 100.0 | RBF | 10.0 | 0.942 | 0.902 | 0.657 | 0.743 |
| 400 | 15 | 0.10 | 0.1 | 10.0 | RBF | 10.0 | 0.947 | 0.906 | 0.661 | 0.701 |
| 400 | 15 | 0.10 | 0.1 | 100.0 | RBF | 10.0 | 0.945 | 0.903 | 0.656 | 0.760 |
| 400 | 15 | 0.50 | 0.1 | 10.0 | RBF | 10.0 | 0.944 | 0.901 | 0.656 | 0.778 |
| 400 | 15 | 0.50 | 0.1 | 100.0 | RBF | 10.0 | 0.943 | 0.901 | 0.656 | 0.778 |
| 400 | 15 | 1.00 | 0.1 | 10.0 | RBF | 10.0 | 0.937 | 0.893 | 0.649 | 0.792 |
| 400 | 15 | 1.00 | 0.1 | 100.0 | RBF | 10.0 | 0.937 | 0.893 | 0.649 | 0.792 |

The columns corresponding to "d", "$\alpha$", "$\beta$", "$\gamma$", "usim", and "$\sigma$" have the latent dimension, weighting factor, latent vector regularization parameter, cell line similarity regularization parameter, cell line similarity function, and parameter for rbf cell line similarity, respectively, for pLETORg.
